# Supplementary material for: QuadVerse: An Integrated Framework Aligning Visual-Physical Reality for Quadruped Simulation
Source: arXiv:2606.07118 source file (2026-06-08)
Supplement: Supplementary file 1 [file 8_appendix.tex]

\clearpage
\onecolumn

\makeatletter
\@ifundefined{appendices}{\appendix}{\appendices}
\makeatother

\makeatletter
\@ifundefined{thesubsectiondis}{}{%
}

\@ifundefined{@IEEEprocessthesectionargument}{}{%
  \def\@IEEEprocessthesectionargument#1{%
  \@ifmtarg{#1}{%
  \@IEEEappendixsavesection*{\appendixname~\thesectiondis}%
  \addcontentsline{toc}{section}{\appendixname~\thesection}}{%
  \@IEEEappendixsavesection*{\appendixname~\thesectiondis. #1}%
  \addcontentsline{toc}{section}{\appendixname~\thesection. #1}}}%
}
\makeatother

\newpage

\makeatletter
\global\@topnum 0
\def\Etoc@@startlocaltochook{%
  \global\let\etoclocaltop\Etoc@minf
  \setcounter{tocdepth}{3}%
}
\makeatother

\begin{center}
    \Huge \textbf{Appendix}
\end{center}

\etocsettocstyle{\section*{Table of Contents}}{}
\localtableofcontents

\vspace{1em}
\hrule
\vspace{2em}

\makeatletter
\global\@topnum 0
\makeatother

% !TeX root = ../../main.tex

\section{Details of Geometry-Anchored Reconstruction}
\label{app:reconstruction_details}

This section provides the detailed formulations of the geometry constraints used in our reconstruction pipeline. 
Our goal is not only to obtain photorealistic novel-view rendering, but also to recover surface geometry suitable for mesh extraction and downstream physical simulation.

\subsection{Geometry-Constrained Gaussian Optimization}
\label{app:geometry_constrained_gs}

We represent the scene as a set of 3D Gaussian primitives~\cite{kerbl3Dgaussians}. 
Each Gaussian is parameterized by a center position $\boldsymbol{\mu}_i \in \mathbb{R}^3$, covariance matrix $\boldsymbol{\Sigma}_i \in \mathbb{R}^{3\times3}$, opacity $\alpha_i$, and spherical harmonics coefficients $\boldsymbol{c}_i$. 
Although standard 3DGS provides efficient photorealistic rendering, its optimization is primarily driven by image reconstruction losses and may produce inaccurate surface geometry. 
To make the reconstructed scene suitable for collision mesh extraction, we incorporate several geometry-oriented regularization terms.

\paragraph{2D Planar Regularization.}
Following \cite{huang20242dgs}, we enforce a regularization term to flatten 3D Gaussian ellipsoids into 2D surfels. We minimize the scale component corresponding to the local z-axis (the smallest scale) to ensure primitives align with the physical surface:
\begin{equation}
    \mathcal{L}_{scale} = \sum_{i} \| \min(\boldsymbol{s}_{i,x}, \boldsymbol{s}_{i,y}, \boldsymbol{s}_{i,z}) \|_1
\end{equation}
where $\boldsymbol{s}_{i,\cdot}$ represents the scale factors of the $i$-th Gaussian along its local axes.

\paragraph{Unbiased Depth Rendering.}
To eliminate depth errors arising from the positional bias of weight accumulation in volumetric rendering, we adopt the unbiased depth rendering strategy proposed in \cite{chen2024pgsr}. This method analytically computes the intersection of rays with Gaussian planes to generate depth maps that accurately conform to the true geometric surface.

\paragraph{Multi-View Photometric Consistency.}
Relying solely on single-view reconstruction loss is insufficient for global geometric consistency. Inspired by \cite{campbell2008using, fu2022geo, chen2024pgsr}, we incorporate a multi-view photometric consistency loss. For a pixel $\mathbf{p}_r$ in a reference view $r$, we utilize the rendered depth $d_r$ and normal $\mathbf{n}_r$ to construct an induced homography $\mathbf{H}_{rn}$, warping the local patch to a neighboring view $n$. We constrain surface consistency by maximizing the Normalized Cross-Correlation (NCC):
\begin{equation}
    \mathcal{L}_{multi} = \frac{1}{|\mathcal{W}|} \sum_{\mathbf{p}_r \in \mathcal{W}} \left( 1 - \text{NCC}(\mathcal{P}(\mathbf{p}_r), \mathcal{P}(\mathbf{H}_{rn}\mathbf{p}_r)) \right)
\end{equation}
where $\mathcal{W}$ denotes the set of valid pixels and $\mathcal{P}(\cdot)$ represents the local patch centered at the pixel.

\subsection{Integration of Normal Priors}
\label{app:normal_prior}
Photometric consistency often degrades in texture-less or non-Lambertian regions. To enhance geometric fidelity, we utilize \cite{ye2024stablenormal} to predict a geometric normal map $\mathbf{N}_{prior}$ for each frame, serving as a prior to constrain the rendered normals $\mathbf{N}_{rend}$. The normal consistency loss $\mathcal{L}_{normal}$ is defined as:
\begin{equation}
    \omega_{img}(\mathbf{p}) = \left( \text{clip}\left( 1.0 - \|\nabla \boldsymbol{I}(\mathbf{p})\|, 0, 1 \right) \right)^2
\end{equation}
\begin{equation}
    \mathcal{L}_{normal} = \frac{1}{|\mathcal{\boldsymbol{W}}|} \sum_{\mathbf{p} \in \mathcal{W}} \omega_{img}(\mathbf{p}) \| \mathbf{N}_{prior}(\mathbf{p}) - \mathbf{N}_{rend}(\mathbf{p}) \|_1
\end{equation}
where $\|\nabla \boldsymbol{I}(\mathbf{p})\|$ is the magnitude of the image gradient. The weight $\omega_{img}$ adaptively attenuates the supervision in high-frequency texture regions.

\subsection{Overall Optimization Objective}
\label{app:overall_reconstruction_objective}

The final reconstruction objective combines the standard image reconstruction loss with the geometry-oriented regularization terms:
\begin{equation}
    \mathcal{L}_{recon}
    =
    \mathcal{L}_{rgb}
    +
    \lambda_{scale}\mathcal{L}_{scale}
    +
    \lambda_{multi}\mathcal{L}_{multi}
    +
    \lambda_{normal}\mathcal{L}_{normal},
    \label{eq:app_recon_objective}
\end{equation}
where $\mathcal{L}_{rgb}$ is the standard photometric rendering loss, and $\lambda_{scale}$, $\lambda_{multi}$, and $\lambda_{normal}$ are weighting coefficients. 
In our experiments, we set $\lambda_{scale}=100$, $\lambda_{multi}=0.15$, and $\lambda_{normal}=0.01$.

% !TeX root = ../../main.tex

\section{Details of Semantic Mesh-Based Contact Calibration}
\label{sec:supp_contact_calibration}

This section provides implementation details for the semantic mesh-based contact calibration described in the main paper. 
The calibration pipeline consists of three steps: semantic Gaussian training, mesh-level semantic propagation, and prior-posterior friction calibration. 

\subsection{Semantic Gaussian Training and Mesh Label Propagation}
\label{sec:supp_semantic_gaussian}

We define a compact set of terrain-level semantic classes for contact calibration, focusing on visually distinguishable categories that are relevant to foot-terrain interaction rather than fine-grained object recognition. 
Raw 2D segmentation labels are merged into a small number of contact-relevant terrain categories, such as \textit{hard ground}, \textit{grass}, \textit{snow/ice}, \textit{soil}, \textit{sand}, \textit{gravel}, \textit{wood}, \textit{tile}, and \textit{obstacle/background}. 
This merged label space preserves the terrain semantics needed for coarse physical reasoning while avoiding unnecessary visual granularity. 
The category set is not fixed and can be expanded or merged according to the semantic diversity of each reconstructed environment.

To associate semantic labels with the reconstructed 3D scene, we augment each Gaussian primitive with a learnable semantic feature vector $\boldsymbol{f}_i \in \mathbb{R}^{C}$, where $C$ is the number of merged semantic classes. 
During rendering, these 3D semantic features are splatted to the image plane in the same manner as color features, producing pixel-wise semantic logits $\boldsymbol{S}_{rend}$. 
We supervise the rendered semantic logits using pseudo-labels $\boldsymbol{L}_{pseudo}$ generated by a 2D segmentation model~\cite{chen2022vision}. 
The semantic loss is defined as
\begin{equation}
    \mathcal{L}_{sem}
    =
    \mathrm{CrossEntropy}
    \left(
    \boldsymbol{S}_{rend},
    \boldsymbol{L}_{pseudo}
    \right).
    \label{eq:supp_semantic_loss}
\end{equation}
This loss is jointly optimized with the photometric reconstruction loss and geometry regularization terms, yielding a 3DGS scene that is both geometrically consistent and semantically annotated.

After mesh extraction, we propagate the learned Gaussian semantics to the collision mesh. 
For each mesh face, we use its center point as the query point and retrieve the $K=5$ nearest Gaussian primitives in 3D space. 
Each neighboring Gaussian is assigned the semantic class with the largest feature logit, and the mesh-face label is determined by majority voting among the five neighbors. 
Small isolated regions can be merged into the neighboring majority class to avoid fragmented material assignments. 
The resulting per-face semantic labels define region-level terrain partitions for coarse friction assignment and posterior calibration.

\subsection{LLM-Assisted Coarse Friction Prior}
\label{sec:supp_llm_prior}

For each semantic terrain class, we query a commonsense reasoning model, GPT-4~\cite{achiam2023gpt}, to obtain a deterministic nominal friction coefficient. 
The LLM output is not treated as an exact physical measurement; instead, it provides a reasonable initialization for spatially varying contact parameters.
We use a fixed prompt template and deterministic decoding to ensure consistent output formatting across scenes.
The prompt takes the robot context and the list of semantic terrain labels as input, and returns a JSON object mapping each label to a scalar friction coefficient.
The prompt template is shown in Table~\ref{tab:supp_llm_prompt}.

\begin{table}[ht]
\centering
\caption{Prompt template used for LLM-assisted coarse friction prior initialization.}
\label{tab:supp_llm_prompt}
\begin{tcolorbox}[
    width=\linewidth,
    colback=gray!4,
    colframe=gray!50,
    boxrule=0.5pt,
    arc=2pt,
    left=8pt,
    right=8pt,
    top=4pt,
    bottom=4pt,
    fonttitle=\bfseries\small,
    title=LLM Prompt Template for Coarse Friction Prior,
]
\footnotesize
\setlength{\parskip}{5pt}

\noindent\textbf{System prompt.}
You are an expert in robotics simulation and terrain contact modeling.
Estimate coarse friction coefficients for a quadruped robot walking on different terrain surfaces.

\noindent\textbf{Robot context.}
\begin{itemize}[leftmargin=1.4em, itemsep=1pt, topsep=2pt, parsep=0pt]
    \item Robot: Unitree Go2 quadruped robot.
    \item Foot material: rubber foot pads.
    \item Robot weight: approximately 15\,kg.
\end{itemize}

\noindent\textbf{Task.}
Given a list of semantic terrain labels, assign one deterministic nominal friction coefficient to each terrain class.
The values should be coarse priors for simulation, not exact measured physical parameters.

\noindent\textbf{Constraints.}
\begin{itemize}[leftmargin=1.4em, itemsep=1pt, topsep=2pt, parsep=0pt]
    \item Each coefficient should be a float in $[0.0,\,1.5]$.
    \item Return only a JSON object.
    \item Do not include explanations.
\end{itemize}

\noindent\textbf{User input.}
List of semantic terrain labels:
\texttt{[class\_1, class\_2, \ldots, class\_N]}.
\end{tcolorbox}
\end{table}

The returned class names are normalized to match the semantic labels on the mesh. 
For regions whose nominal friction exceeds an empirical slip threshold, we directly keep the coarse prior because the robot trajectory is weakly affected by the exact value in this high-traction regime. 
The threshold is empirically set to $\mu_{\mathrm{slip}}=0.5$ based on preliminary replay experiments.
Posterior search is applied only to slip-prone semantic regions whose friction prior falls below this threshold.

\subsection{Trajectory-Based Posterior Friction Search}
\label{sec:supp_posterior_search}

For slip-prone regions, we refine the friction coefficient using real-world locomotion replay. 
The optimization variable is a single region-level friction coefficient $\mu_r$ for each slip-prone semantic region $r$, rather than a separate coefficient for every mesh face. 
This region-level parameterization keeps the search low-dimensional and matches the semantic partition used by the simulator.

As formulated in Eq.~\ref{eq:friction_search} of the main paper, posterior calibration selects the friction value that minimizes the trajectory discrepancy between simulated replay and real robot motion. In practice, the objective is evaluated over multiple recorded replay segments rather than a single trajectory. 
For each segment, we initialize the simulation from the recorded base pose and joint state, replay the recorded locomotion command sequence, and compute the mean base-position error against the corresponding recorded LiDAR-SLAM trajectory.

We use a one-dimensional grid search centered at the coarse prior $\mu_r^0$. 
Specifically, we search $\mu_r \in [\mu_r^0 - 0.2, \mu_r^0 + 0.2]$ with step size $\Delta\mu=0.01$, clipped to the valid simulator range. 
During the search for one slip-prone region, friction values of all other regions are kept fixed at their current priors. 
If multiple slip-prone regions are present, we calibrate them region by region.
After posterior search, the optimized friction coefficient $\mu_r^\star$ is assigned to all mesh faces belonging to the corresponding semantic region. 
The resulting contact-calibrated terrain is then used for residual dynamics compensation and downstream policy training.

% !TeX root = ../../main.tex

\section{Details of Residual Dynamics Compensation}
\label{sec:supp_dynamics_training}

\subsection{Network Architecture and State Space}
The residual dynamics policy is implemented as a Multilayer Perceptron (MLP) with two hidden layers of 128 units each, utilizing ELU activation functions. The network operates at the simulation control frequency (500 Hz).

We employ an asymmetric actor-critic architecture to leverage privileged information during training. 
\textbf{The policy network (actor)} uses only simulation-available observations so that it can be inserted into the simulation loop during replay and downstream policy fine-tuning.
Its input includes the target joint positions from the locomotion policy, proprioceptive joint positions and velocities, binary foot contact states, the gravity vector in the body frame, base height, body orientation, and the previous action. 
\textbf{The value network (critic)} augments this observation with ground-truth real-world signals to guide learning: real-world joint states, measured foot contact forces, base yaw rate, and true body orientation. 
To capture temporal dynamics and actuator delays, both networks stack a history window of the preceding 20 frames.

\subsection{Training Process and Initialization Strategy}
The training process is governed by specific termination criteria to ensure the learned residual dynamics remain within a valid distribution. An episode is terminated and reset if: (1) the playback trajectory reaches its end; (2) abnormal external forces are detected on the base; or (3) the simulated joint positions deviate from the real-world reference by more than 0.4 rad. Large deviations indicate that the simulation state has diverged significantly from the reference data, rendering subsequent samples uninformative for residual learning.

Upon reset, the simulation is initialized by sampling a timestamp from the recorded replay data. 
The recorded base pose is first transformed into the simulator frame aligned with the reconstructed mesh. 
The simulated robot's base pose and joint states are then initialized from the corresponding recorded values, while unobserved or noisy quantities such as base linear velocity are initialized using finite differences or set to zero for stability.

This incomplete state initialization inevitably introduces transient tracking errors at the beginning of an episode (a "cold start" problem). To mitigate the bias introduced by these initial transients, we do not impose a short fixed horizon for episodes. Instead, we allow the simulation to run until the end of the reference trajectory. This strategy provides a sufficiently long horizon for the dynamics to stabilize, ensuring that the gradient updates are dominated by the stable tracking phase rather than the initial alignment error.

\subsection{Reward Formulation}
The reward function is designed to balance joint-space tracking accuracy with gait plausibility. The detailed terms and their corresponding weights are enumerated in Table \ref{tab:reward_terms}.

\begin{table}[h]
\caption{Reward Terms for Dynamics Compensation}
\label{tab:reward_terms}
\centering
\renewcommand{\tabcolsep}{6pt}
\begin{tabular}{lcc}
\toprule
\textbf{Reward Component} & \textbf{Mathematical Term} & \textbf{Weight} \\
\midrule
\multicolumn{3}{c}{\textit{Joint Space Tracking}} \\
\midrule
Joint Pos. (Relaxed) & $\exp(-2.5\|\mathbf{q}_{real} - \mathbf{q}_{sim}\|_2^2)$ & $100.0$ \\
Joint Pos. (Moderate) & $\exp(-20\|\mathbf{q}_{real} - \mathbf{q}_{sim}\|_2^2)$ & $100.0$ \\
Joint Pos. (Strict) & $\exp(-100\|\mathbf{q}_{real} - \mathbf{q}_{sim}\|_2^2)$ & $100.0$ \\
\midrule
\multicolumn{3}{c}{\textit{Gait and Contact Imitation}} \\
\midrule
Foot Contact & $\mathbb{I}(F_{sim} > 10 \land F_{real} > 20)$ & $100.0$ \\
Foot Slip Penalty & $\exp(-10\|\mathbf{v}_{foot, xy}^{sim}\|_2^2)$ & $100.0$ \\
Base Linear Vel. (Z) & $\exp(-10\|\mathbf{v}_{z}^{sim}\|_2^2)$ & $50.0$ \\
Ang. Vel. (Yaw) & $\exp(-4\|\omega_{yaw}^{real} - \omega_{yaw}^{sim}\|_2^2)$ & $100.0$ \\
\midrule
\multicolumn{3}{c}{\textit{Regularization}} \\
\midrule
Action Rate & $\exp(-\|\mathbf{a}_{t} - \mathbf{a}_{t-1}\|_2^2)$ & $5.0$ \\
Action Norm & $\exp(-0.01 \|\mathbf{a}_{t}\|_2^2)$ & $100.0$ \\
\bottomrule
\end{tabular}
\end{table}

% !TeX root = ../../main.tex

\section{Additional Qualitative Results of Scene Reconstruction}
\label{sec:supp_reconstruction_results}

Figure~\ref{fig:qualitative_more} shows additional qualitative reconstruction results across multiple outdoor scenarios. From left to right, the four key components are as follows: (a) the rendered RGB image, (b) the rendered normal map, (c) the extracted mesh, and (d) the simulated robot perspective, with the camera viewpoint lowered to mimic the view of a quadruped robot like Go2. These results showcase the strong visual realism, accurate geometric reconstruction, and alignment with the robot's perceptual perspective.

\begin{figure*}[p]
    \centering
    \setlength{\tabcolsep}{1pt}

    \begin{tabular}{cccc}
        \includegraphics[width=0.24\linewidth]{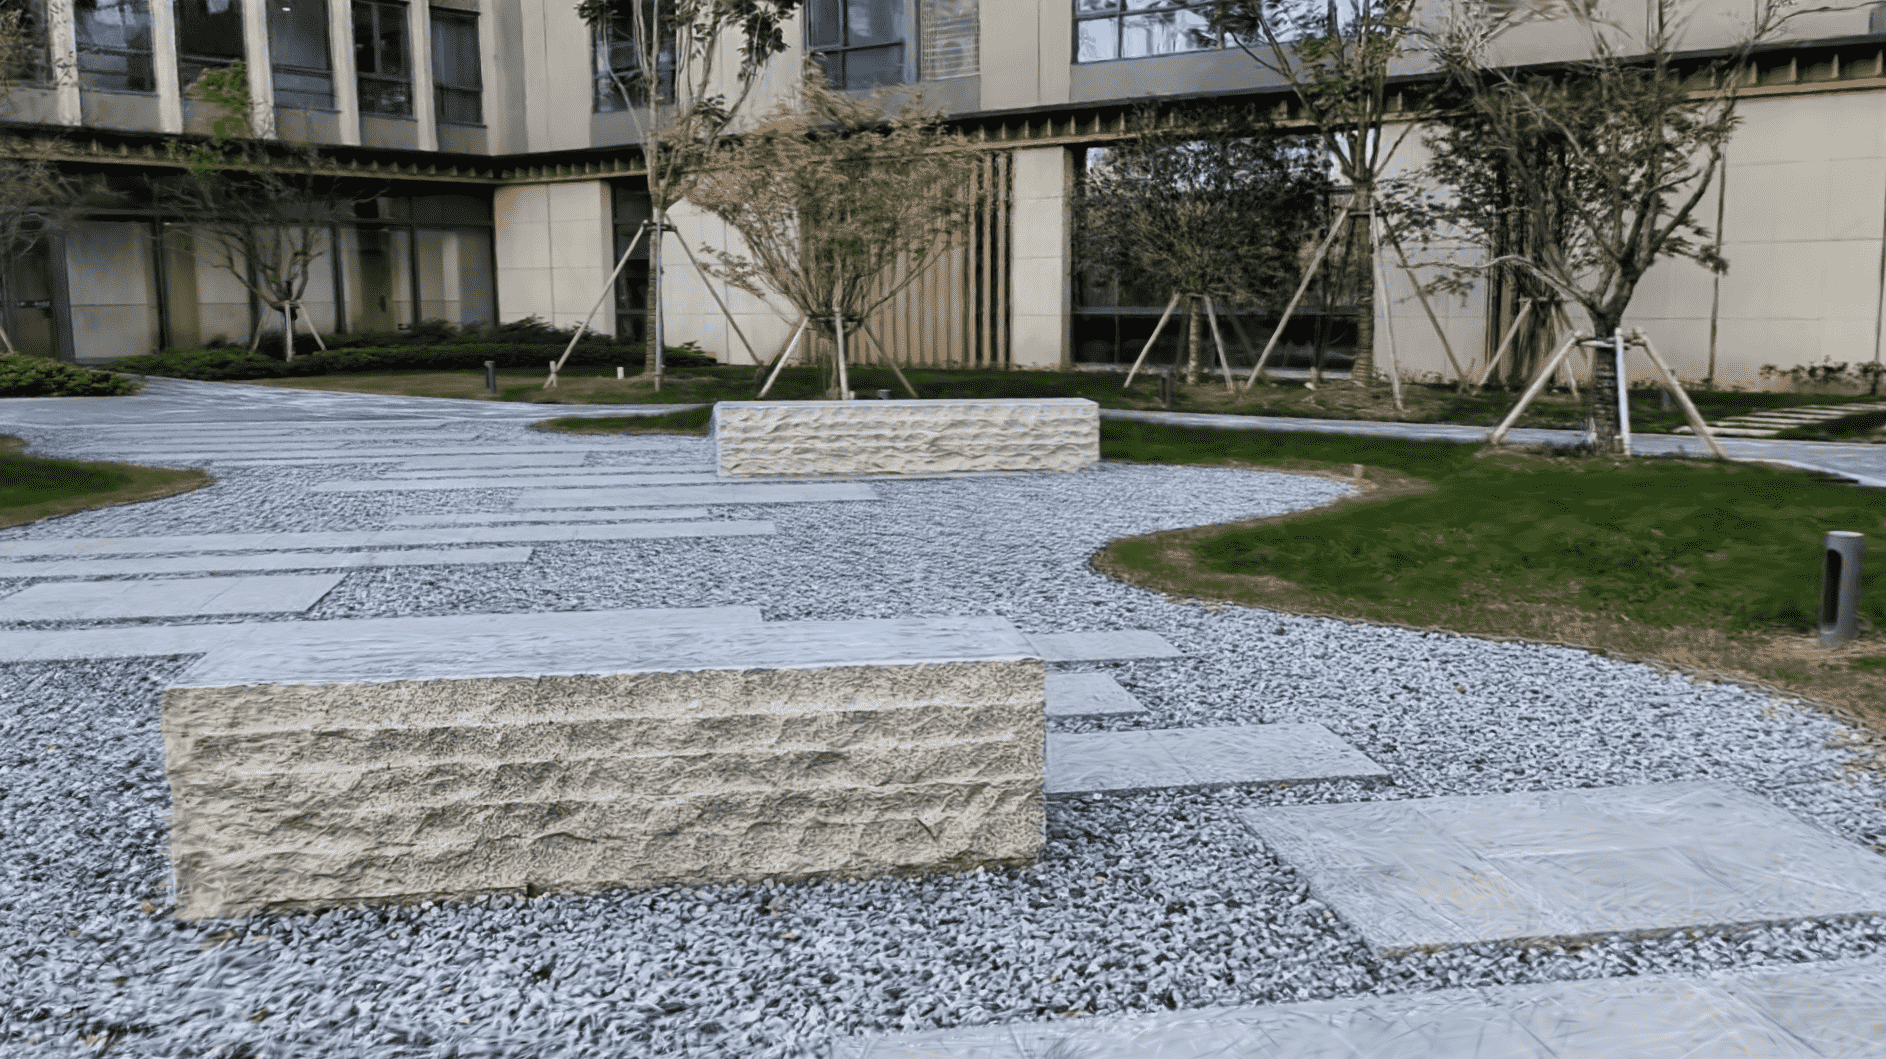} &
        \includegraphics[width=0.24\linewidth]{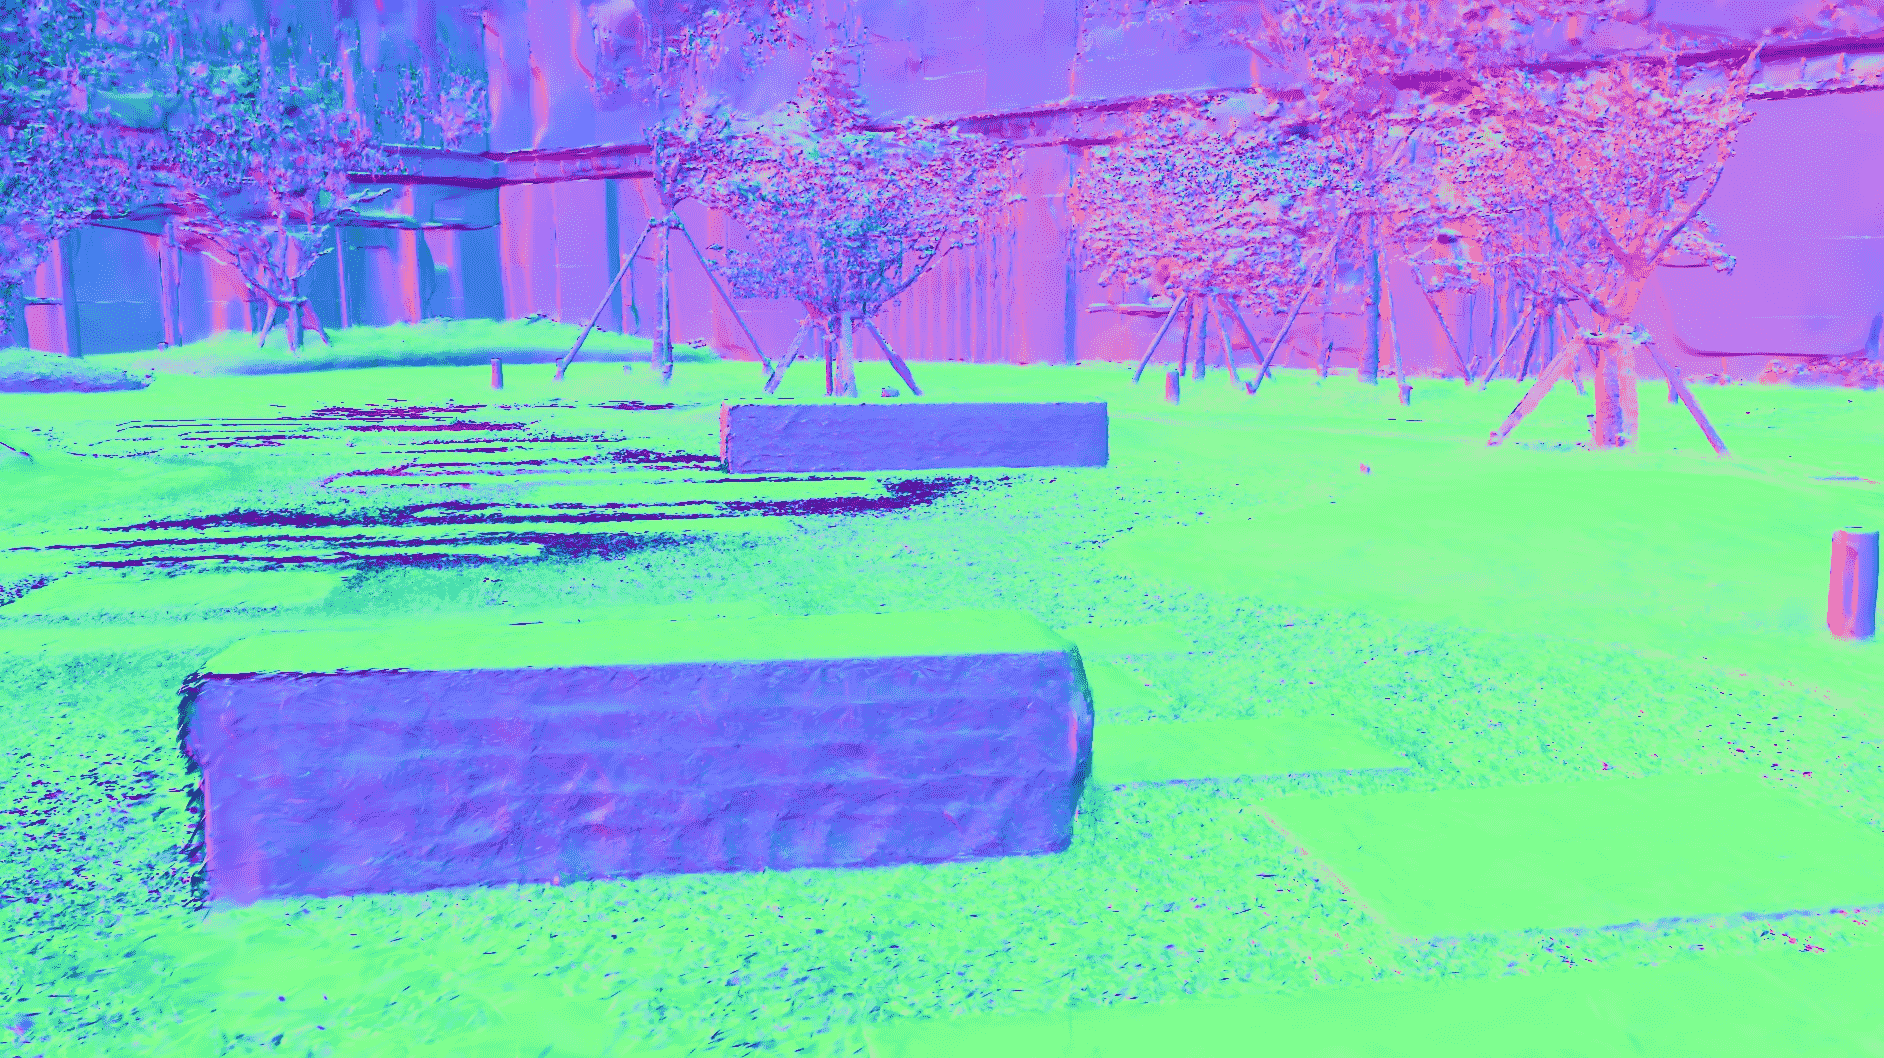} &
        \includegraphics[width=0.24\linewidth]{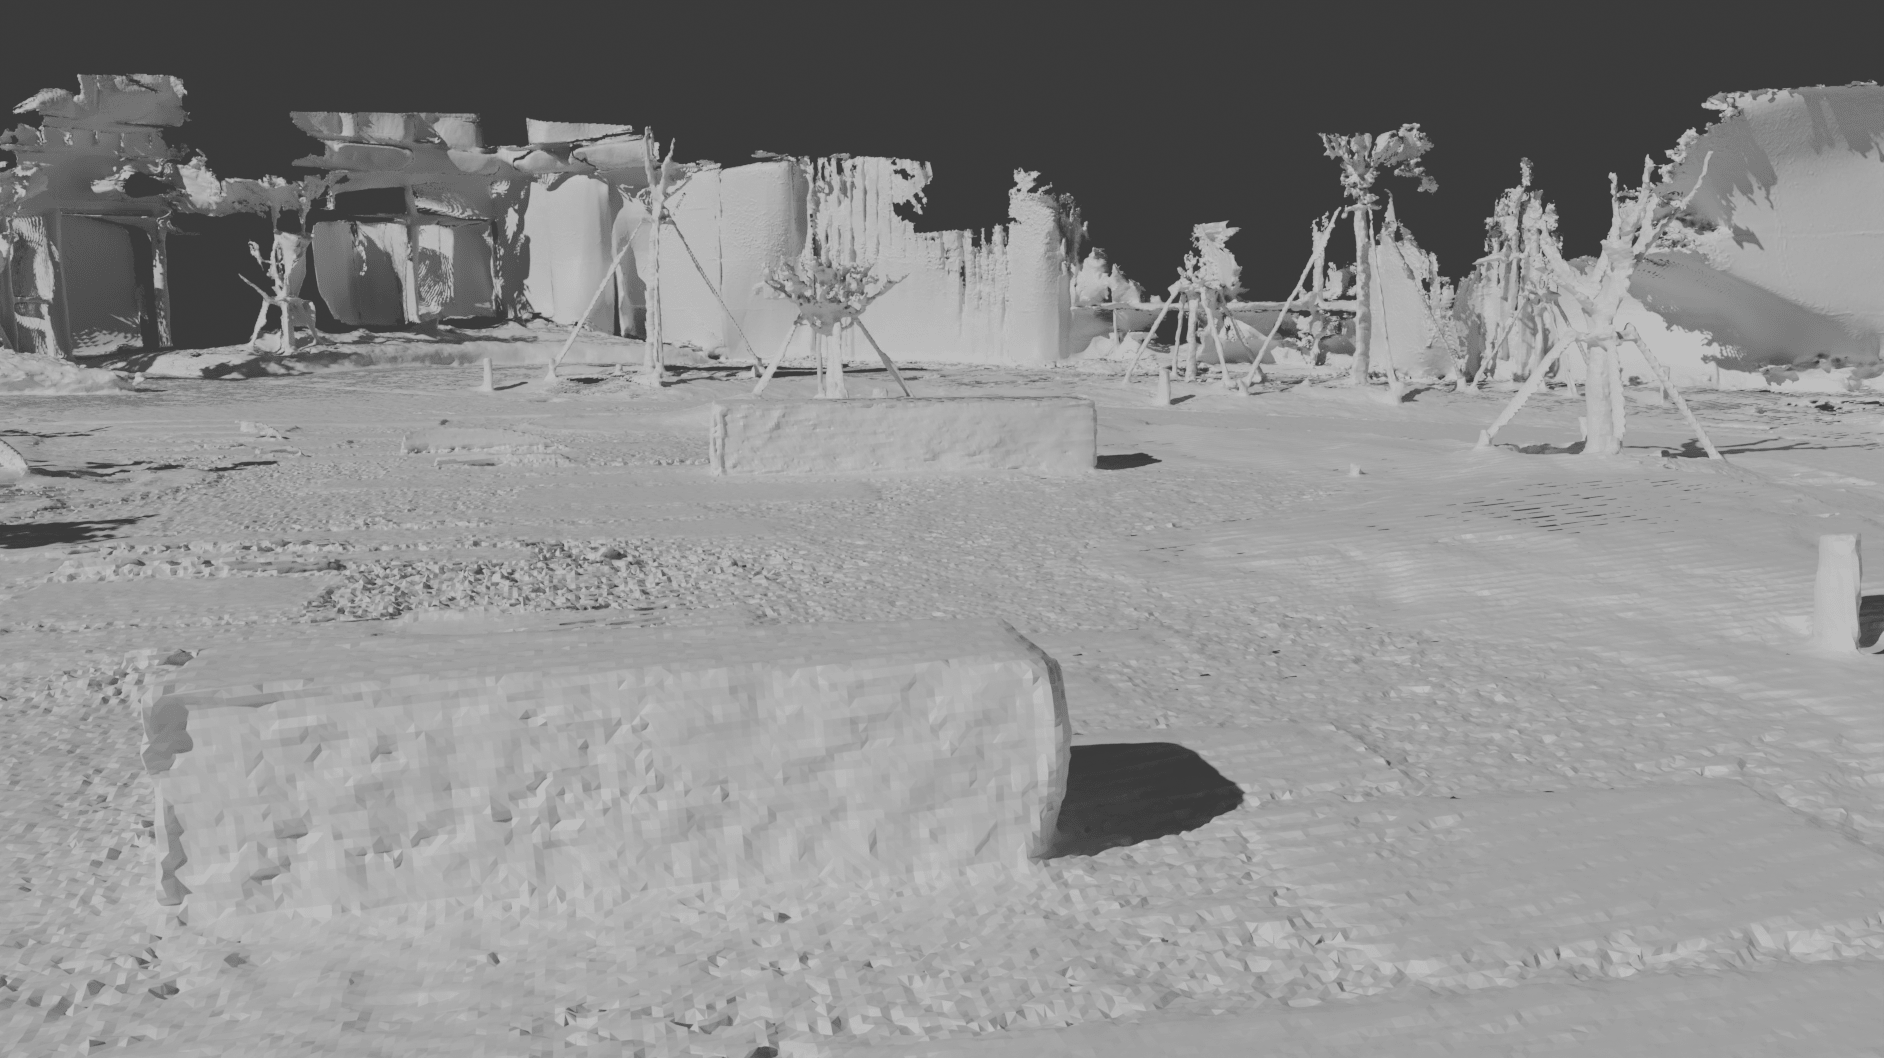} &
        \includegraphics[width=0.24\linewidth]{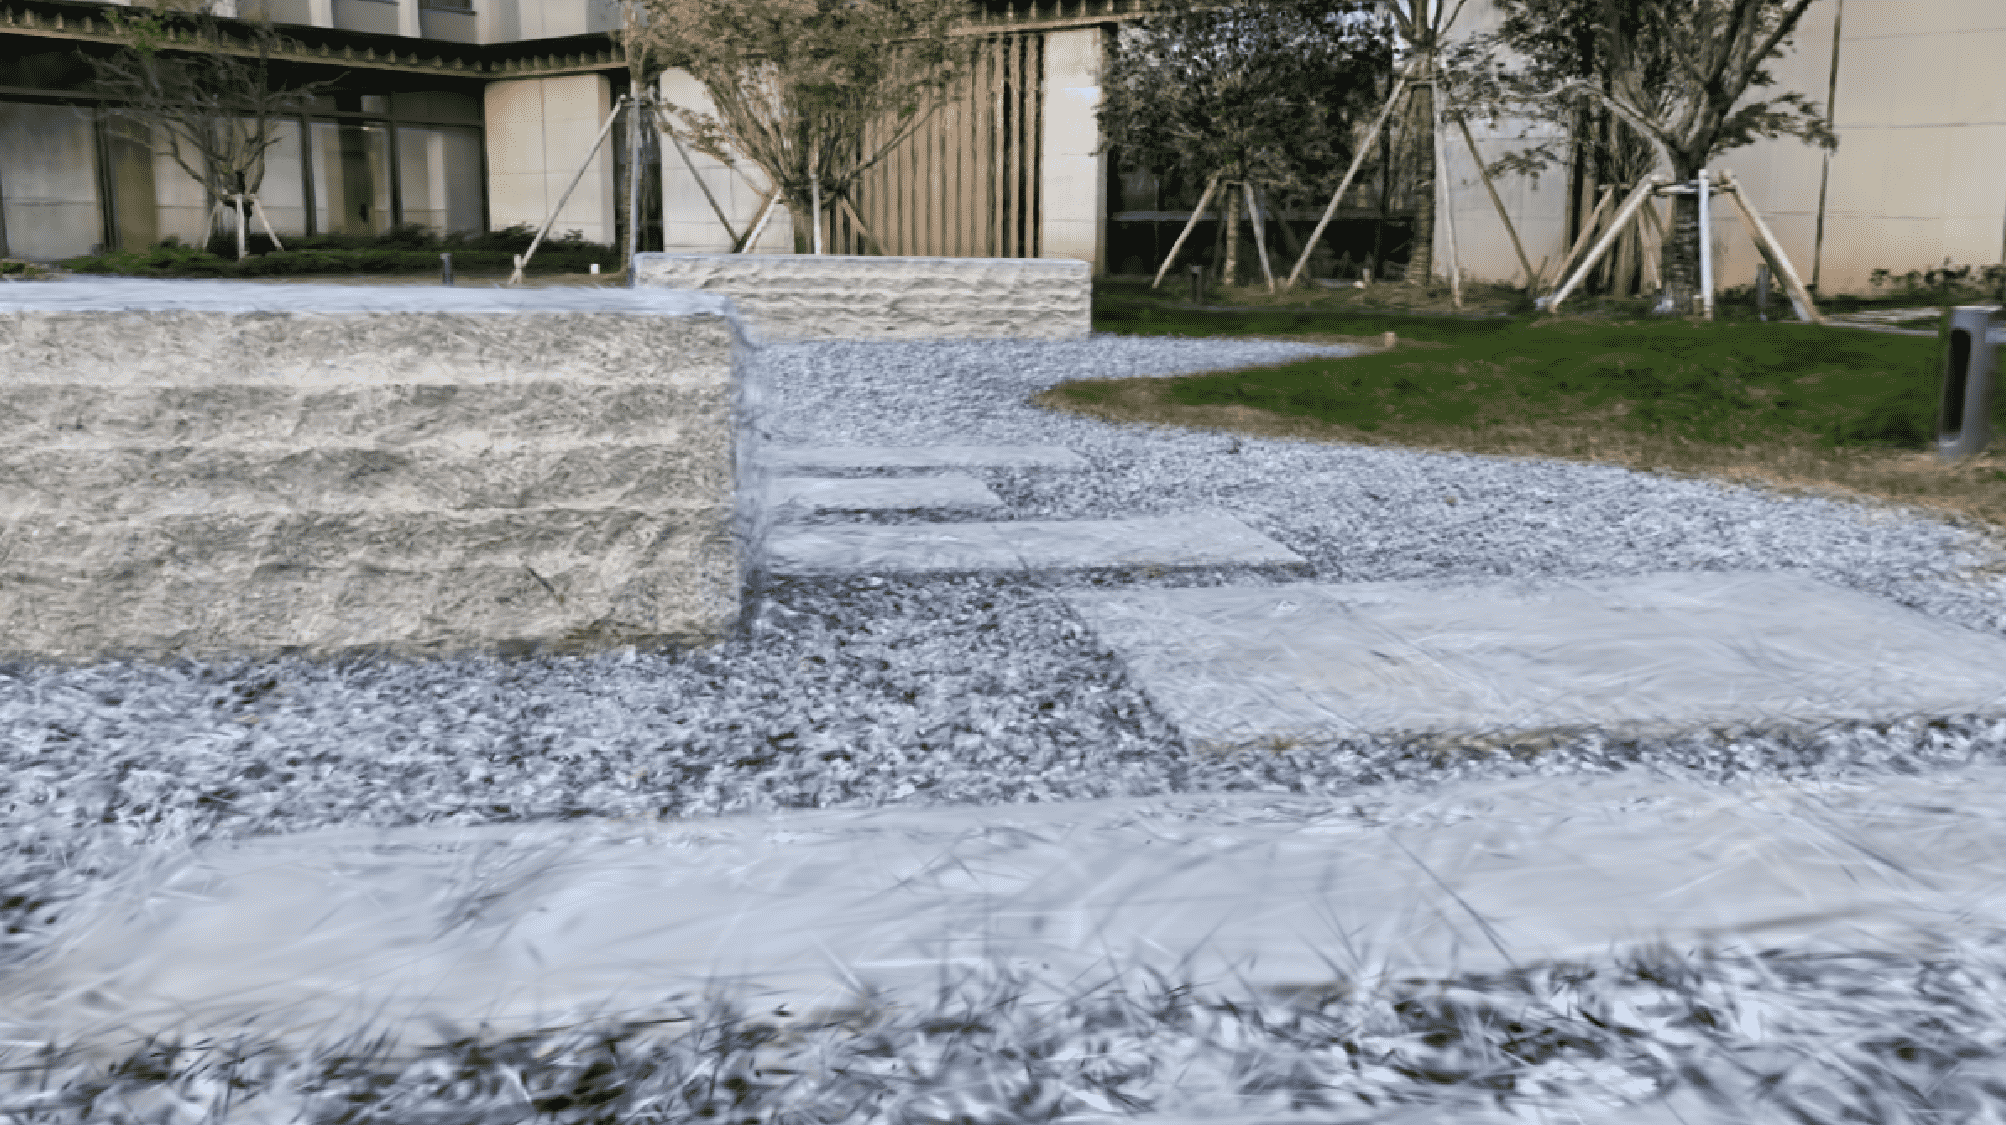} \\

        \includegraphics[width=0.24\linewidth]{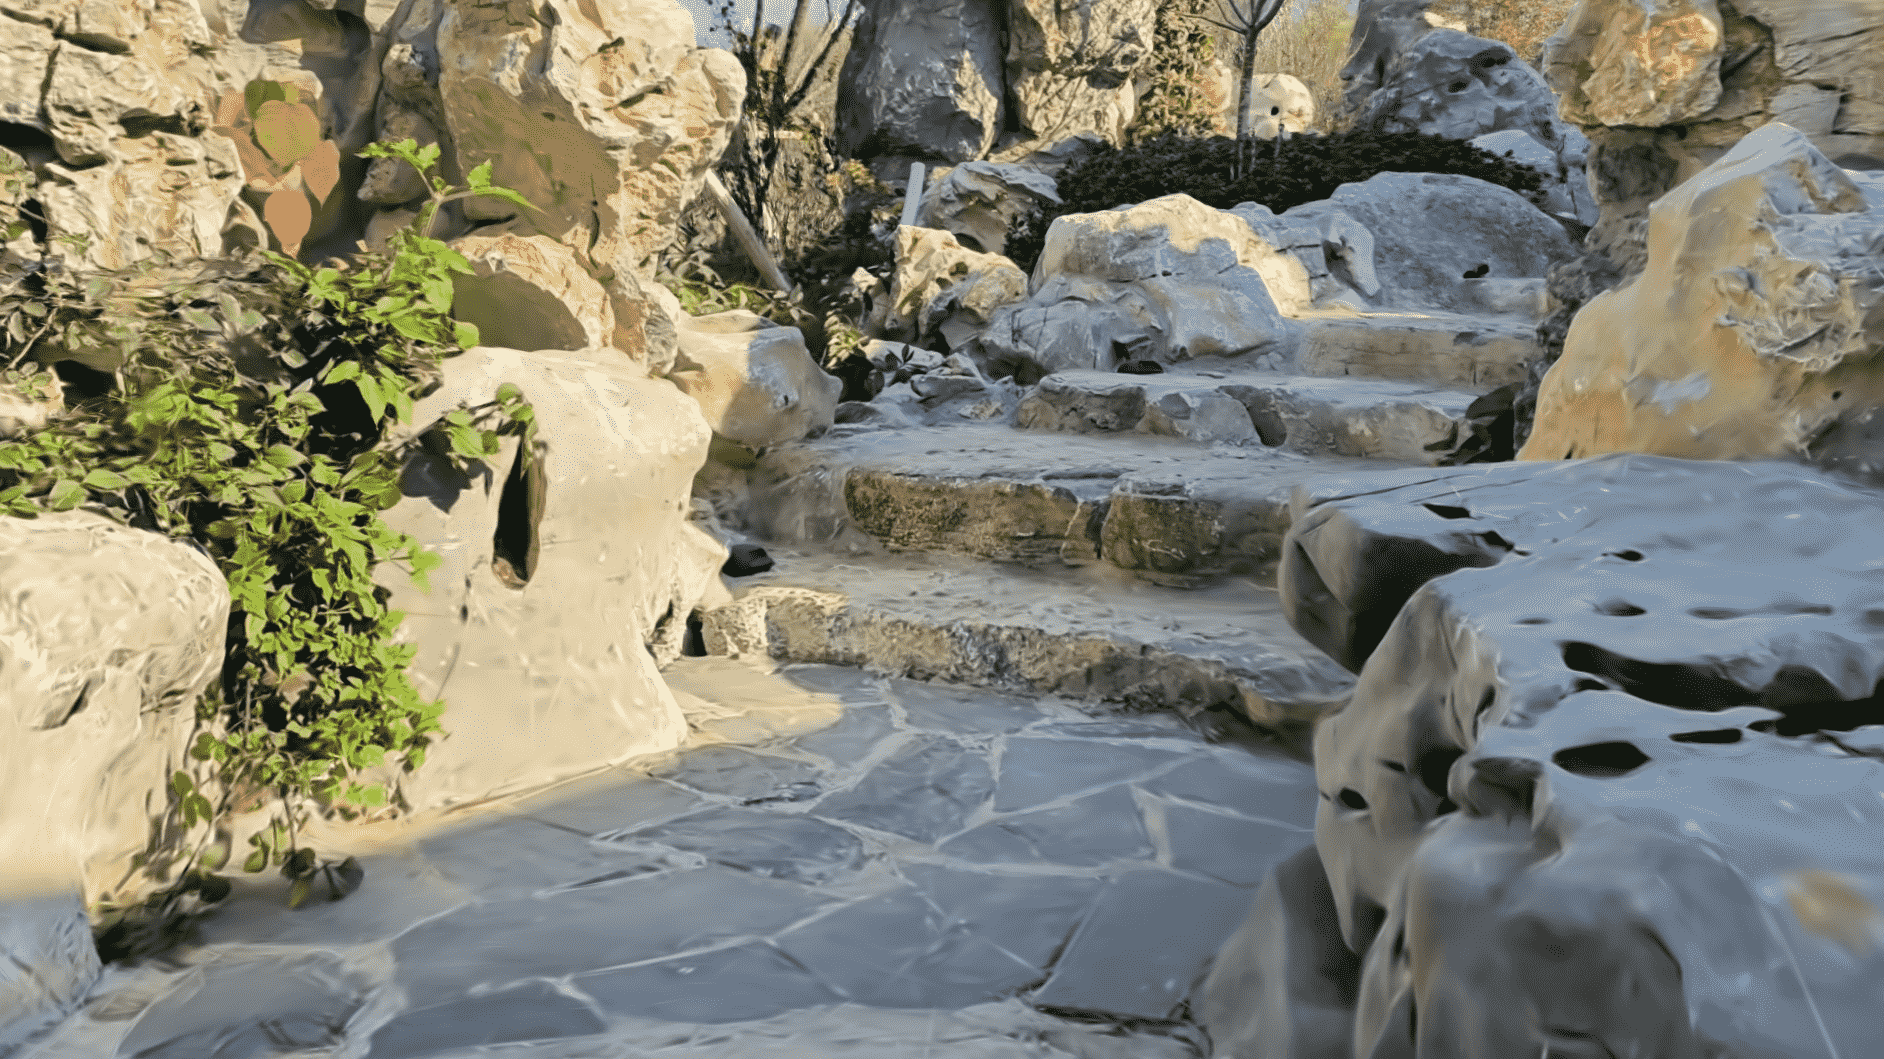} &
        \includegraphics[width=0.24\linewidth]{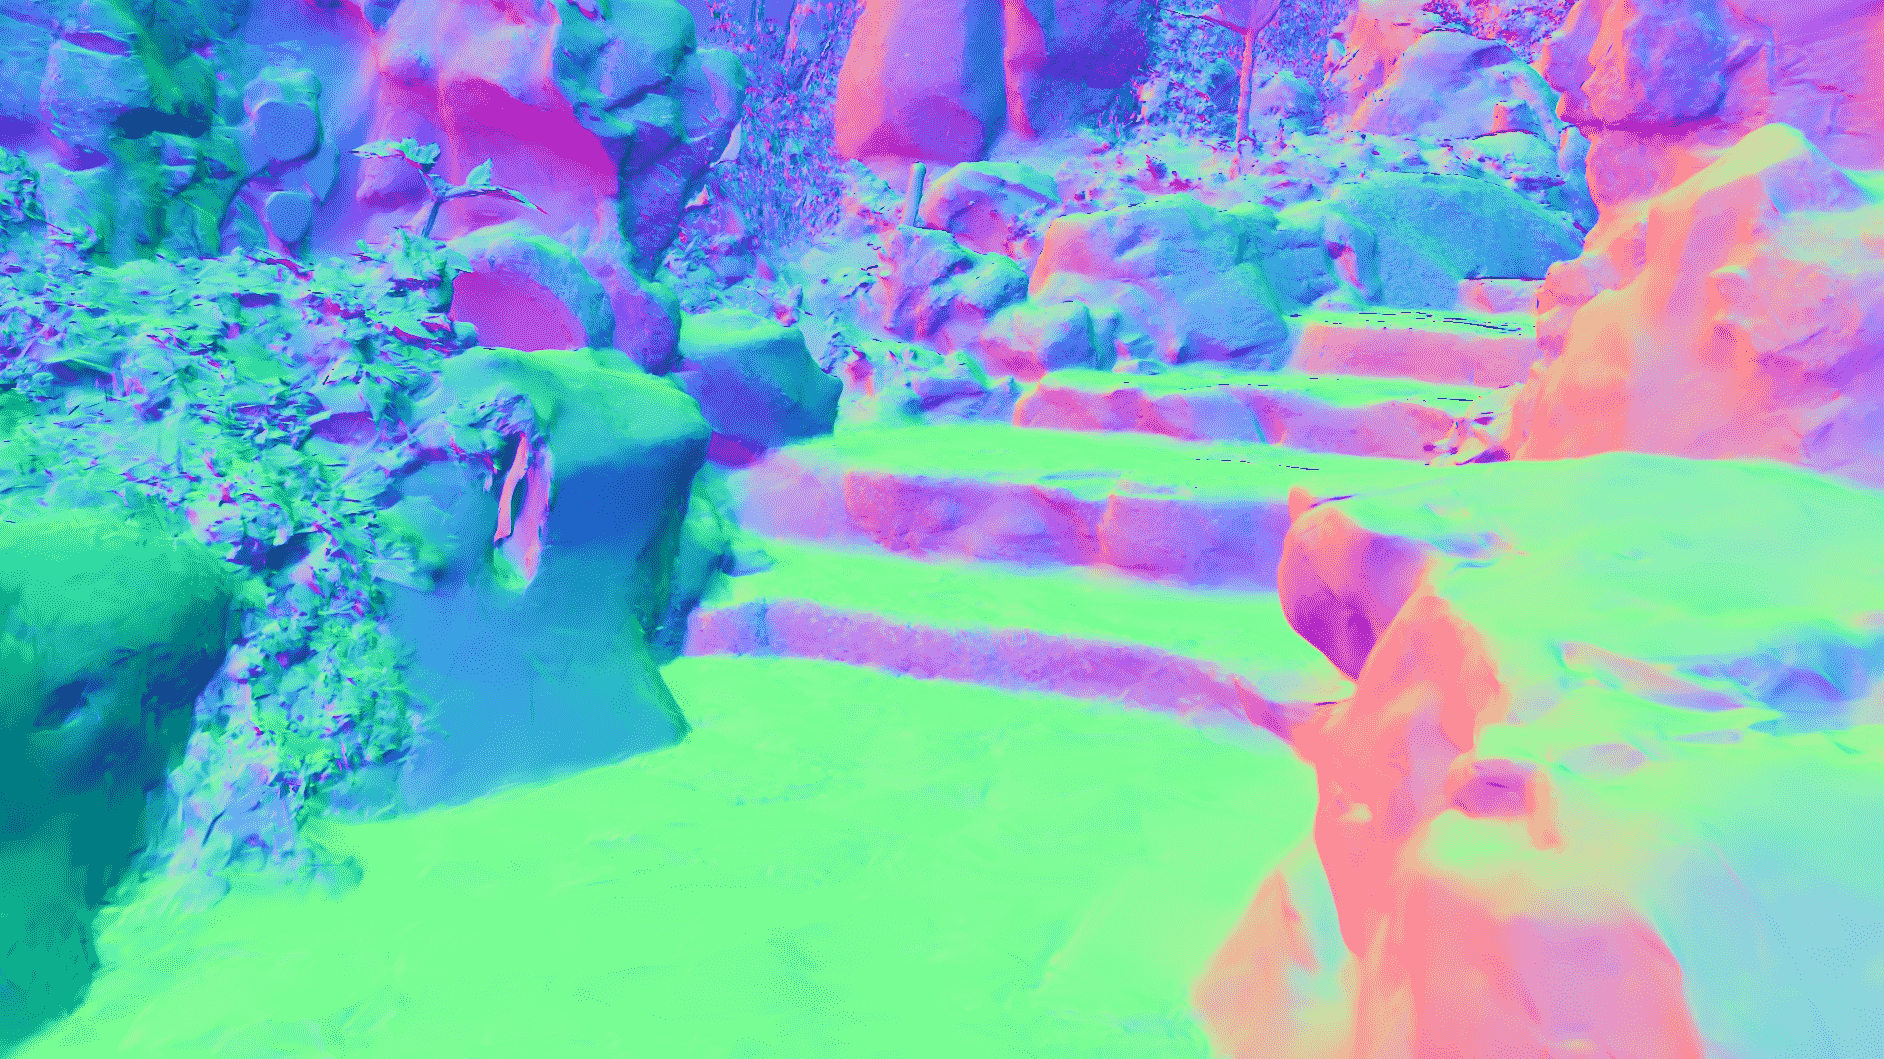} &
        \includegraphics[width=0.24\linewidth]{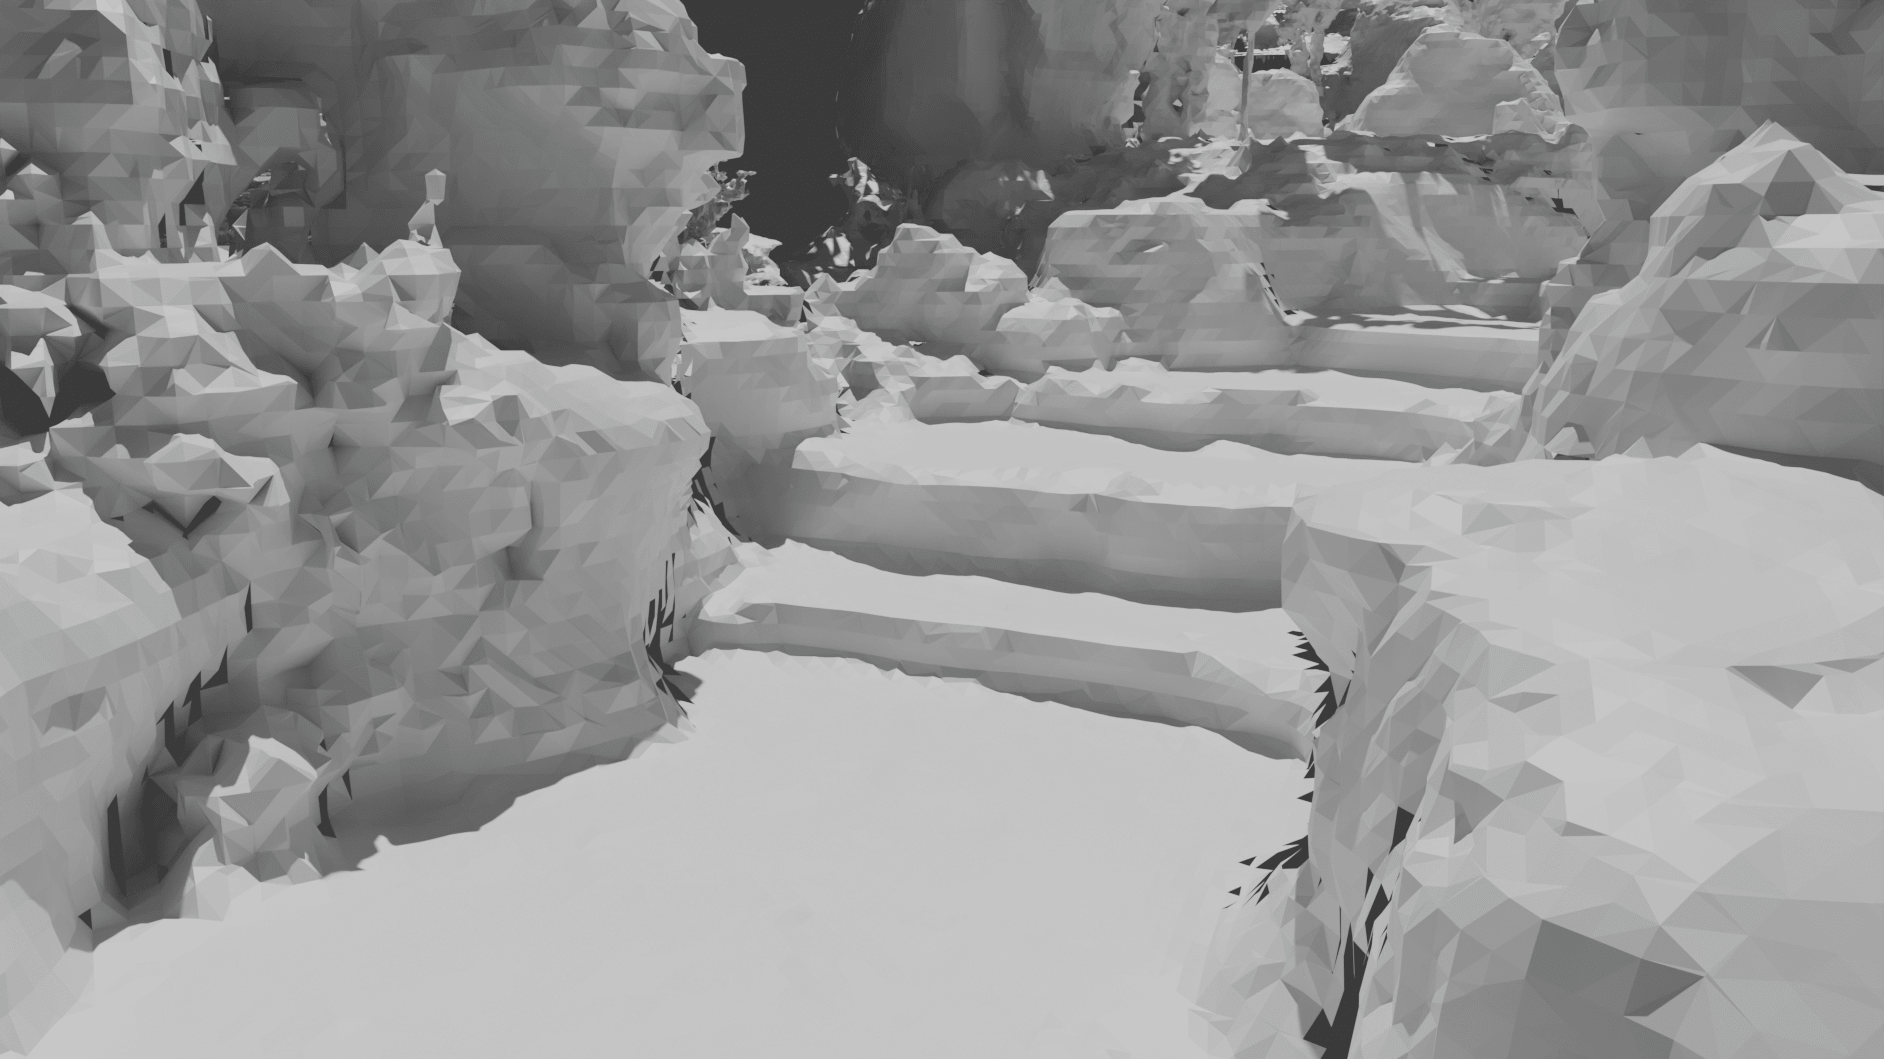} &
        \includegraphics[width=0.24\linewidth]{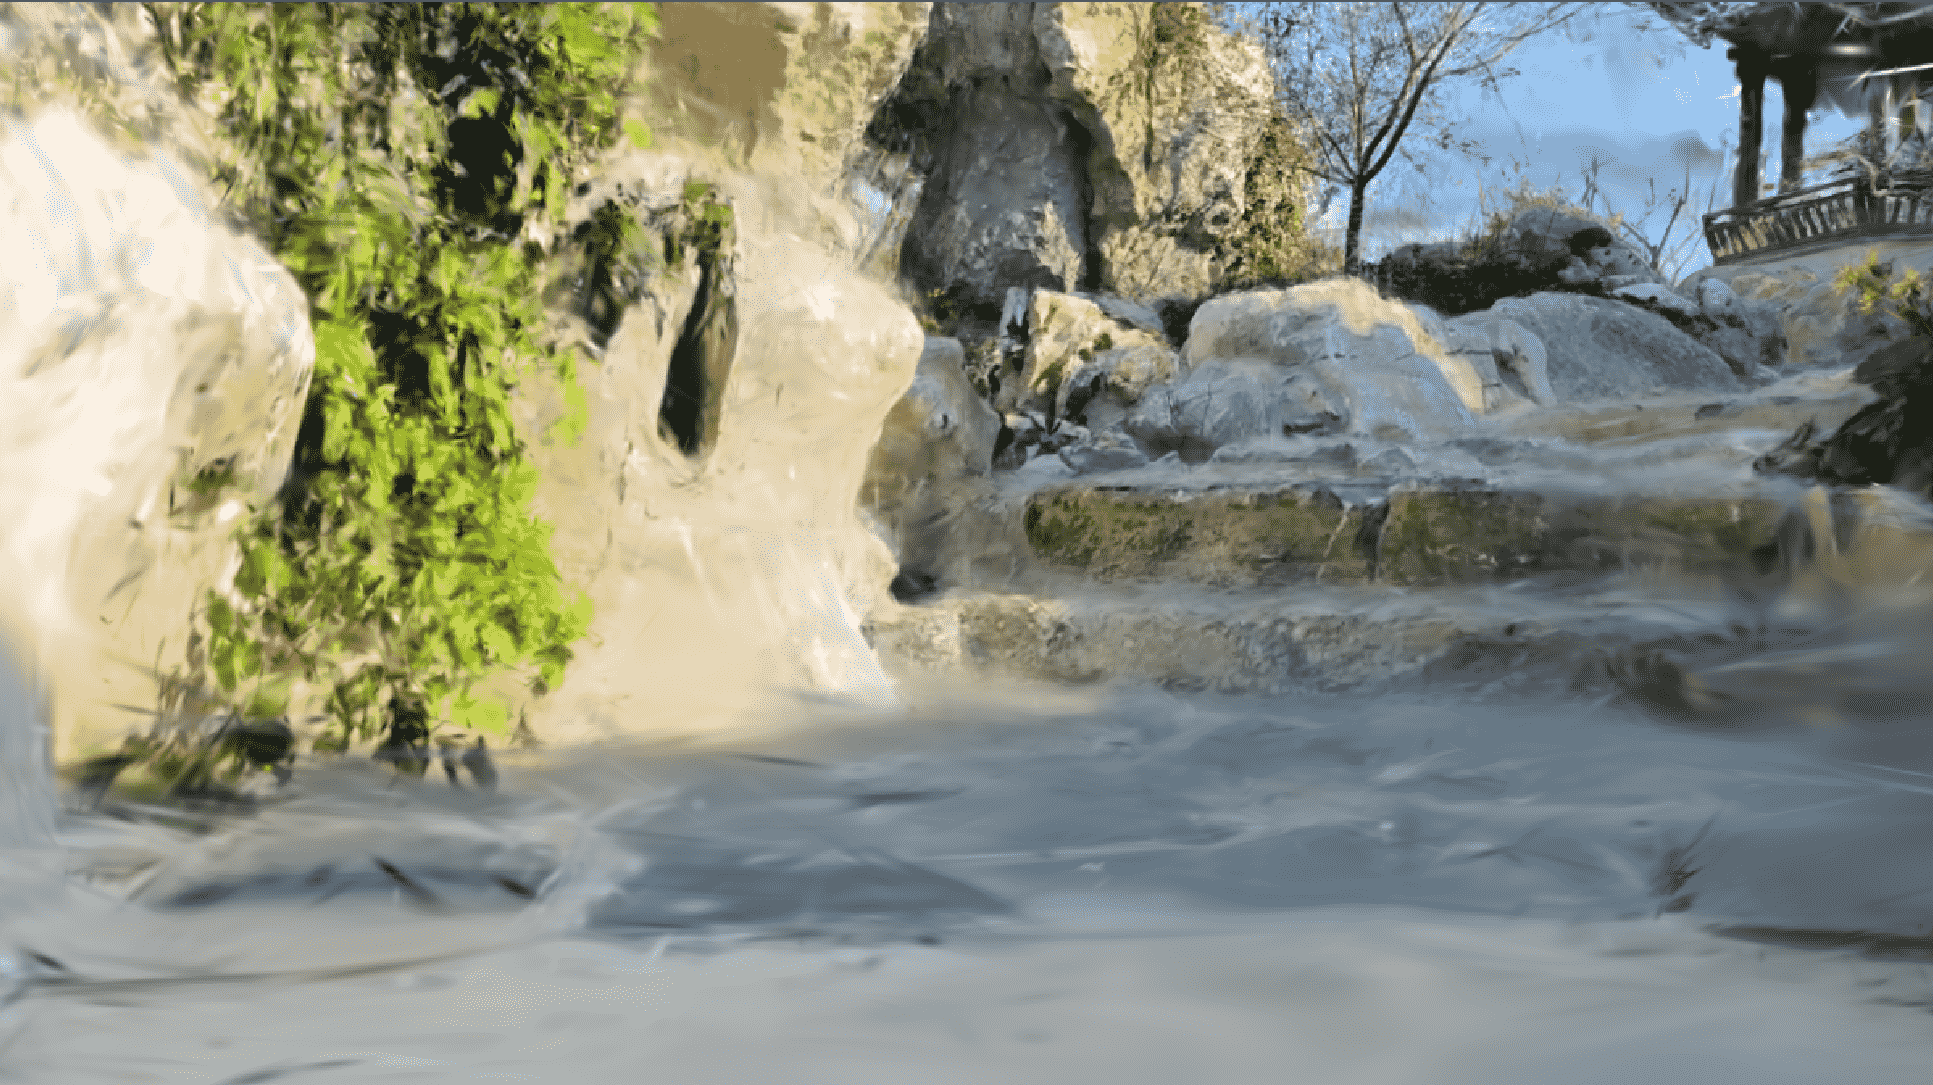} \\

        \includegraphics[width=0.24\linewidth]{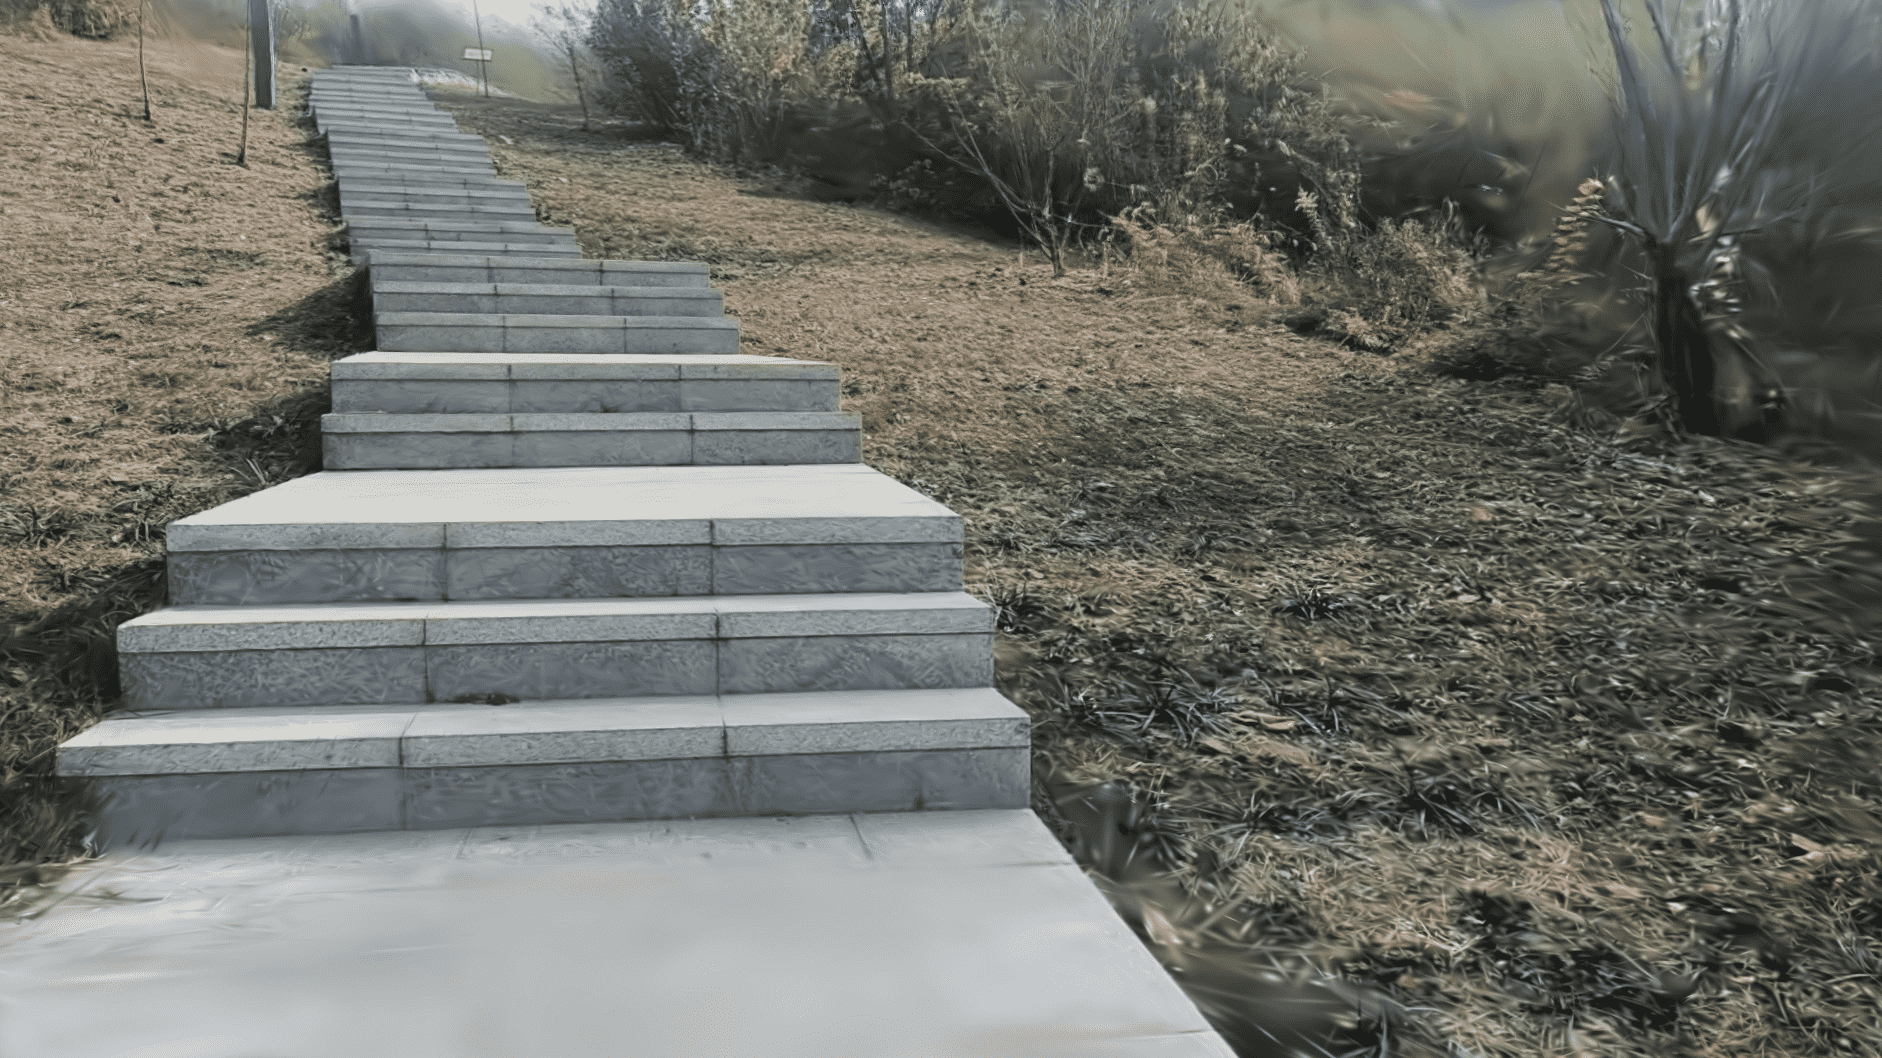} &
        \includegraphics[width=0.24\linewidth]{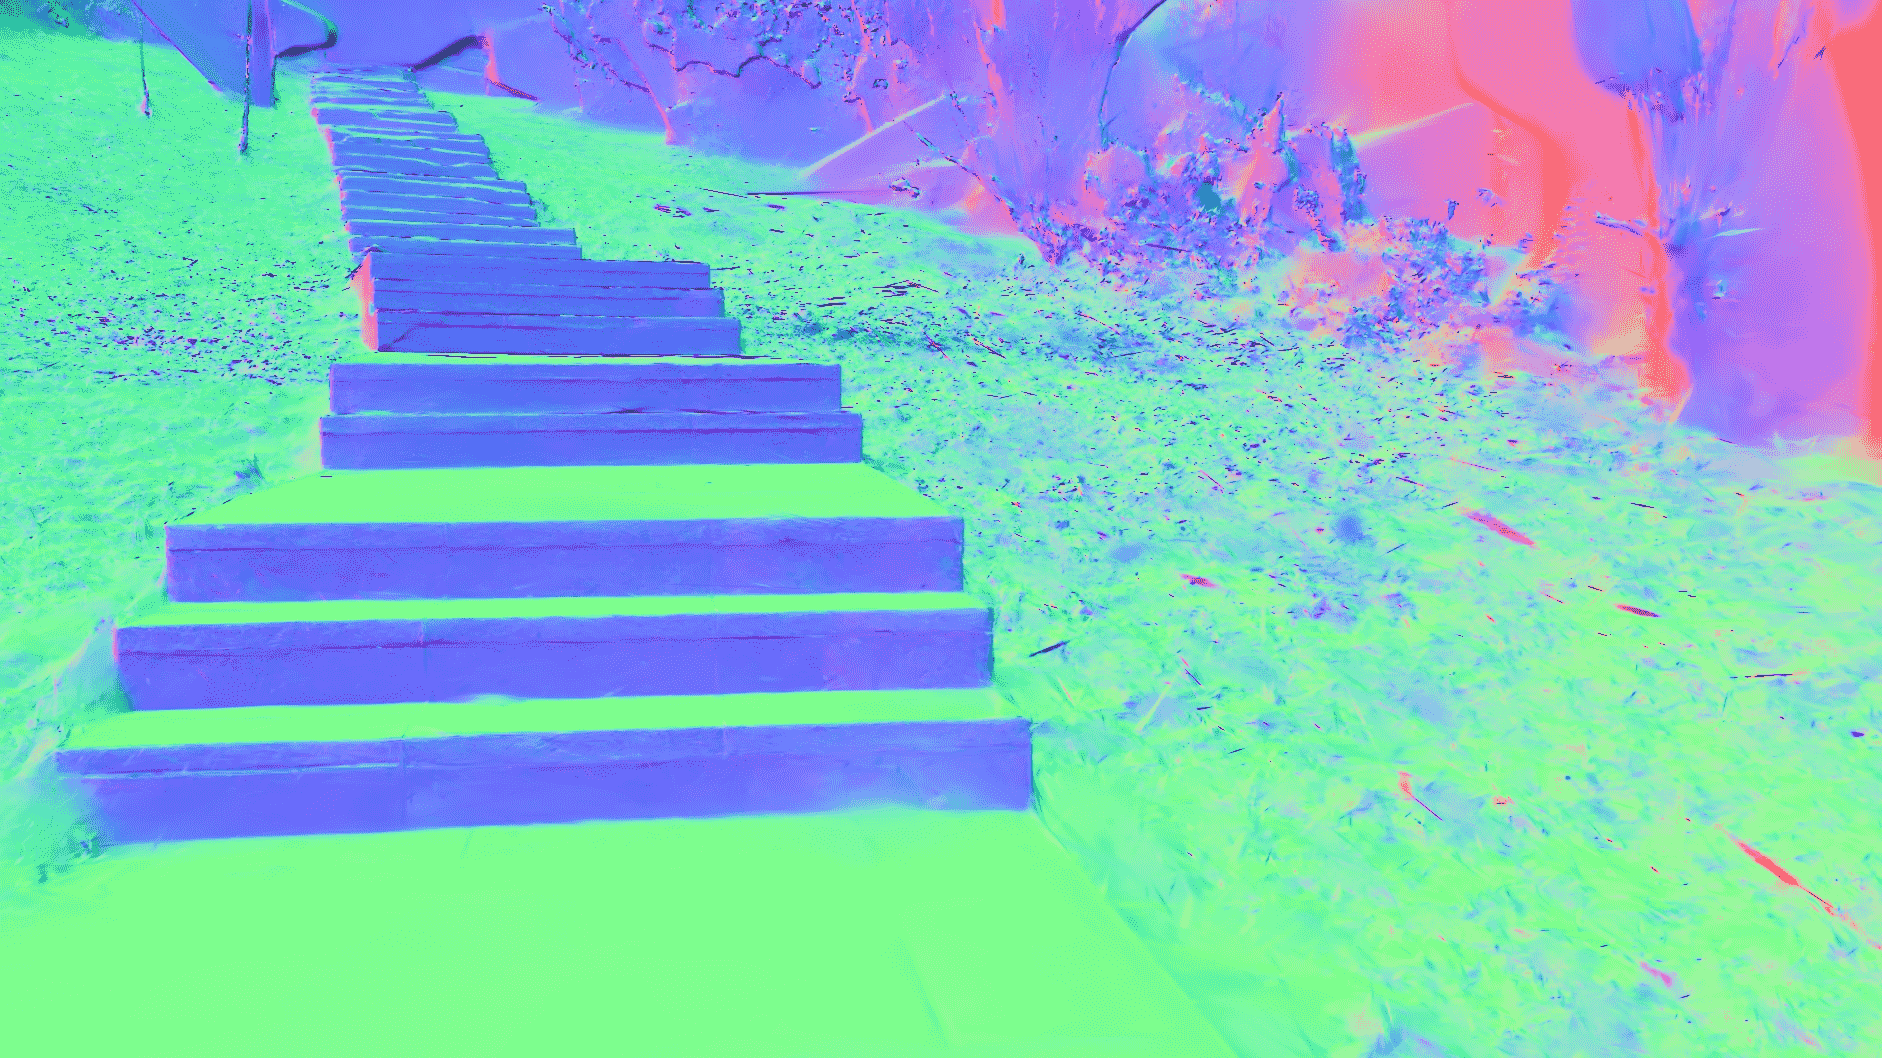} &
        \includegraphics[width=0.24\linewidth]{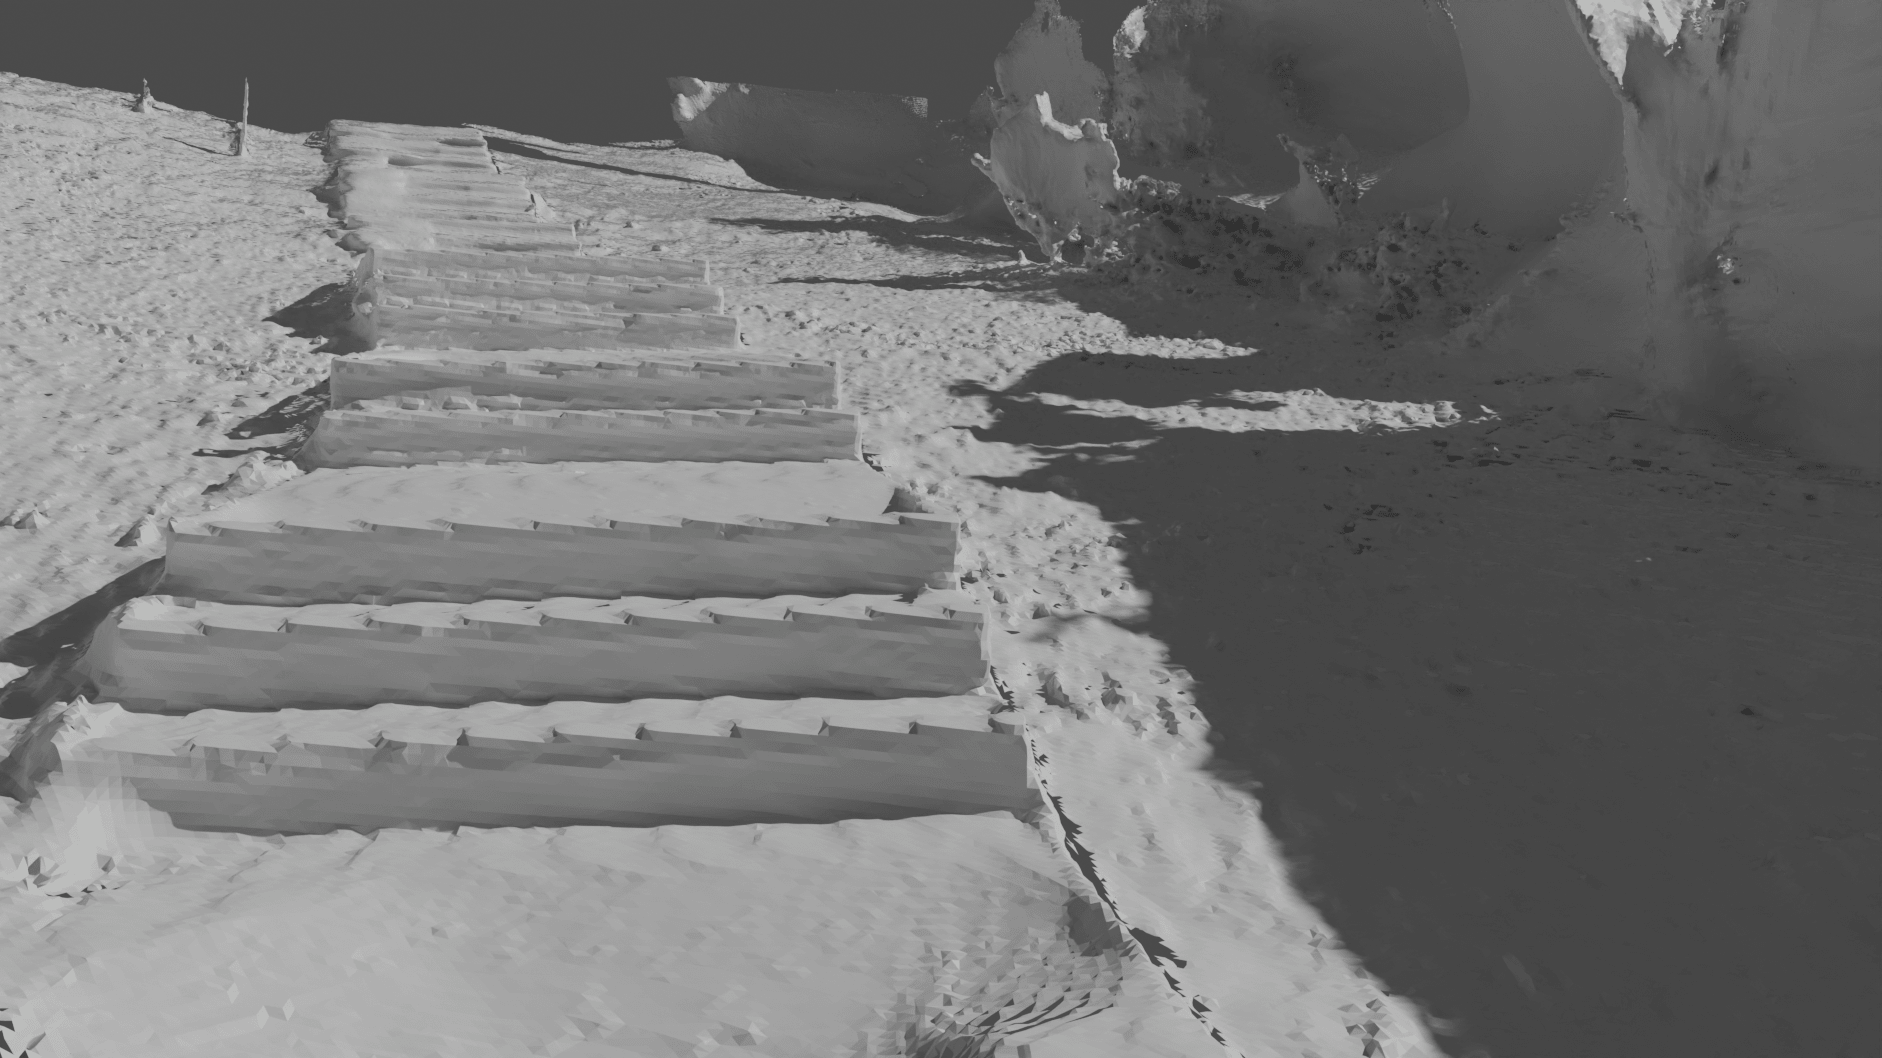} &
        \includegraphics[width=0.24\linewidth]{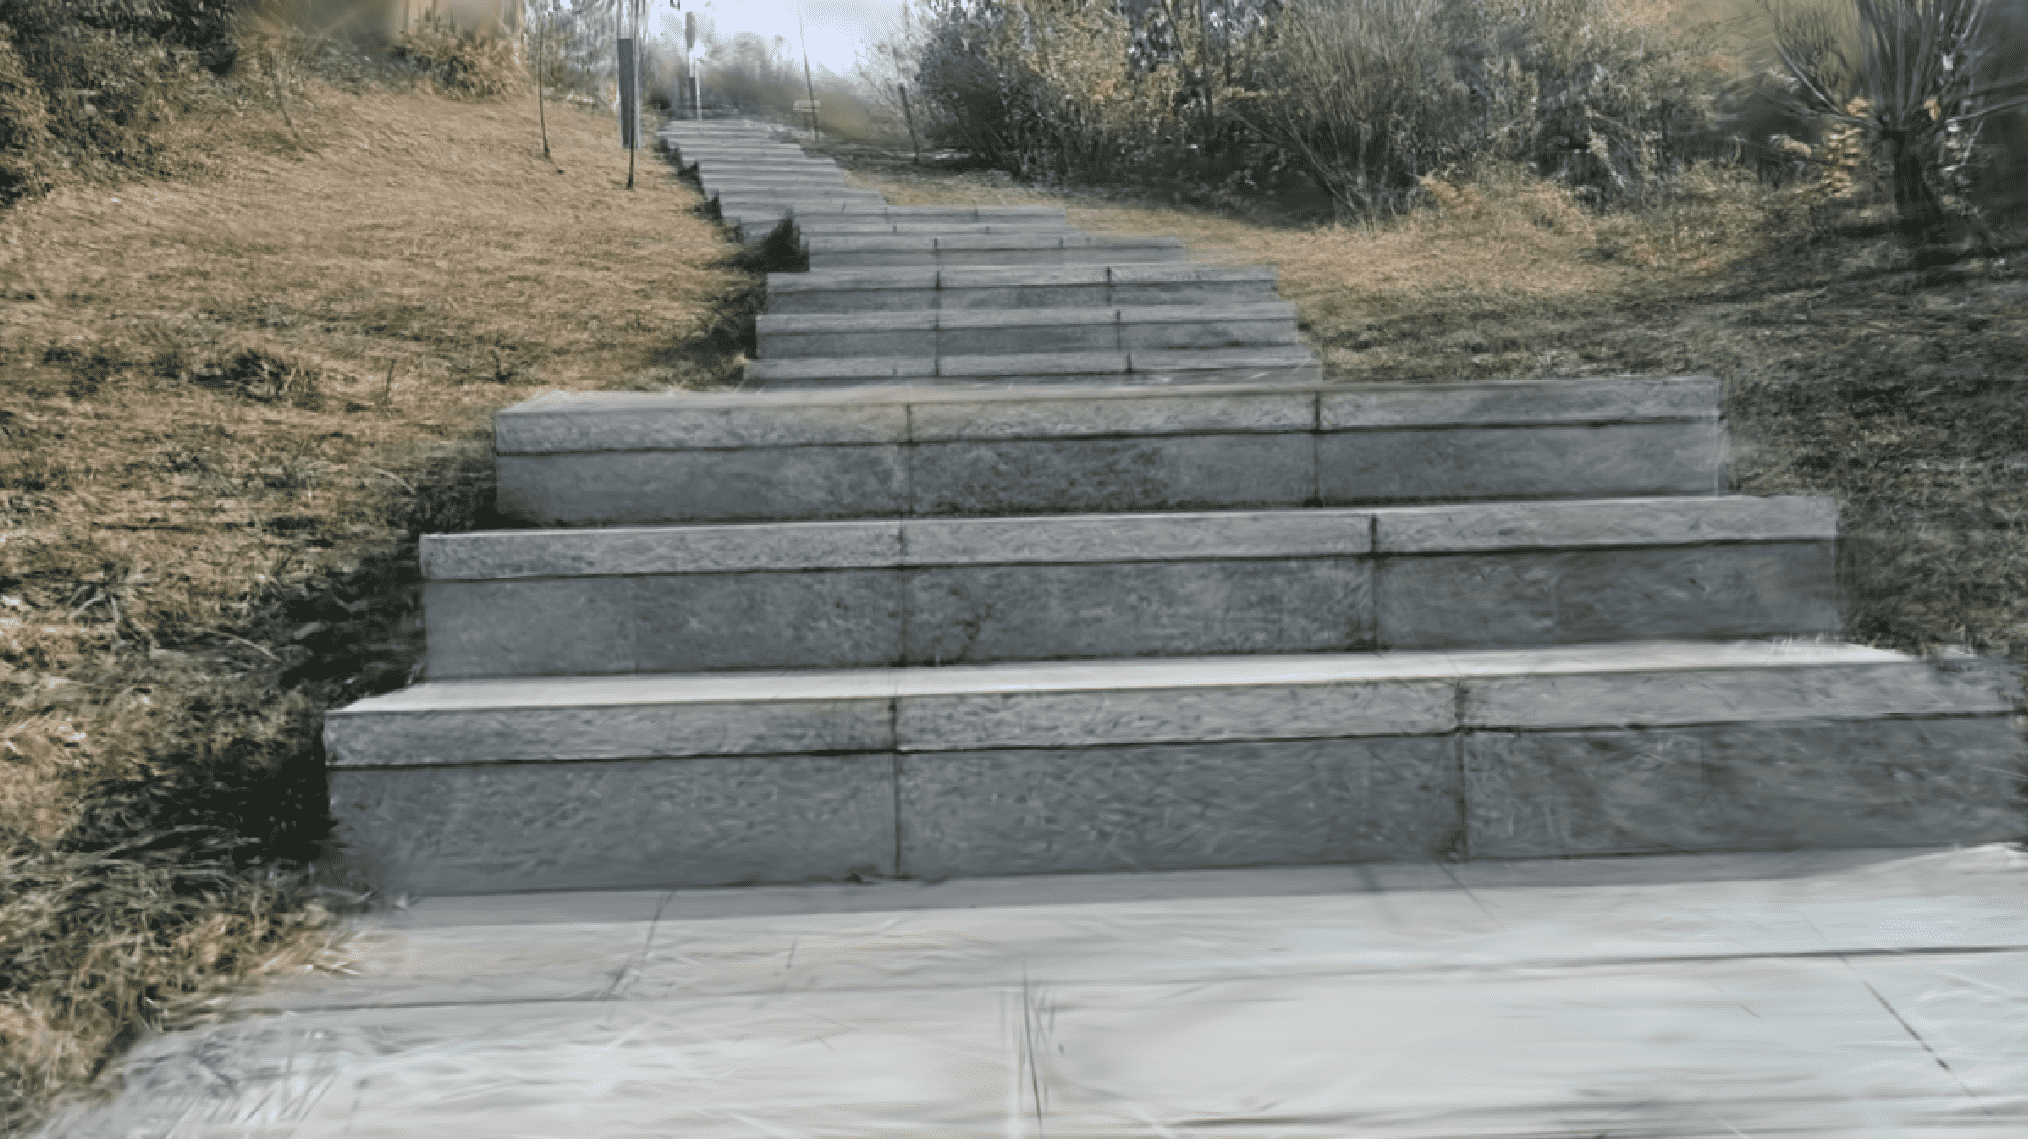} \\

        \includegraphics[width=0.24\linewidth]{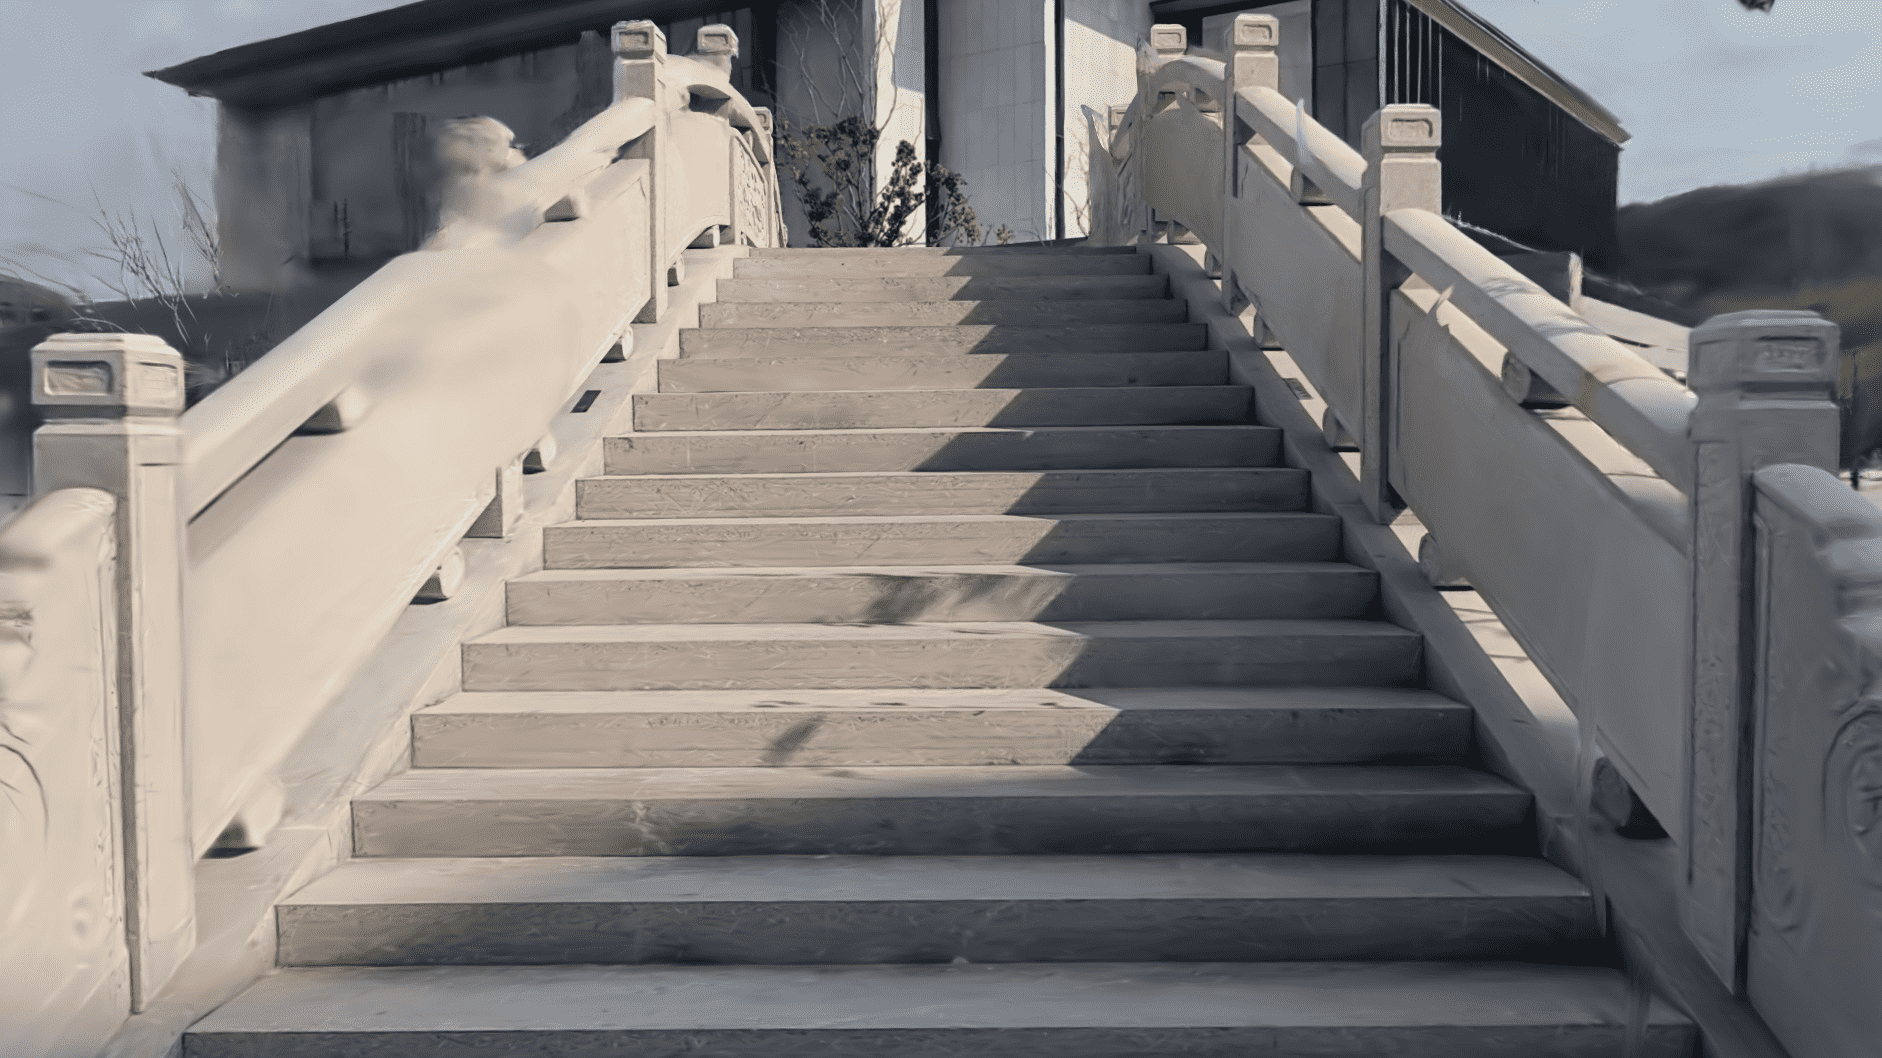} &
        \includegraphics[width=0.24\linewidth]{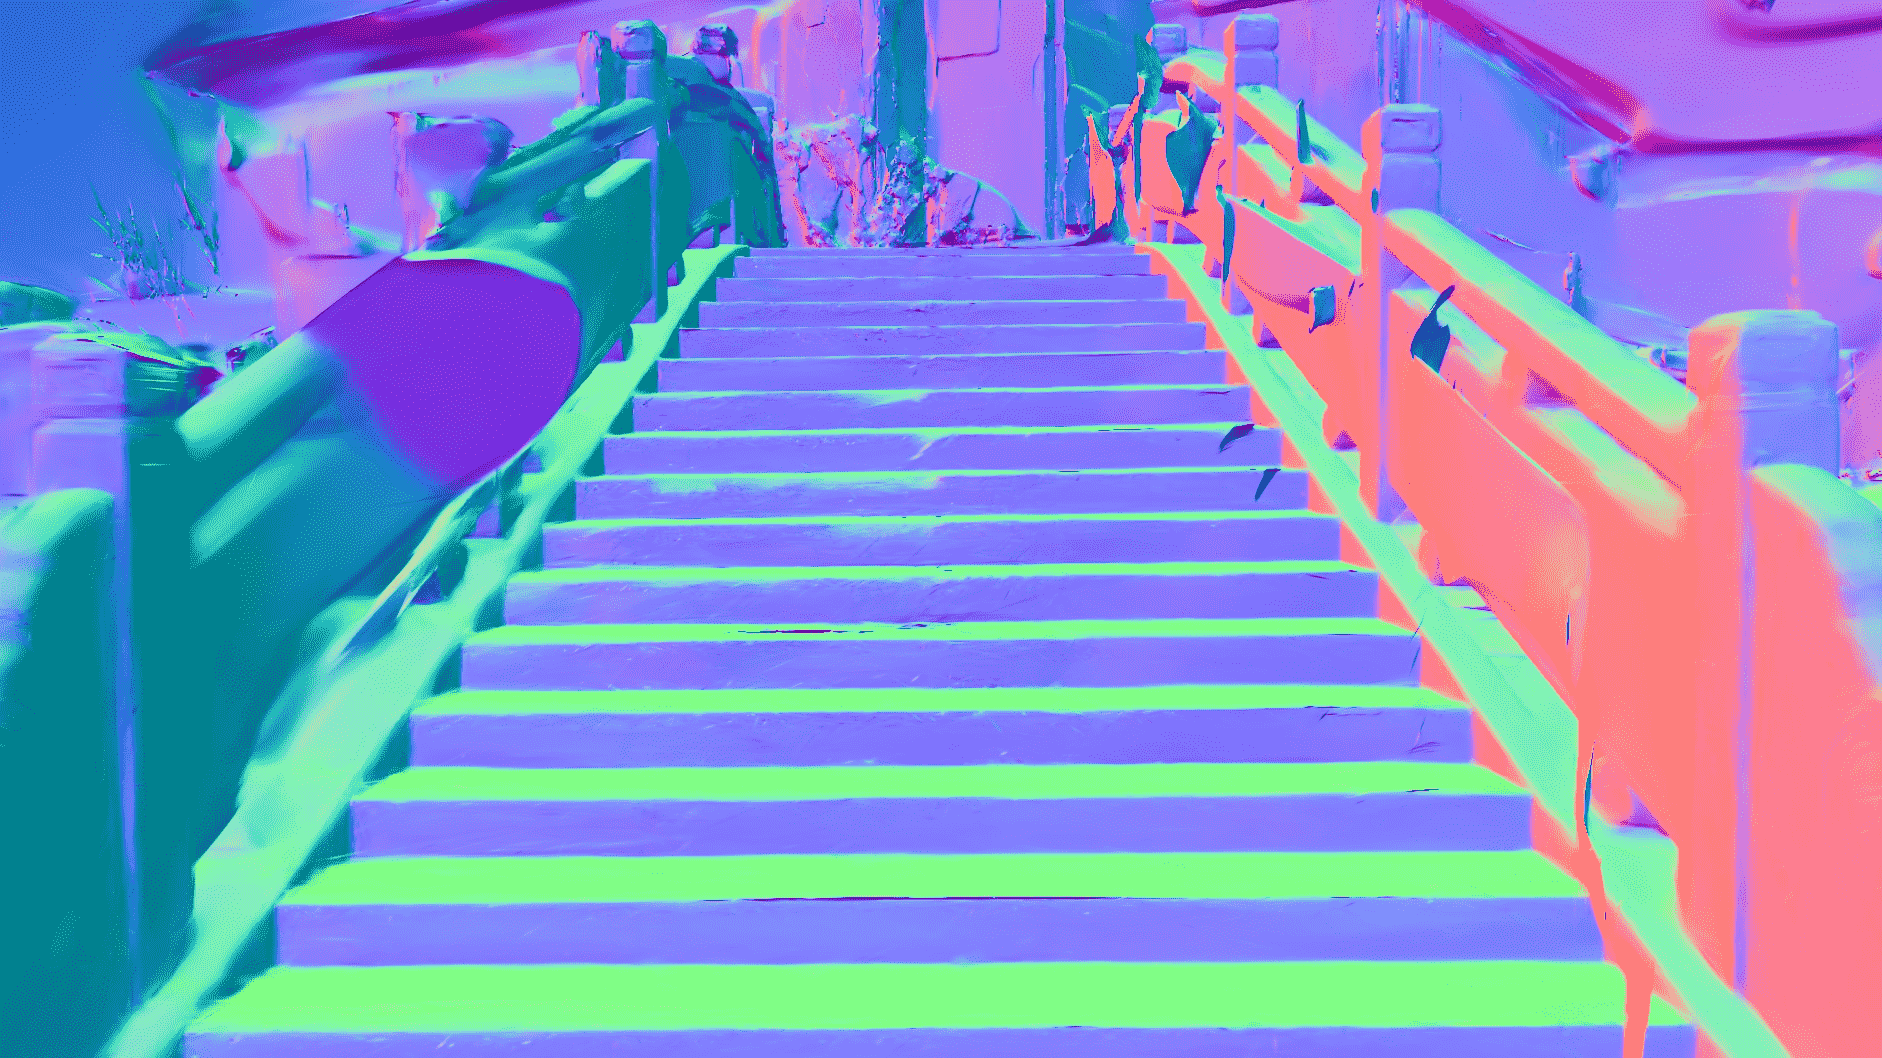} &
        \includegraphics[width=0.24\linewidth]{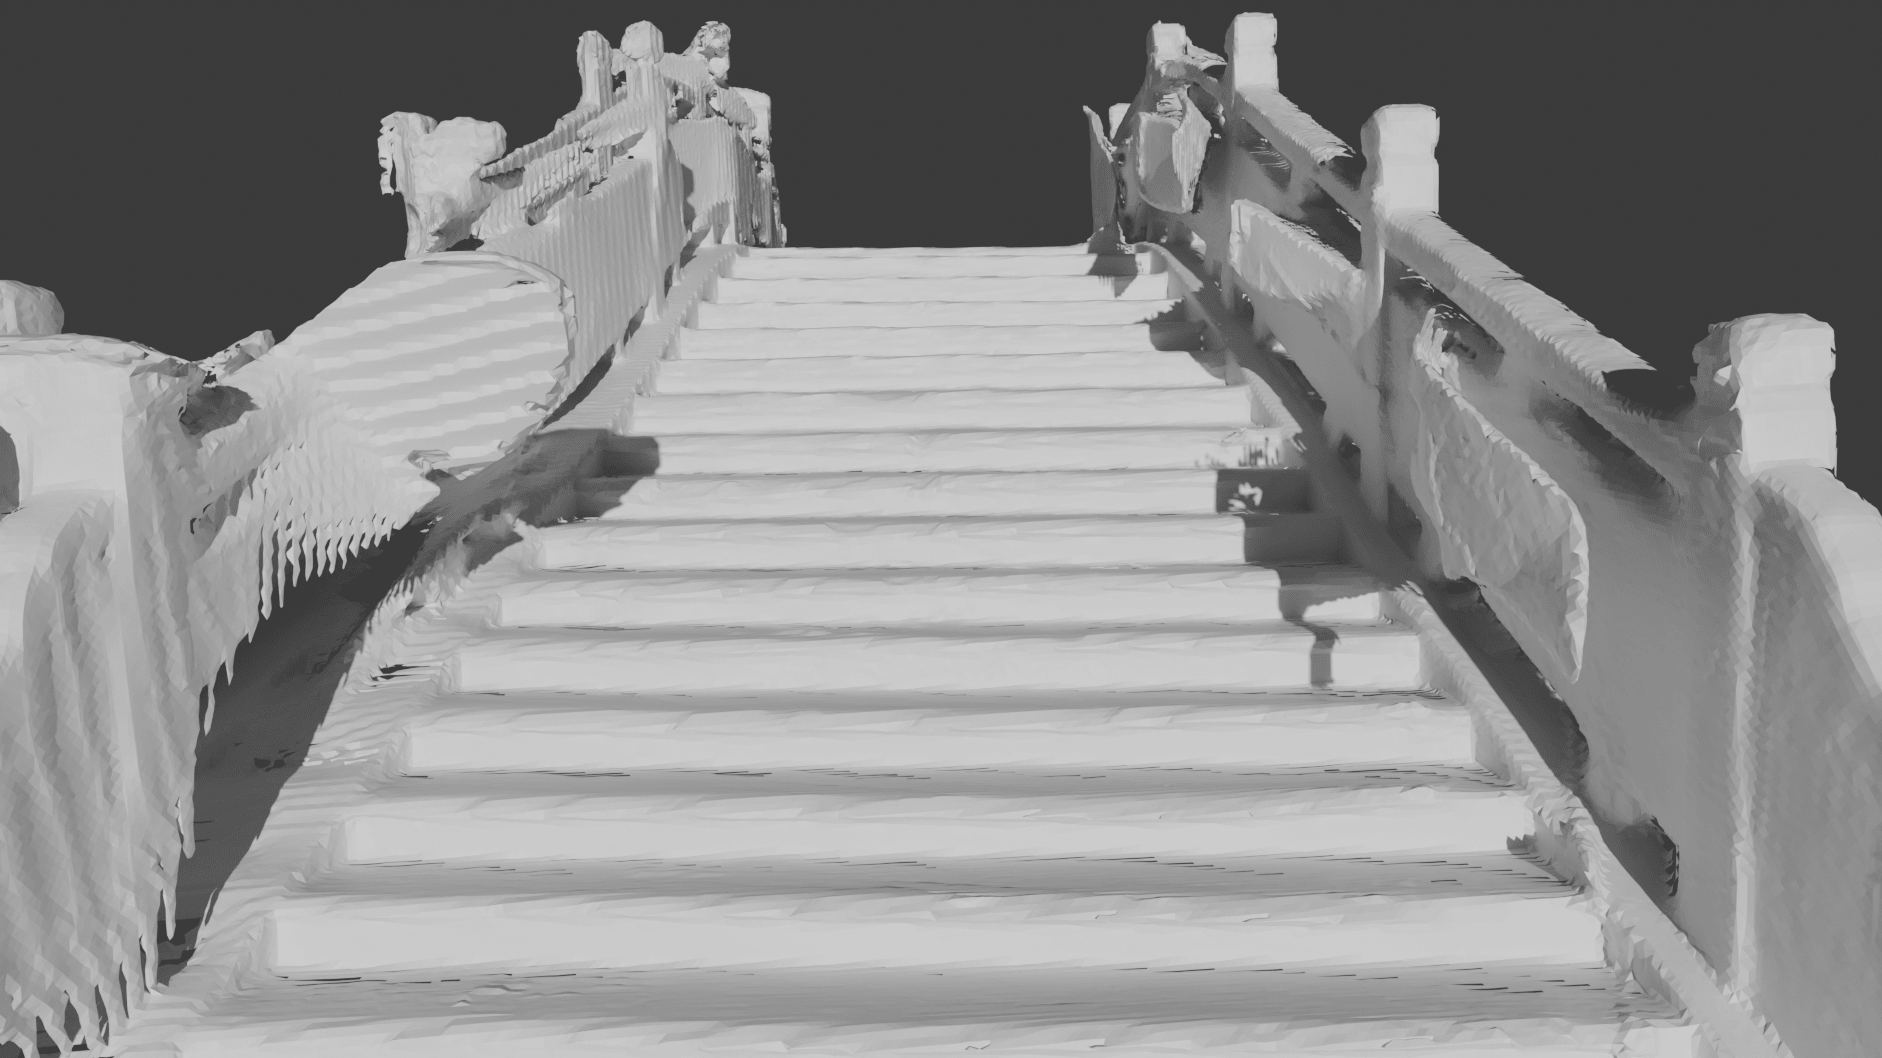} &
        \includegraphics[width=0.24\linewidth]{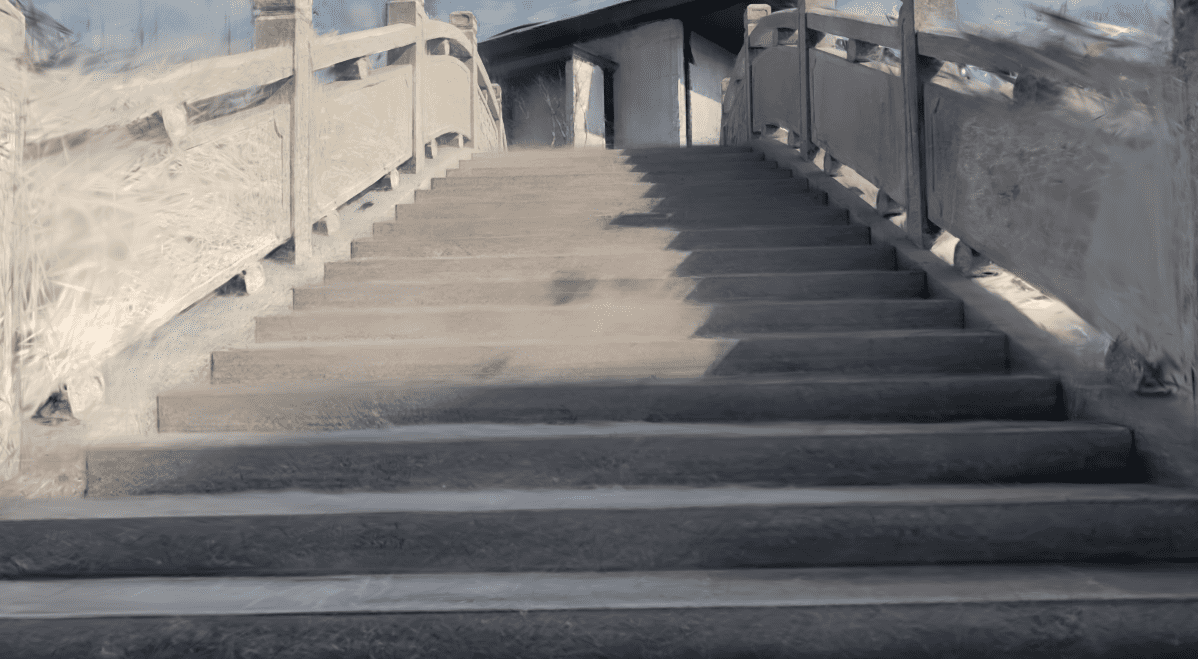} \\

        \includegraphics[width=0.24\linewidth]{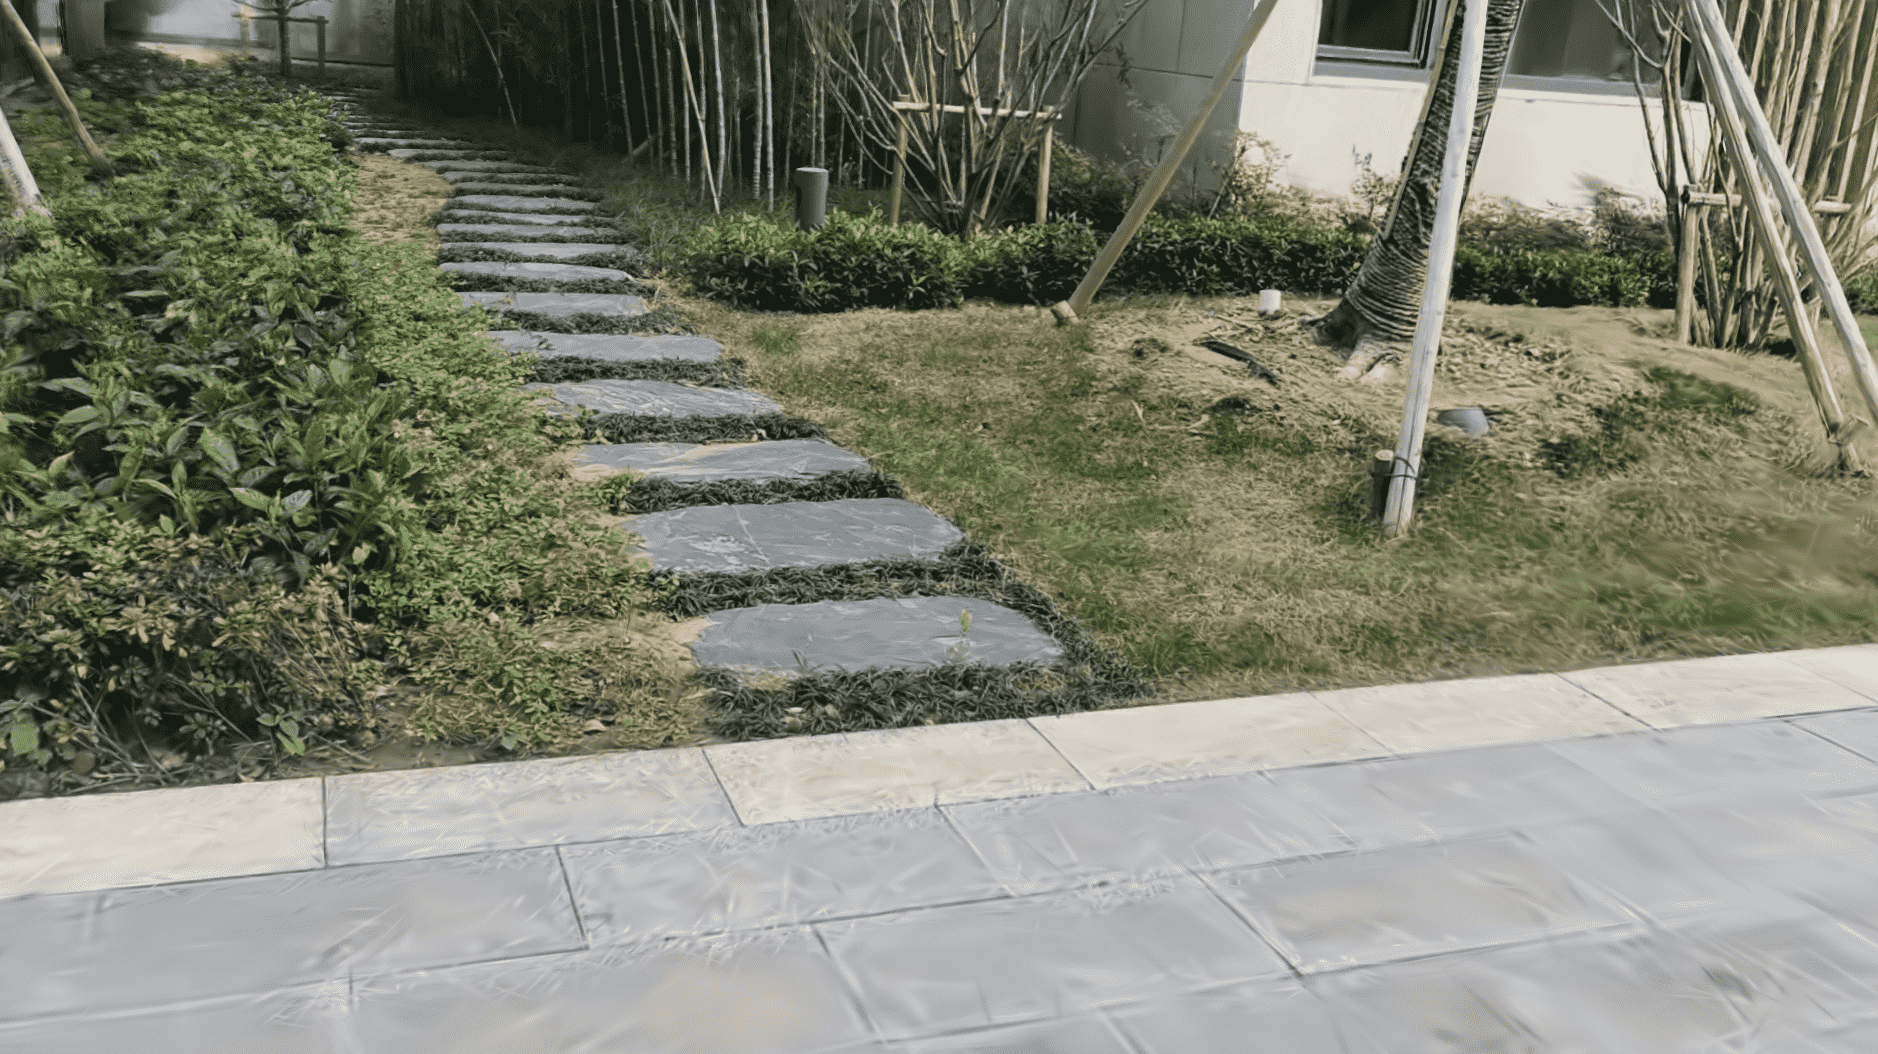} &
        \includegraphics[width=0.24\linewidth]{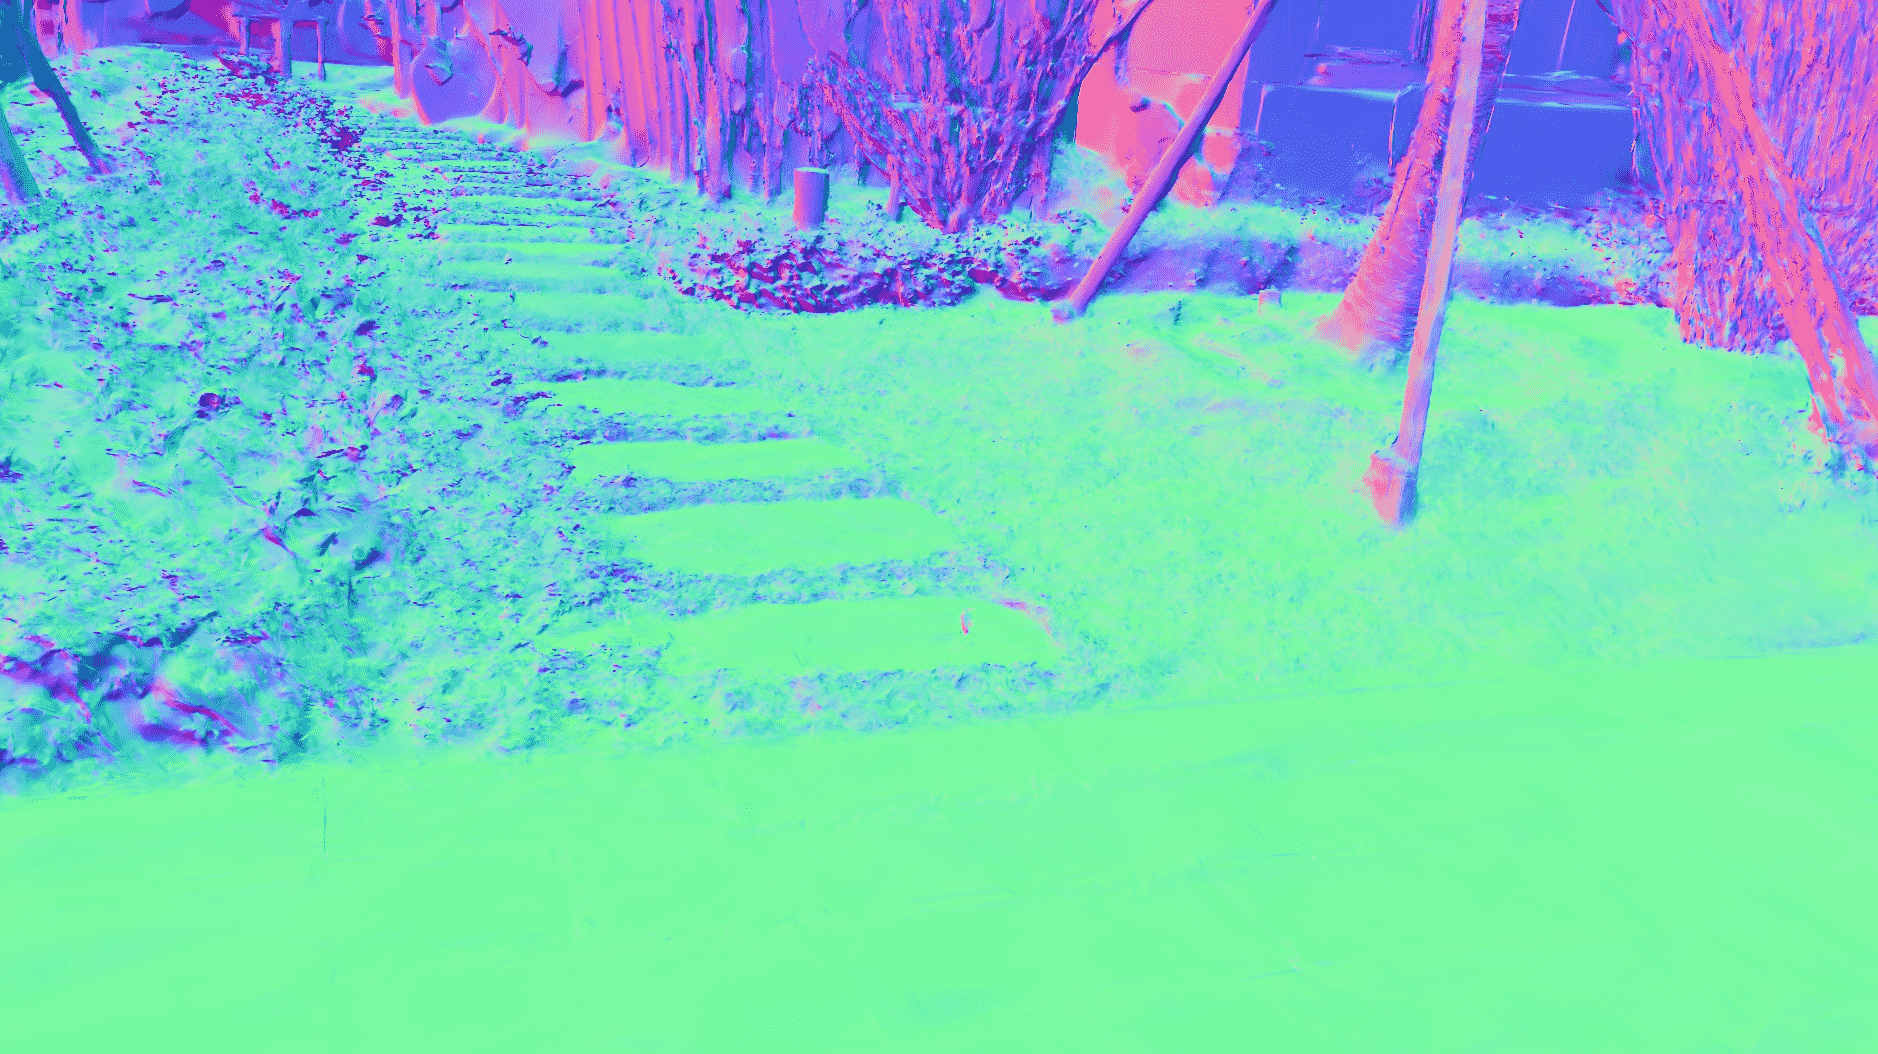} &
        \includegraphics[width=0.24\linewidth]{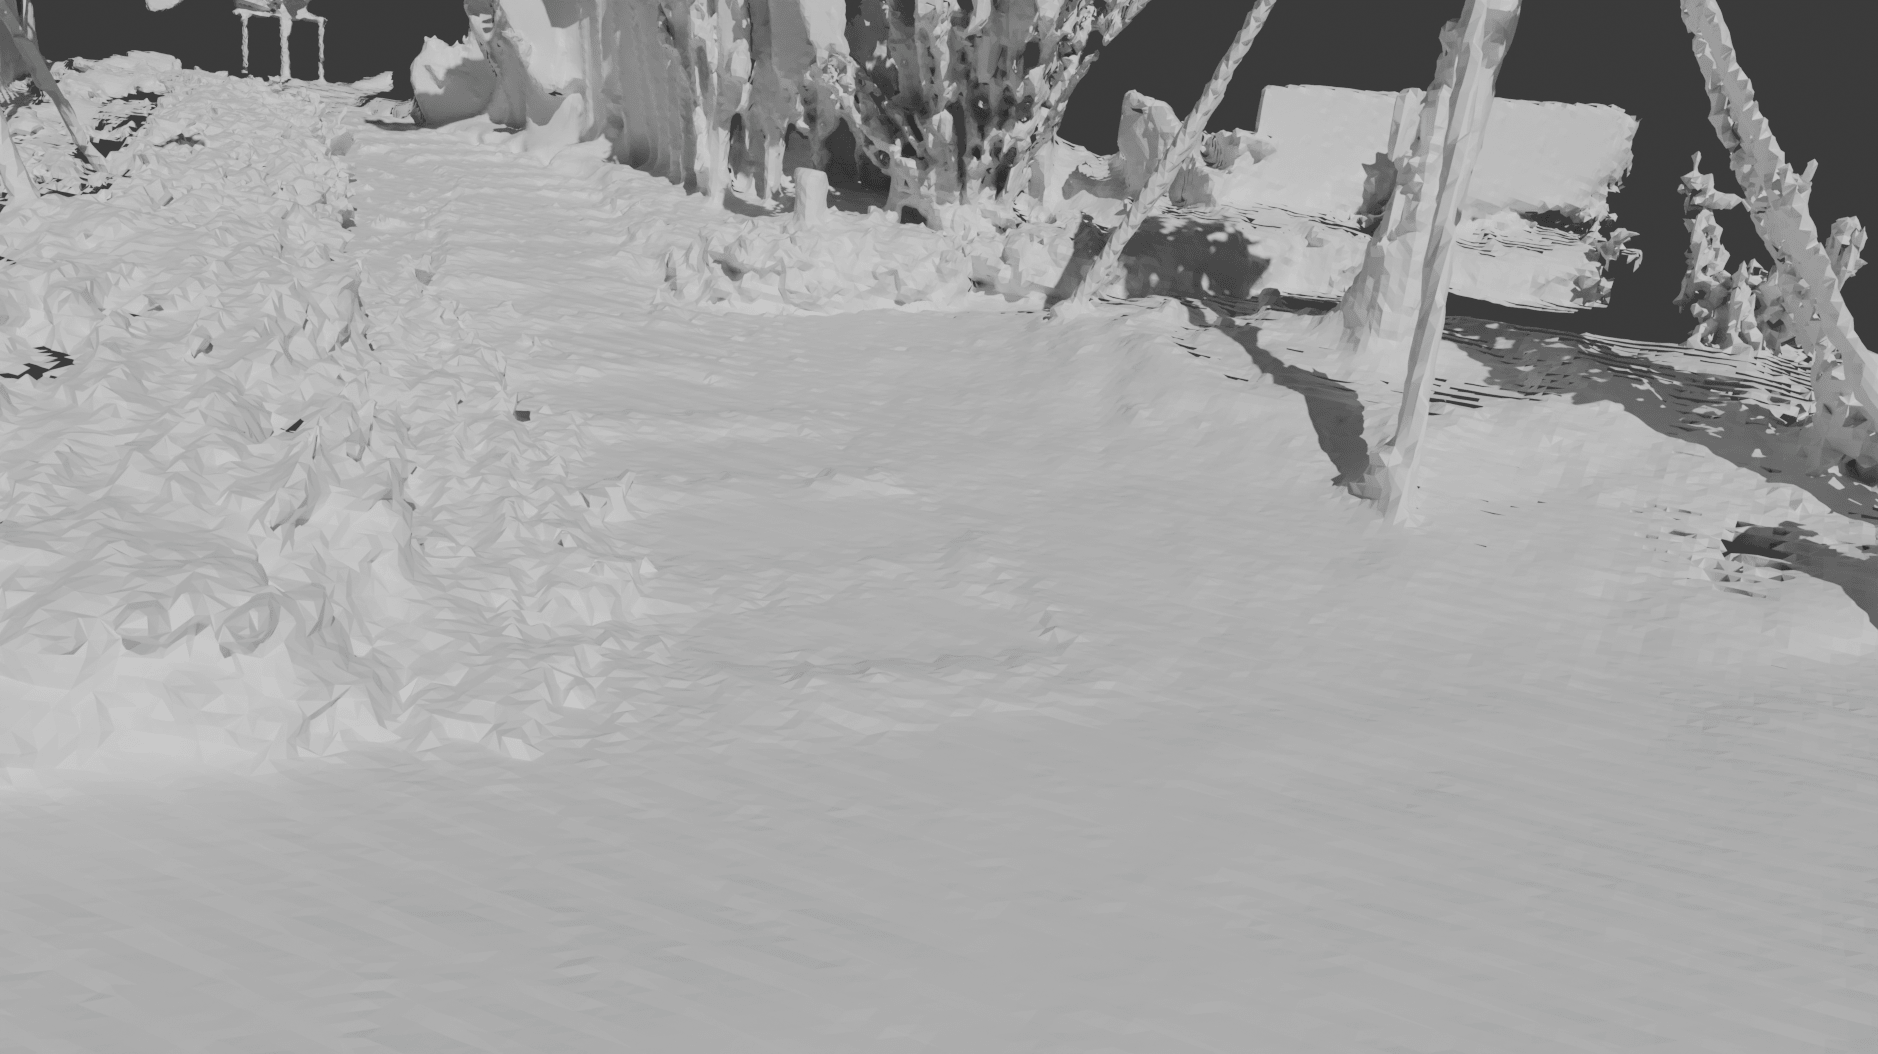} &
        \includegraphics[width=0.24\linewidth]{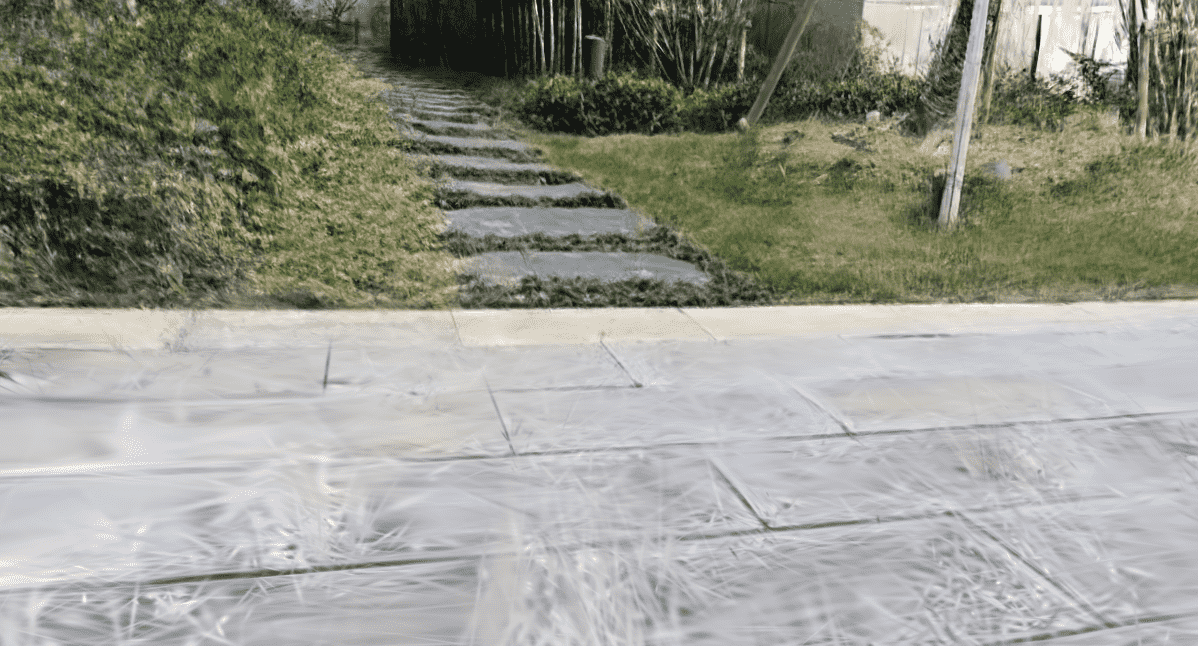} \\

        \includegraphics[width=0.24\linewidth]{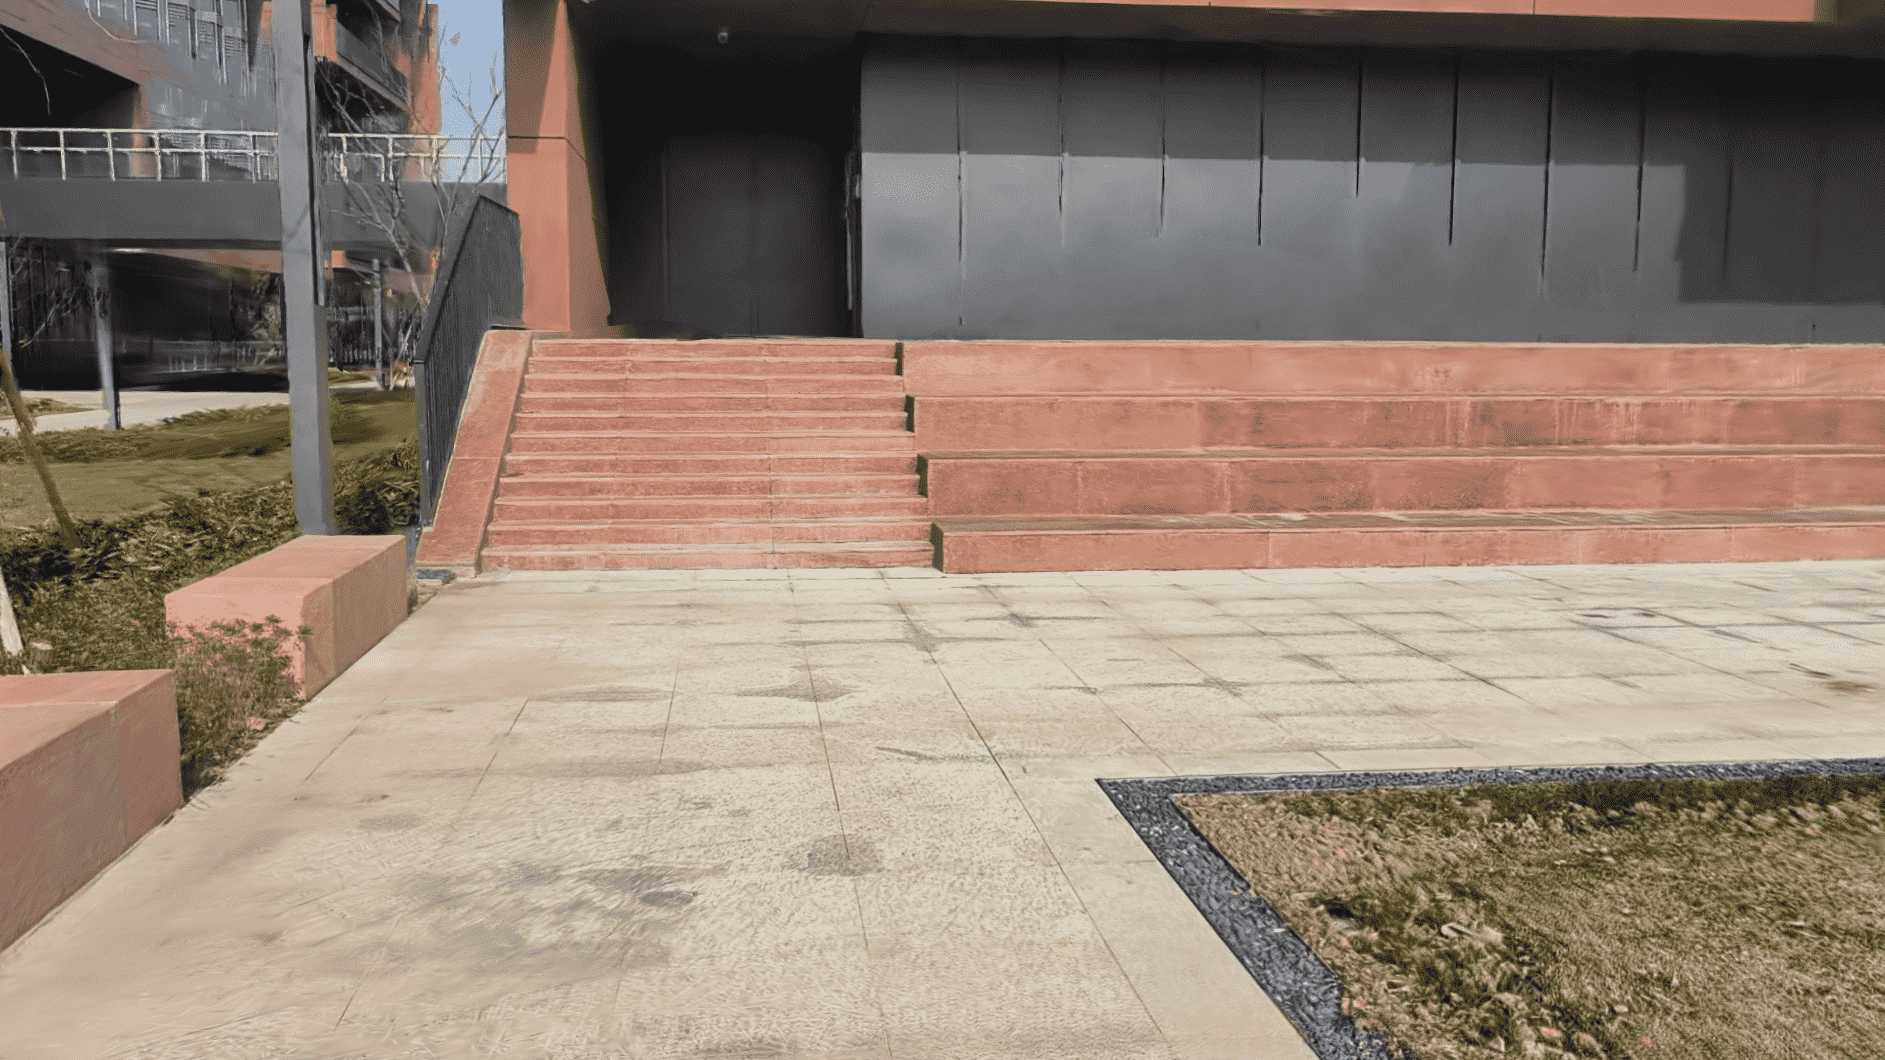} &
        \includegraphics[width=0.24\linewidth]{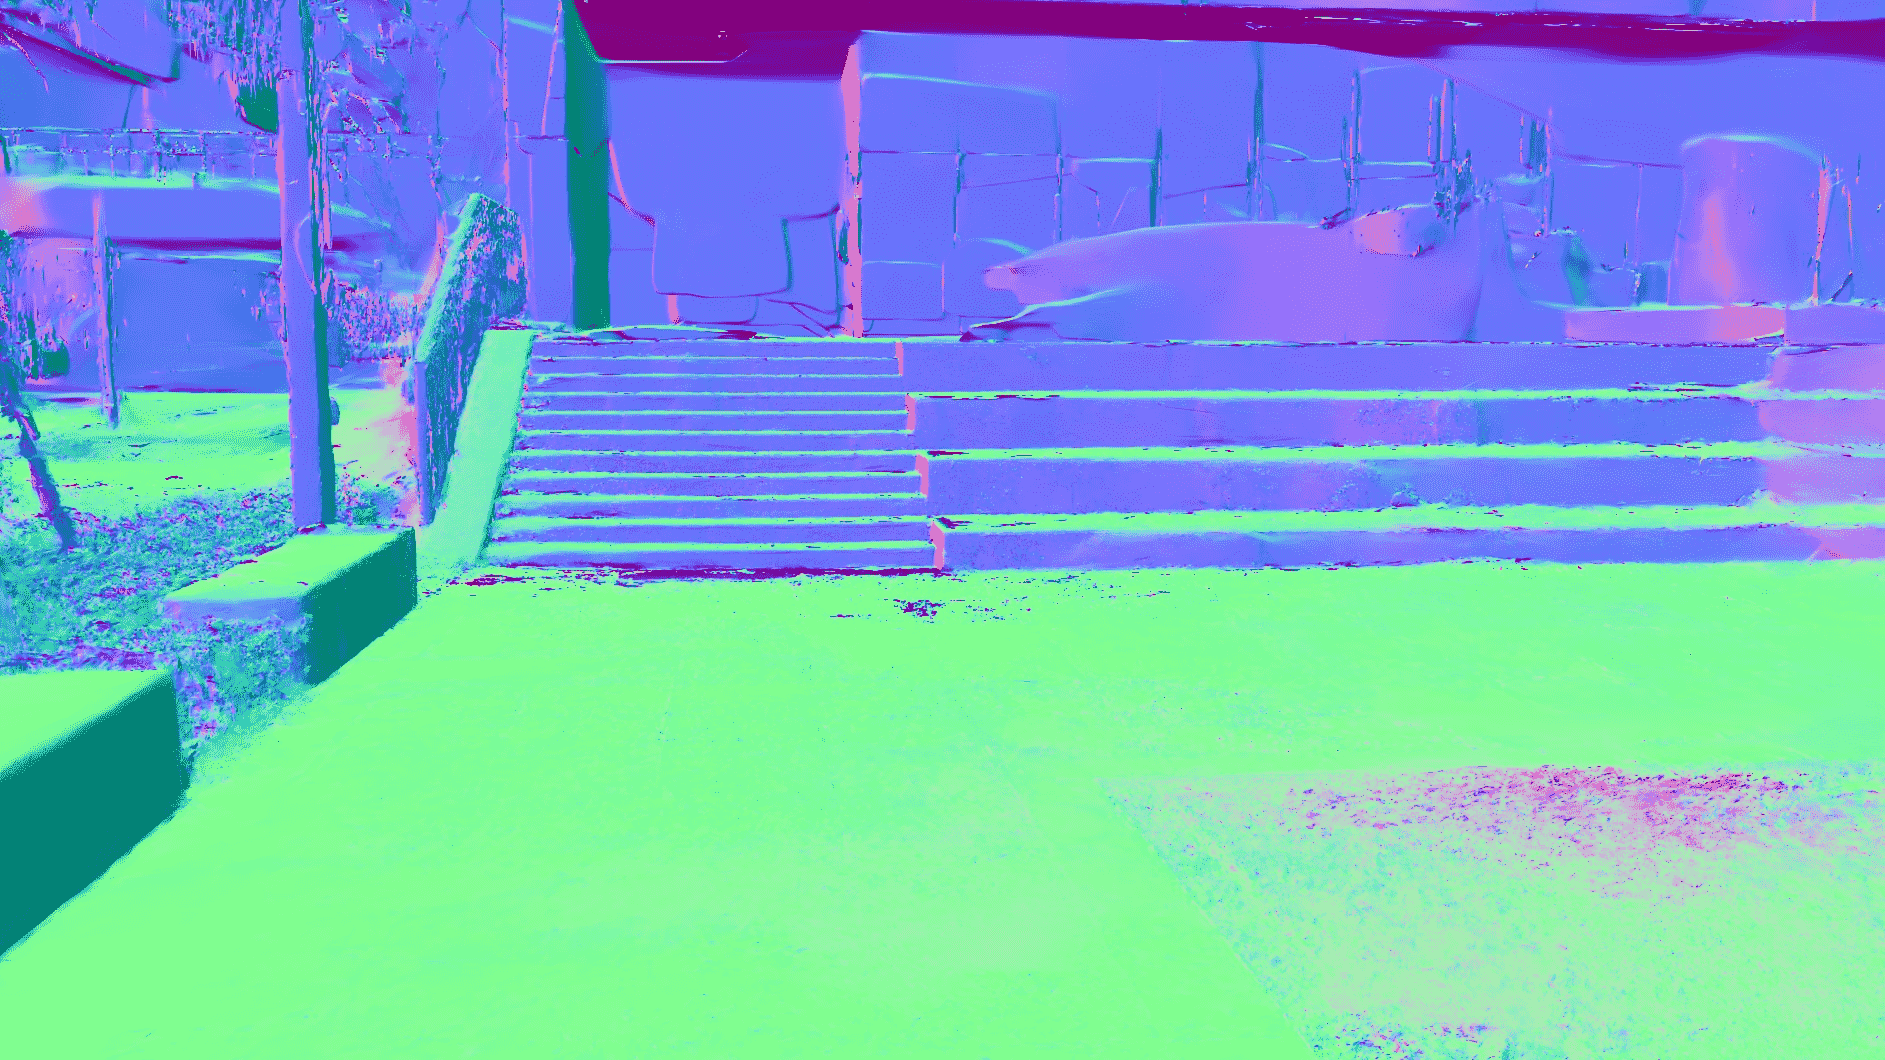} &
        \includegraphics[width=0.24\linewidth]{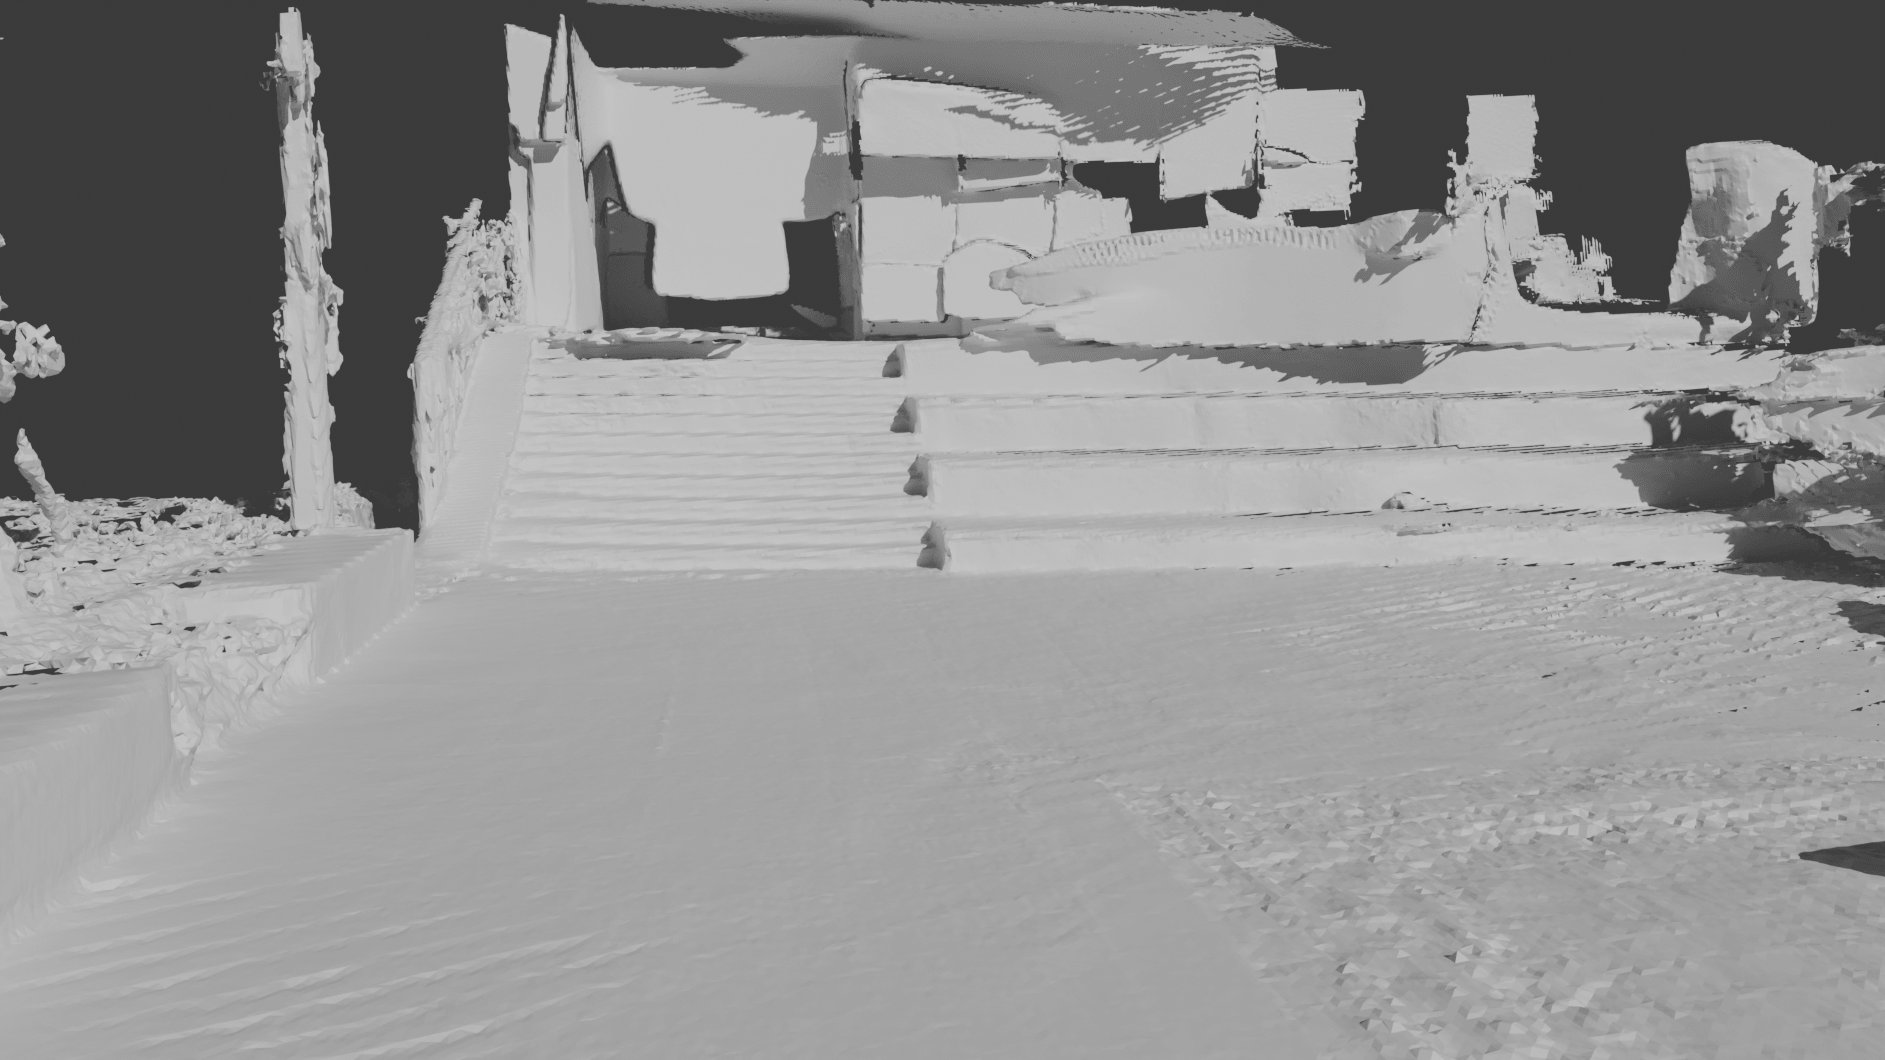} &
        \includegraphics[width=0.24\linewidth]{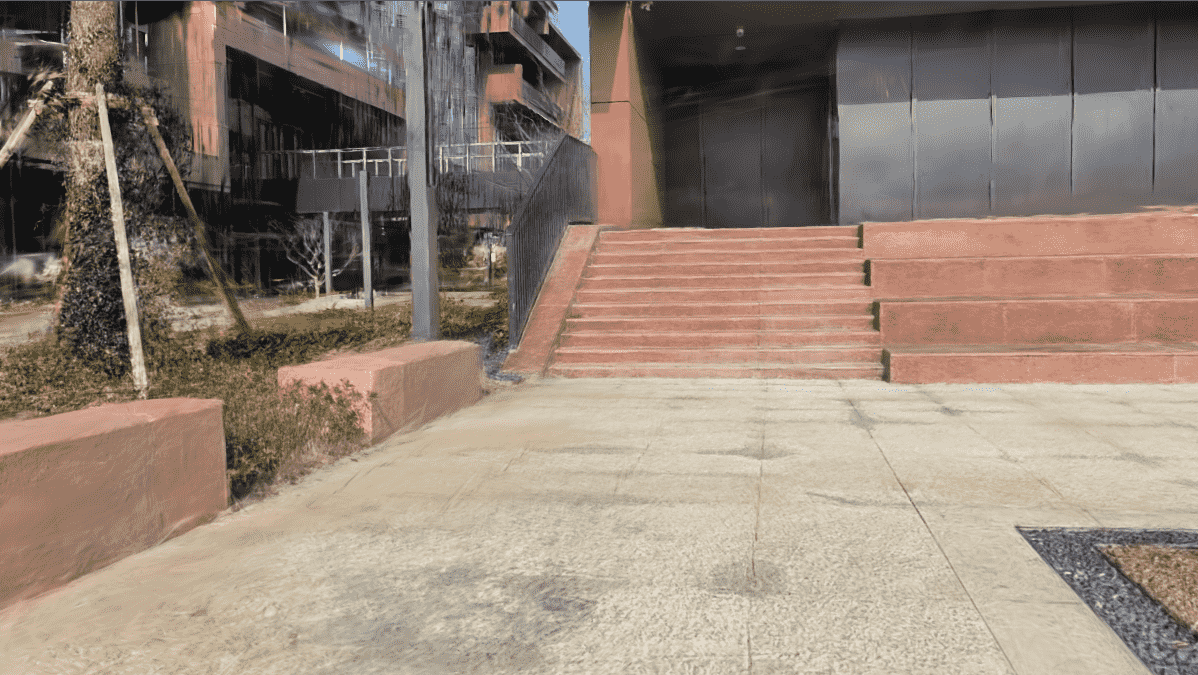} \\

        \includegraphics[width=0.24\linewidth]{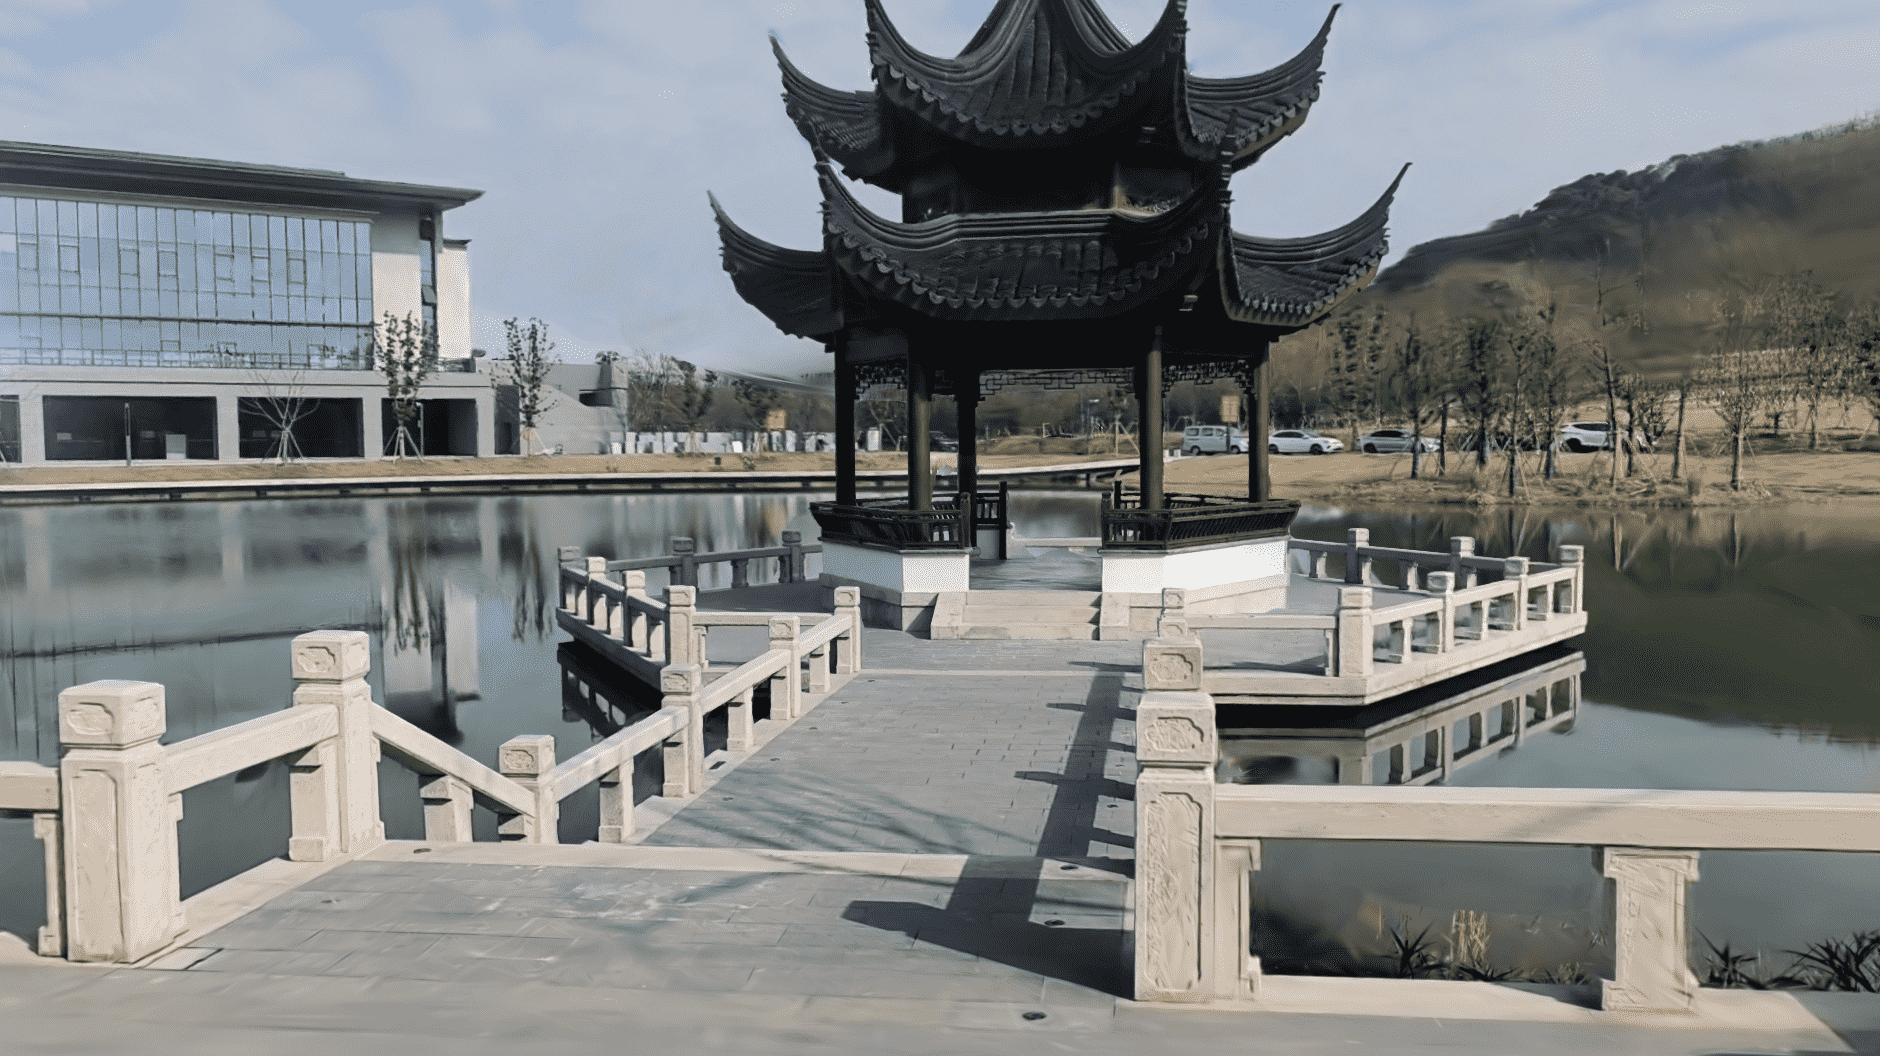} &
        \includegraphics[width=0.24\linewidth]{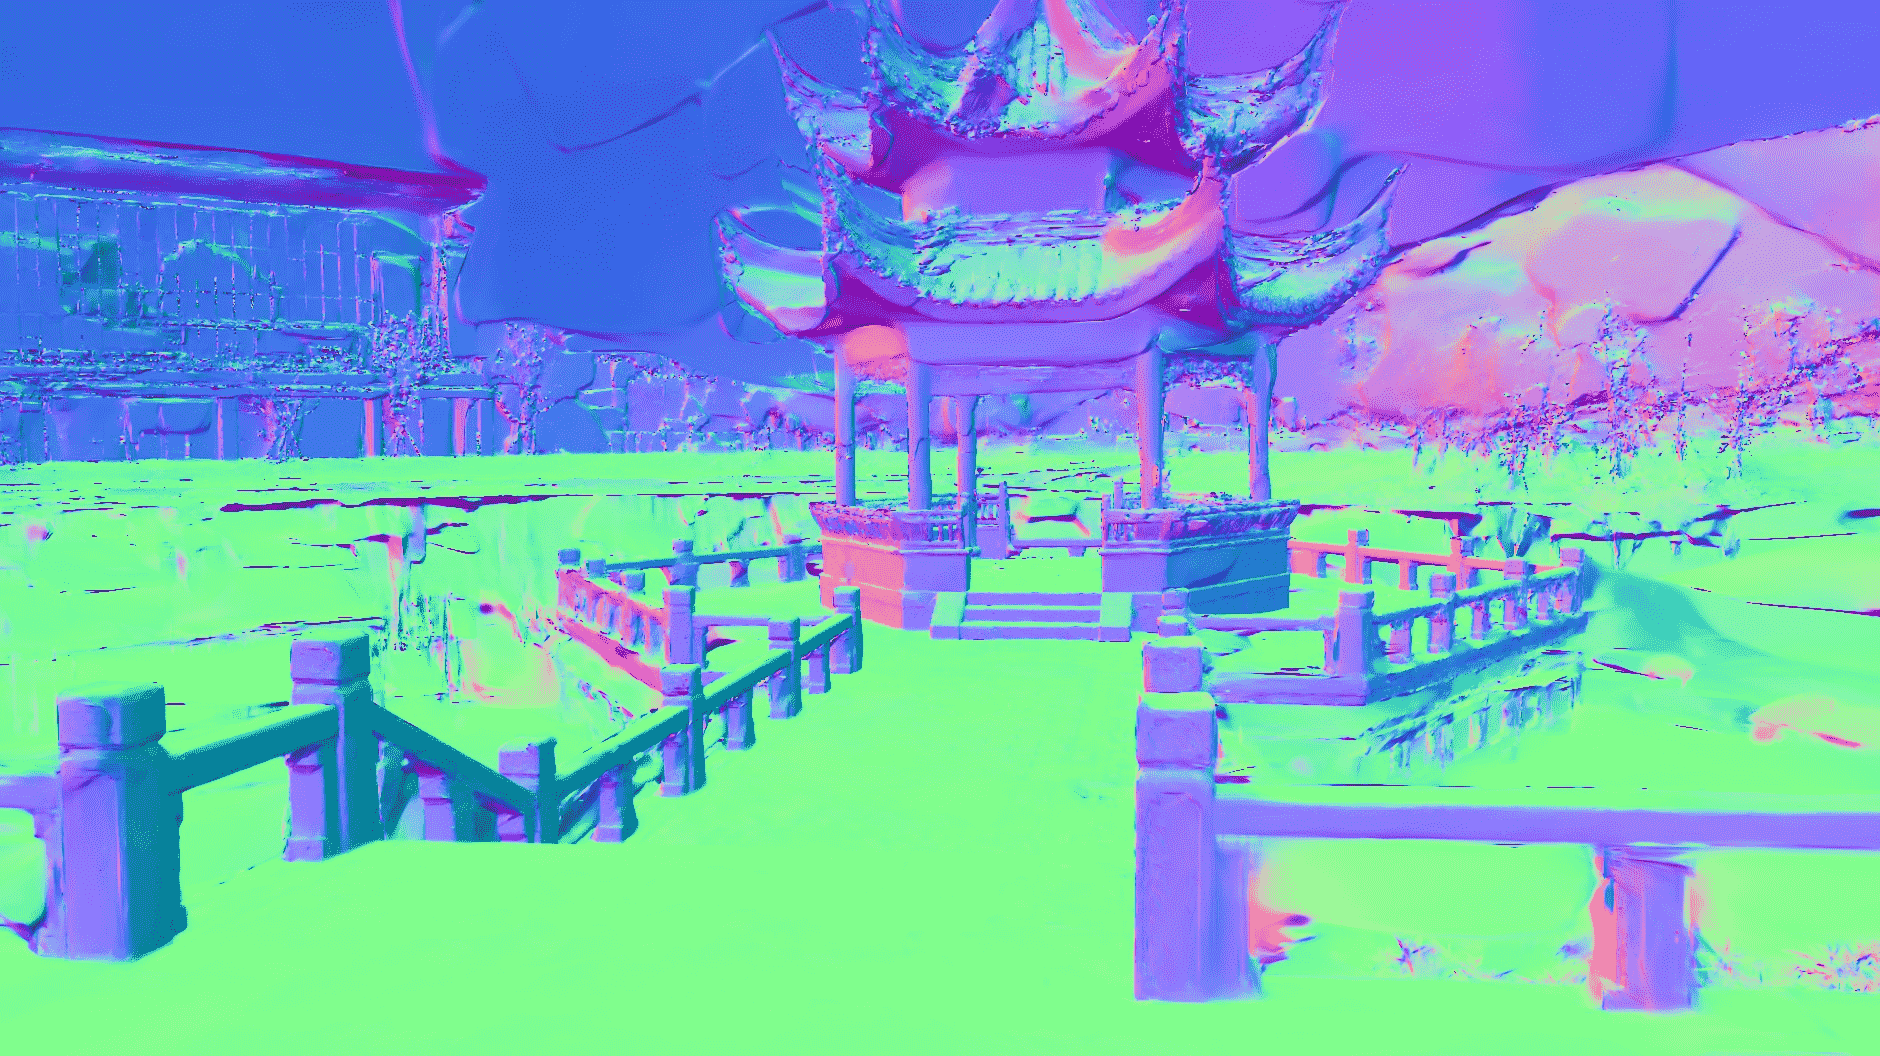} &
        \includegraphics[width=0.24\linewidth]{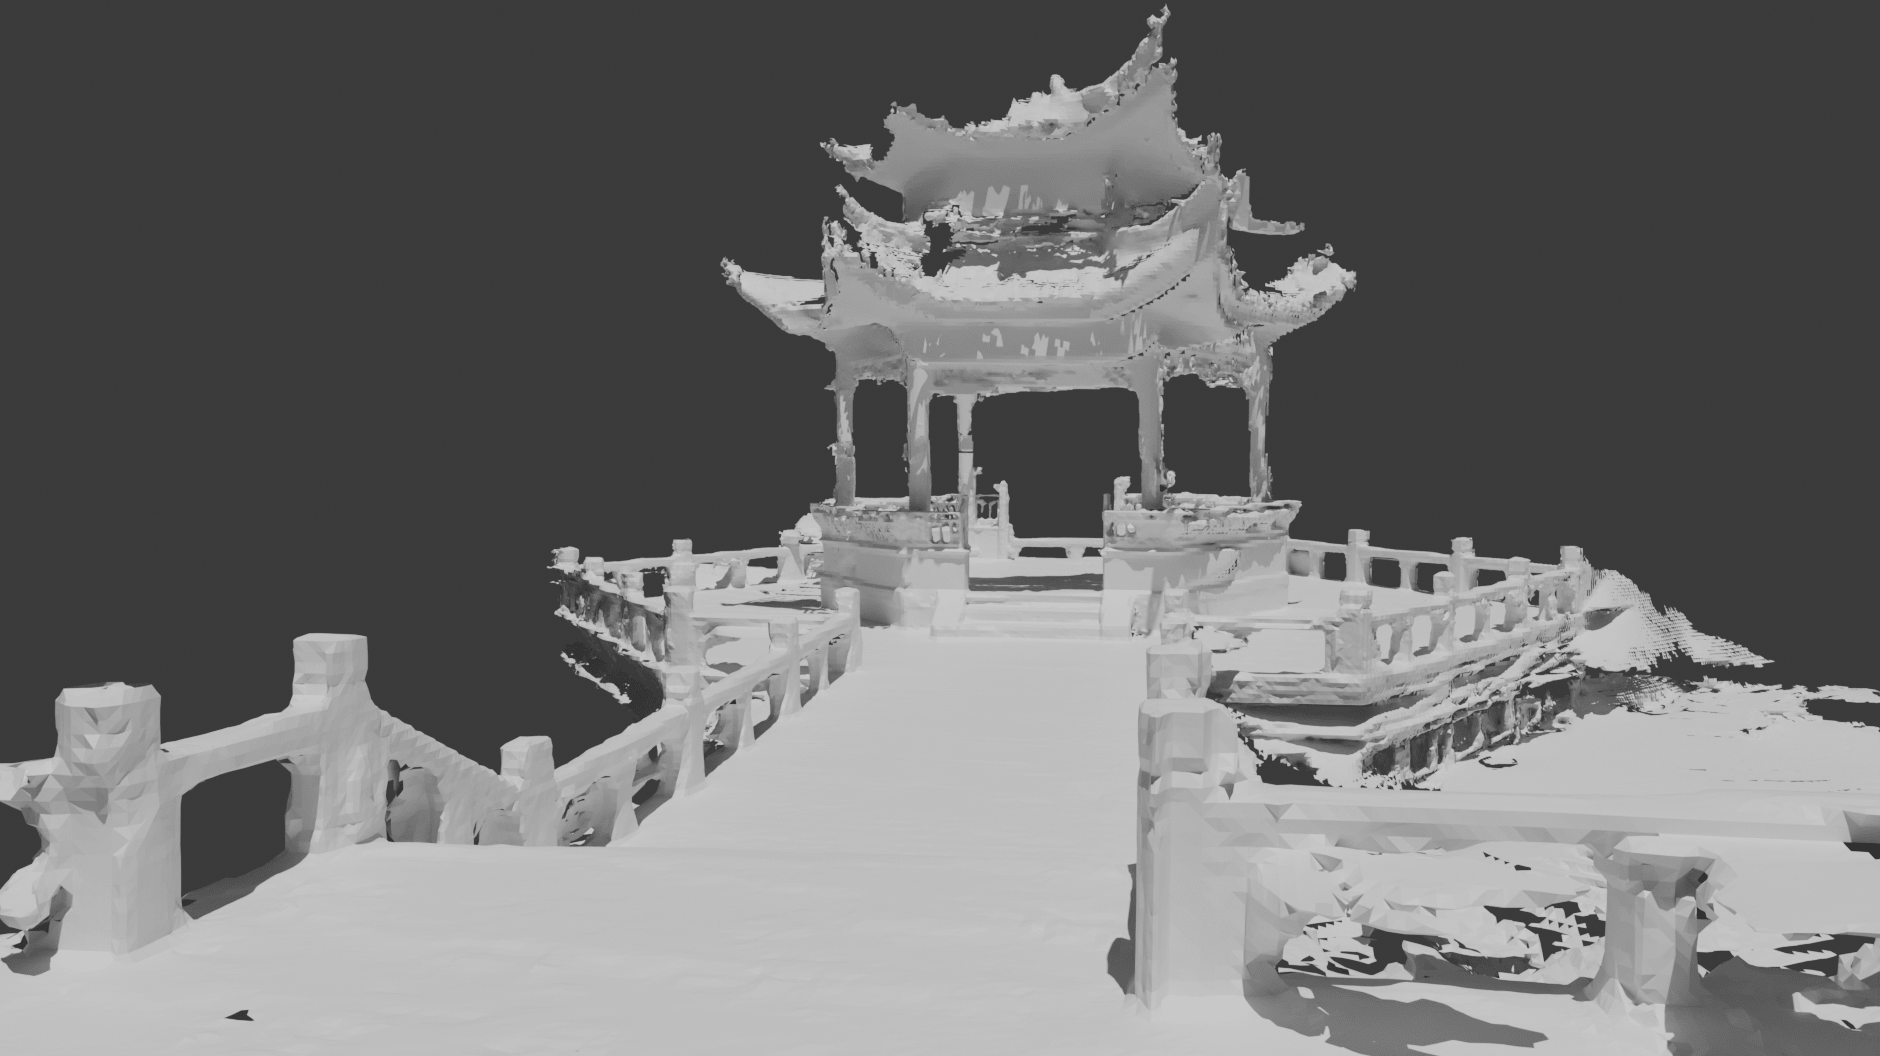} &
        \includegraphics[width=0.24\linewidth]{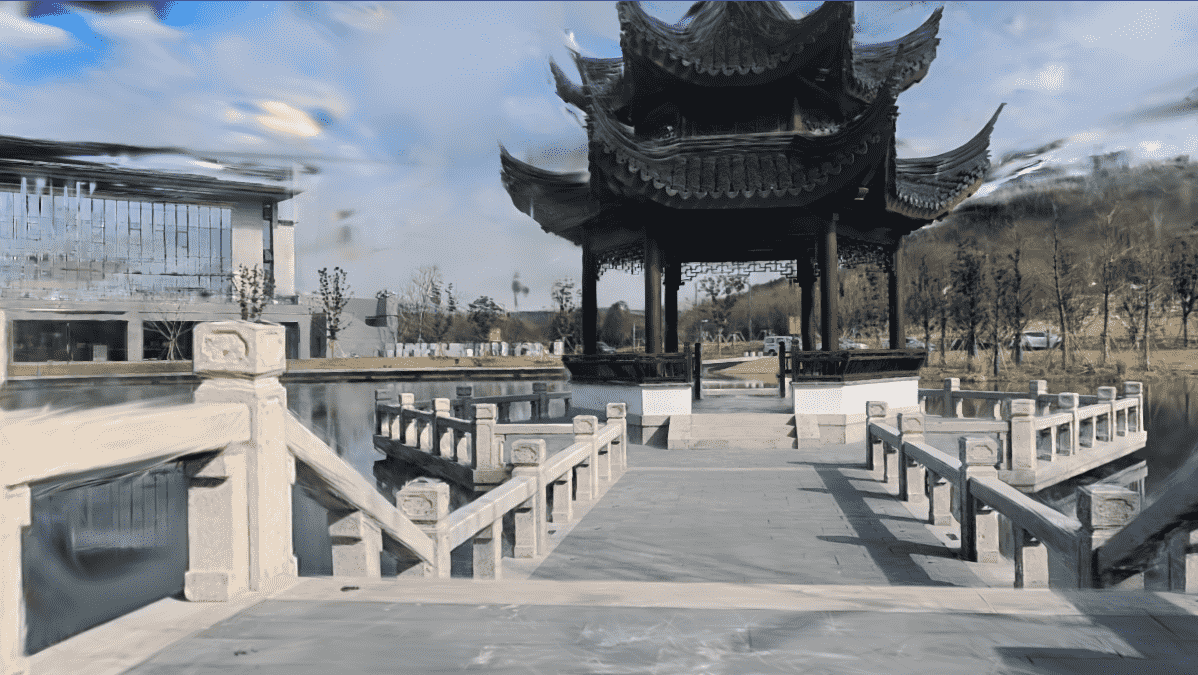} \\

        \includegraphics[width=0.24\linewidth]{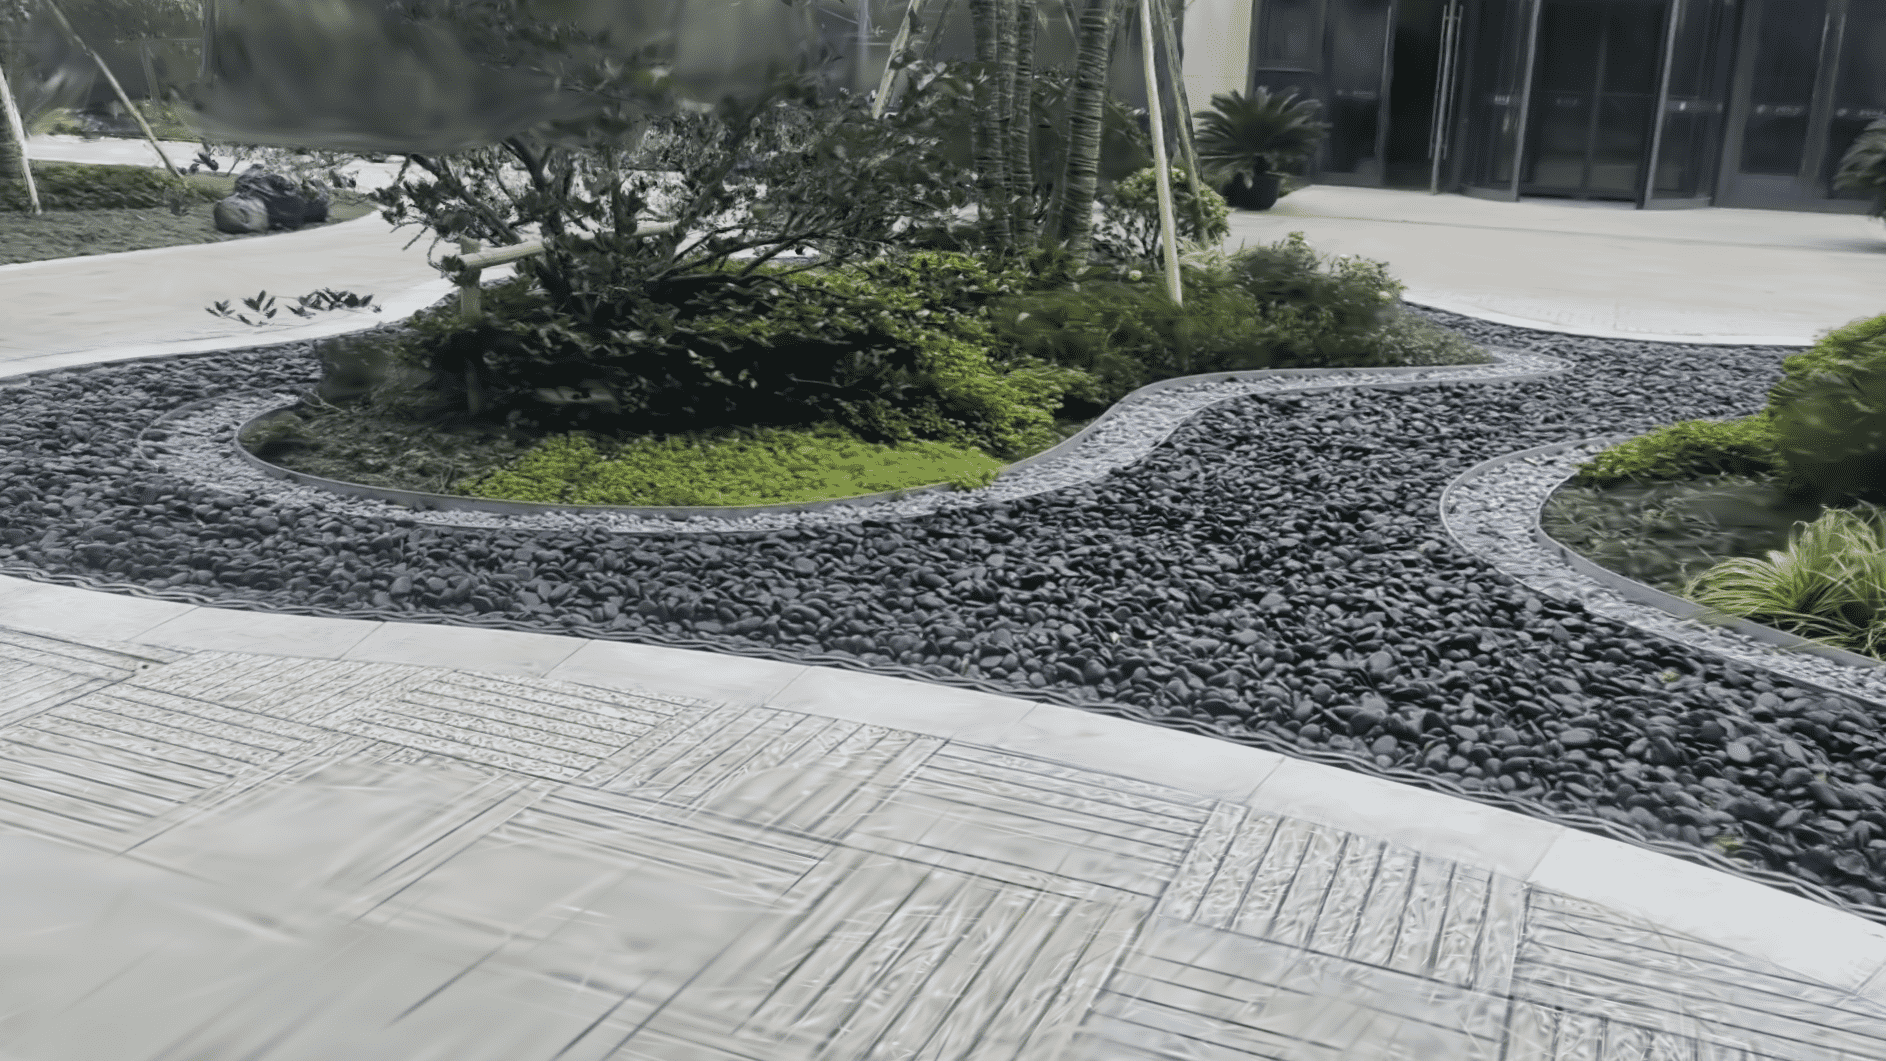} &
        \includegraphics[width=0.24\linewidth]{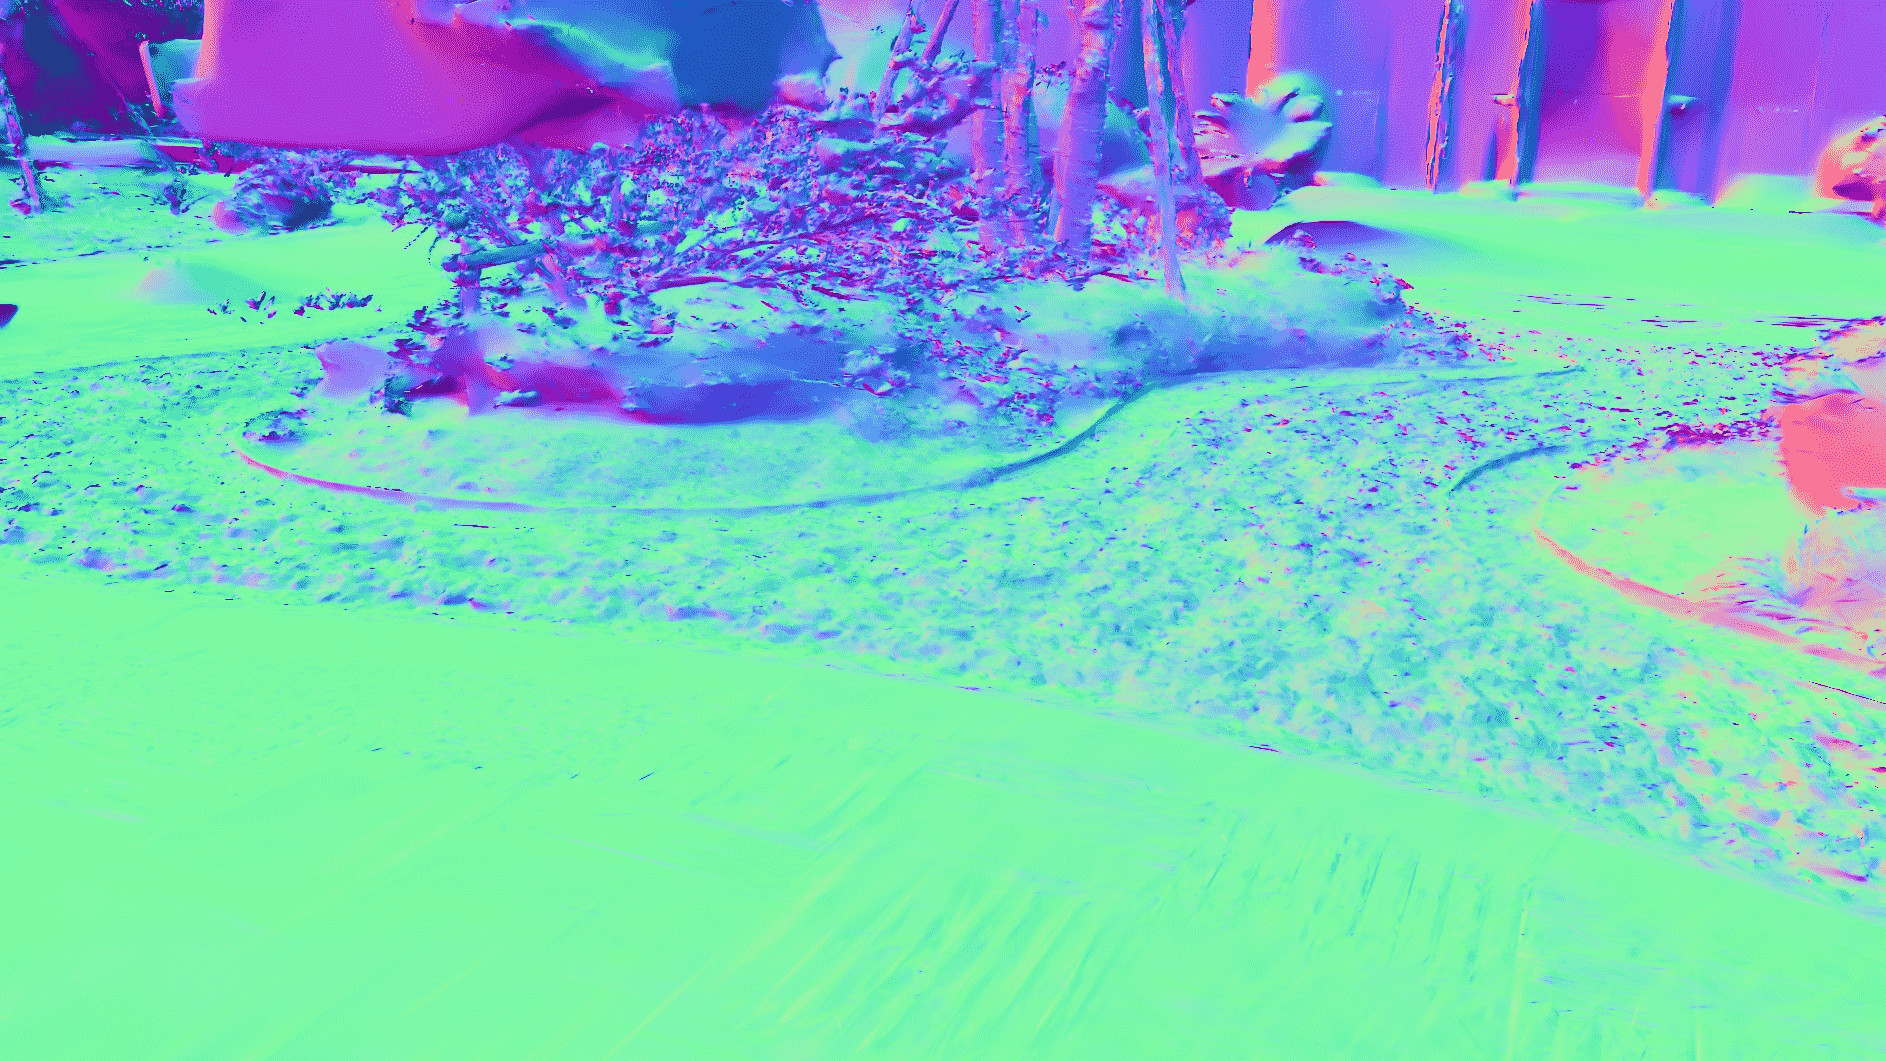} &
        \includegraphics[width=0.24\linewidth]{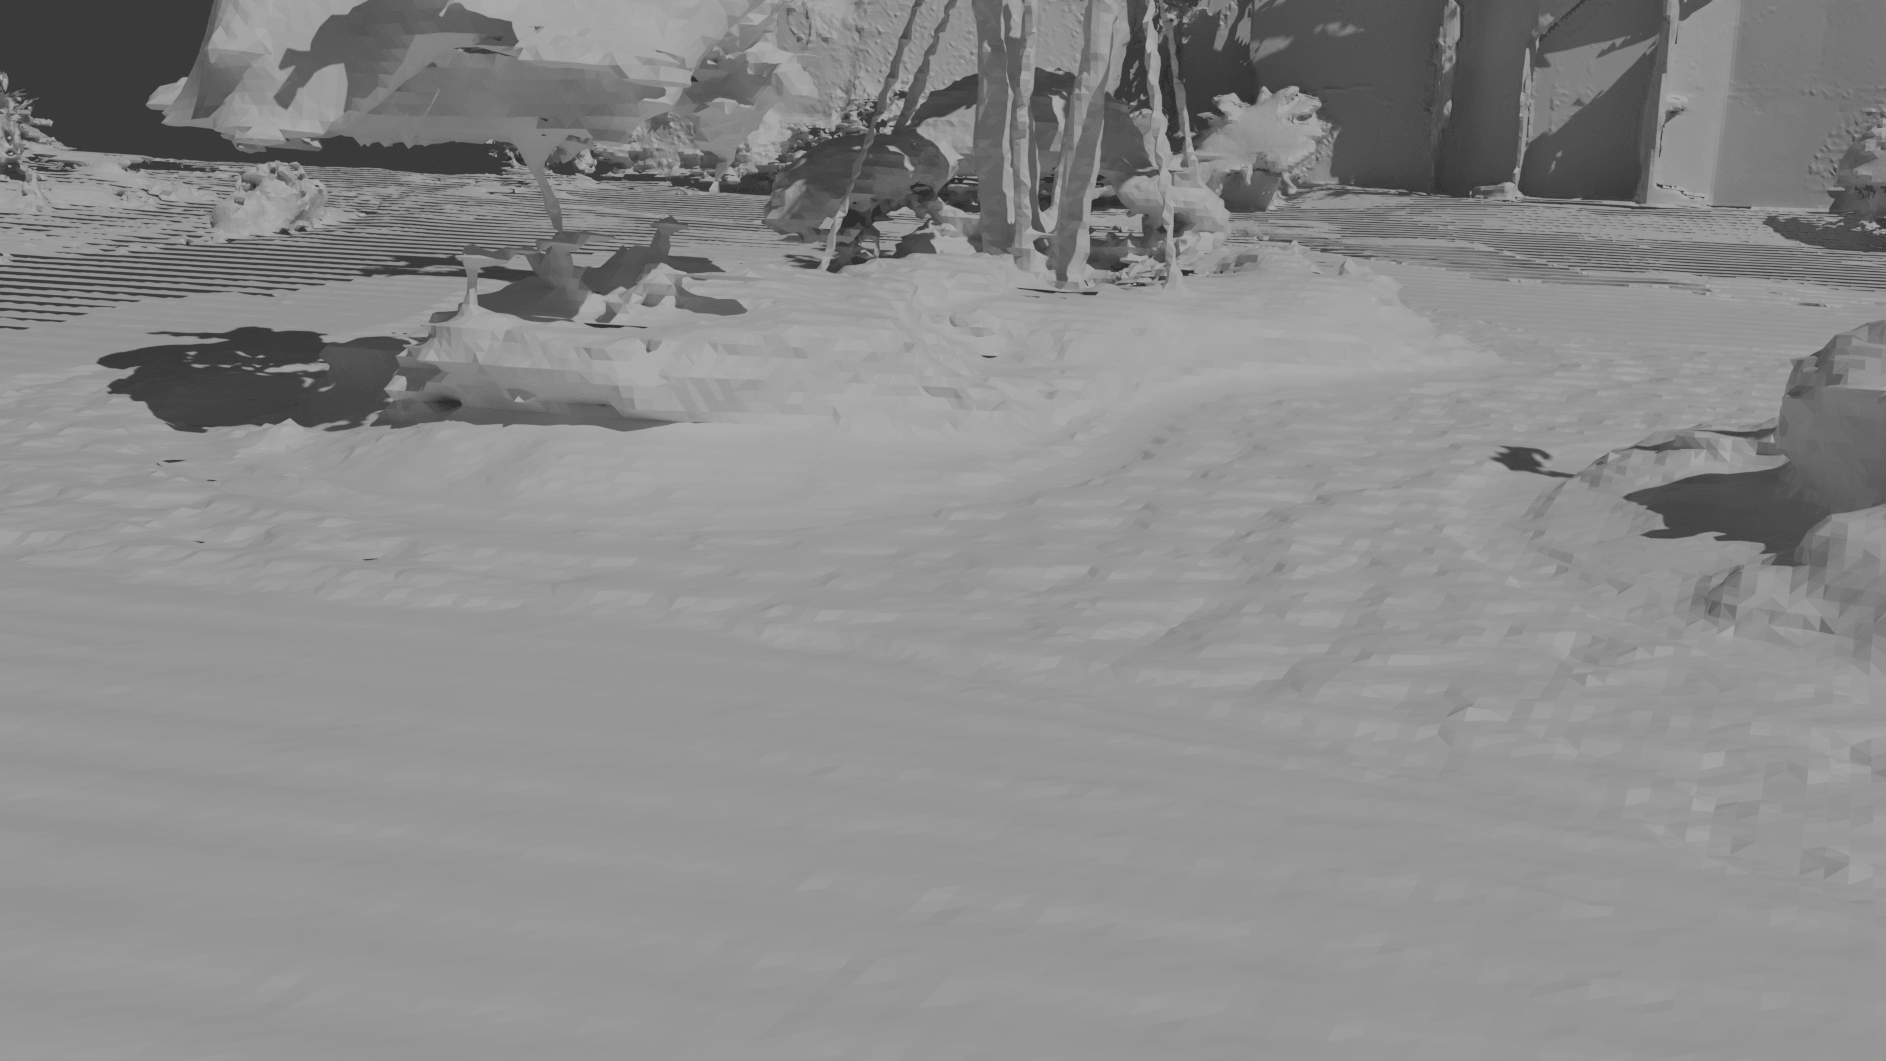} &
        \includegraphics[width=0.24\linewidth]{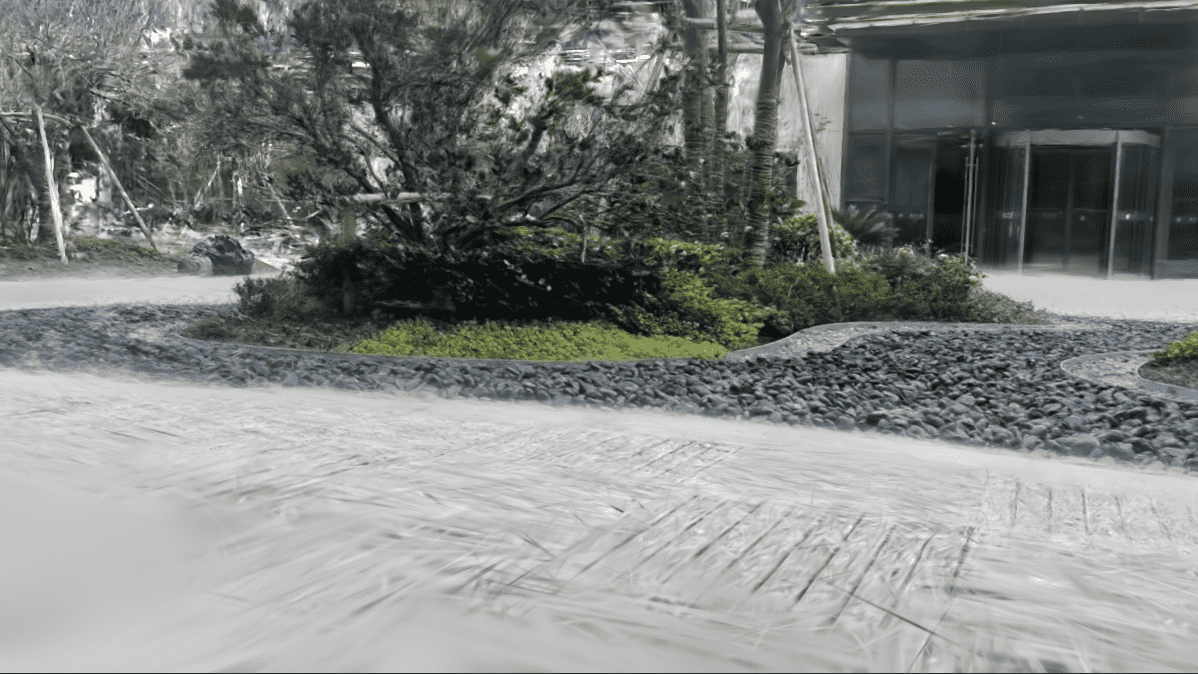} \\

        \small (a) Rendered Image & 
        \small (b) Rendered Normal & 
        \small (c) Extracted Mesh & 
        \small (d) Rendered Robot View \\
    \end{tabular}

    \caption{\textbf{Additional qualitative reconstruction results across various scenes.} 
The reconstruction comprises four components (from left to right): (a) rendered RGB image, (b) rendered normal map, (c) extracted mesh, and (d) simulated robot viewpoint (camera lowered to the eye level of a quadruped robot). These qualitative results further illustrate QuadVerse's visual rendering quality, mesh coherence, and robot-view consistency across diverse outdoor scenes.}
    \label{fig:qualitative_more}
\end{figure*}

% !TeX root = ../../main.tex

\section{Further Experiments and Analysis on Dynamics Compensation}
\label{sec:supp_dynamics_analysis}

This section provides a deeper analysis of the residual dynamics module, evaluating its standalone tracking performance, the necessity of its reward components, and its downstream impact on locomotion policy fine-tuning. We also include preliminary sim-to-sim experiments on additional quadruped platforms.

\subsection{Evaluation of the Residual Network}
\label{sec:supp_residual_eval}

\paragraph{Dataset and Evaluation Protocol.}
To rigorously evaluate the generalization of the residual network, we collected a test dataset consisting of 31 distinct trajectories, each lasting 10,000 frames (20 seconds) with a sampling interval of 0.002s, totaling 620 seconds of diverse locomotion data.
For evaluation, we initialize the simulation at the start of each trajectory and perform an open-loop replay of the recorded joint commands. We assess performance based on joint tracking error and gait consistency over the first 3,000 frames of each segment.

\paragraph{Ablation Study.}
Training the residual network requires a delicate balance between minimizing joint tracking error, maintaining gait similarity, and ensuring long-horizon stability. Figure \ref{fig:train_log} illustrates the learning curves for these objectives. The joint compensation performance typically peaks early but must settle into an equilibrium as gait constraints and longer replay horizons are enforced.
We conducted ablation studies on two critical components: the \textit{Gait Reward} and the \textit{Reset Mechanism}. Removing the reset condition (triggered by large deviations) severely degrades joint tracking performance, as the policy overfits to divergent trajectories rather than learning to correct instantaneous dynamics mismatch. Removing gait constraints can further reduce joint-space error, but it induces physically unrealistic artifacts such as foot jitter and ``sliding'' contacts; including gait rewards therefore helps the learned residual dynamics remain accurate in joint space while staying physically consistent at the contact level.

\begin{figure*}[t]
\centering
\includegraphics[width=1.0\linewidth]{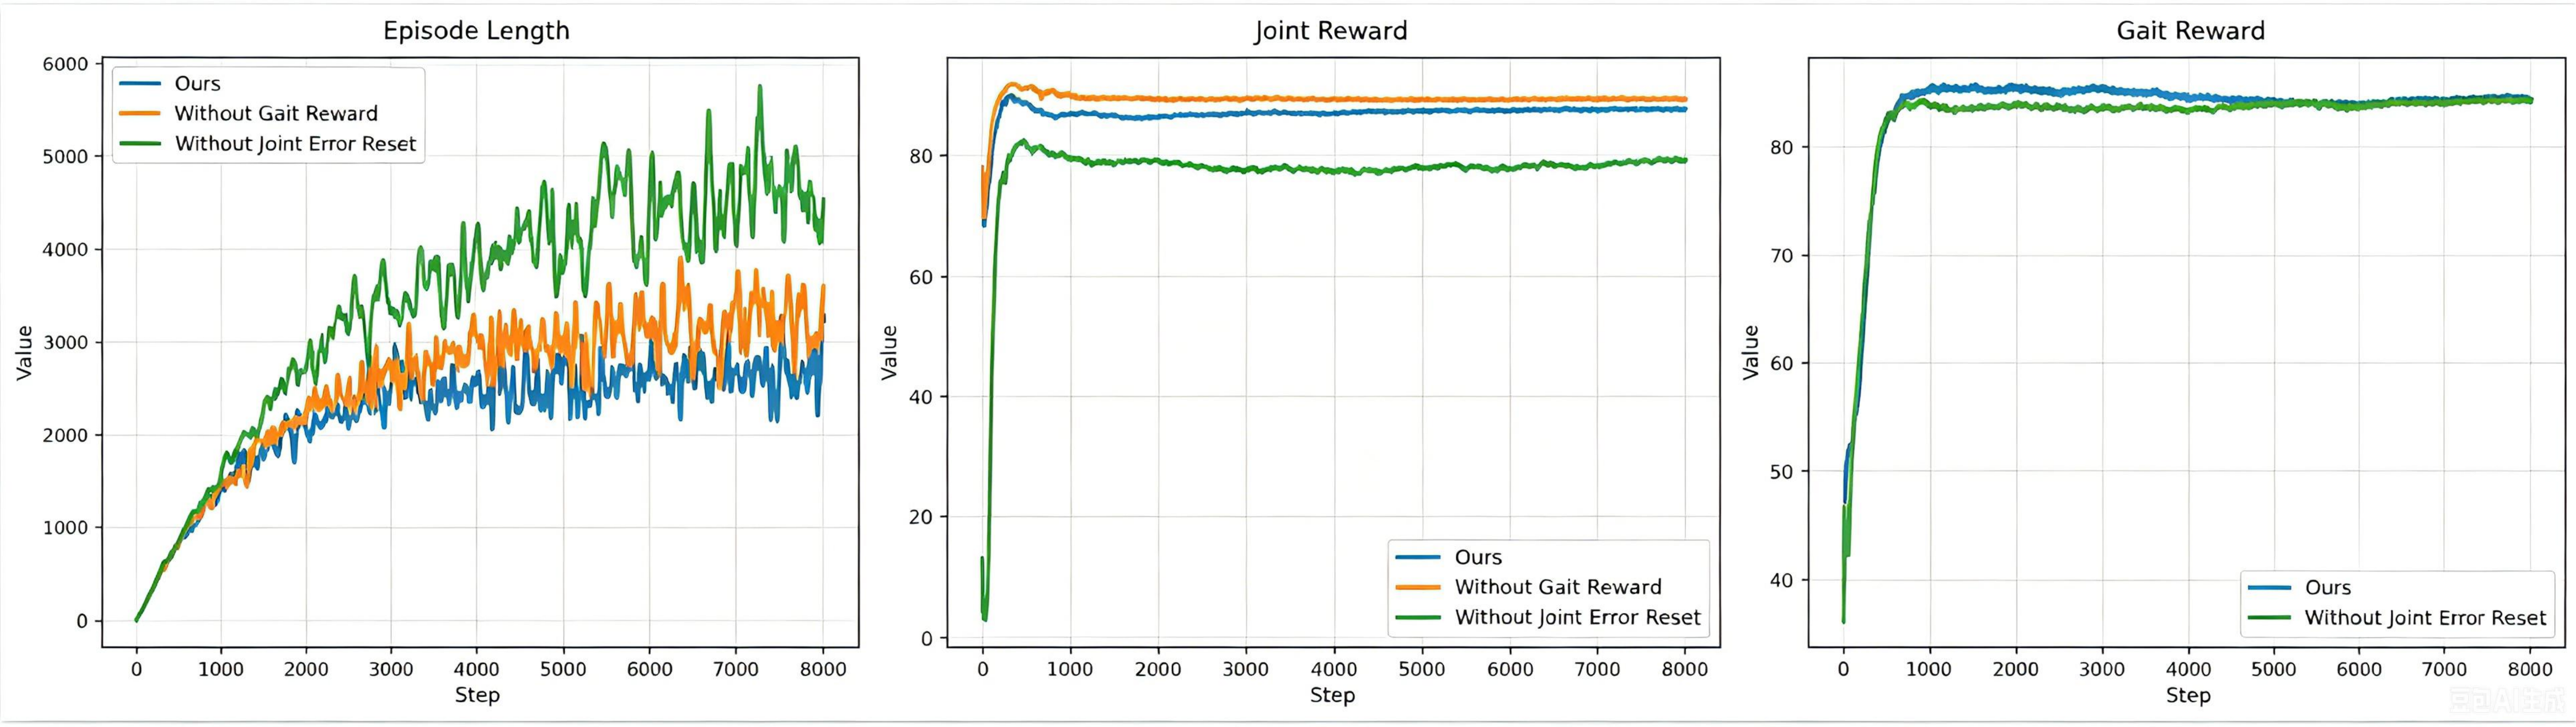}
\caption{Learning curves for average playback length, joint tracking reward, and gait reward. Our method (blue) achieves a balanced performance, whereas removing gait rewards (orange) or reset conditions (green) leads to suboptimal convergence in stability or tracking accuracy.}
\label{fig:train_log}
\end{figure*}

\subsection{Cross-Platform Sim-to-Sim Transfer}
\label{sec:supp_cross_platform}

To assess whether the proposed residual dynamics compensation pipeline is specific to a single robot platform, we further conduct cross-platform sim-to-sim transfer experiments on Unitree Go1 and Unitree A2. 
Due to limited access to additional hardware platforms, these experiments are performed as Isaac Gym-to-MuJoCo transfer rather than full real-world deployment. 
For each robot, we train the residual compensator in Isaac Gym using replay data generated from the target MuJoCo model, and evaluate whether the compensated Isaac Gym replay better matches the MuJoCo reference.

We adopt the same open-loop joint-space replay protocol as in Sec.~\ref{sec:supp_residual_eval}. 
Specifically, we compare the nominal simulator and the residual-compensated simulator by measuring joint-space replay error under identical command replay. 
The compensator consistently improves replay fidelity across platforms. 
For Unitree Go1, the residual compensator reduces the joint-space replay error by 72.5\%; for Unitree A2, the reduction is 85.4\%. 
For reference, the corresponding improvement on Unitree Go2 is 66.1\%. Figures~\ref{fig:cross_platform_joint_space} provides representative joint-space replay curves, analogous to Fig.~\ref{fig:joint_space} in the main paper. 
In both cases, the compensated simulator tracks the reference trajectory much more closely than the nominal simulator, indicating that the benefit of residual compensation is not limited to a single quadruped embodiment. 

\begin{figure*}[t]
    \centering
    \begin{subfigure}[t]{0.48\linewidth}
        \centering
        \includegraphics[width=\linewidth]{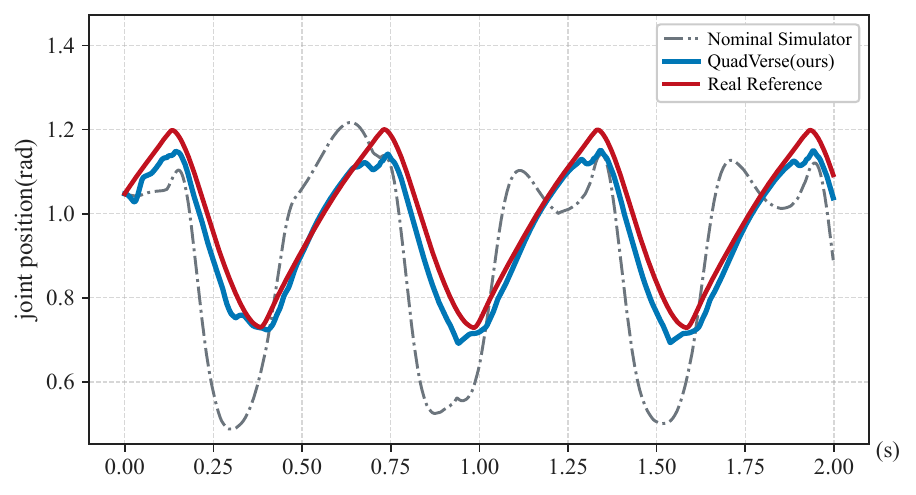}
        \caption{Unitree Go1}
        \label{fig:go1_joint_space}
    \end{subfigure}
    \hfill
    \begin{subfigure}[t]{0.48\linewidth}
        \centering
        \includegraphics[width=\linewidth]{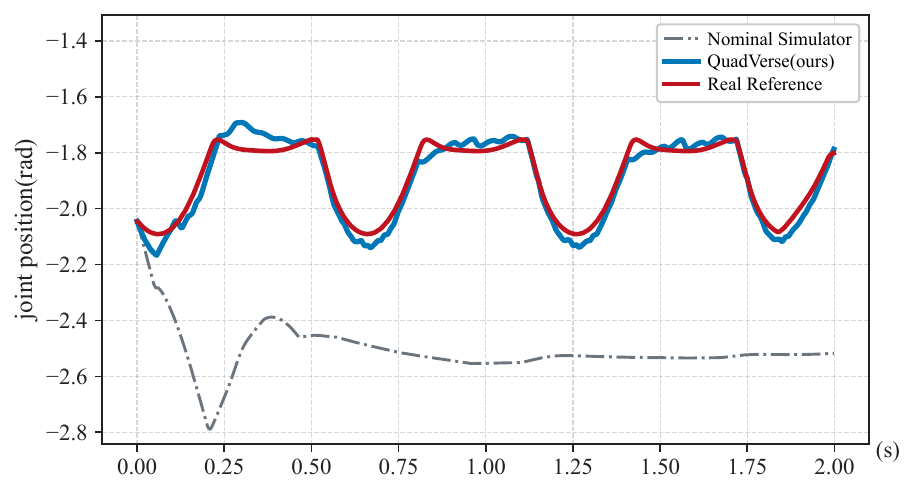}
        \caption{Unitree A2}
        \label{fig:a2_joint_space}
    \end{subfigure}
    \caption{\textbf{Cross-platform joint-space replay in sim-to-sim transfer.}
    Open-loop joint-space replay on Unitree Go1 (left) and Unitree A2 (right). 
    On both platforms, the residual-compensated simulator tracks the reference trajectory more closely than the nominal simulator.}
    \label{fig:cross_platform_joint_space}
\end{figure*}

\subsection{Locomotion Policy Fine-tuning and Deployment}
\label{sec:supp_locomotion_finetuning}

To evaluate whether the compensated dynamics benefits downstream policy learning, we fine-tune a locomotion policy with the frozen residual compensator inserted into the simulation loop. 
Both the nominal pre-training and QuadVerse fine-tuning use the Heterogeneous Information Matching (HIM) locomotion framework with a control frequency of 50\,Hz. 
During fine-tuning, the residual compensator is treated as part of the environment dynamics and its parameters are kept fixed. 
We fine-tune from a pre-trained locomotion policy rather than training from scratch because the pre-trained policy already provides a strong locomotion prior. 
This makes adaptation more sample-efficient and keeps exploration close to the replay distribution where the residual compensator is reliable, whereas early-stage training from scratch may visit highly out-of-distribution actions and states that are not covered by the compensation model.

We evaluate the resulting policies on five real-world locomotion tasks specified by velocity commands: \textit{right-turn}, \textit{left-turn}, \textit{slow-forward}, \textit{fast-forward}, and \textit{figure-eight}, with 10 trials per task. 
As shown in Fig.~\ref{fig:all_traj}, the QuadVerse policy consistently reduces trajectory error across different locomotion modes compared with the nominal policy. 
The improvement is especially visible in turning and figure-eight maneuvers, where actuator mismatch can accumulate into substantial heading and curvature errors; fine-tuning with compensated dynamics improves command tracking and yields more stable real-world trajectories. 
The remaining difference between left-turn and right-turn performance is mainly attributed to the command-tracking bias of the pre-trained locomotion policy, which can already favor one turning direction over the other in simulation.

\begin{figure*}[t]
\centering
\includegraphics[width=1.0\linewidth]{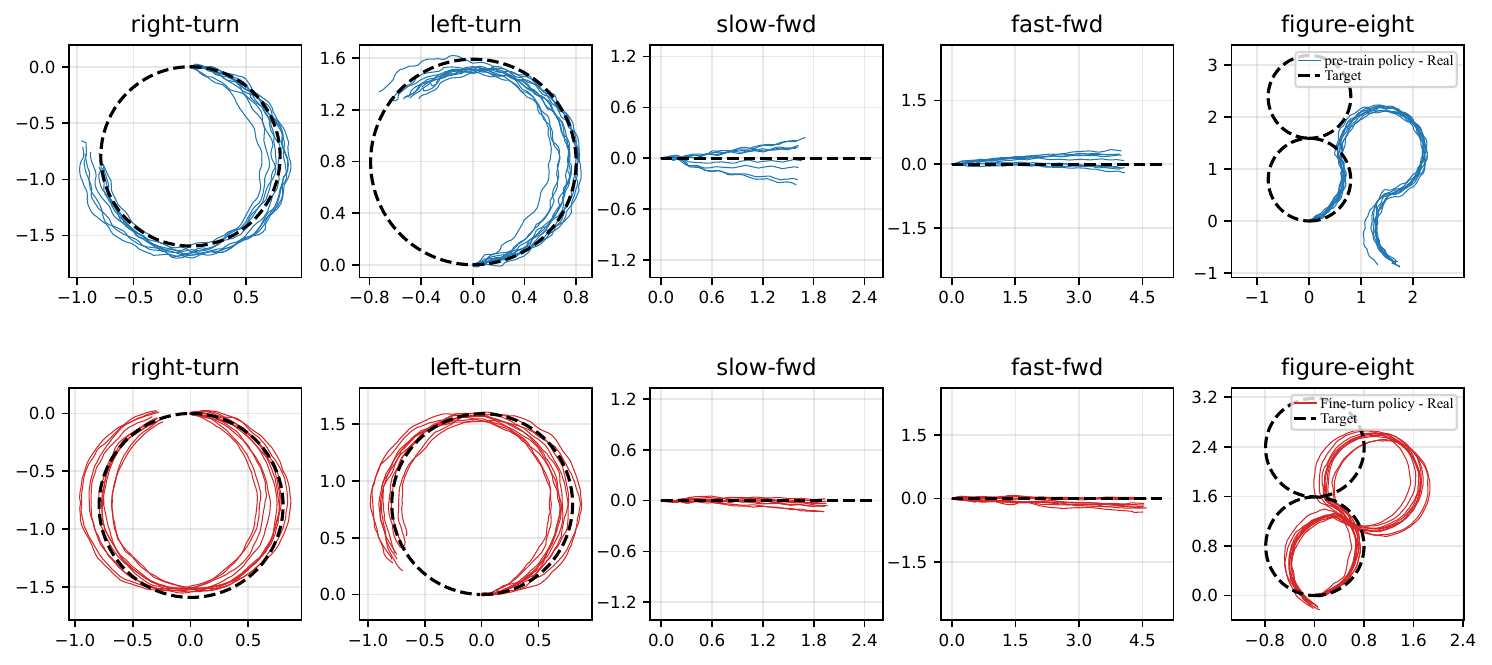}
\caption{\textbf{Additional real-world locomotion tracking results.}
Trajectory error across five locomotion tasks. 
The QuadVerse policy consistently reduces tracking error compared with the nominal policy across different commanded motion patterns.}
\label{fig:all_traj}
\end{figure*}

% !TeX root = ../../main.tex

\section{Details of Navigation Policy}
\label{sec:supp_navigation_details}

\subsection{Task Formulation and Evaluation Protocol} 
\label{sec:supp_nav_task}
We evaluate the full QuadVerse framework through an outdoor visual goal-seeking task. The robot is required to locate and approach a colored target cone using ego-centric RGB observations within a maximum episode duration of $T_{\max}=25$ seconds. An episode is considered successful if the robot's reference point reaches within $\epsilon=0.35$\,m of the target cone. To prevent the policy from overfitting to a fixed start-goal configuration, both the robot initial state and the goal location are randomized within predefined feasible regions during training and evaluation. For real-world evaluation, we conduct 25 trials with randomized initial robot poses and goal locations. Simulation results are averaged over 200 episodes. Success rate (SR) is defined as the fraction of successful episodes, and average reaching time (ART) is computed over all trials, with failed trials assigned the maximum episode duration $T_{\max}$.

\subsection{Navigation Policy Training} 
\label{sec:supp_nav_hierarchy}
The navigation policy is trained entirely within the QuadVerse simulation framework. We first reconstruct the deployment scene from captured RGB videos and use the optimized 3DGS representation to render ego-centric visual observations consistent with the robot's head-mounted camera. The reconstructed scene is also converted into a collision-ready semantic mesh and calibrated into a contact-calibrated terrain. The replay-trained residual actuator compensator is then frozen and inserted into the simulation loop, allowing the navigation policy to be trained under dynamics that better match real-world execution. The navigation policy itself does not use real-world navigation rollouts for training or fine-tuning. After training in simulation, the visual navigation policy is deployed zero-shot to the physical robot.

We use a hierarchical control architecture to decouple visual navigation from low-level locomotion. 
The high-level visual navigation policy runs at 5\,Hz and outputs a velocity command $\boldsymbol{v}_{\mathrm{cmd}}=(v_x, v_y, \omega_{\mathrm{yaw}})$, which is then tracked by the low-level locomotion controller.
The low-level controller runs at 50\,Hz and generates joint position targets from the commanded velocity and proprioceptive observations. During navigation policy training, the low-level locomotion controller is frozen, while the residual actuator compensator remains active in the simulation loop. The high-level policy observation consists of three components: 
(1) visual observation, ego-centric RGB images rendered from the reconstructed 3DGS scene. A frozen visual encoder is used to extract image features.
(2) task command, a one-hot encoding of the target color or target category.
(3) proprioceptive history, robot state history including base angular velocity, projected gravity, joint states, and the previous velocity command.
The policy output is squashed by a $\tanh$ activation and then scaled to predefined command limits, i.e., $|v_x| \leq 0.9$\,m/s, $|v_y| \leq 0.4$\,m/s, and $|\omega_{yaw}| \leq 1.0$\,rad/s.

The high-level visual navigation policy is modeled as an actor-critic network and trained using PPO. To handle partial observability, the policy includes an LSTM recurrent module. Training is performed in the QuadVerse simulation environment using 1024 parallel environments for 150 iterations. We apply visual and dynamics domain randomization to improve deployment robustness. Visual randomization includes camera extrinsic perturbation, image noise, brightness variation, and motion blur. Dynamics randomization includes perturbations to robot mass, friction, external disturbances, and initial robot states. 

\begin{table}[h]
\caption{Reward Function for the High-Level Navigation Policy}
\label{tab:nav_rewards}
\centering
\renewcommand{\tabcolsep}{5pt}
\begin{tabular}{llc}
\toprule
\textbf{Reward Term} & \textbf{Mathematical Formulation} & \textbf{Weight} \\
\midrule
\multicolumn{3}{c}{\textit{Task Achievement}} \\
\midrule
Reach Goal & $\mathbb{I}(d_t < 0.35)$ & $0.5$ \\
Goal Progress & $(d_{t-1} - d_t)\,\mathbb{I}(d_t > 0.35)$ & $5.0$ \\
Goal Close & $\mathrm{clip}\!\left(\frac{0.75-d_t}{0.75-0.35},0,1\right)$ & $0.2$ \\
Goal Heading & $1 - 2|\Delta\psi_t|/\pi$, if $d_t>0.35$; otherwise $1$ & $0.3$ \\
Stand Still & $\mathbb{I}(d_t < 0.35)(\|\boldsymbol{v}_{cmd}\|_2+0.4)^{-1}$ & $1.0$ \\
\midrule
\multicolumn{3}{c}{\textit{Command Tracking \& Regularization}} \\
\midrule
Track Lin. Vel. & $\exp(-\|\boldsymbol{v}_{xy}^{cmd}-\boldsymbol{v}_{xy}^{base}\|_2^2/0.25)$ & $0.2$ \\
Track Ang. Vel. & $\exp(-(\omega_z^{cmd}-\omega_z^{base})^2/0.25)$ & $0.2$ \\
Action Magnitude & $\|\boldsymbol{a}_{high}\|_2^2$ & $-0.002$ \\
\bottomrule
\end{tabular}
\end{table}

\subsection{Reward Design} 
\label{sec:supp_nav_reward} 
The high-level policy is trained with a composite reward consisting of target-reaching rewards, planar progress and heading terms, velocity-tracking terms, and an action-magnitude penalty. Let $d_t$ denote the planar head-to-goal distance and $\Delta\psi_t$ denote the yaw error between the robot heading and the goal direction. The configured reward weights are shown in Table~\ref{tab:nav_rewards}; internally, each configured weight is multiplied by the high-level control period.
\section{Conclusion}
\label{sec:supp_conclusion}

This supplementary material provides implementation details and extended analyses that support the main paper. 
We first present the reconstruction losses and semantic mesh calibration protocol, including semantic Gaussian training, LLM-assisted coarse friction priors, and trajectory-based posterior friction search. 
We then detail the residual actuator compensation module, including its network architecture, replay initialization, reward design, and ablation studies. 
Additional reconstruction examples, cross-platform sim-to-sim transfer results, locomotion fine-tuning experiments, and navigation policy details further demonstrate how the components of QuadVerse are instantiated in practice. 
Together, these supplementary results clarify the calibration and training procedures used to construct the aligned simulation environment for zero-shot quadruped visual-navigation deployment.
