# Supplementary material for: QuadVerse: An Integrated Framework Aligning Visual-Physical Reality for Quadruped Simulation
Source: arXiv:2606.07118 source file (2026-06-08)
Supplement: Supplementary file 2 [file 0_reconstruction_details.tex]

% !TeX root = ../../main.tex

\section{Details of Geometry-Anchored Reconstruction}
\label{app:reconstruction_details}

This section provides the detailed formulations of the geometry constraints used in our reconstruction pipeline. 
Our goal is not only to obtain photorealistic novel-view rendering, but also to recover surface geometry suitable for mesh extraction and downstream physical simulation.

\subsection{Geometry-Constrained Gaussian Optimization}
\label{app:geometry_constrained_gs}

We represent the scene as a set of 3D Gaussian primitives~\cite{kerbl3Dgaussians}. 
Each Gaussian is parameterized by a center position $\boldsymbol{\mu}_i \in \mathbb{R}^3$, covariance matrix $\boldsymbol{\Sigma}_i \in \mathbb{R}^{3\times3}$, opacity $\alpha_i$, and spherical harmonics coefficients $\boldsymbol{c}_i$. 
Although standard 3DGS provides efficient photorealistic rendering, its optimization is primarily driven by image reconstruction losses and may produce inaccurate surface geometry. 
To make the reconstructed scene suitable for collision mesh extraction, we incorporate several geometry-oriented regularization terms.

\paragraph{2D Planar Regularization.}
Following \cite{huang20242dgs}, we enforce a regularization term to flatten 3D Gaussian ellipsoids into 2D surfels. We minimize the scale component corresponding to the local z-axis (the smallest scale) to ensure primitives align with the physical surface:
\begin{equation}
    \mathcal{L}_{scale} = \sum_{i} \| \min(\boldsymbol{s}_{i,x}, \boldsymbol{s}_{i,y}, \boldsymbol{s}_{i,z}) \|_1
\end{equation}
where $\boldsymbol{s}_{i,\cdot}$ represents the scale factors of the $i$-th Gaussian along its local axes.

\paragraph{Unbiased Depth Rendering.}
To eliminate depth errors arising from the positional bias of weight accumulation in volumetric rendering, we adopt the unbiased depth rendering strategy proposed in \cite{chen2024pgsr}. This method analytically computes the intersection of rays with Gaussian planes to generate depth maps that accurately conform to the true geometric surface.

\paragraph{Multi-View Photometric Consistency.}
Relying solely on single-view reconstruction loss is insufficient for global geometric consistency. Inspired by \cite{campbell2008using, fu2022geo, chen2024pgsr}, we incorporate a multi-view photometric consistency loss. For a pixel $\mathbf{p}_r$ in a reference view $r$, we utilize the rendered depth $d_r$ and normal $\mathbf{n}_r$ to construct an induced homography $\mathbf{H}_{rn}$, warping the local patch to a neighboring view $n$. We constrain surface consistency by maximizing the Normalized Cross-Correlation (NCC):
\begin{equation}
    \mathcal{L}_{multi} = \frac{1}{|\mathcal{W}|} \sum_{\mathbf{p}_r \in \mathcal{W}} \left( 1 - \text{NCC}(\mathcal{P}(\mathbf{p}_r), \mathcal{P}(\mathbf{H}_{rn}\mathbf{p}_r)) \right)
\end{equation}
where $\mathcal{W}$ denotes the set of valid pixels and $\mathcal{P}(\cdot)$ represents the local patch centered at the pixel.

\subsection{Integration of Normal Priors}
\label{app:normal_prior}
Photometric consistency often degrades in texture-less or non-Lambertian regions. To enhance geometric fidelity, we utilize \cite{ye2024stablenormal} to predict a geometric normal map $\mathbf{N}_{prior}$ for each frame, serving as a prior to constrain the rendered normals $\mathbf{N}_{rend}$. The normal consistency loss $\mathcal{L}_{normal}$ is defined as:
\begin{equation}
    \omega_{img}(\mathbf{p}) = \left( \text{clip}\left( 1.0 - \|\nabla \boldsymbol{I}(\mathbf{p})\|, 0, 1 \right) \right)^2
\end{equation}
\begin{equation}
    \mathcal{L}_{normal} = \frac{1}{|\mathcal{\boldsymbol{W}}|} \sum_{\mathbf{p} \in \mathcal{W}} \omega_{img}(\mathbf{p}) \| \mathbf{N}_{prior}(\mathbf{p}) - \mathbf{N}_{rend}(\mathbf{p}) \|_1
\end{equation}
where $\|\nabla \boldsymbol{I}(\mathbf{p})\|$ is the magnitude of the image gradient. The weight $\omega_{img}$ adaptively attenuates the supervision in high-frequency texture regions.

\subsection{Overall Optimization Objective}
\label{app:overall_reconstruction_objective}

The final reconstruction objective combines the standard image reconstruction loss with the geometry-oriented regularization terms:
\begin{equation}
    \mathcal{L}_{recon}
    =
    \mathcal{L}_{rgb}
    +
    \lambda_{scale}\mathcal{L}_{scale}
    +
    \lambda_{multi}\mathcal{L}_{multi}
    +
    \lambda_{normal}\mathcal{L}_{normal},
    \label{eq:app_recon_objective}
\end{equation}
where $\mathcal{L}_{rgb}$ is the standard photometric rendering loss, and $\lambda_{scale}$, $\lambda_{multi}$, and $\lambda_{normal}$ are weighting coefficients. 
In our experiments, we set $\lambda_{scale}=100$, $\lambda_{multi}=0.15$, and $\lambda_{normal}=0.01$.
