# Supplementary material for: QuadVerse: An Integrated Framework Aligning Visual-Physical Reality for Quadruped Simulation
Source: arXiv:2606.07118 source file (2026-06-08)
Supplement: Supplementary file 3 [file 1_contact_calibration.tex]

% !TeX root = ../../main.tex

\section{Details of Semantic Mesh-Based Contact Calibration}
\label{sec:supp_contact_calibration}

This section provides implementation details for the semantic mesh-based contact calibration described in the main paper. 
The calibration pipeline consists of three steps: semantic Gaussian training, mesh-level semantic propagation, and prior-posterior friction calibration. 

\subsection{Semantic Gaussian Training and Mesh Label Propagation}
\label{sec:supp_semantic_gaussian}

We define a compact set of terrain-level semantic classes for contact calibration, focusing on visually distinguishable categories that are relevant to foot-terrain interaction rather than fine-grained object recognition. 
Raw 2D segmentation labels are merged into a small number of contact-relevant terrain categories, such as \textit{hard ground}, \textit{grass}, \textit{snow/ice}, \textit{soil}, \textit{sand}, \textit{gravel}, \textit{wood}, \textit{tile}, and \textit{obstacle/background}. 
This merged label space preserves the terrain semantics needed for coarse physical reasoning while avoiding unnecessary visual granularity. 
The category set is not fixed and can be expanded or merged according to the semantic diversity of each reconstructed environment.

To associate semantic labels with the reconstructed 3D scene, we augment each Gaussian primitive with a learnable semantic feature vector $\boldsymbol{f}_i \in \mathbb{R}^{C}$, where $C$ is the number of merged semantic classes. 
During rendering, these 3D semantic features are splatted to the image plane in the same manner as color features, producing pixel-wise semantic logits $\boldsymbol{S}_{rend}$. 
We supervise the rendered semantic logits using pseudo-labels $\boldsymbol{L}_{pseudo}$ generated by a 2D segmentation model~\cite{chen2022vision}. 
The semantic loss is defined as
\begin{equation}
    \mathcal{L}_{sem}
    =
    \mathrm{CrossEntropy}
    \left(
    \boldsymbol{S}_{rend},
    \boldsymbol{L}_{pseudo}
    \right).
    \label{eq:supp_semantic_loss}
\end{equation}
This loss is jointly optimized with the photometric reconstruction loss and geometry regularization terms, yielding a 3DGS scene that is both geometrically consistent and semantically annotated.

After mesh extraction, we propagate the learned Gaussian semantics to the collision mesh. 
For each mesh face, we use its center point as the query point and retrieve the $K=5$ nearest Gaussian primitives in 3D space. 
Each neighboring Gaussian is assigned the semantic class with the largest feature logit, and the mesh-face label is determined by majority voting among the five neighbors. 
Small isolated regions can be merged into the neighboring majority class to avoid fragmented material assignments. 
The resulting per-face semantic labels define region-level terrain partitions for coarse friction assignment and posterior calibration.

\subsection{LLM-Assisted Coarse Friction Prior}
\label{sec:supp_llm_prior}

For each semantic terrain class, we query a commonsense reasoning model, GPT-4~\cite{achiam2023gpt}, to obtain a deterministic nominal friction coefficient. 
The LLM output is not treated as an exact physical measurement; instead, it provides a reasonable initialization for spatially varying contact parameters.
We use a fixed prompt template and deterministic decoding to ensure consistent output formatting across scenes.
The prompt takes the robot context and the list of semantic terrain labels as input, and returns a JSON object mapping each label to a scalar friction coefficient.
The prompt template is shown in Table~\ref{tab:supp_llm_prompt}.

\begin{table}[ht]
\centering
\caption{Prompt template used for LLM-assisted coarse friction prior initialization.}
\label{tab:supp_llm_prompt}
\begin{tcolorbox}[
    width=\linewidth,
    colback=gray!4,
    colframe=gray!50,
    boxrule=0.5pt,
    arc=2pt,
    left=8pt,
    right=8pt,
    top=4pt,
    bottom=4pt,
    fonttitle=\bfseries\small,
    title=LLM Prompt Template for Coarse Friction Prior,
]
\footnotesize
\setlength{\parskip}{5pt}

\noindent\textbf{System prompt.}
You are an expert in robotics simulation and terrain contact modeling.
Estimate coarse friction coefficients for a quadruped robot walking on different terrain surfaces.

\noindent\textbf{Robot context.}
\begin{itemize}[leftmargin=1.4em, itemsep=1pt, topsep=2pt, parsep=0pt]
    \item Robot: Unitree Go2 quadruped robot.
    \item Foot material: rubber foot pads.
    \item Robot weight: approximately 15\,kg.
\end{itemize}

\noindent\textbf{Task.}
Given a list of semantic terrain labels, assign one deterministic nominal friction coefficient to each terrain class.
The values should be coarse priors for simulation, not exact measured physical parameters.

\noindent\textbf{Constraints.}
\begin{itemize}[leftmargin=1.4em, itemsep=1pt, topsep=2pt, parsep=0pt]
    \item Each coefficient should be a float in $[0.0,\,1.5]$.
    \item Return only a JSON object.
    \item Do not include explanations.
\end{itemize}

\noindent\textbf{User input.}
List of semantic terrain labels:
\texttt{[class\_1, class\_2, \ldots, class\_N]}.
\end{tcolorbox}
\end{table}

The returned class names are normalized to match the semantic labels on the mesh. 
For regions whose nominal friction exceeds an empirical slip threshold, we directly keep the coarse prior because the robot trajectory is weakly affected by the exact value in this high-traction regime. 
The threshold is empirically set to $\mu_{\mathrm{slip}}=0.5$ based on preliminary replay experiments.
Posterior search is applied only to slip-prone semantic regions whose friction prior falls below this threshold.

\subsection{Trajectory-Based Posterior Friction Search}
\label{sec:supp_posterior_search}

For slip-prone regions, we refine the friction coefficient using real-world locomotion replay. 
The optimization variable is a single region-level friction coefficient $\mu_r$ for each slip-prone semantic region $r$, rather than a separate coefficient for every mesh face. 
This region-level parameterization keeps the search low-dimensional and matches the semantic partition used by the simulator.

As formulated in Eq.~\ref{eq:friction_search} of the main paper, posterior calibration selects the friction value that minimizes the trajectory discrepancy between simulated replay and real robot motion. In practice, the objective is evaluated over multiple recorded replay segments rather than a single trajectory. 
For each segment, we initialize the simulation from the recorded base pose and joint state, replay the recorded locomotion command sequence, and compute the mean base-position error against the corresponding recorded LiDAR-SLAM trajectory.

We use a one-dimensional grid search centered at the coarse prior $\mu_r^0$. 
Specifically, we search $\mu_r \in [\mu_r^0 - 0.2, \mu_r^0 + 0.2]$ with step size $\Delta\mu=0.01$, clipped to the valid simulator range. 
During the search for one slip-prone region, friction values of all other regions are kept fixed at their current priors. 
If multiple slip-prone regions are present, we calibrate them region by region.
After posterior search, the optimized friction coefficient $\mu_r^\star$ is assigned to all mesh faces belonging to the corresponding semantic region. 
The resulting contact-calibrated terrain is then used for residual dynamics compensation and downstream policy training.
