# Supplementary material for: QuadVerse: An Integrated Framework Aligning Visual-Physical Reality for Quadruped Simulation
Source: arXiv:2606.07118 source file (2026-06-08)
Supplement: Supplementary file 4 [file 2_dynamics_training.tex]

% !TeX root = ../../main.tex

\section{Details of Residual Dynamics Compensation}
\label{sec:supp_dynamics_training}

\subsection{Network Architecture and State Space}
The residual dynamics policy is implemented as a Multilayer Perceptron (MLP) with two hidden layers of 128 units each, utilizing ELU activation functions. The network operates at the simulation control frequency (500 Hz).

We employ an asymmetric actor-critic architecture to leverage privileged information during training. 
\textbf{The policy network (actor)} uses only simulation-available observations so that it can be inserted into the simulation loop during replay and downstream policy fine-tuning.
Its input includes the target joint positions from the locomotion policy, proprioceptive joint positions and velocities, binary foot contact states, the gravity vector in the body frame, base height, body orientation, and the previous action. 
\textbf{The value network (critic)} augments this observation with ground-truth real-world signals to guide learning: real-world joint states, measured foot contact forces, base yaw rate, and true body orientation. 
To capture temporal dynamics and actuator delays, both networks stack a history window of the preceding 20 frames.

\subsection{Training Process and Initialization Strategy}
The training process is governed by specific termination criteria to ensure the learned residual dynamics remain within a valid distribution. An episode is terminated and reset if: (1) the playback trajectory reaches its end; (2) abnormal external forces are detected on the base; or (3) the simulated joint positions deviate from the real-world reference by more than 0.4 rad. Large deviations indicate that the simulation state has diverged significantly from the reference data, rendering subsequent samples uninformative for residual learning.

Upon reset, the simulation is initialized by sampling a timestamp from the recorded replay data. 
The recorded base pose is first transformed into the simulator frame aligned with the reconstructed mesh. 
The simulated robot's base pose and joint states are then initialized from the corresponding recorded values, while unobserved or noisy quantities such as base linear velocity are initialized using finite differences or set to zero for stability.

This incomplete state initialization inevitably introduces transient tracking errors at the beginning of an episode (a "cold start" problem). To mitigate the bias introduced by these initial transients, we do not impose a short fixed horizon for episodes. Instead, we allow the simulation to run until the end of the reference trajectory. This strategy provides a sufficiently long horizon for the dynamics to stabilize, ensuring that the gradient updates are dominated by the stable tracking phase rather than the initial alignment error.

\subsection{Reward Formulation}
The reward function is designed to balance joint-space tracking accuracy with gait plausibility. The detailed terms and their corresponding weights are enumerated in Table \ref{tab:reward_terms}.

\begin{table}[h]
\caption{Reward Terms for Dynamics Compensation}
\label{tab:reward_terms}
\centering

\begin{tabular}{lcc}
\toprule
\textbf{Reward Component} & \textbf{Mathematical Term} & \textbf{Weight} \\
\midrule
\multicolumn{3}{c}{\textit{Joint Space Tracking}} \\
\midrule
Joint Pos. (Relaxed) & $\exp(-2.5\|\mathbf{q}_{real} - \mathbf{q}_{sim}\|_2^2)$ & $100.0$ \\
Joint Pos. (Moderate) & $\exp(-20\|\mathbf{q}_{real} - \mathbf{q}_{sim}\|_2^2)$ & $100.0$ \\
Joint Pos. (Strict) & $\exp(-100\|\mathbf{q}_{real} - \mathbf{q}_{sim}\|_2^2)$ & $100.0$ \\
\midrule
\multicolumn{3}{c}{\textit{Gait and Contact Imitation}} \\
\midrule
Foot Contact & $\mathbb{I}(F_{sim} > 10 \land F_{real} > 20)$ & $100.0$ \\
Foot Slip Penalty & $\exp(-10\|\mathbf{v}_{foot, xy}^{sim}\|_2^2)$ & $100.0$ \\
Base Linear Vel. (Z) & $\exp(-10\|\mathbf{v}_{z}^{sim}\|_2^2)$ & $50.0$ \\
Ang. Vel. (Yaw) & $\exp(-4\|\omega_{yaw}^{real} - \omega_{yaw}^{sim}\|_2^2)$ & $100.0$ \\
\midrule
\multicolumn{3}{c}{\textit{Regularization}} \\
\midrule
Action Rate & $\exp(-\|\mathbf{a}_{t} - \mathbf{a}_{t-1}\|_2^2)$ & $5.0$ \\
Action Norm & $\exp(-0.01 \|\mathbf{a}_{t}\|_2^2)$ & $100.0$ \\
\bottomrule
\end{tabular}
\end{table}
