# Supplementary material for: QuadVerse: An Integrated Framework Aligning Visual-Physical Reality for Quadruped Simulation
Source: arXiv:2606.07118 source file (2026-06-08)
Supplement: Supplementary file 5 [file 3_reconstruction_results.tex]

% !TeX root = ../../main.tex

\section{Additional Qualitative Results of Scene Reconstruction}
\label{sec:supp_reconstruction_results}

Figure~\ref{fig:qualitative_more} shows additional qualitative reconstruction results across multiple outdoor scenarios. From left to right, the four key components are as follows: (a) the rendered RGB image, (b) the rendered normal map, (c) the extracted mesh, and (d) the simulated robot perspective, with the camera viewpoint lowered to mimic the view of a quadruped robot like Go2. These results showcase the strong visual realism, accurate geometric reconstruction, and alignment with the robot's perceptual perspective.

\begin{figure*}[p]
    \centering
    \setlength{\tabcolsep}{1pt}

    \begin{tabular}{cccc}
        \includegraphics[width=0.24\linewidth]{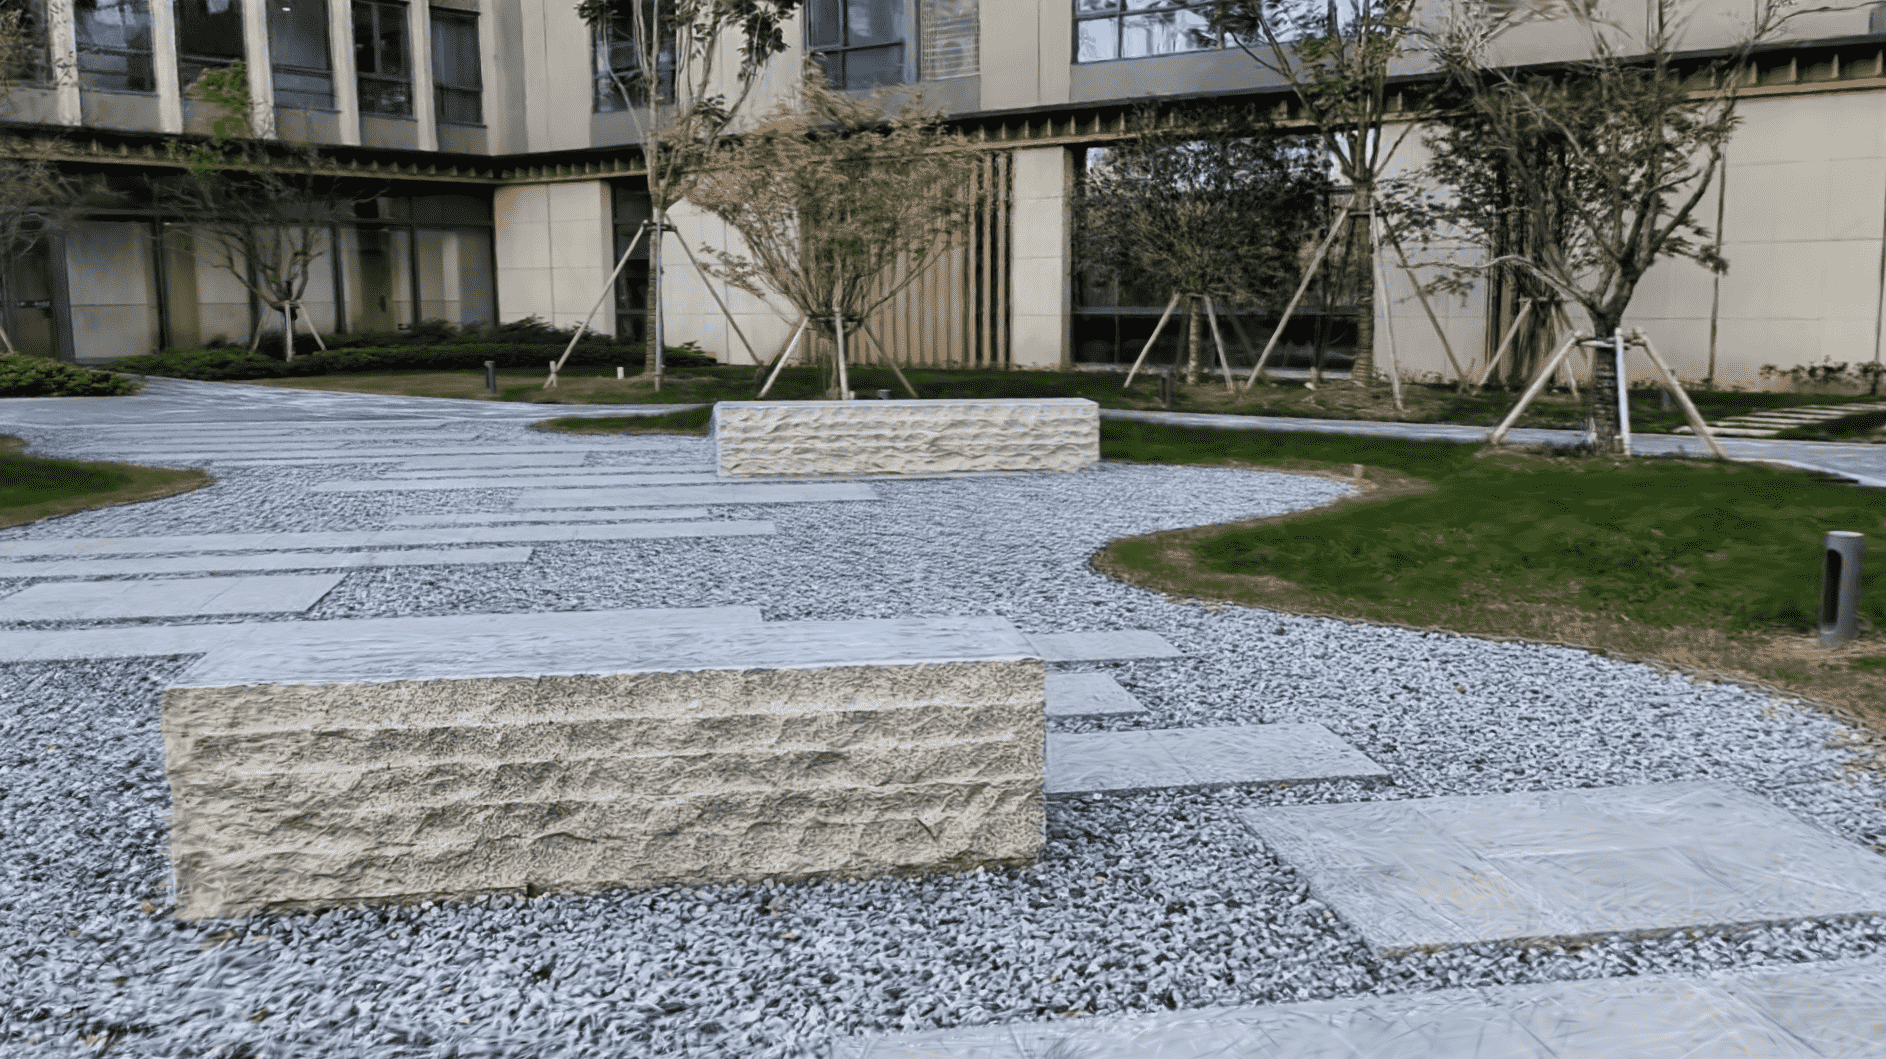} &
        \includegraphics[width=0.24\linewidth]{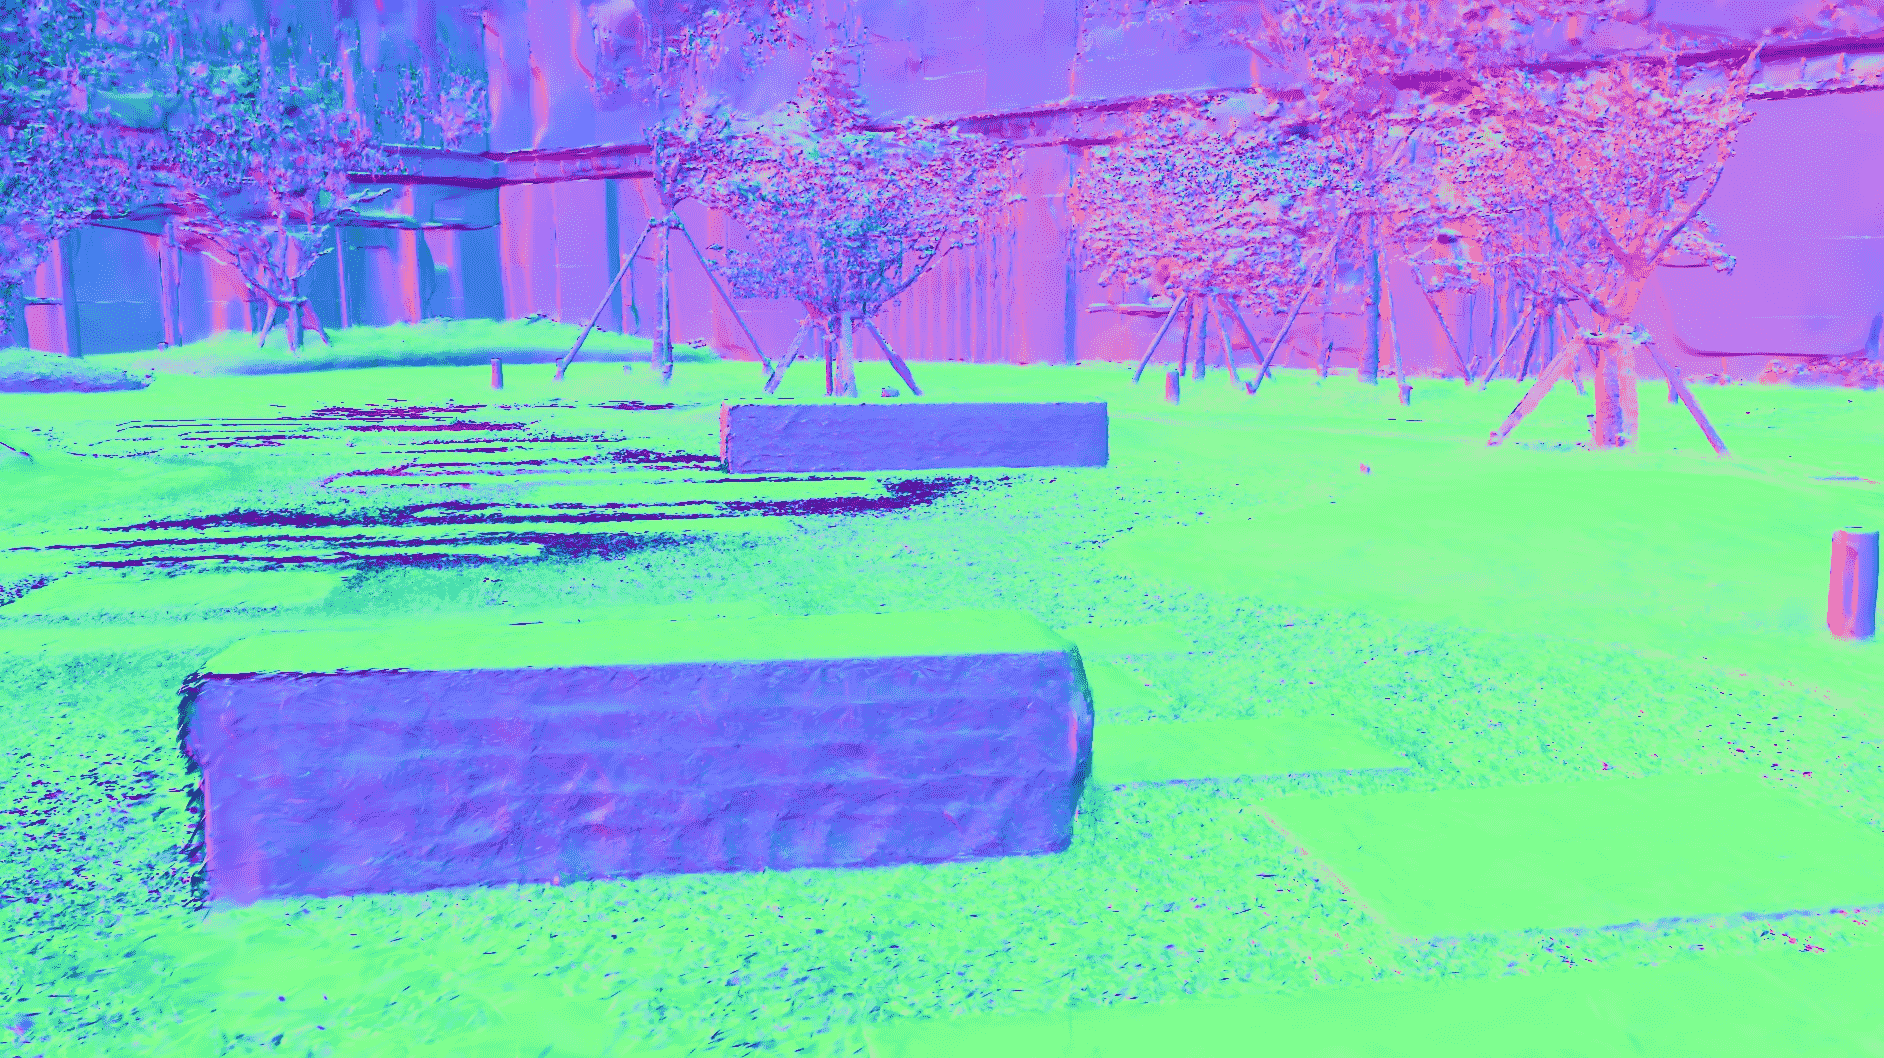} &
        \includegraphics[width=0.24\linewidth]{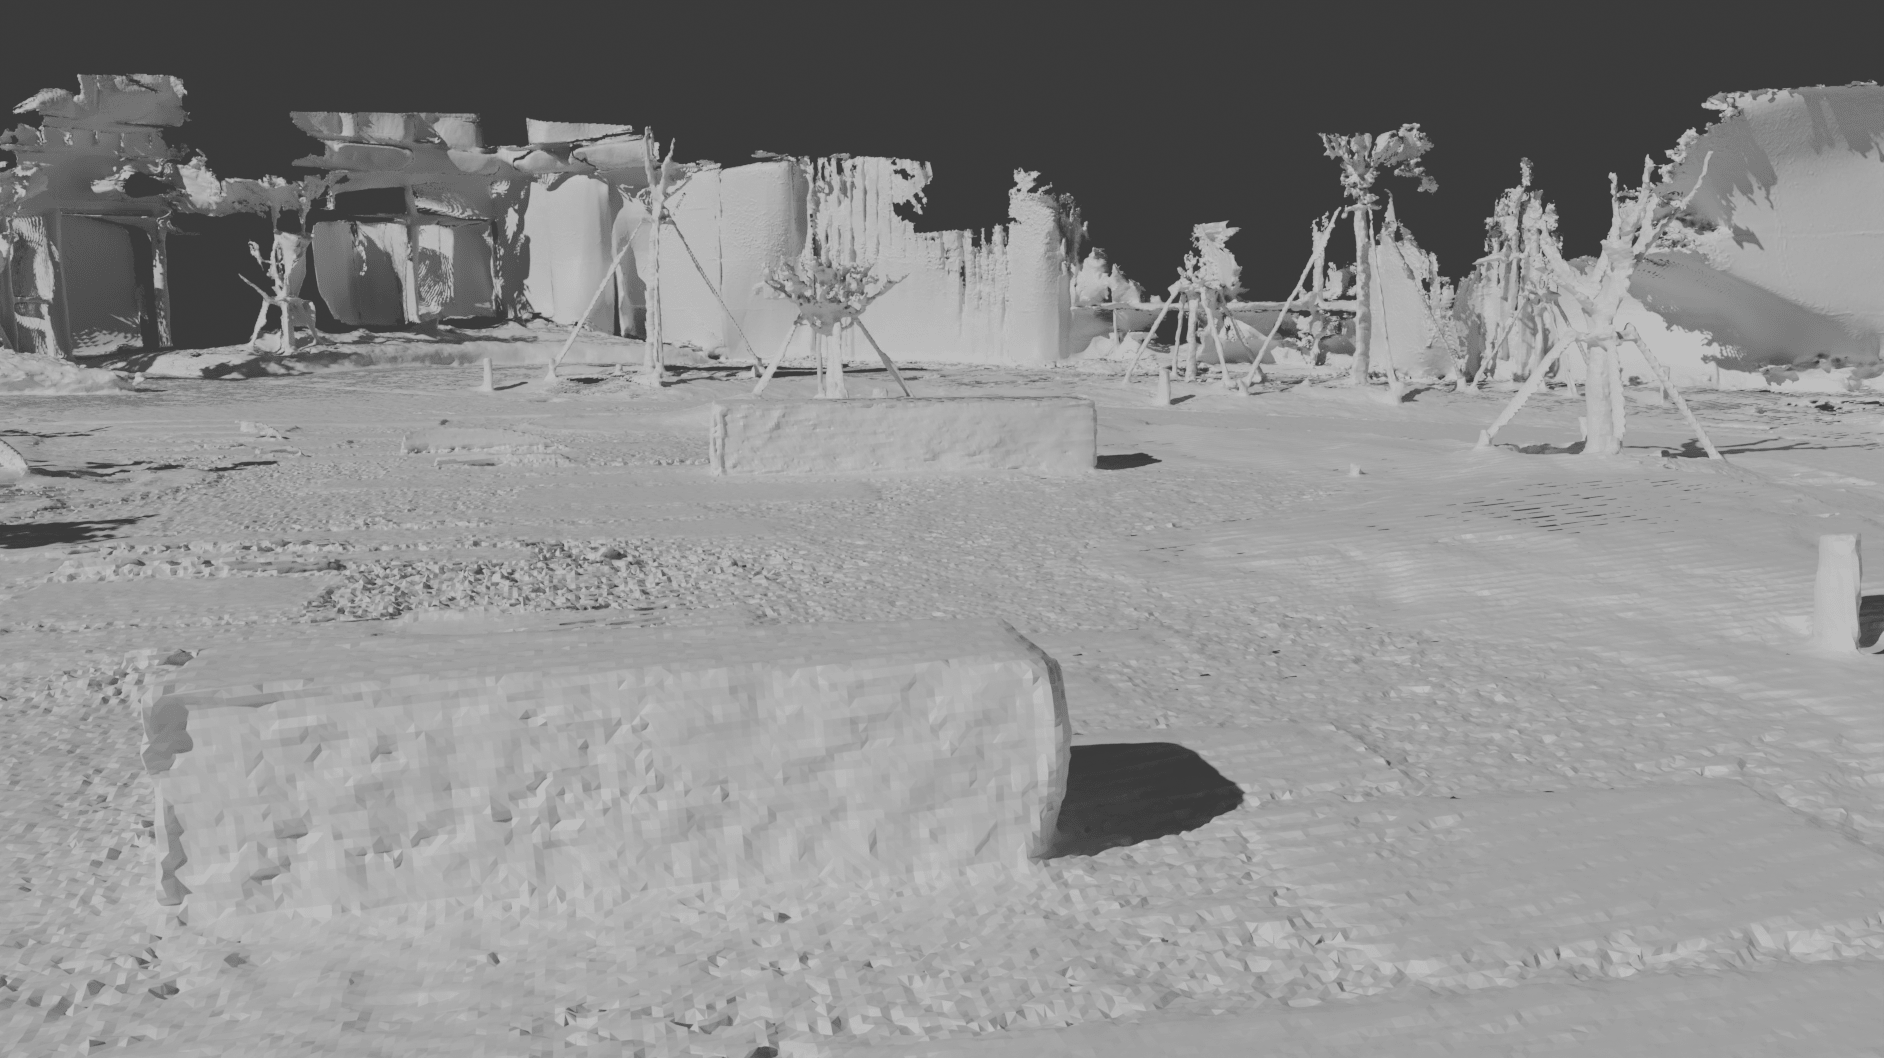} &
        \includegraphics[width=0.24\linewidth]{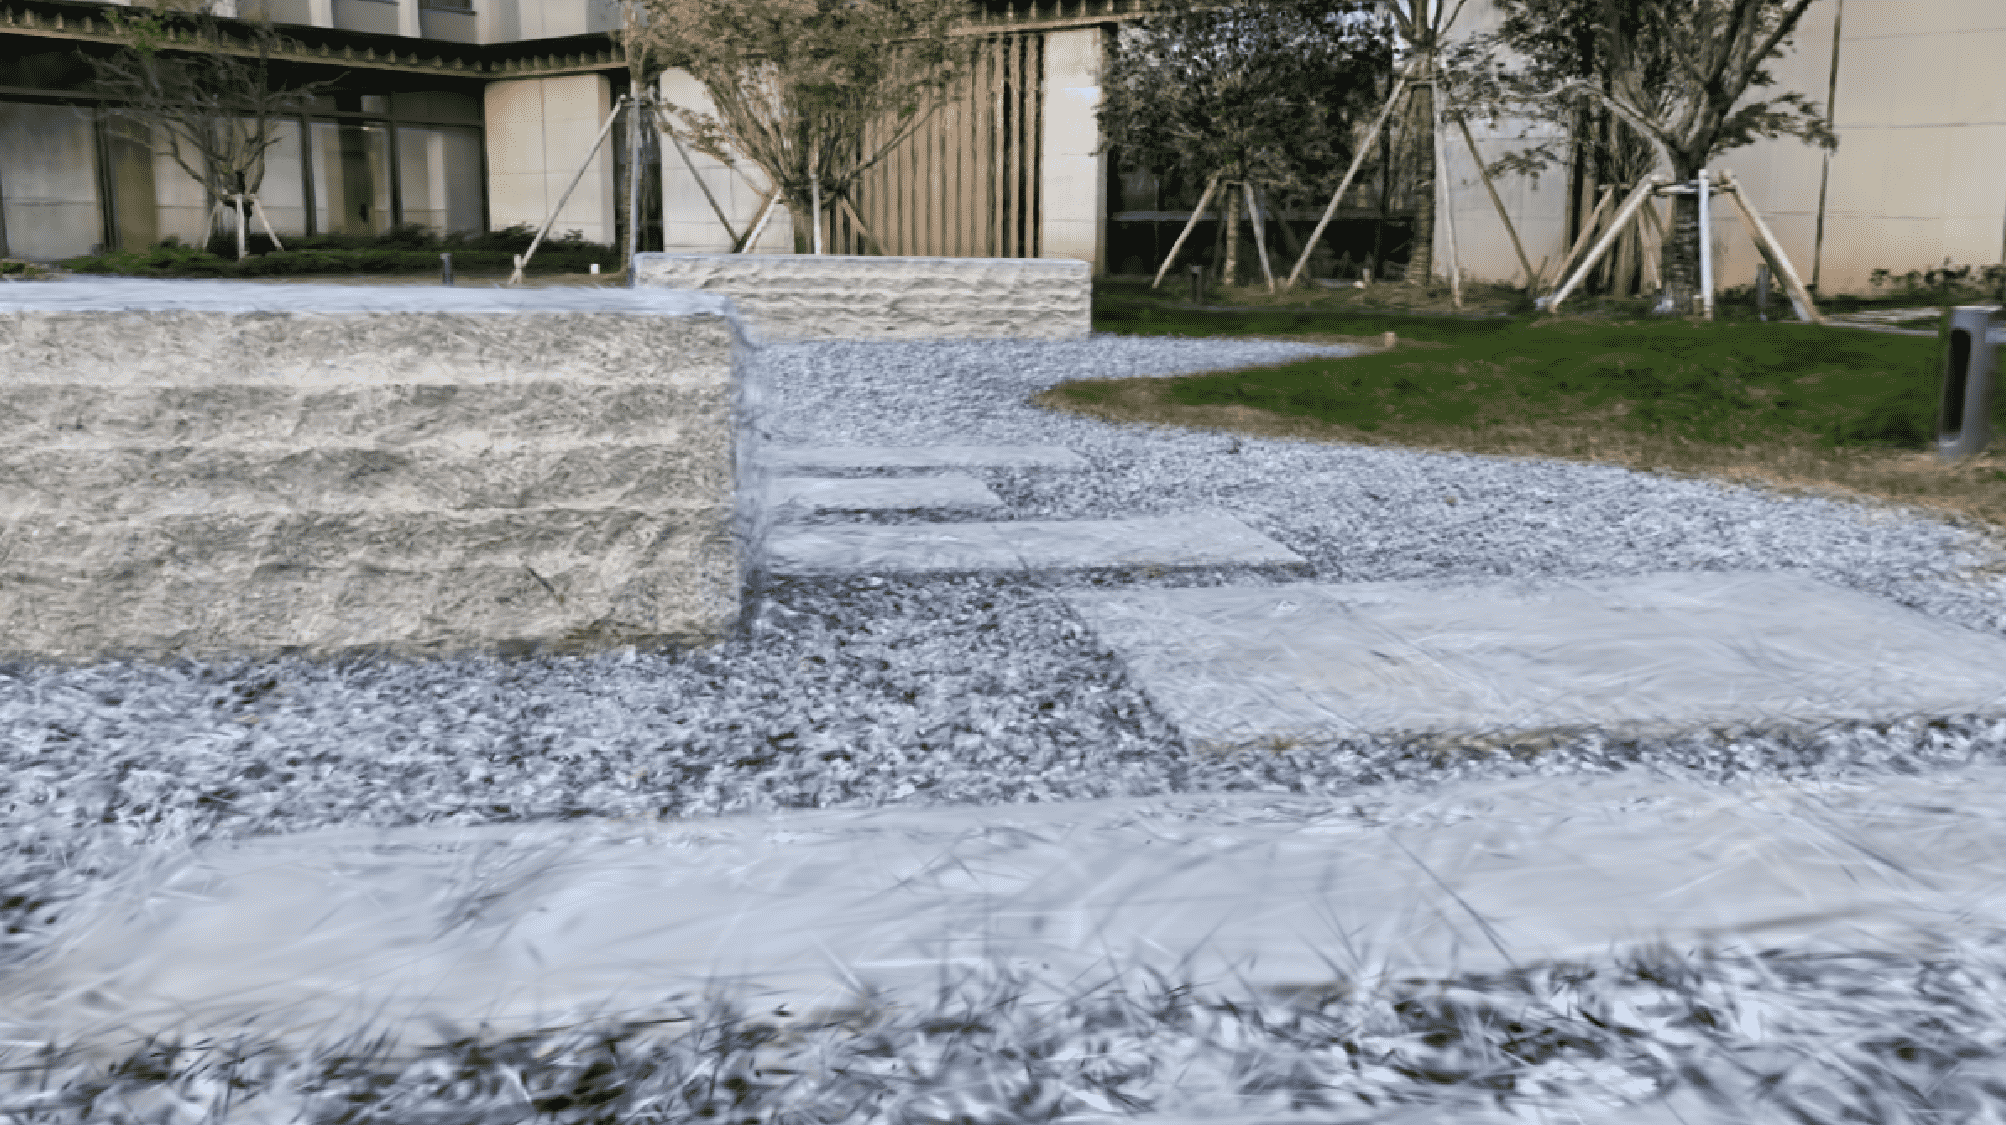} \\

        \includegraphics[width=0.24\linewidth]{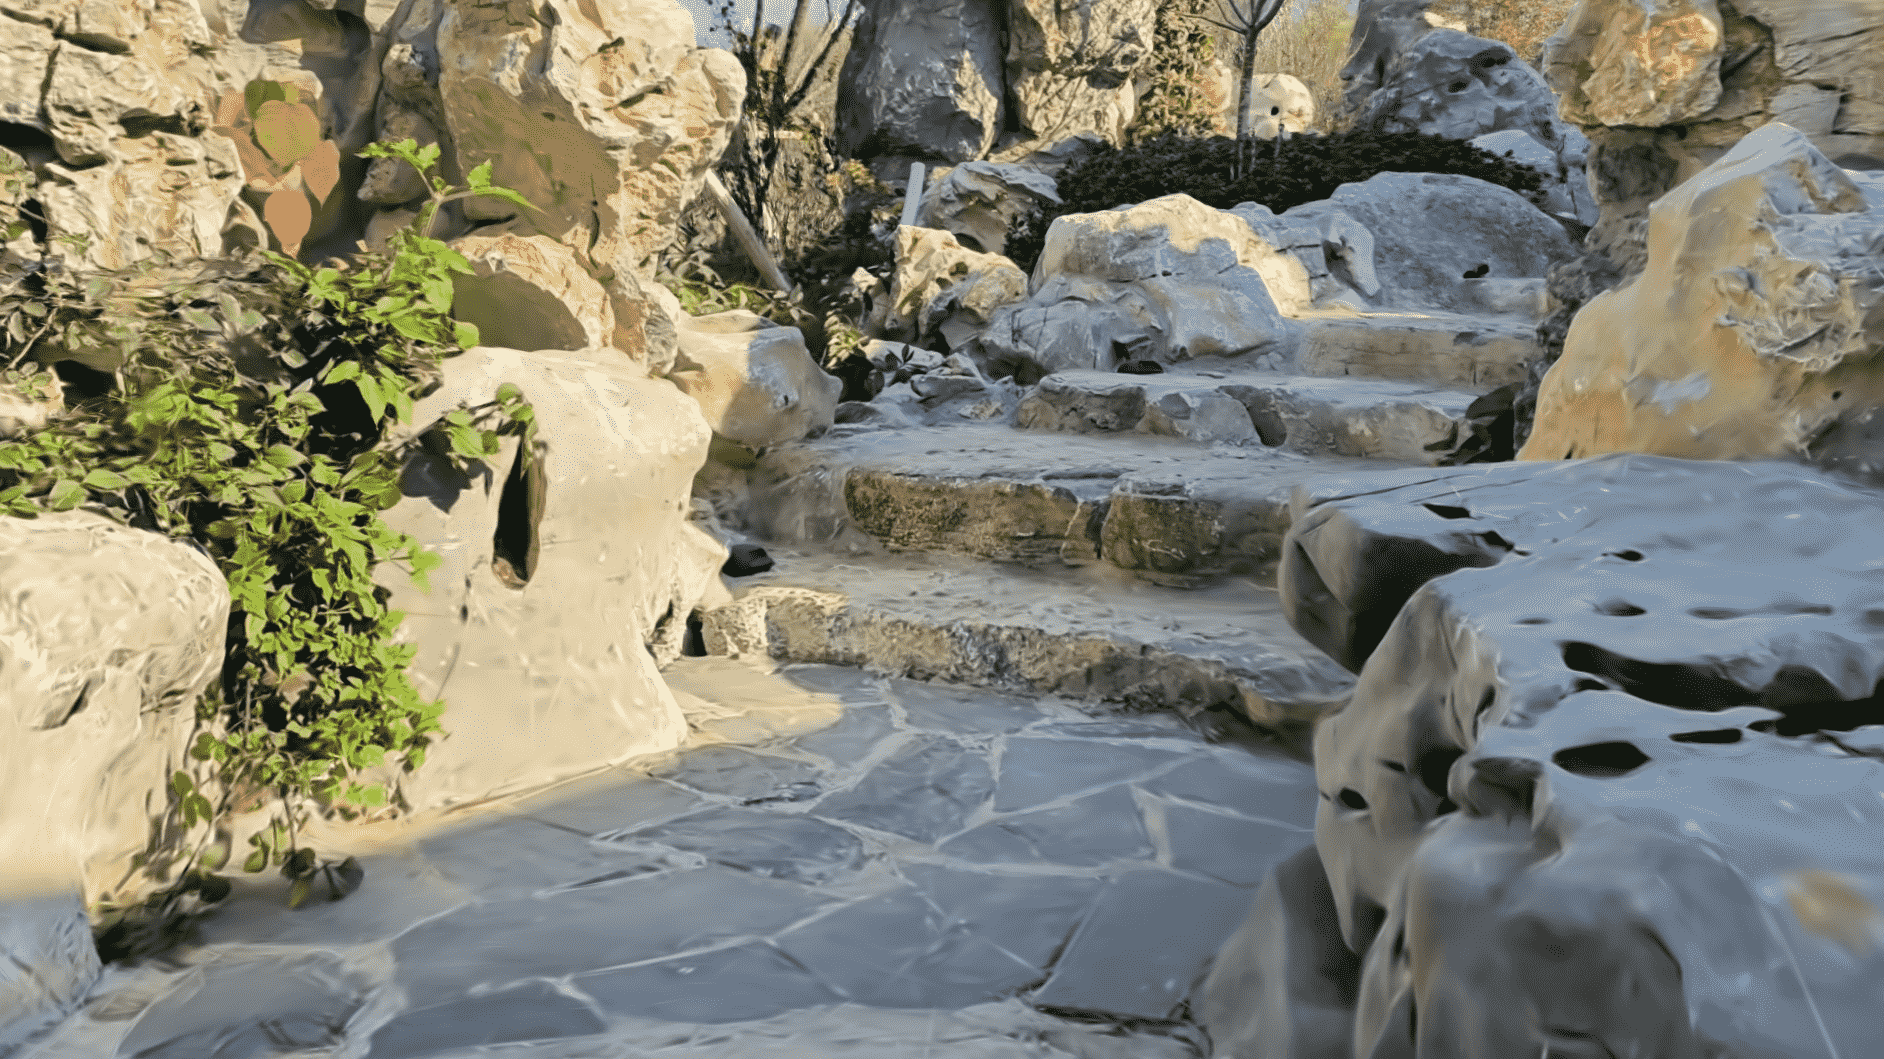} &
        \includegraphics[width=0.24\linewidth]{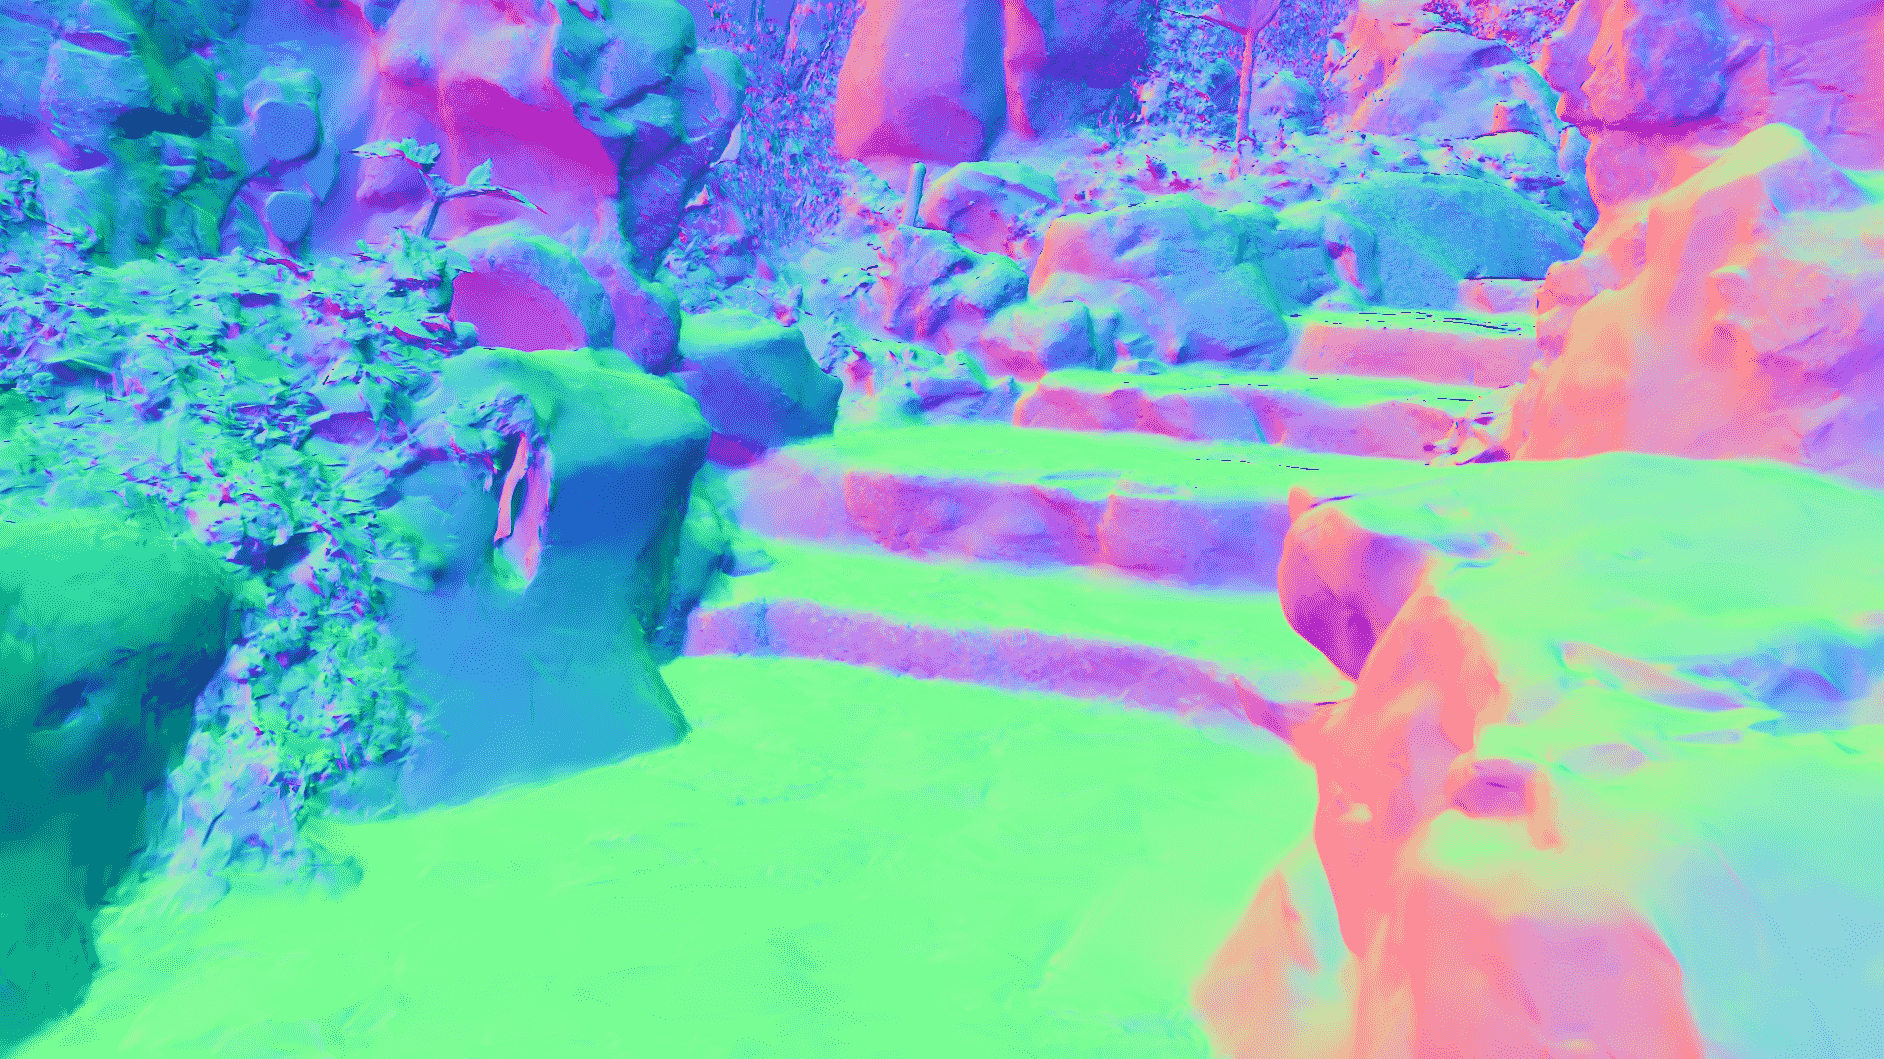} &
        \includegraphics[width=0.24\linewidth]{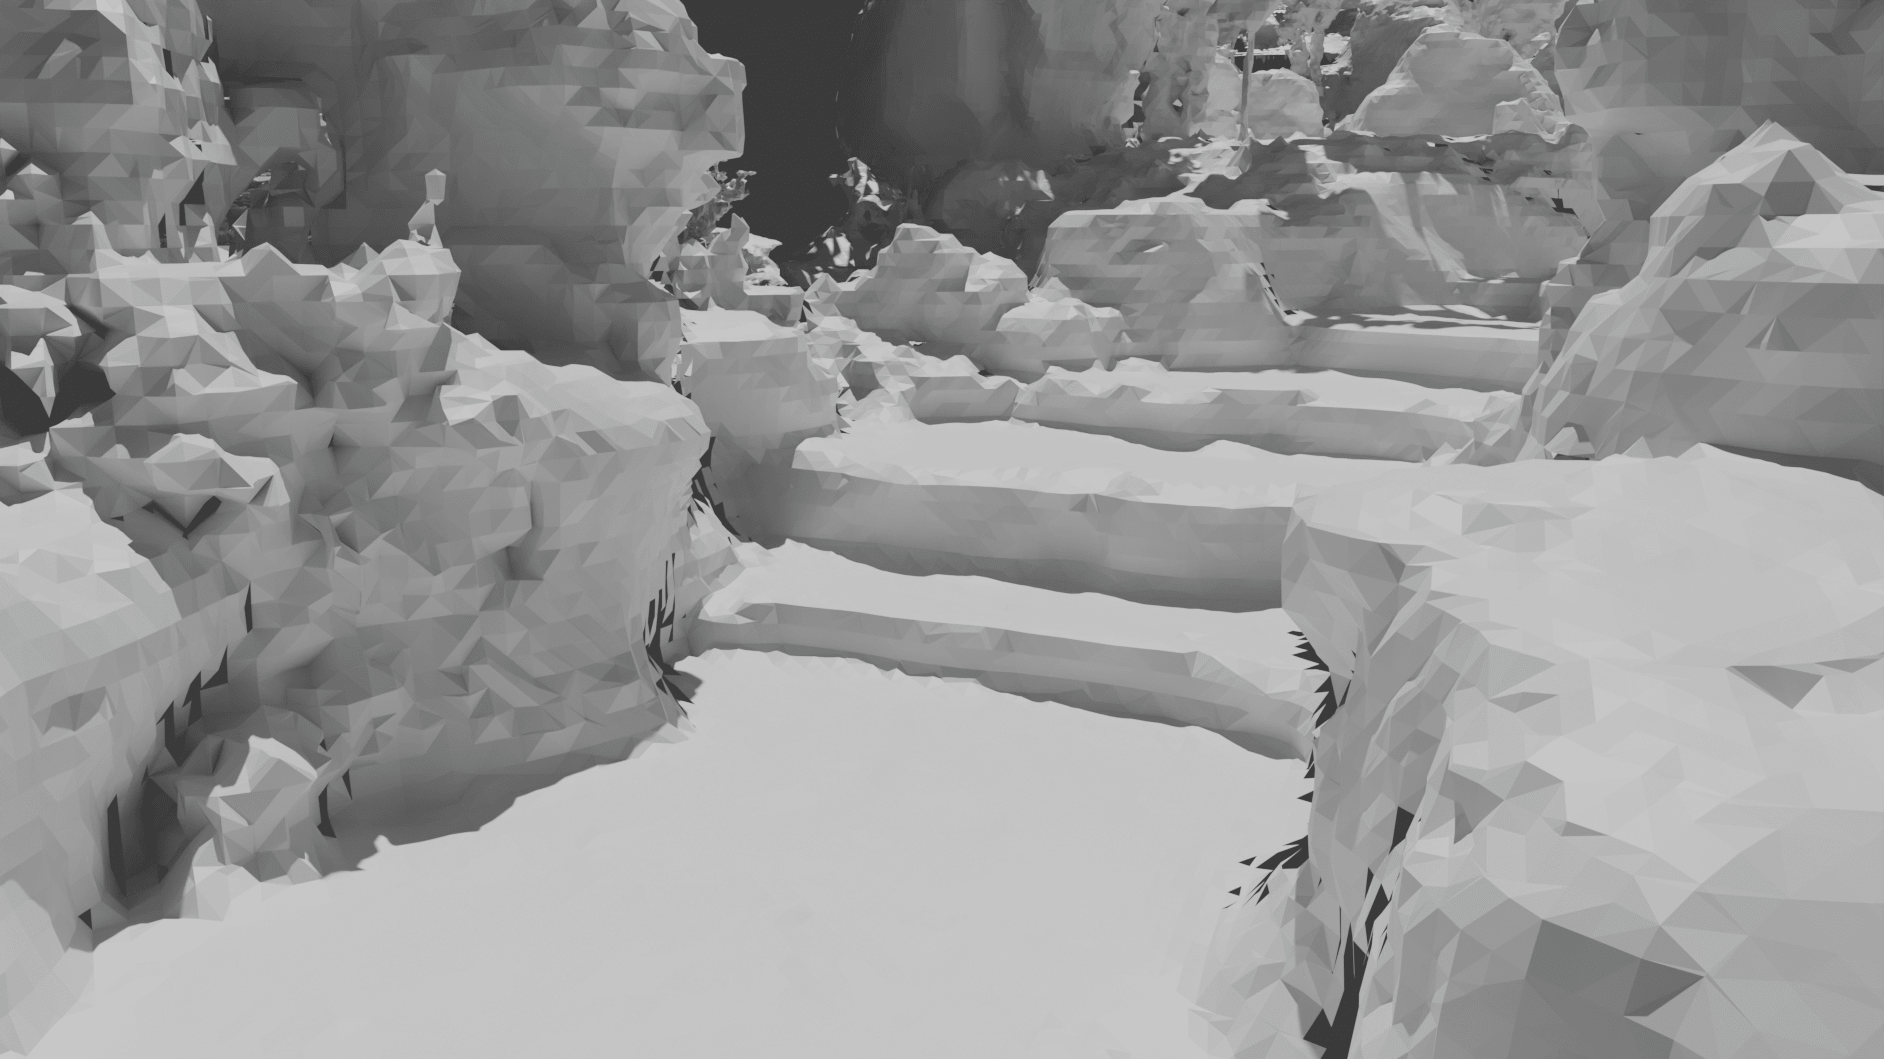} &
        \includegraphics[width=0.24\linewidth]{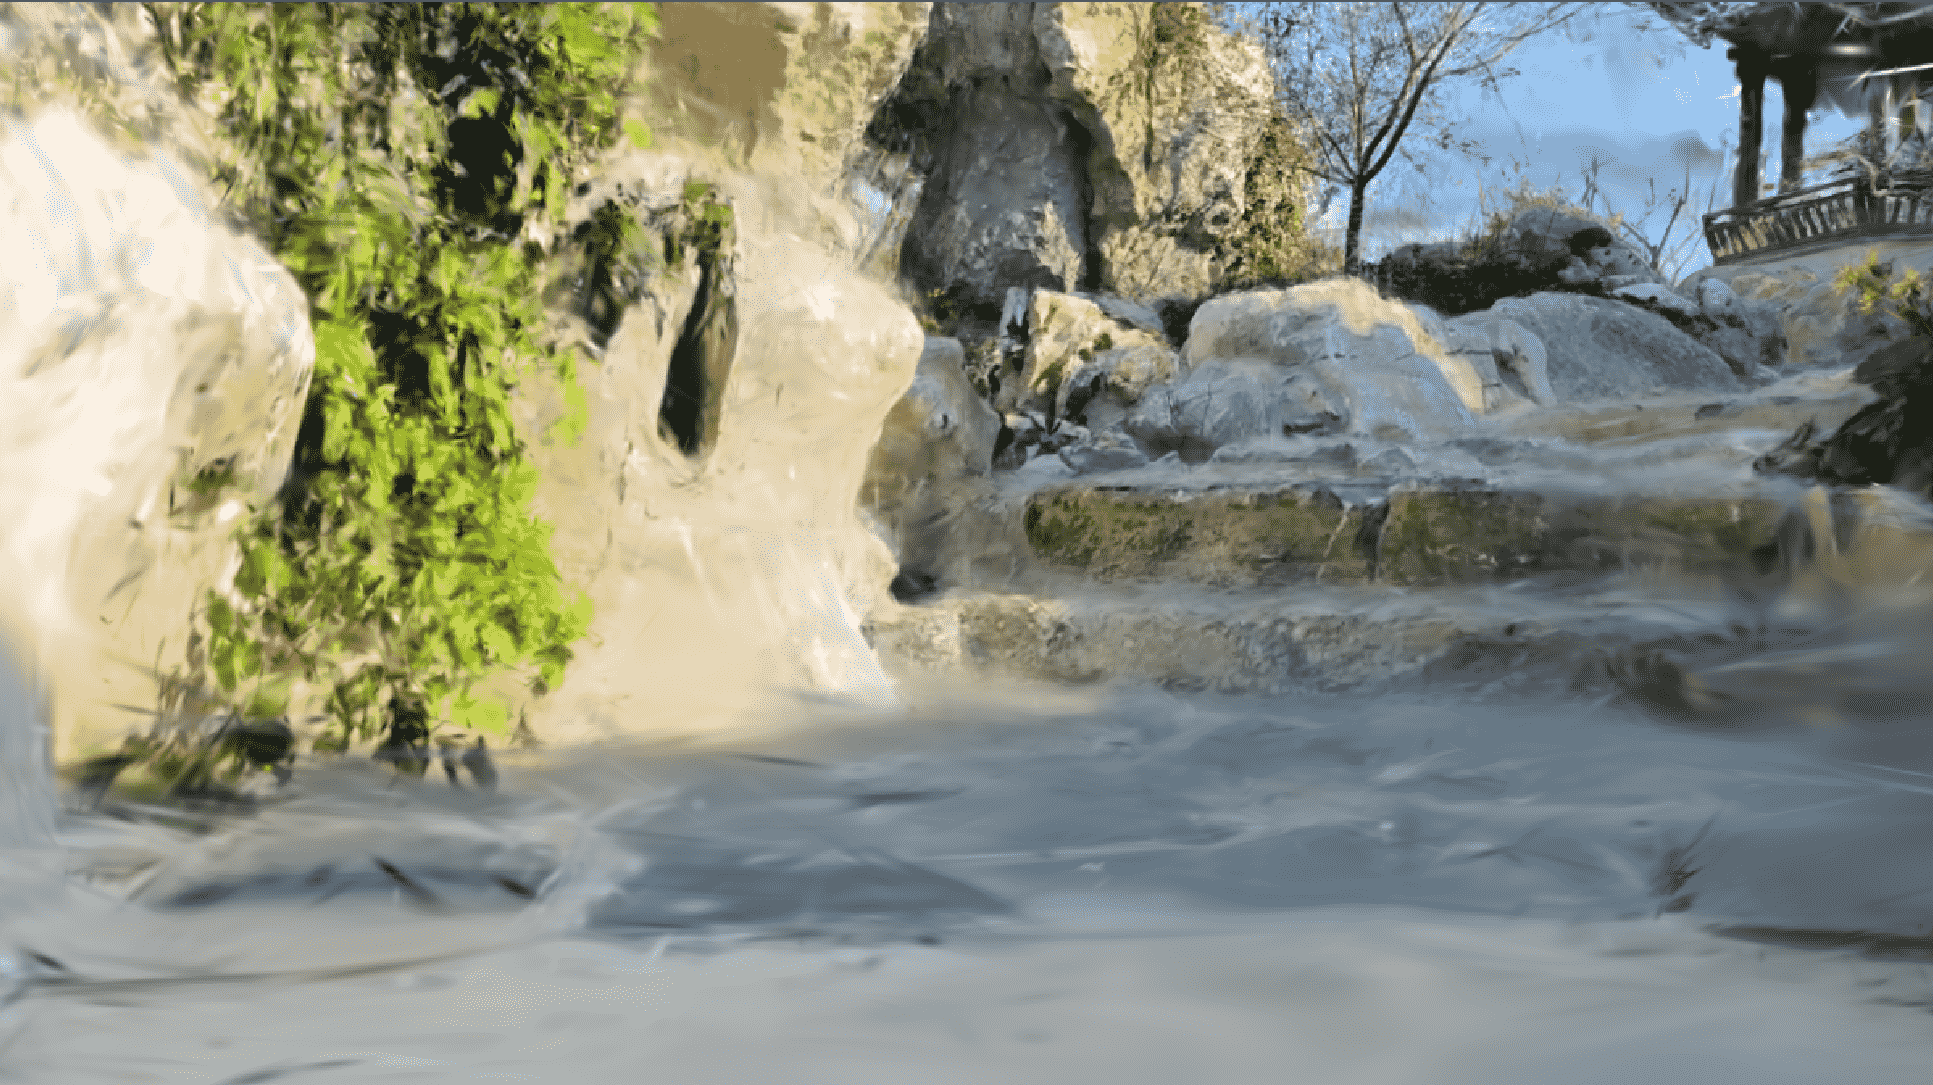} \\

        \includegraphics[width=0.24\linewidth]{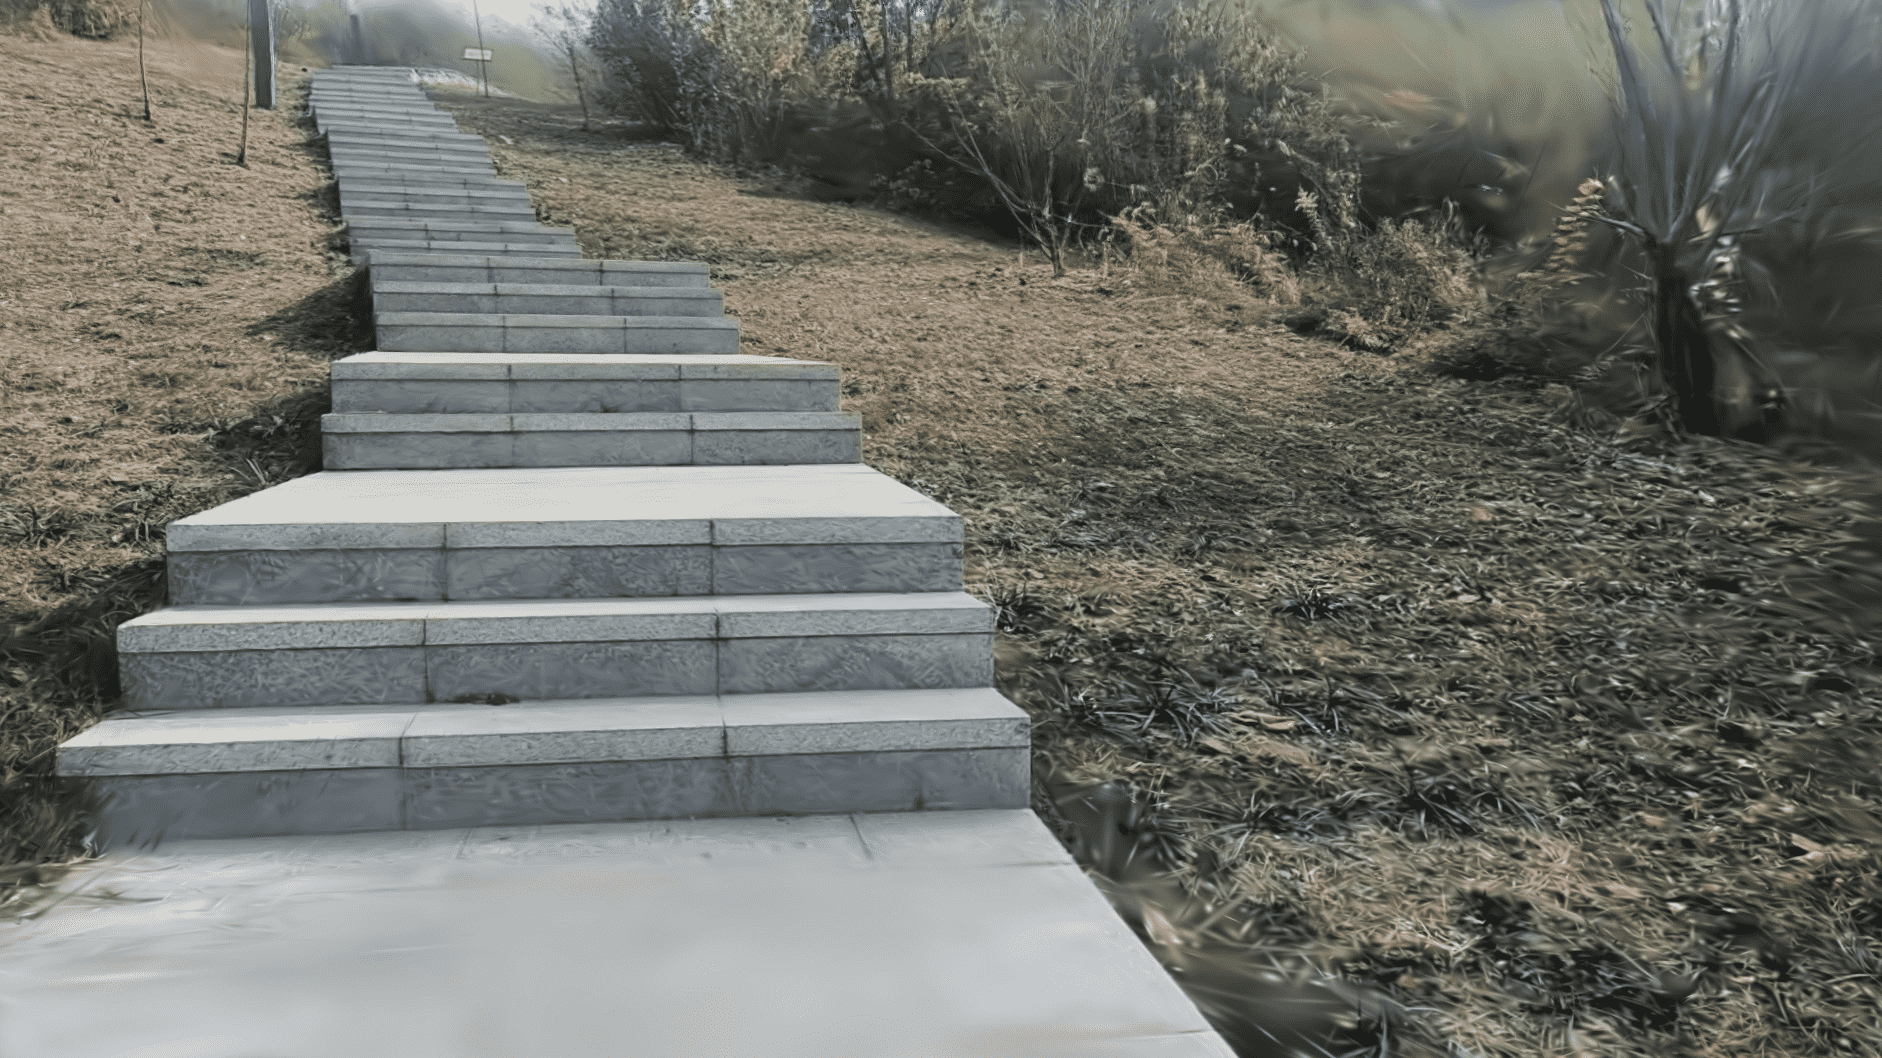} &
        \includegraphics[width=0.24\linewidth]{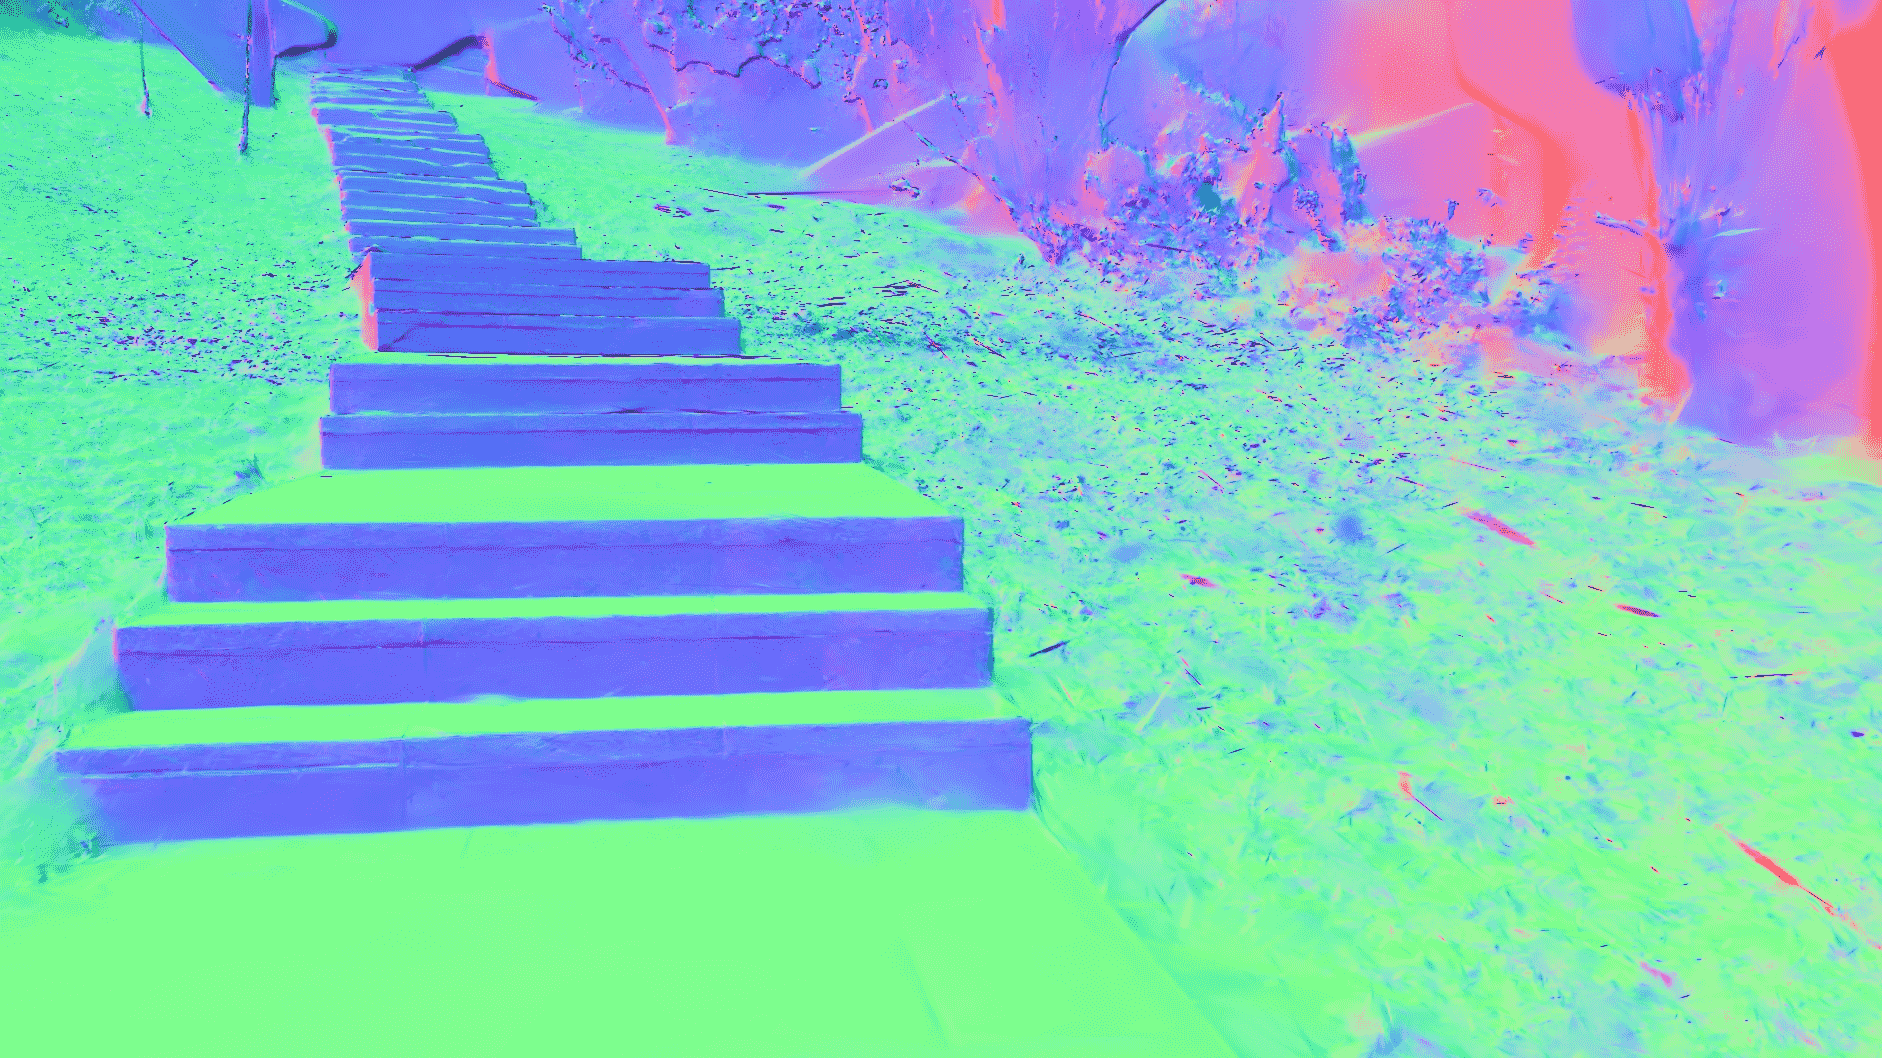} &
        \includegraphics[width=0.24\linewidth]{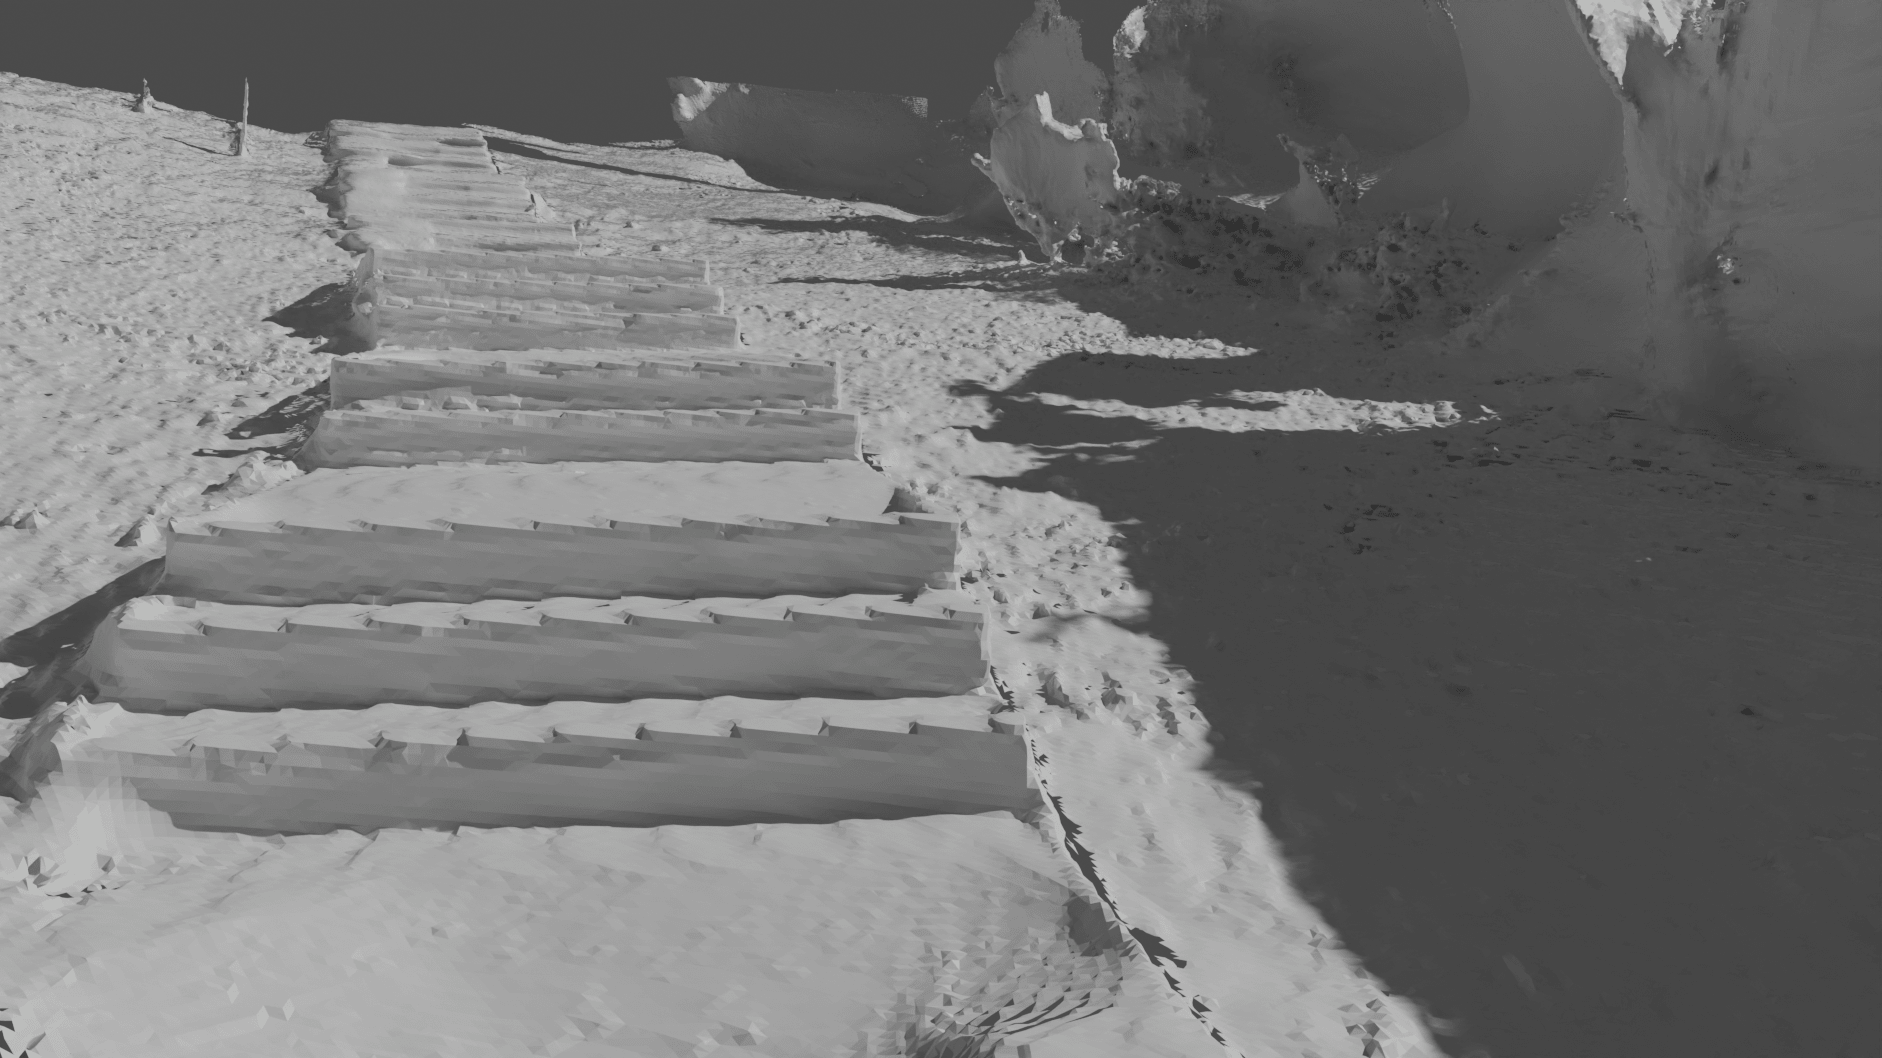} &
        \includegraphics[width=0.24\linewidth]{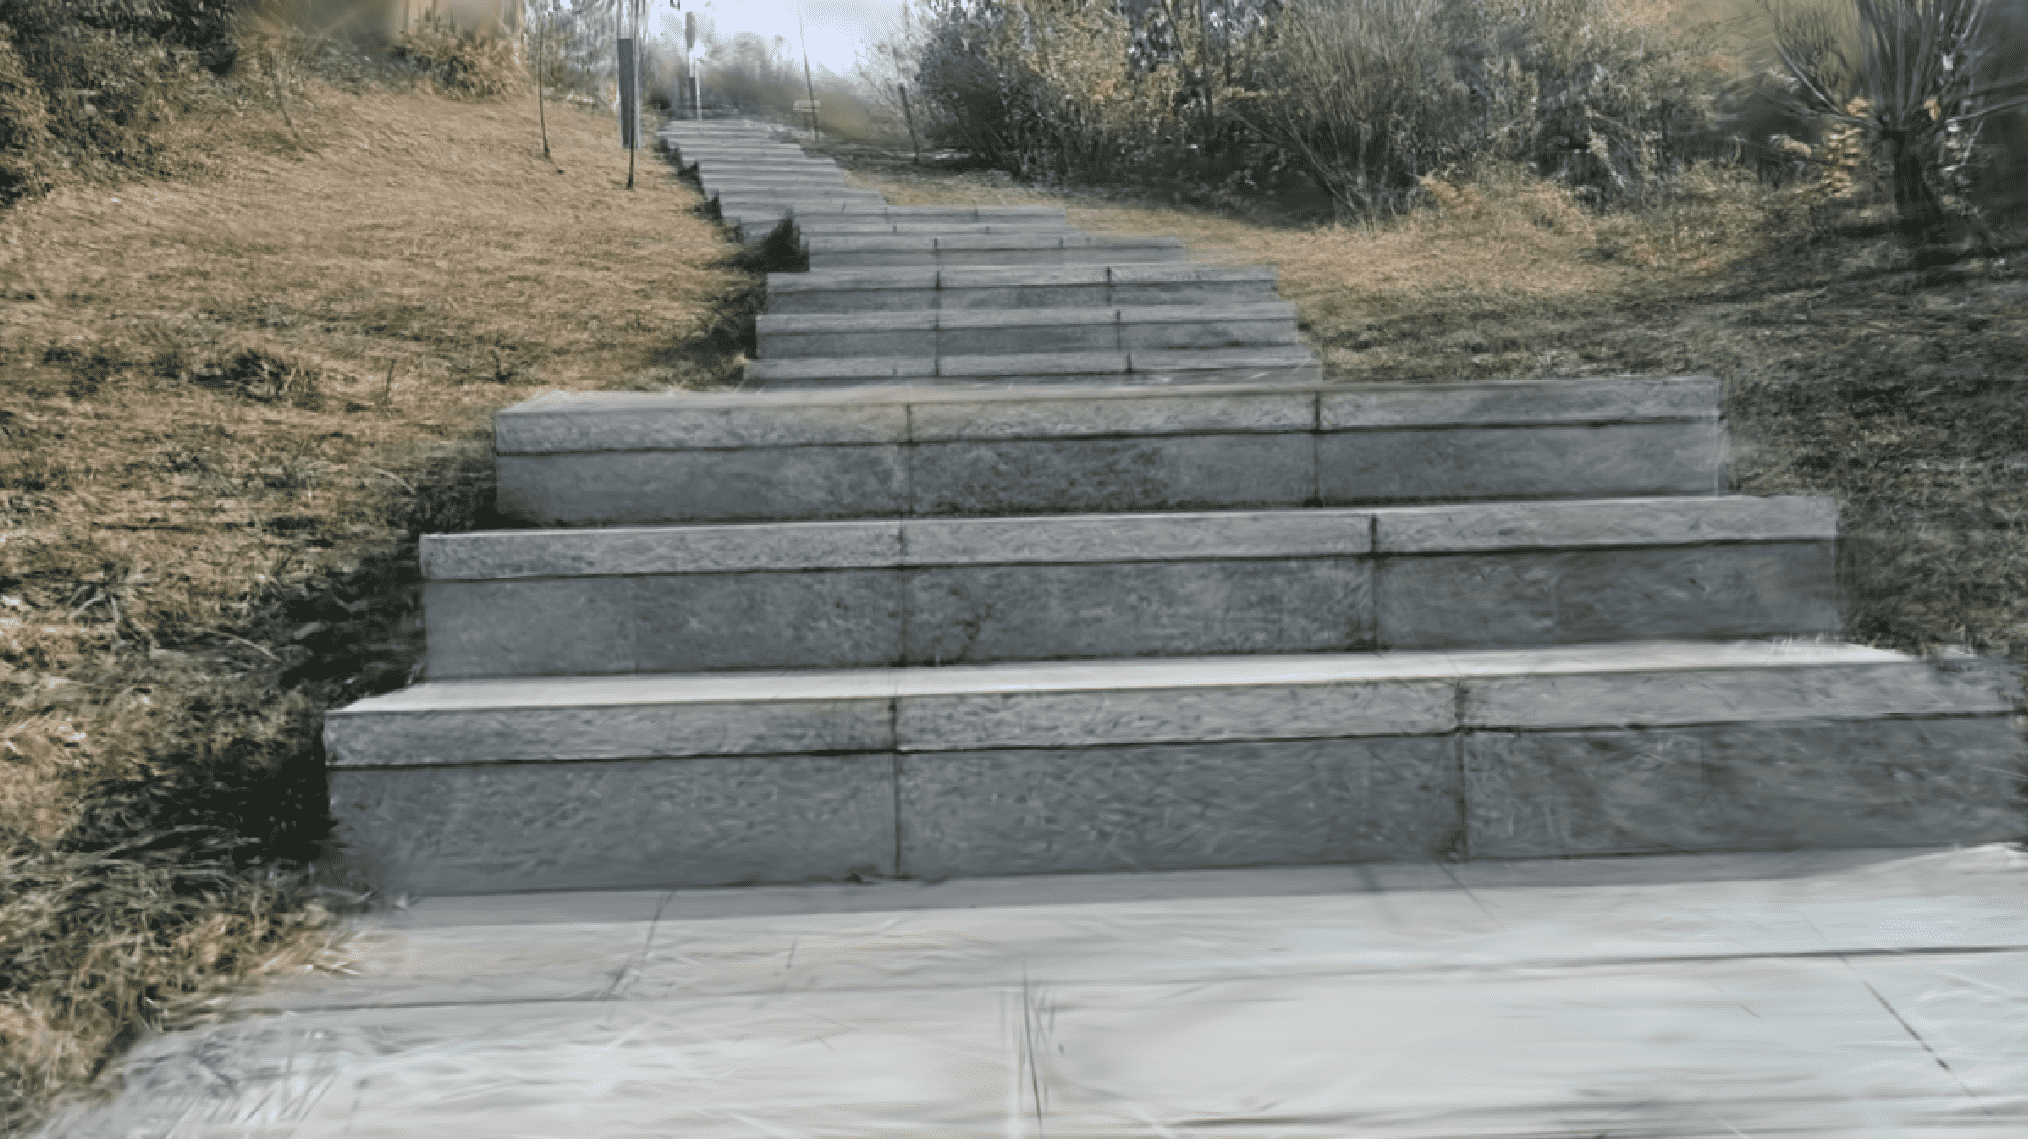} \\

        \includegraphics[width=0.24\linewidth]{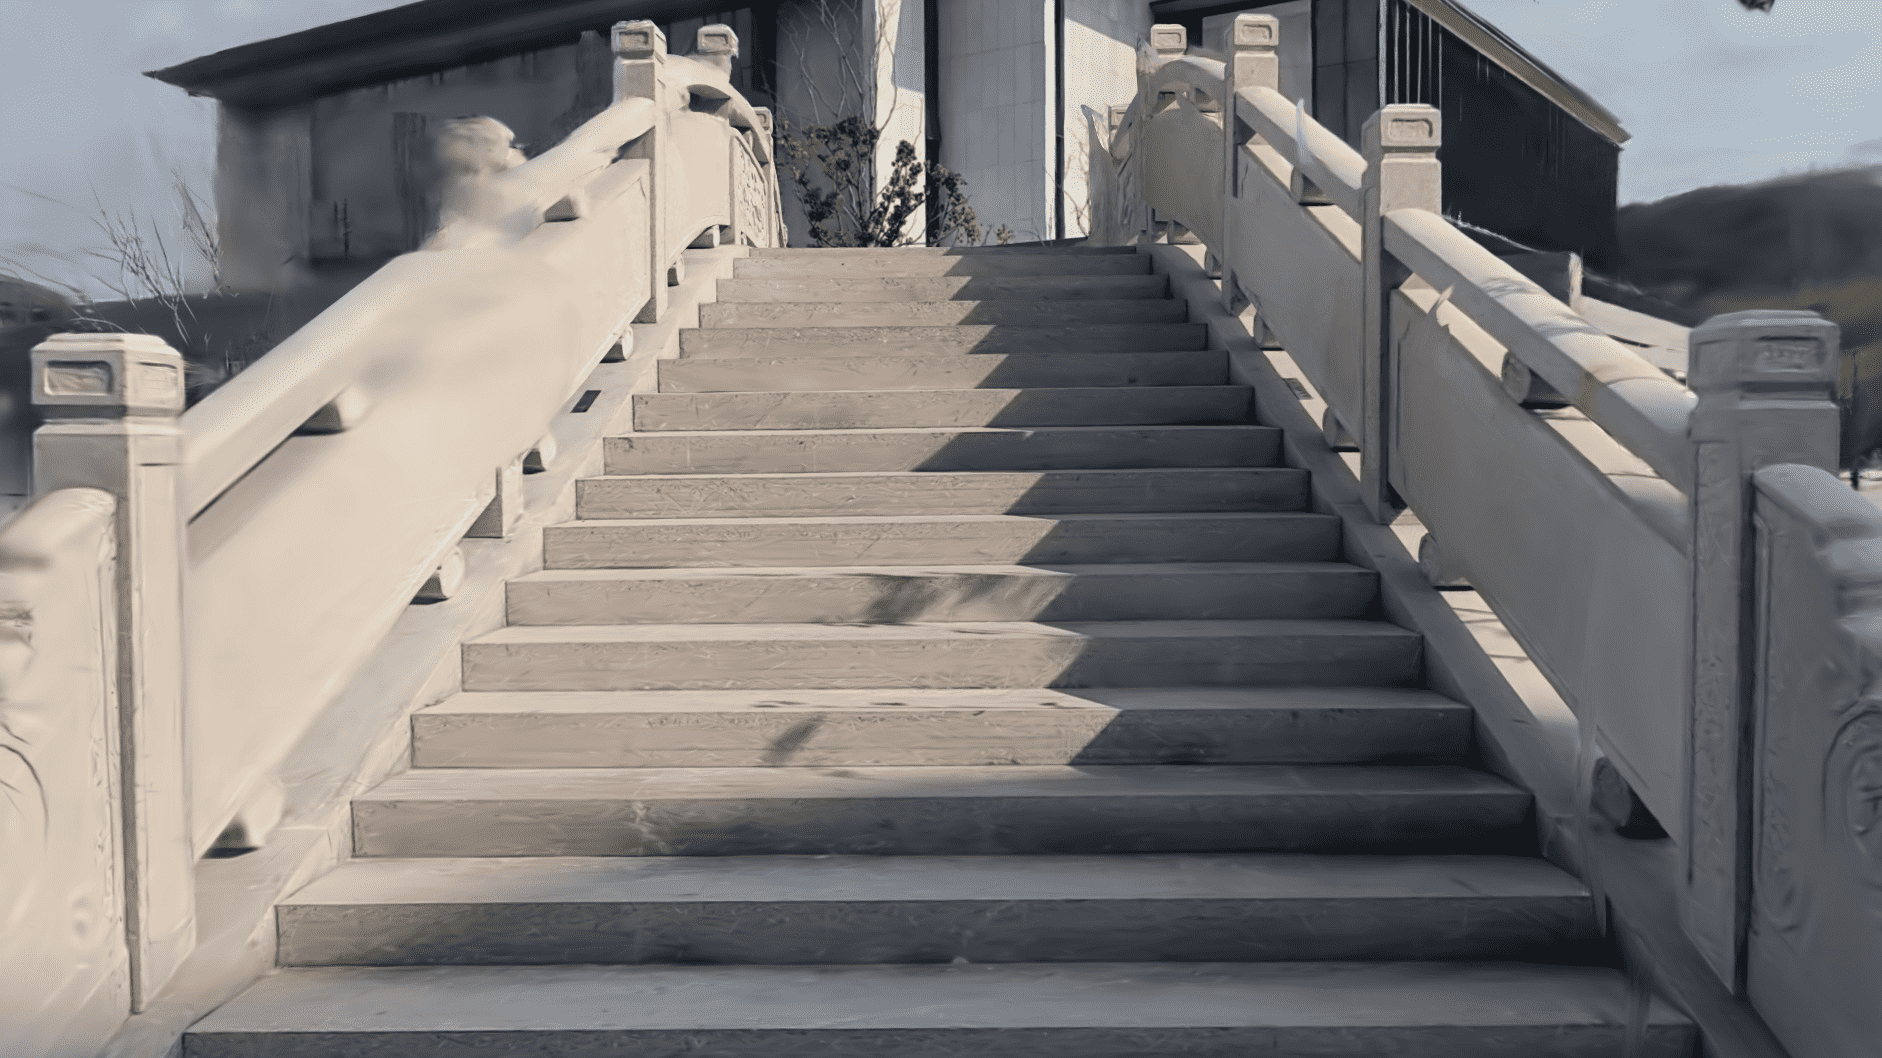} &
        \includegraphics[width=0.24\linewidth]{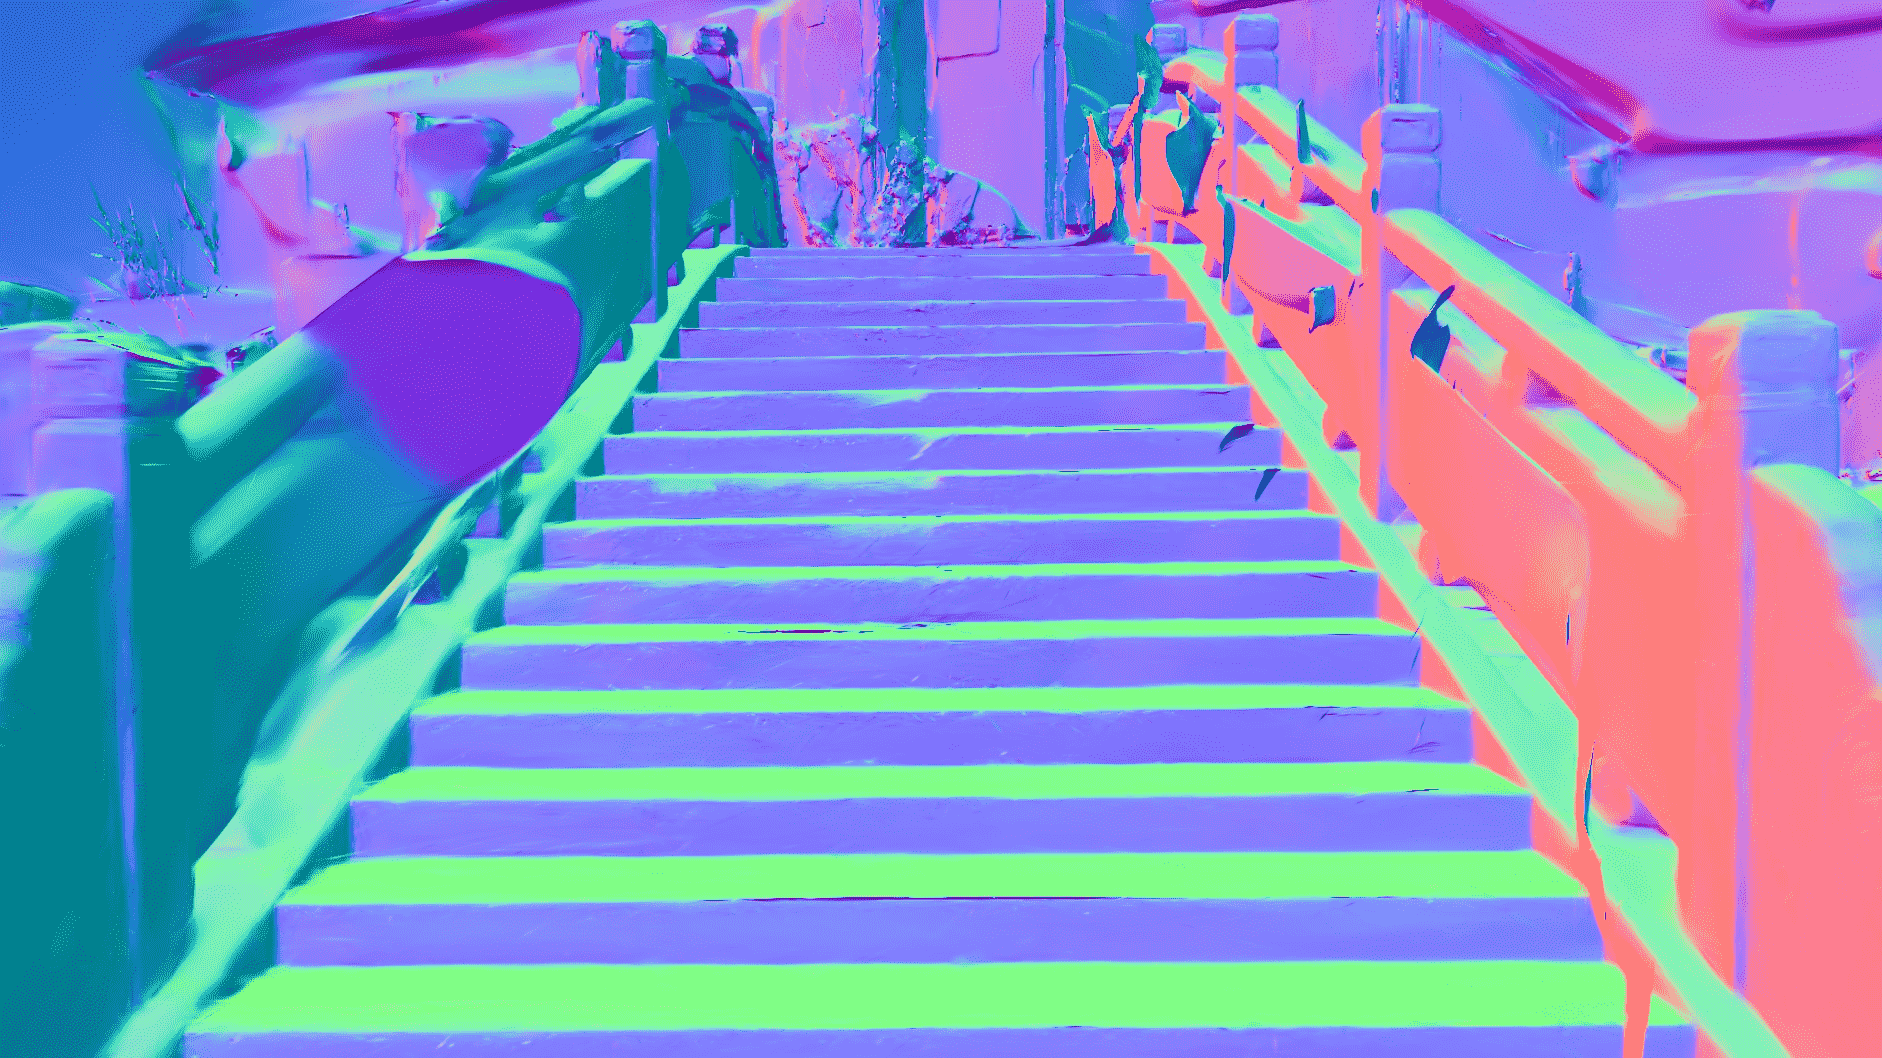} &
        \includegraphics[width=0.24\linewidth]{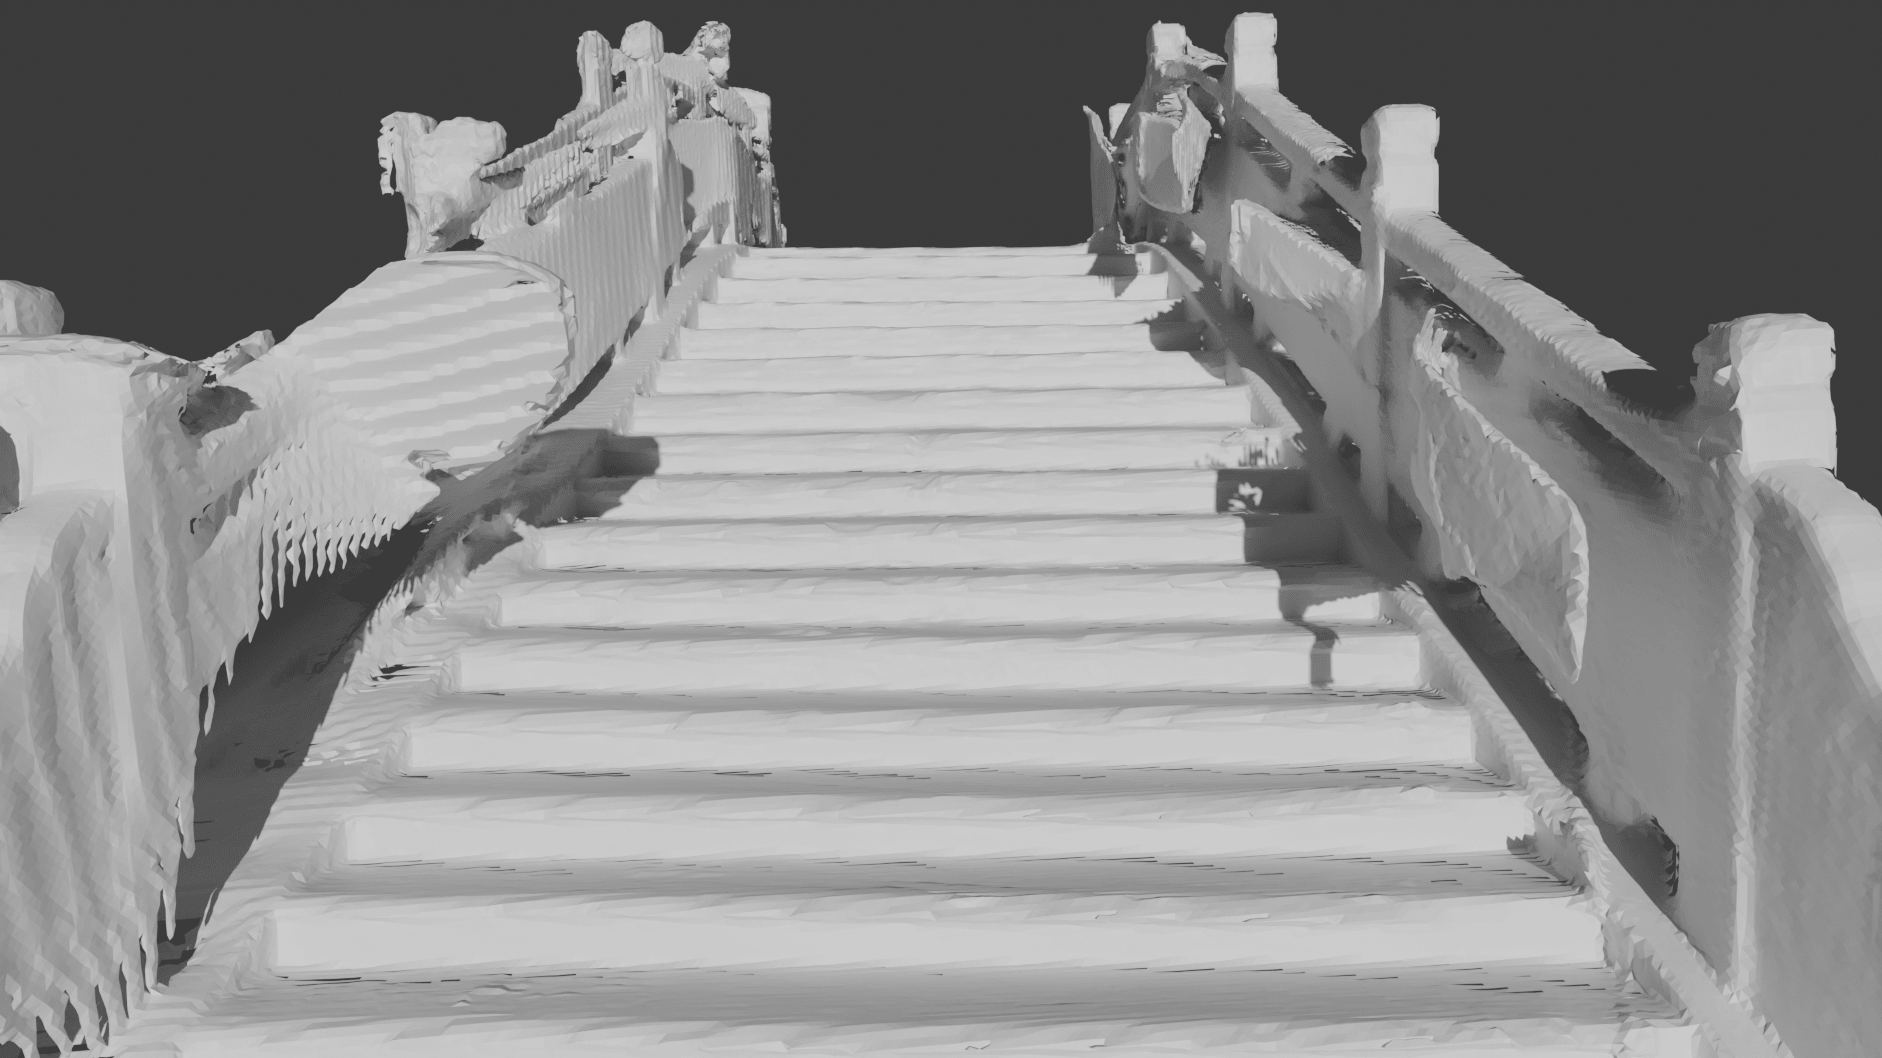} &
        \includegraphics[width=0.24\linewidth]{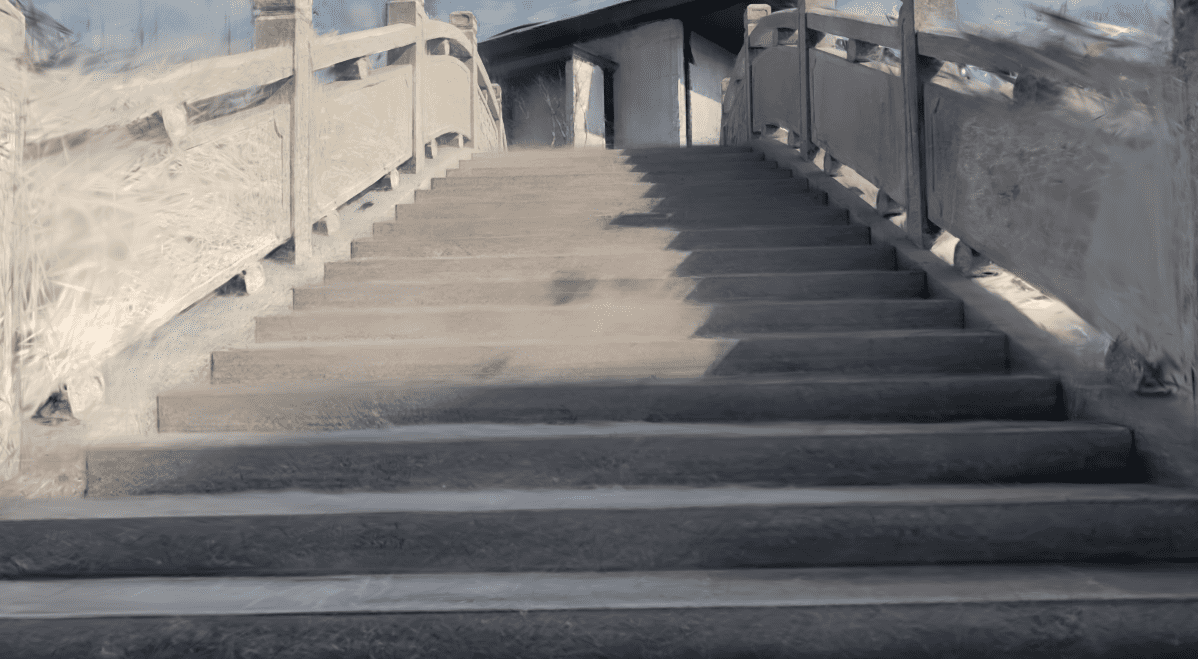} \\

        \includegraphics[width=0.24\linewidth]{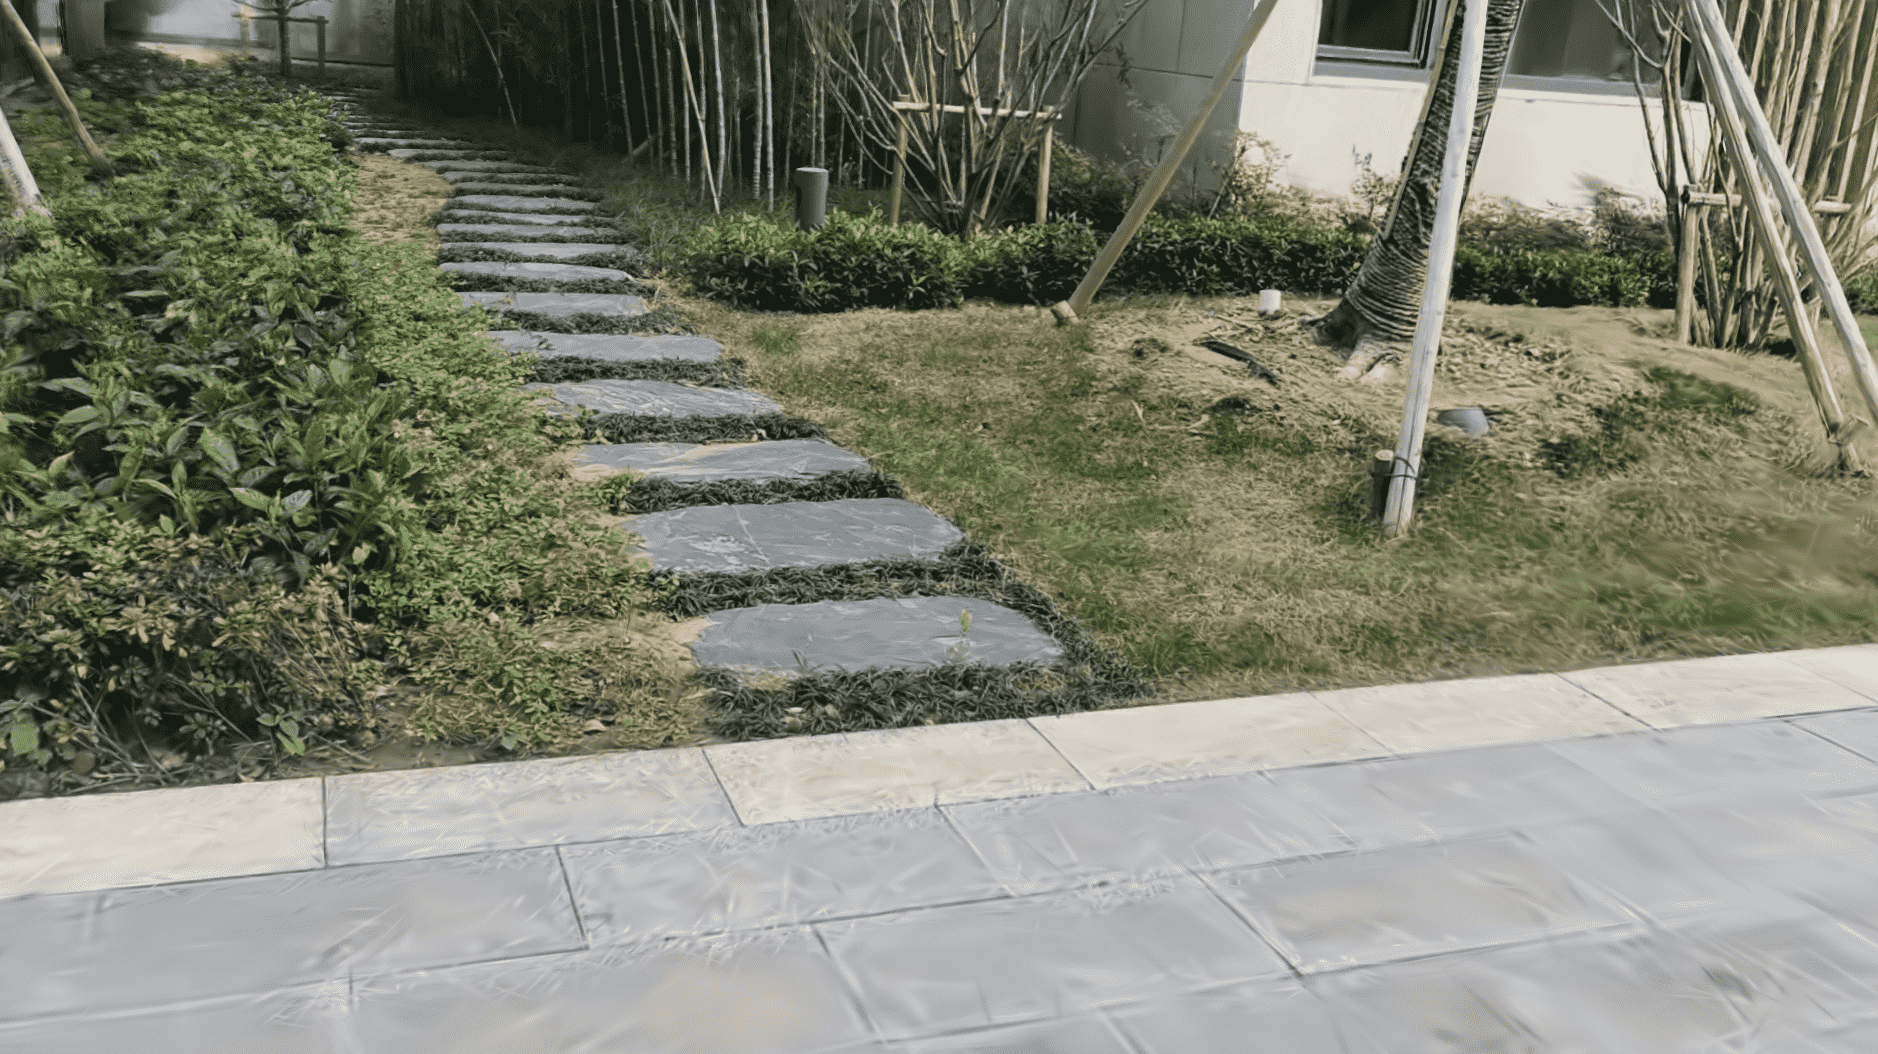} &
        \includegraphics[width=0.24\linewidth]{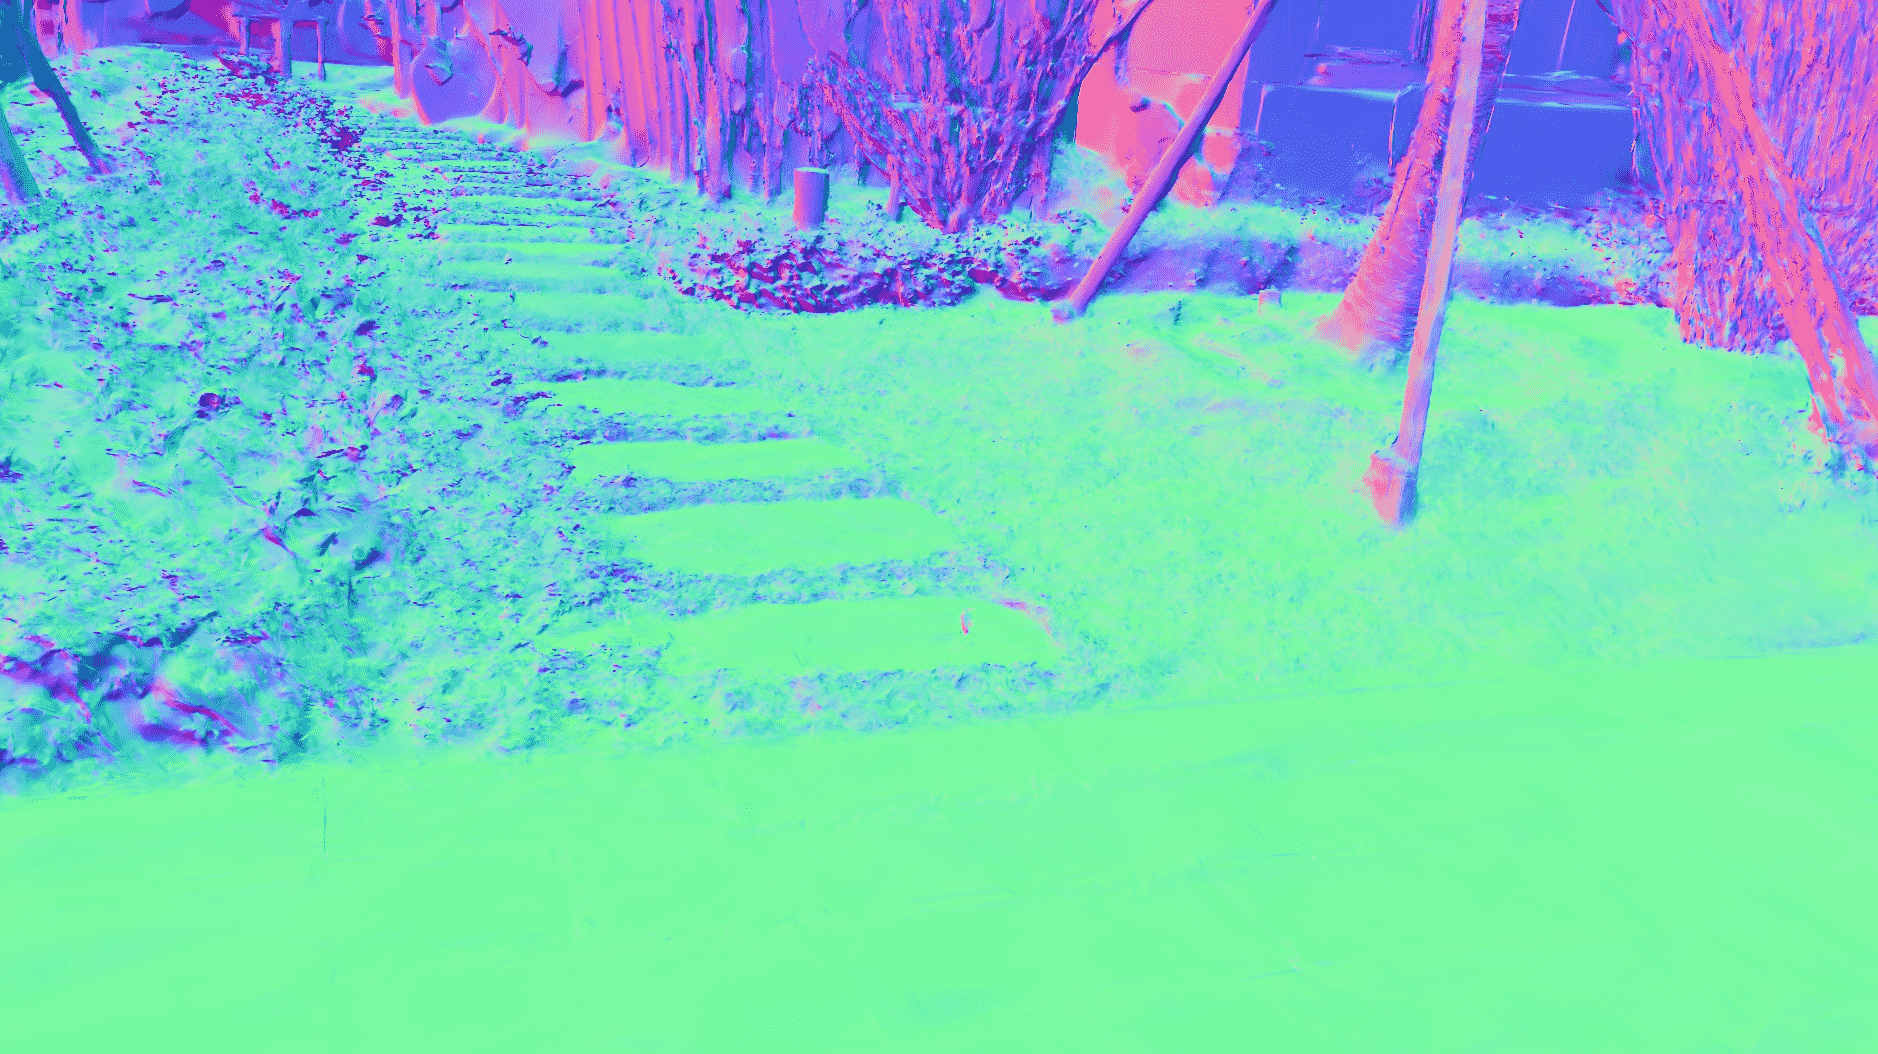} &
        \includegraphics[width=0.24\linewidth]{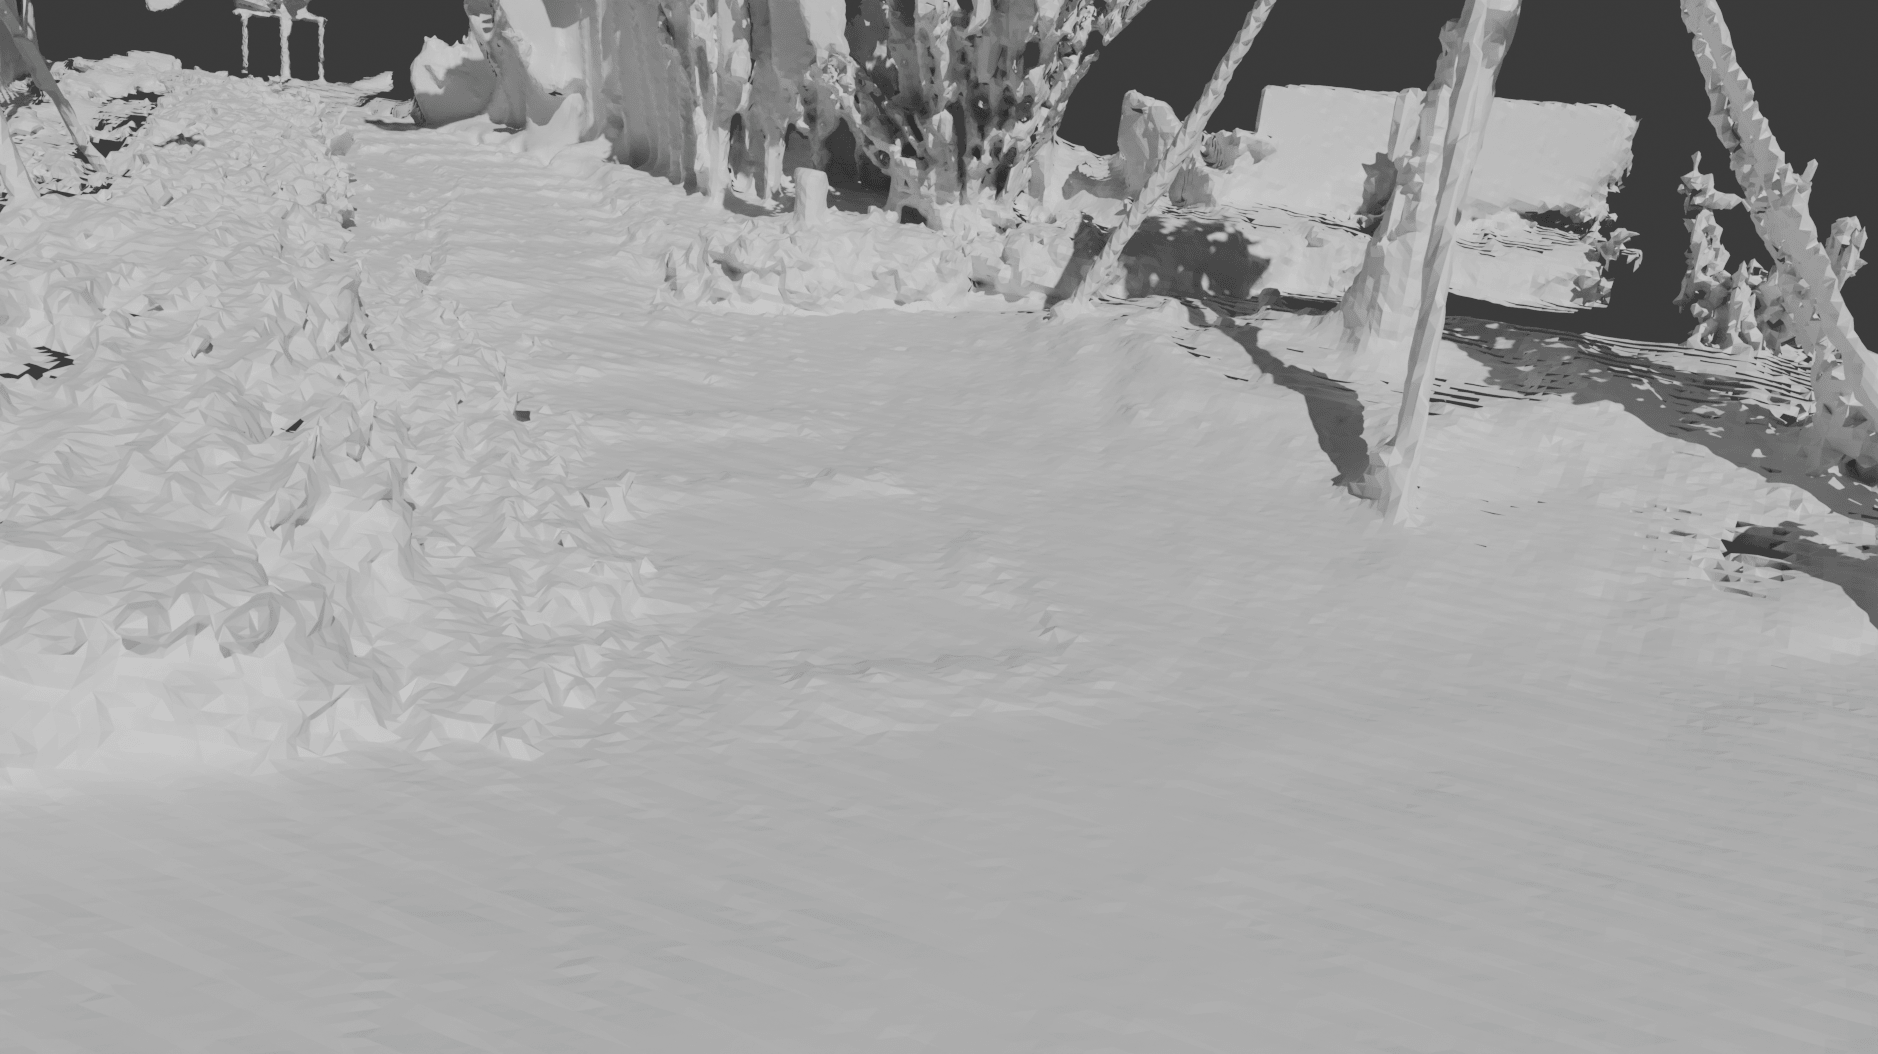} &
        \includegraphics[width=0.24\linewidth]{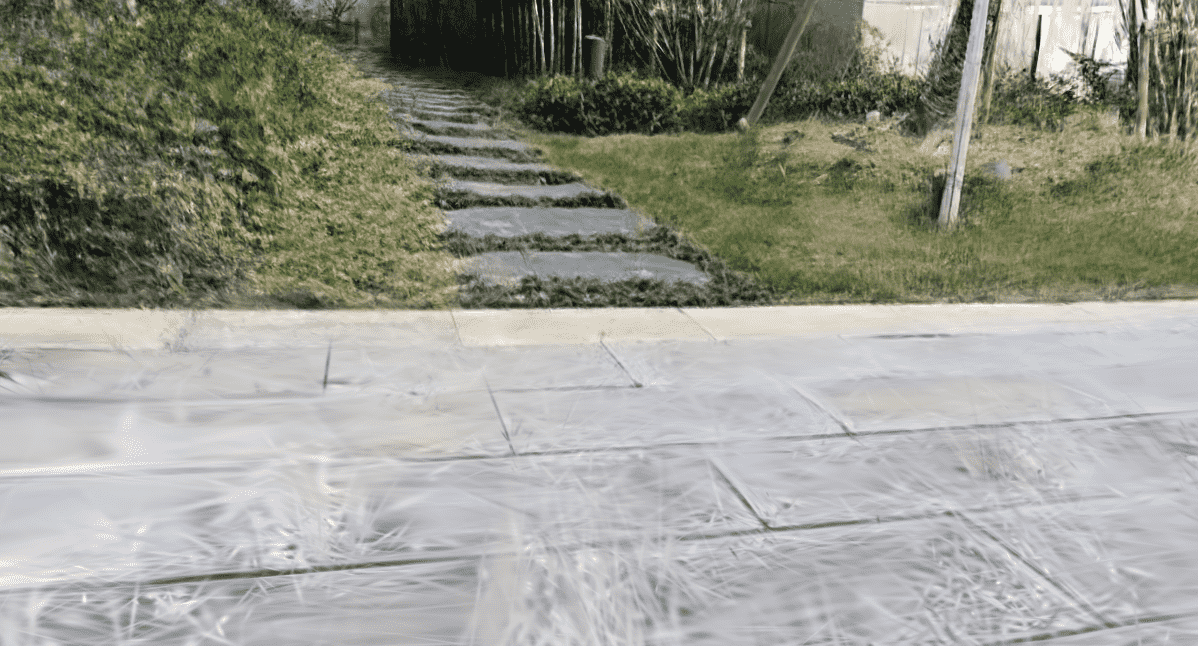} \\

        \includegraphics[width=0.24\linewidth]{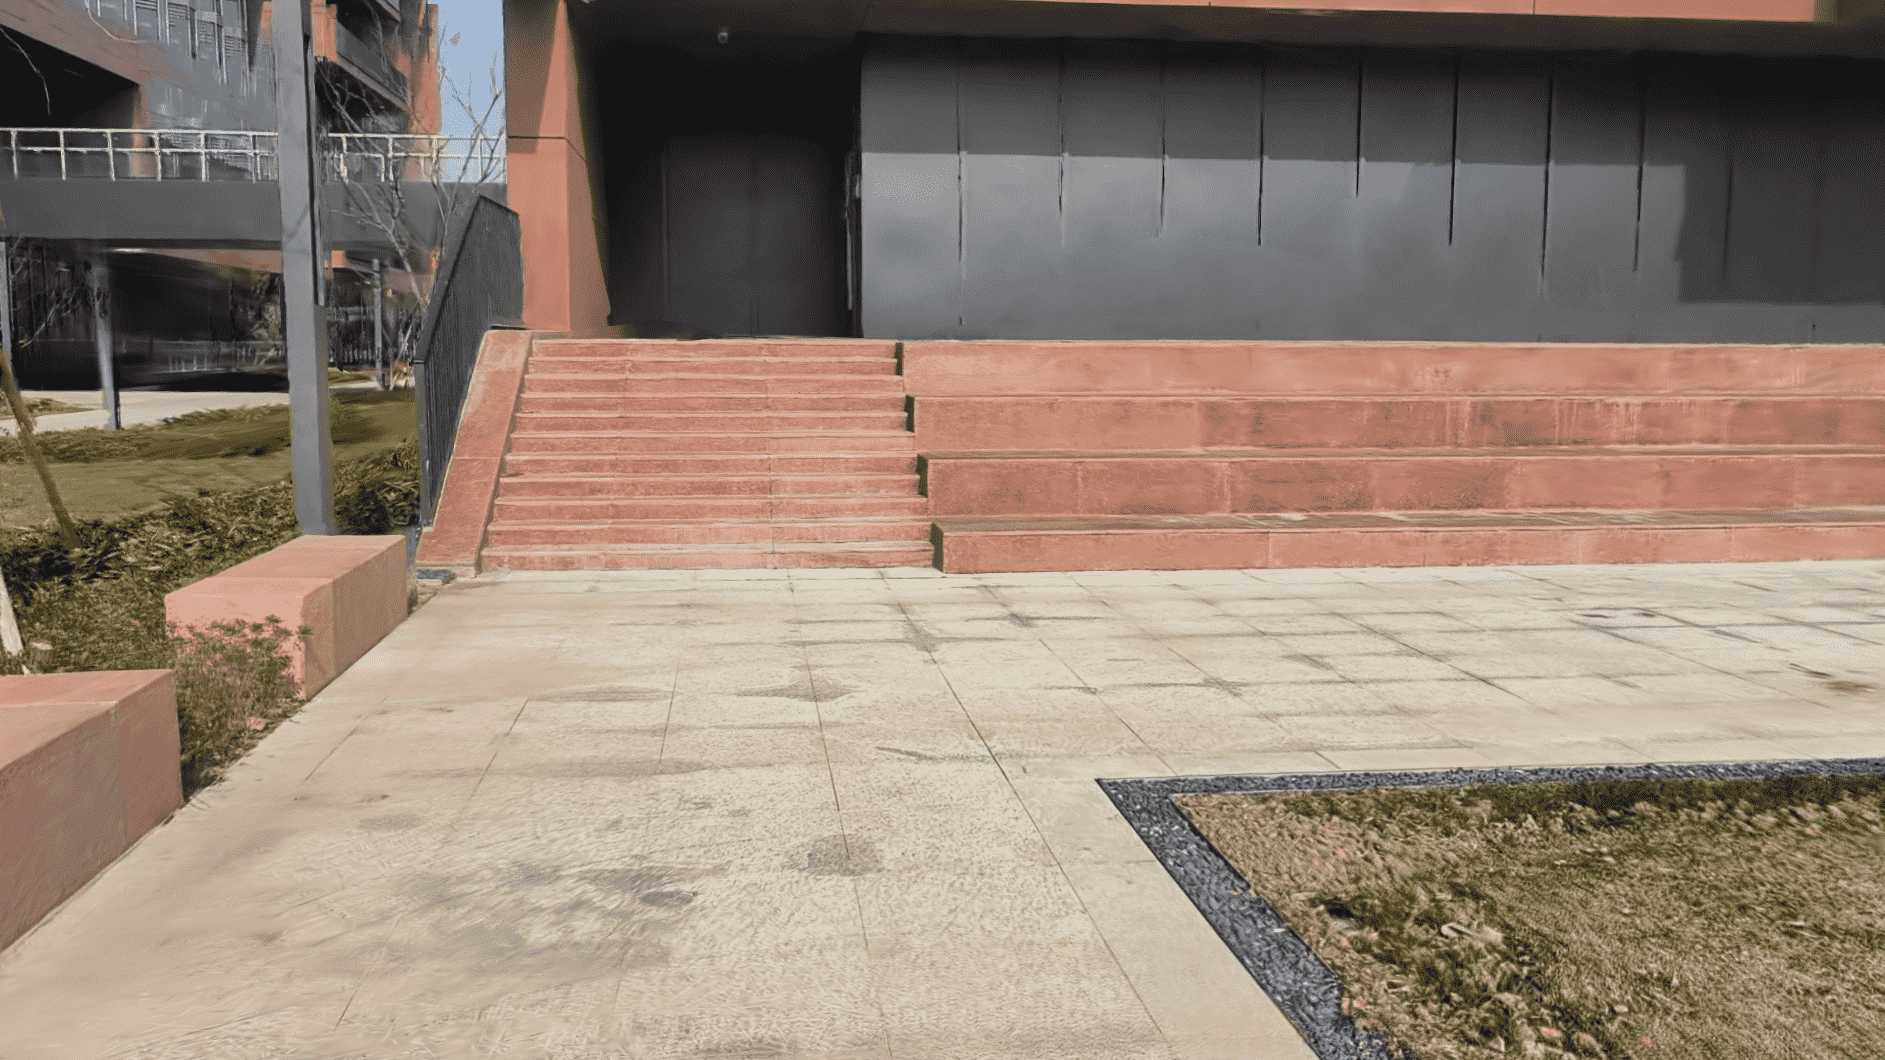} &
        \includegraphics[width=0.24\linewidth]{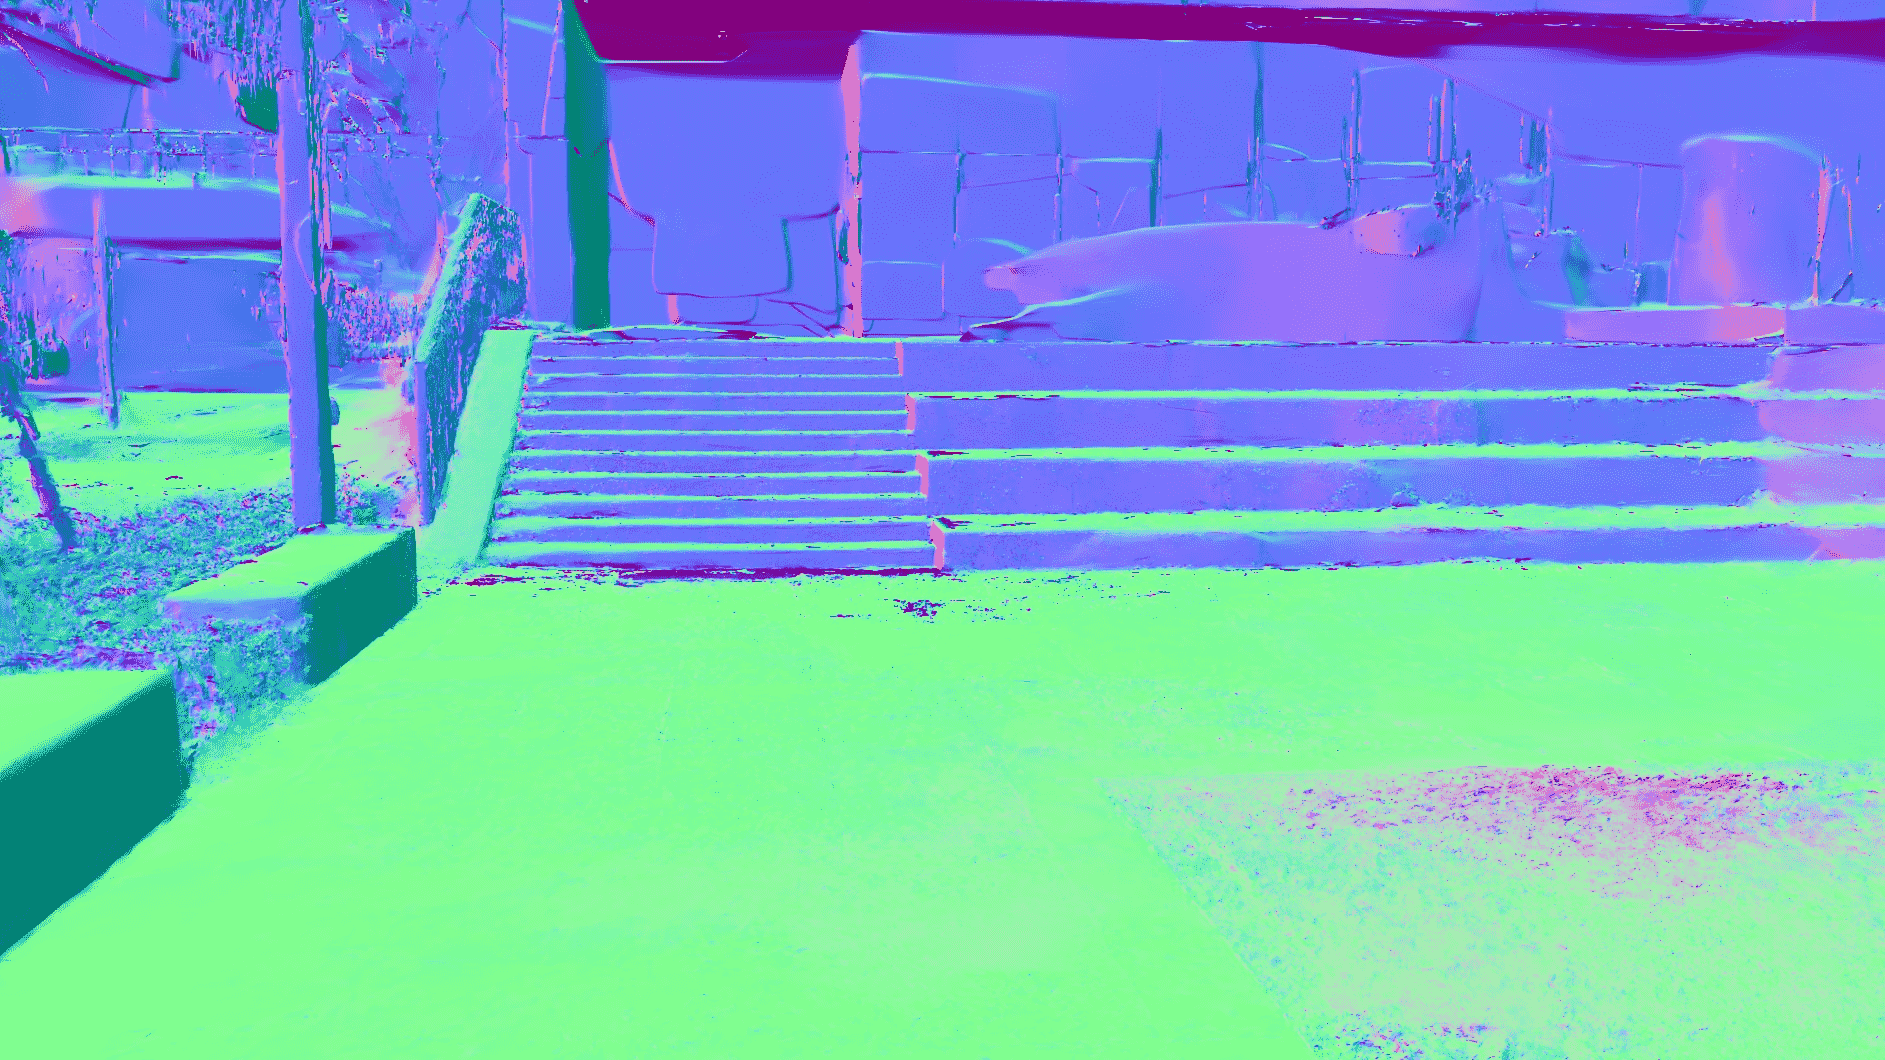} &
        \includegraphics[width=0.24\linewidth]{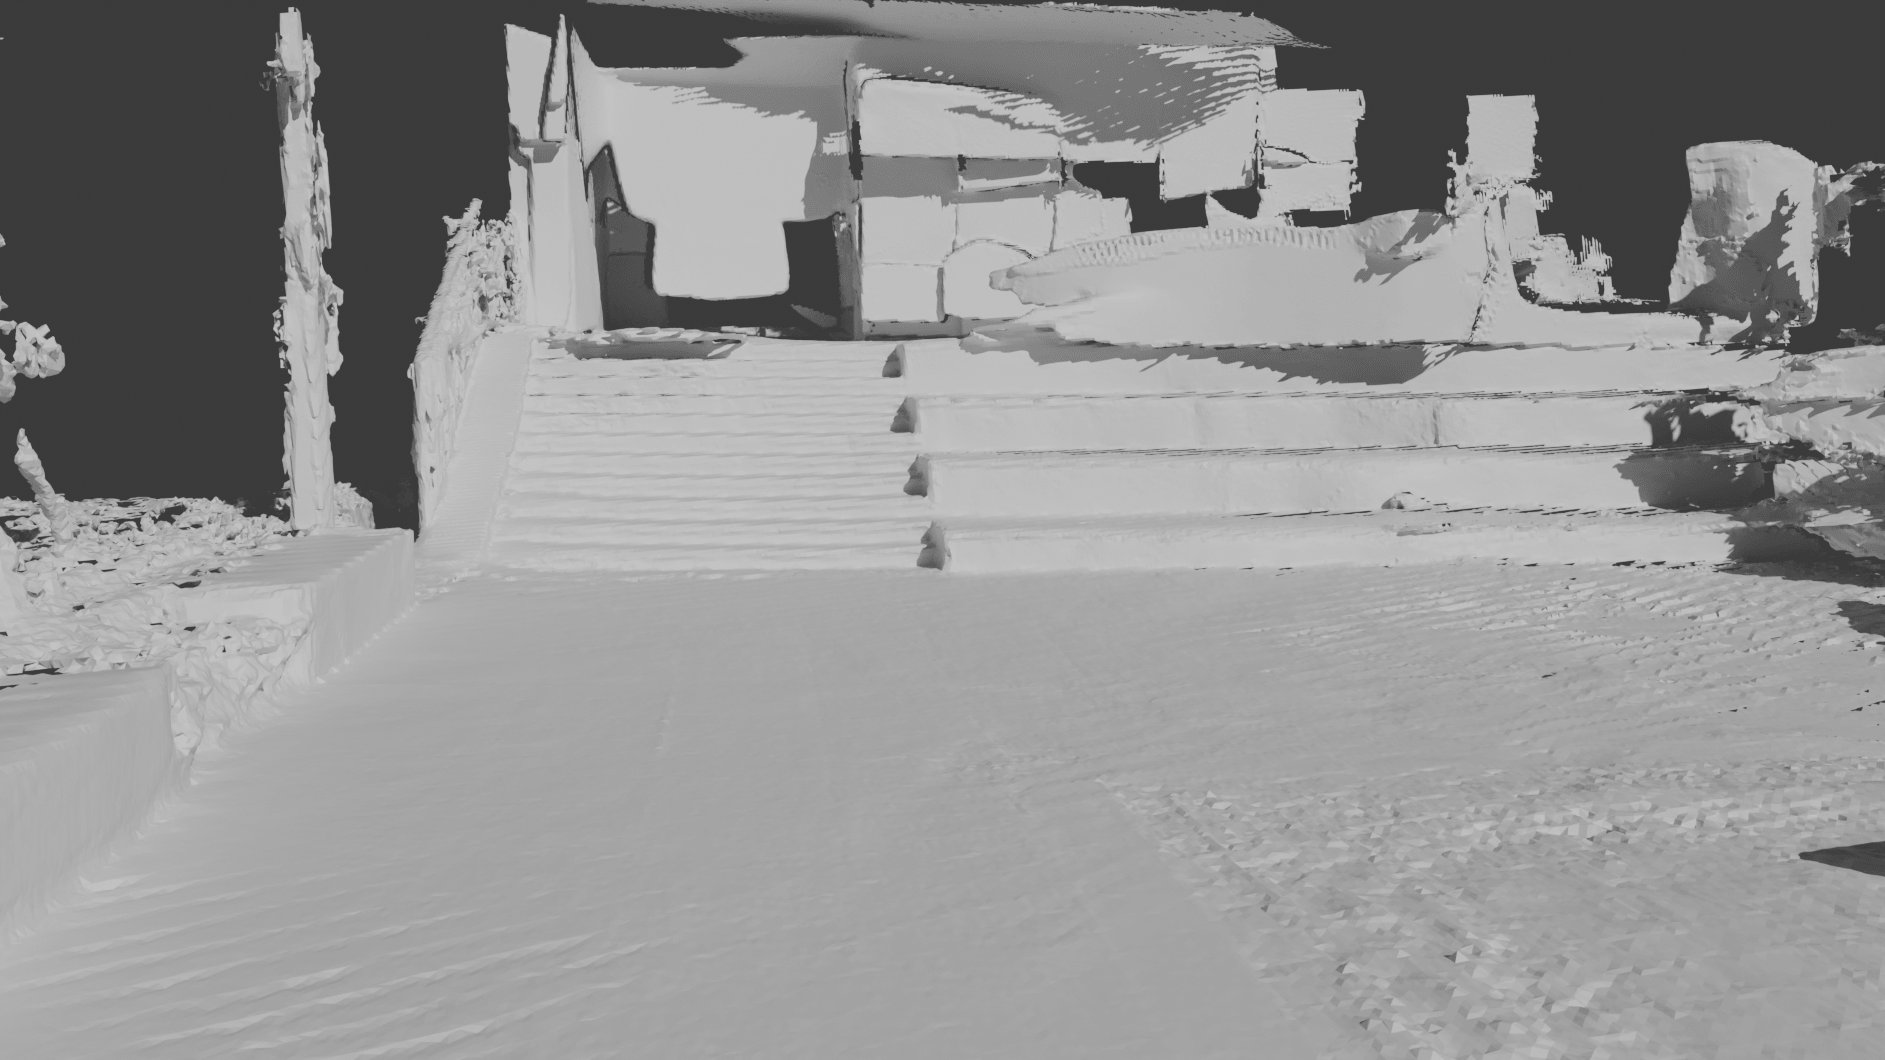} &
        \includegraphics[width=0.24\linewidth]{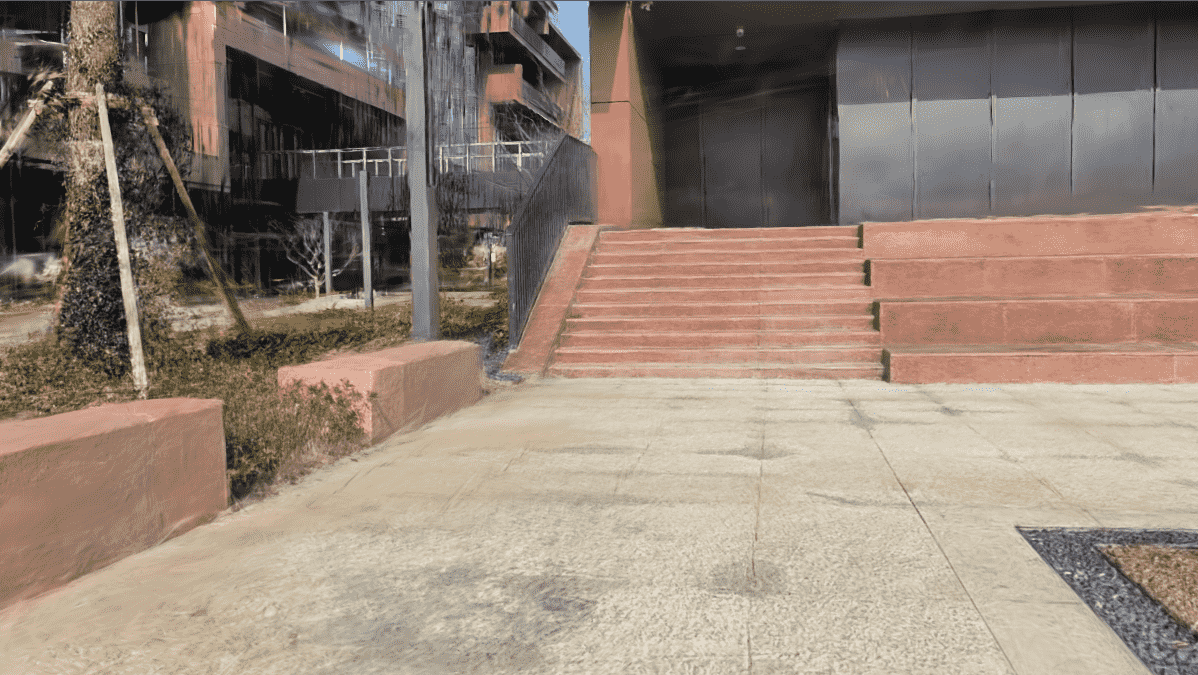} \\

        \includegraphics[width=0.24\linewidth]{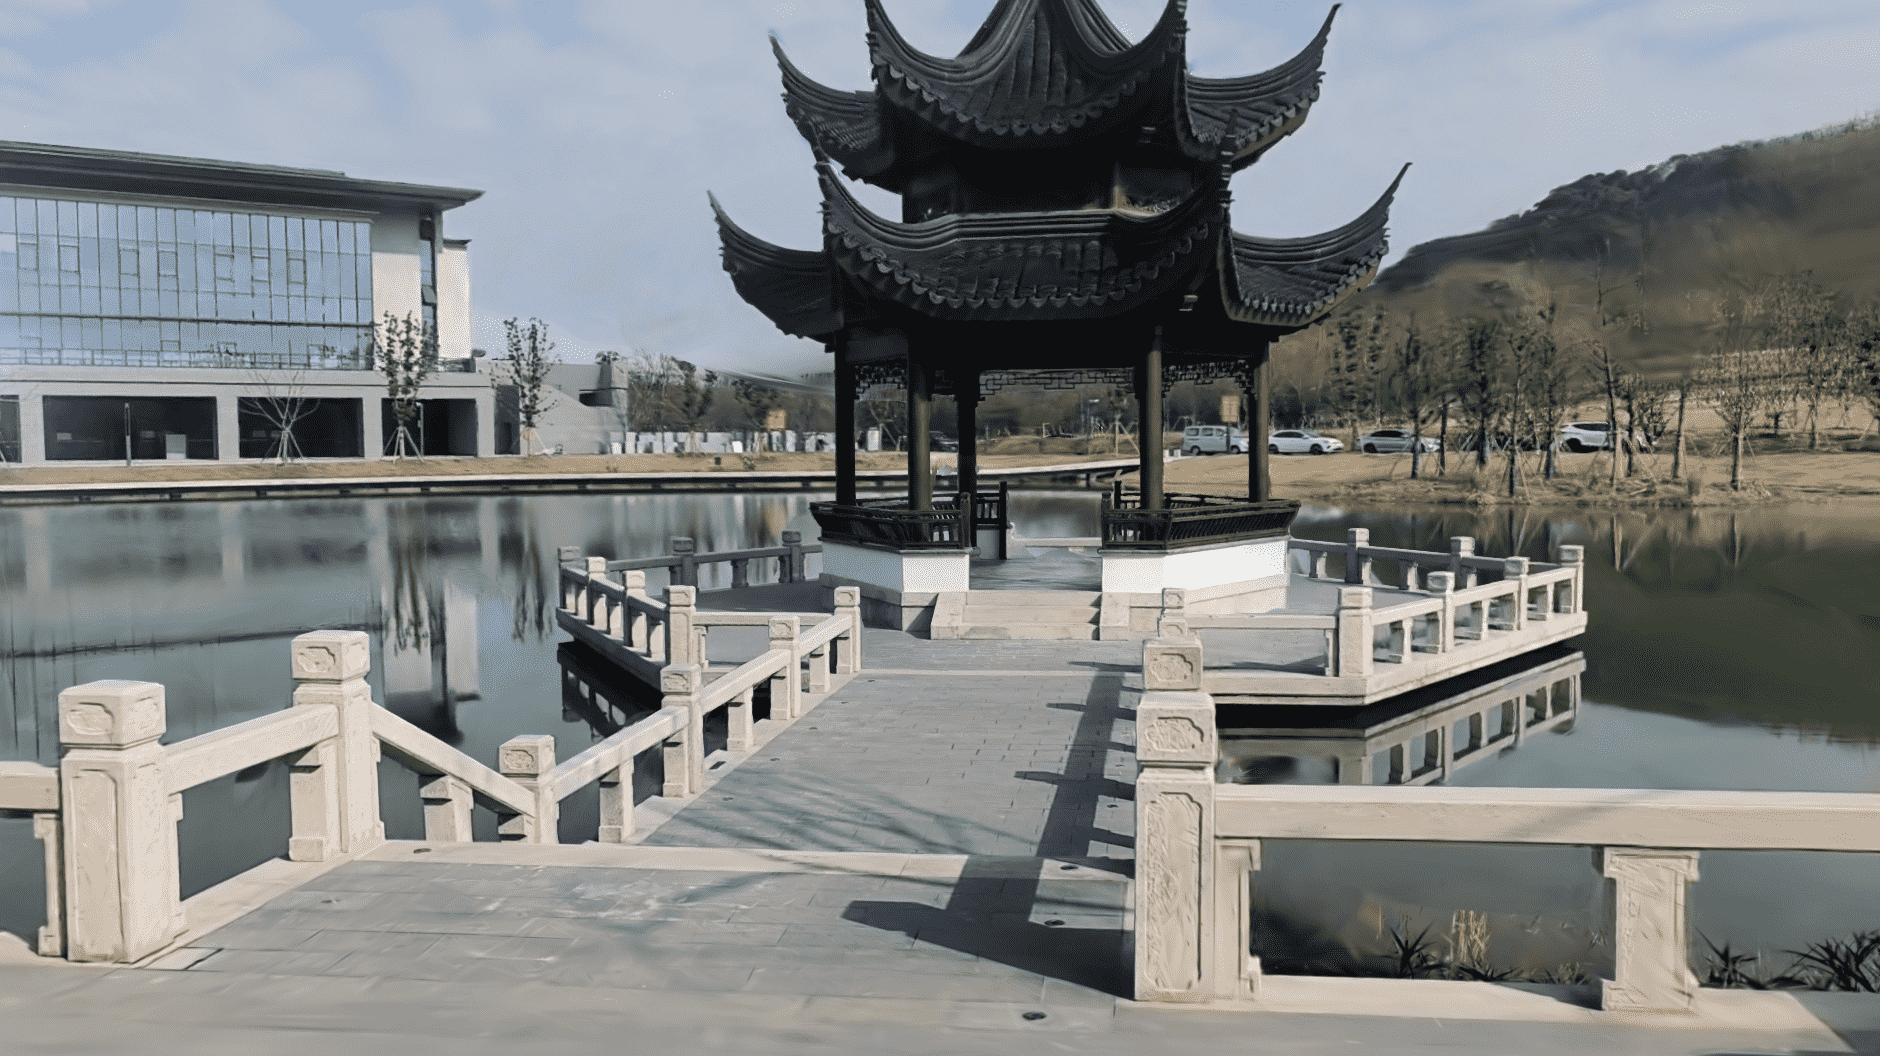} &
        \includegraphics[width=0.24\linewidth]{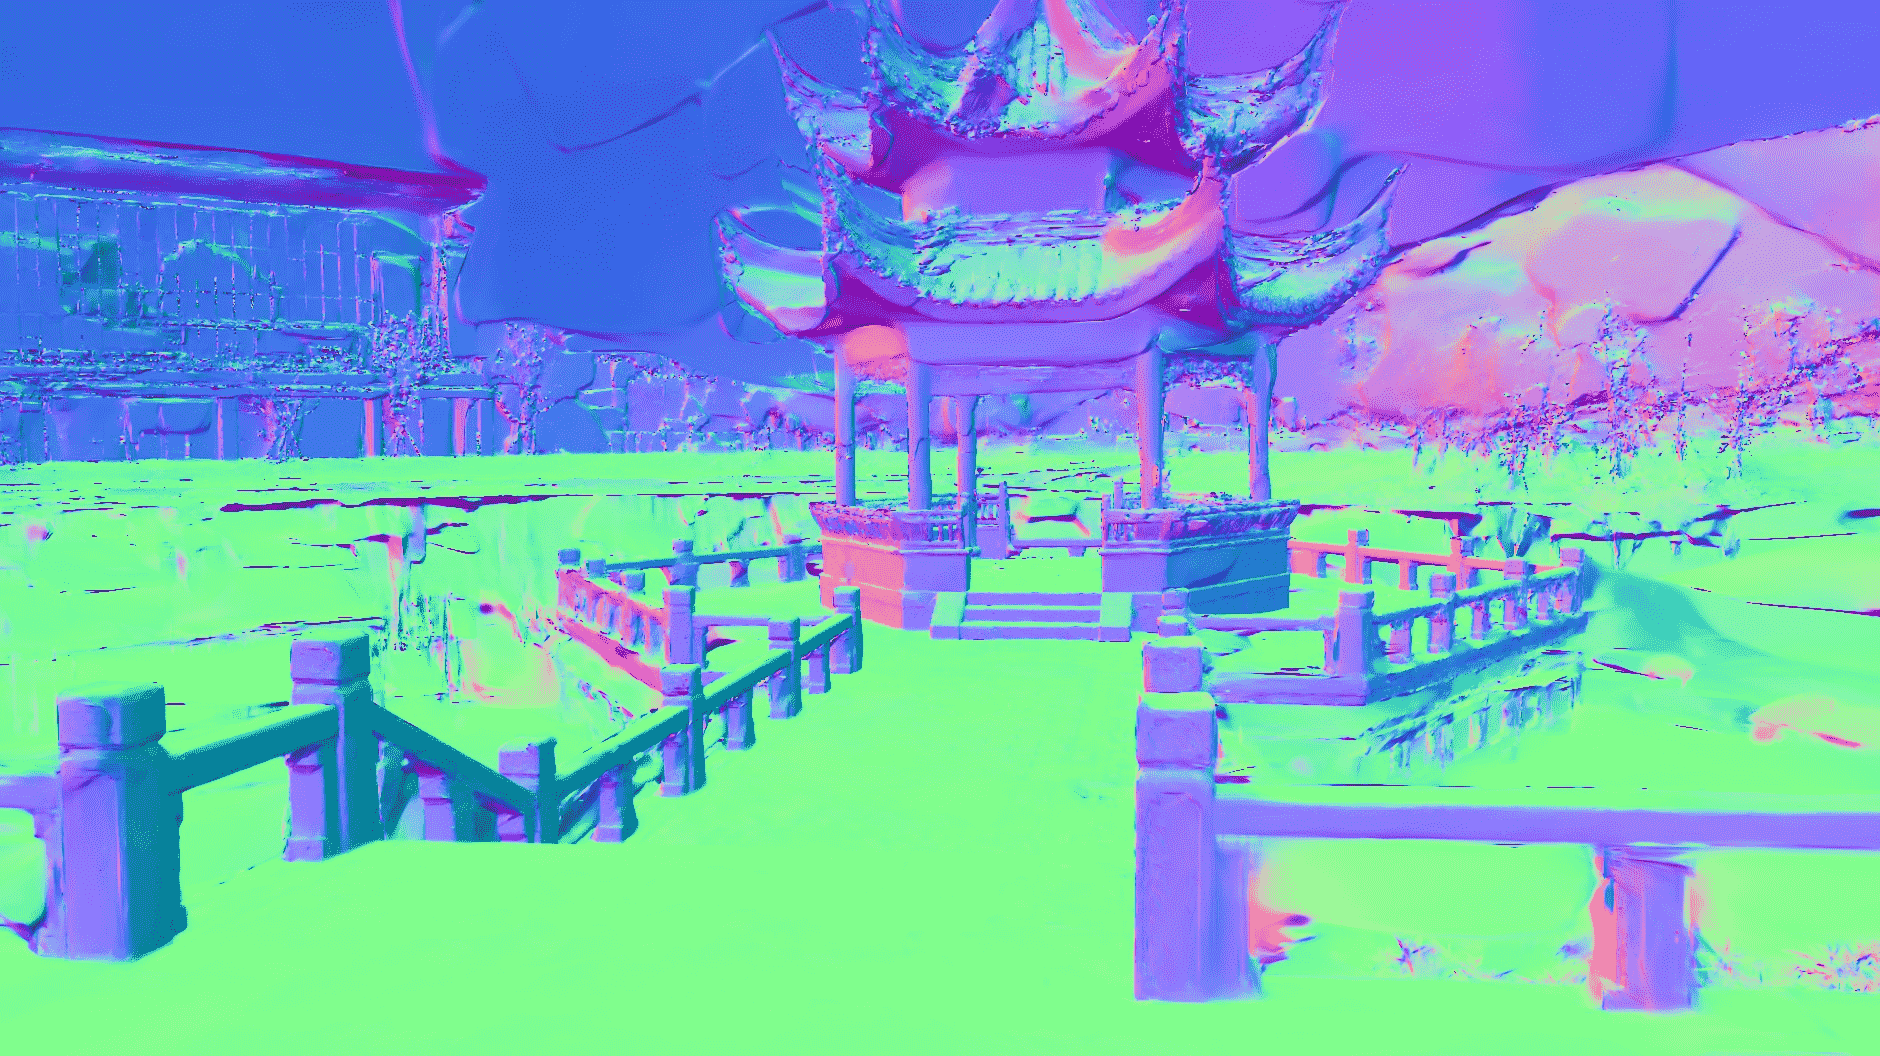} &
        \includegraphics[width=0.24\linewidth]{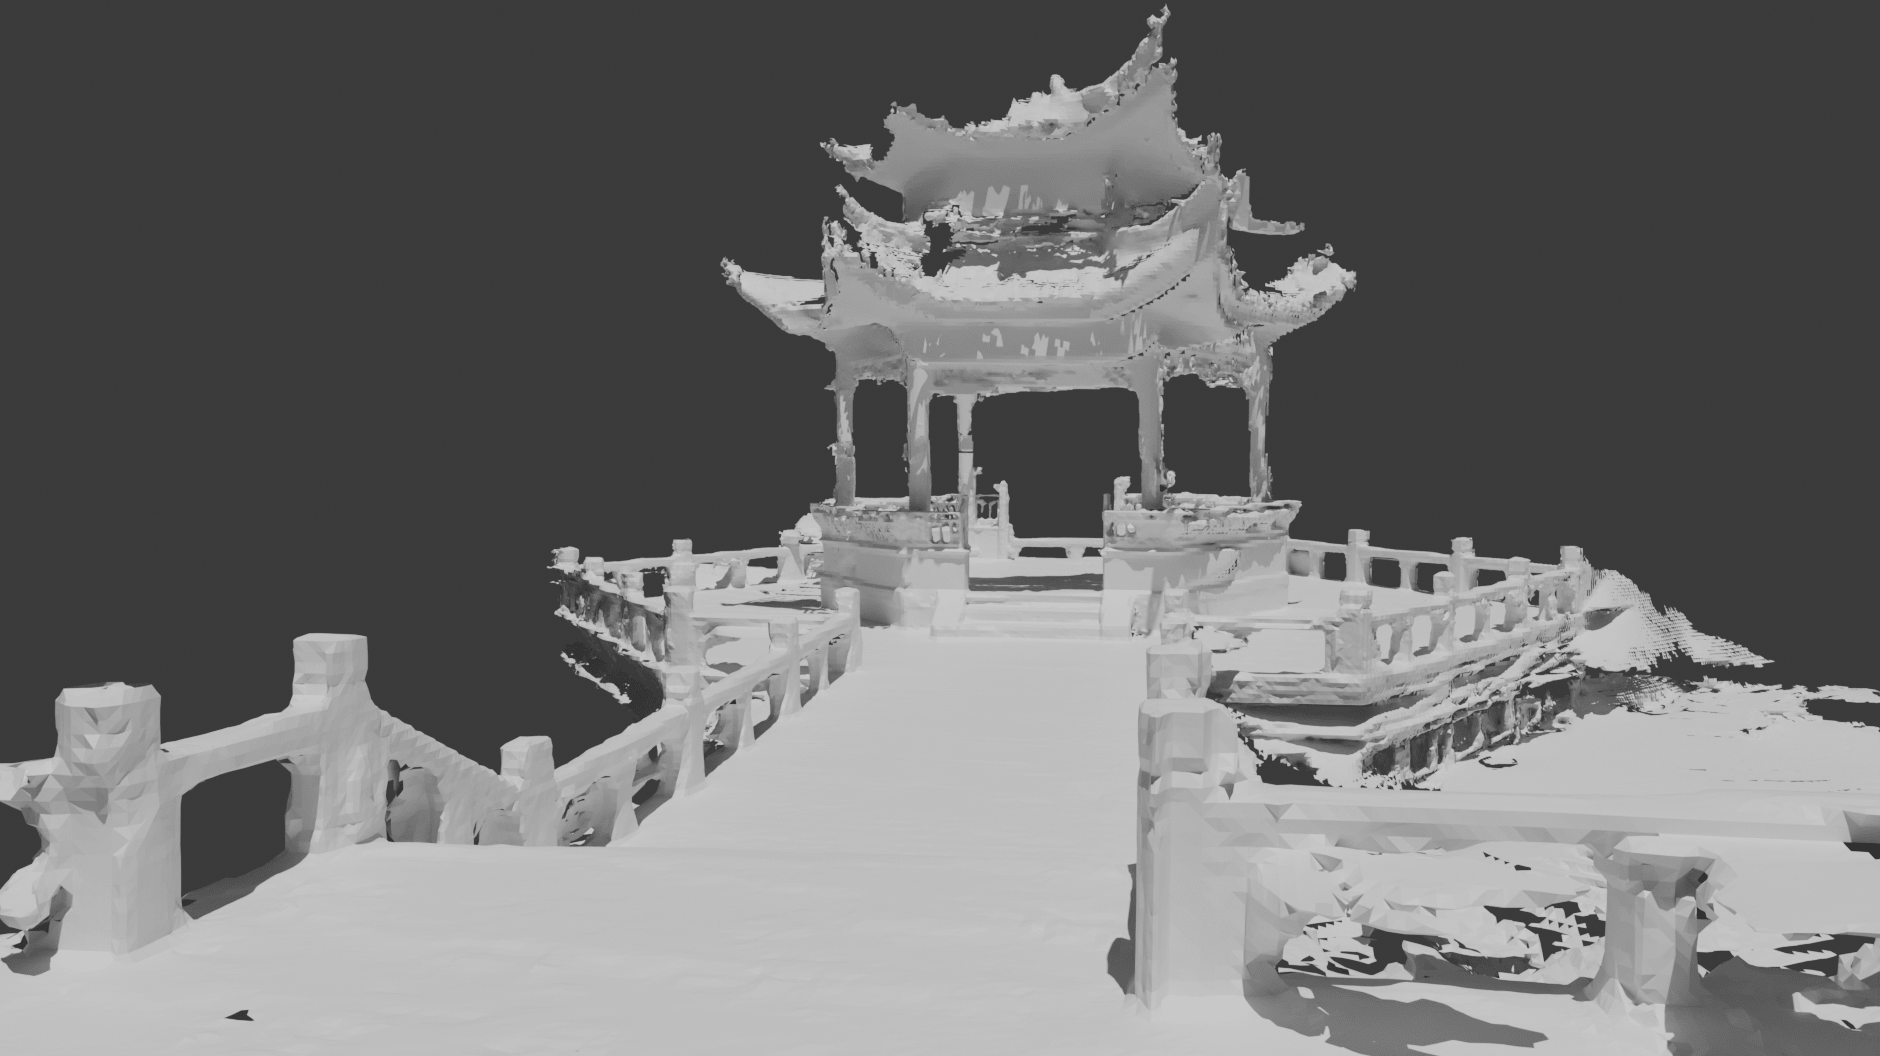} &
        \includegraphics[width=0.24\linewidth]{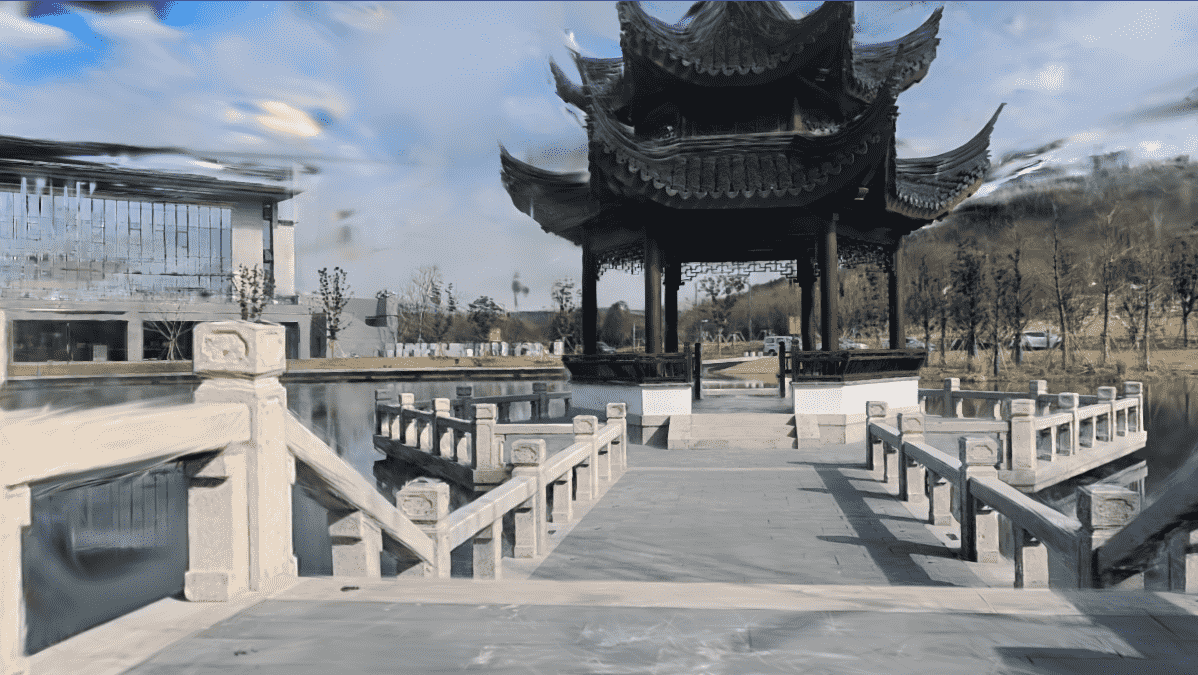} \\

        \includegraphics[width=0.24\linewidth]{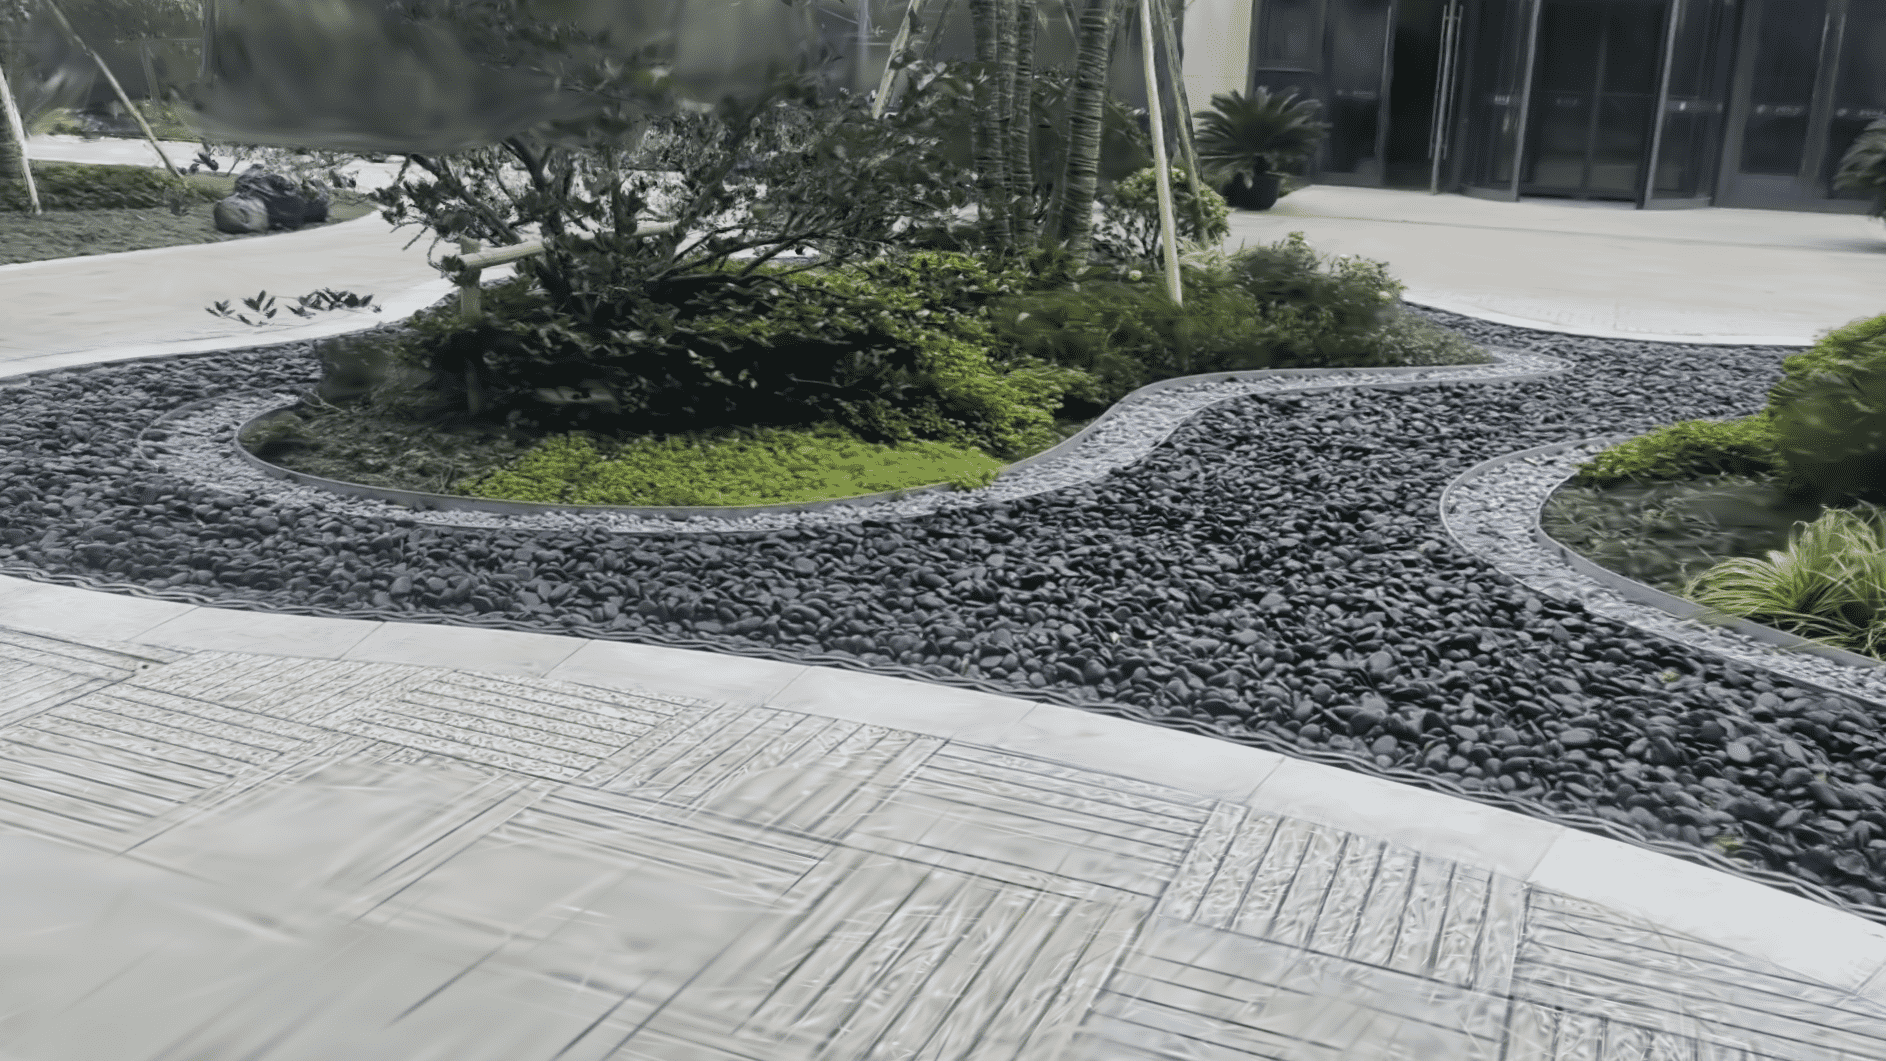} &
        \includegraphics[width=0.24\linewidth]{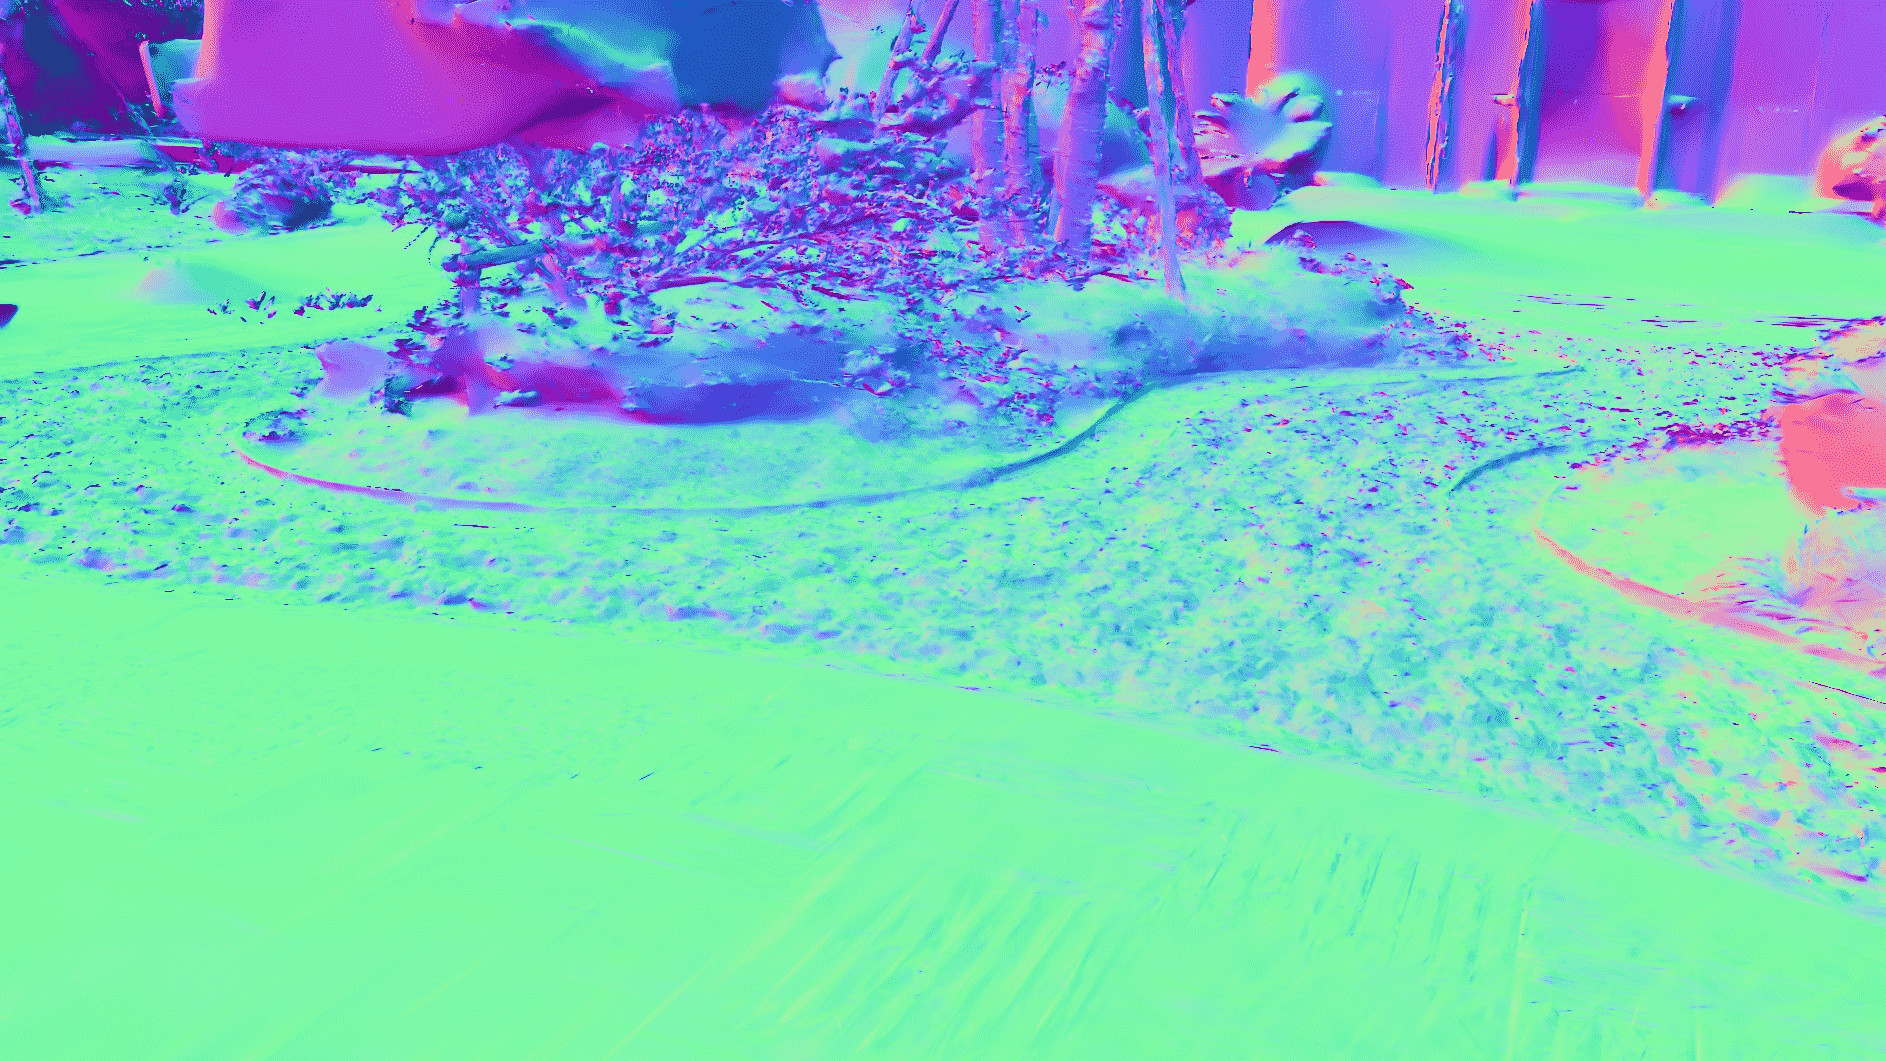} &
        \includegraphics[width=0.24\linewidth]{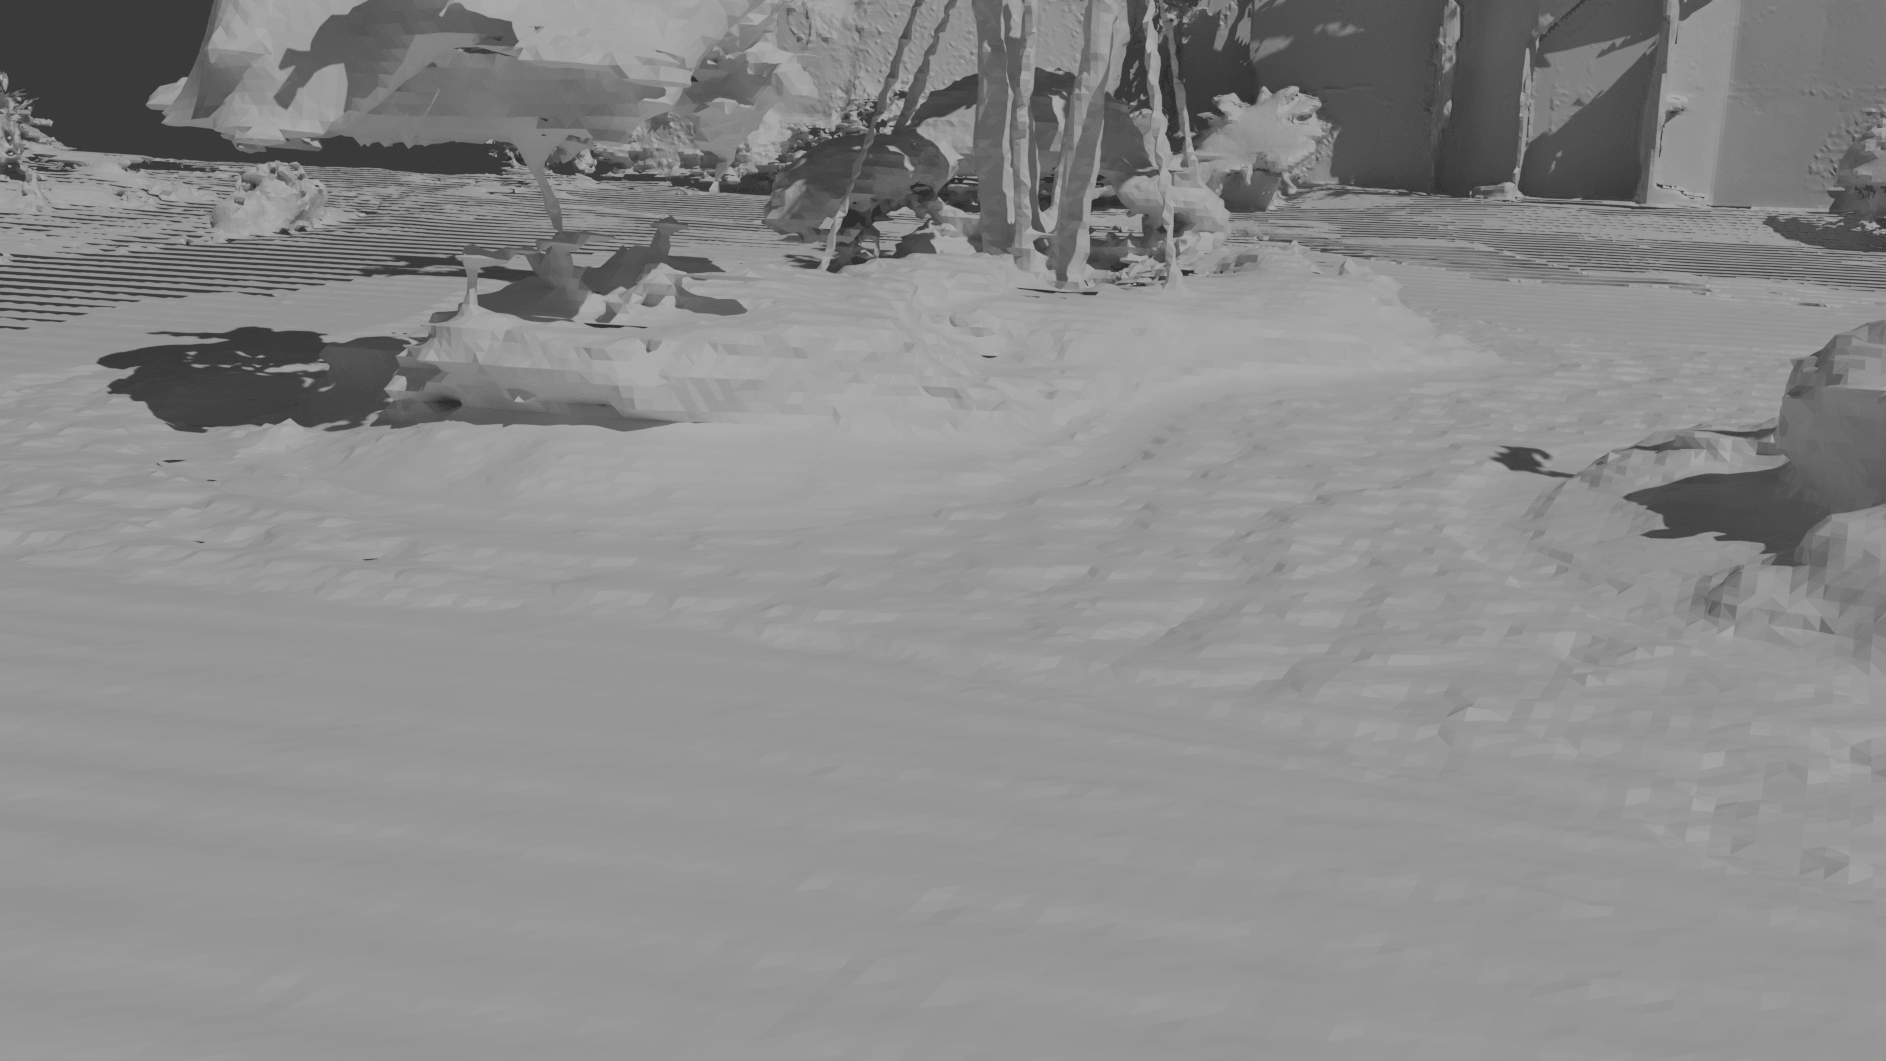} &
        \includegraphics[width=0.24\linewidth]{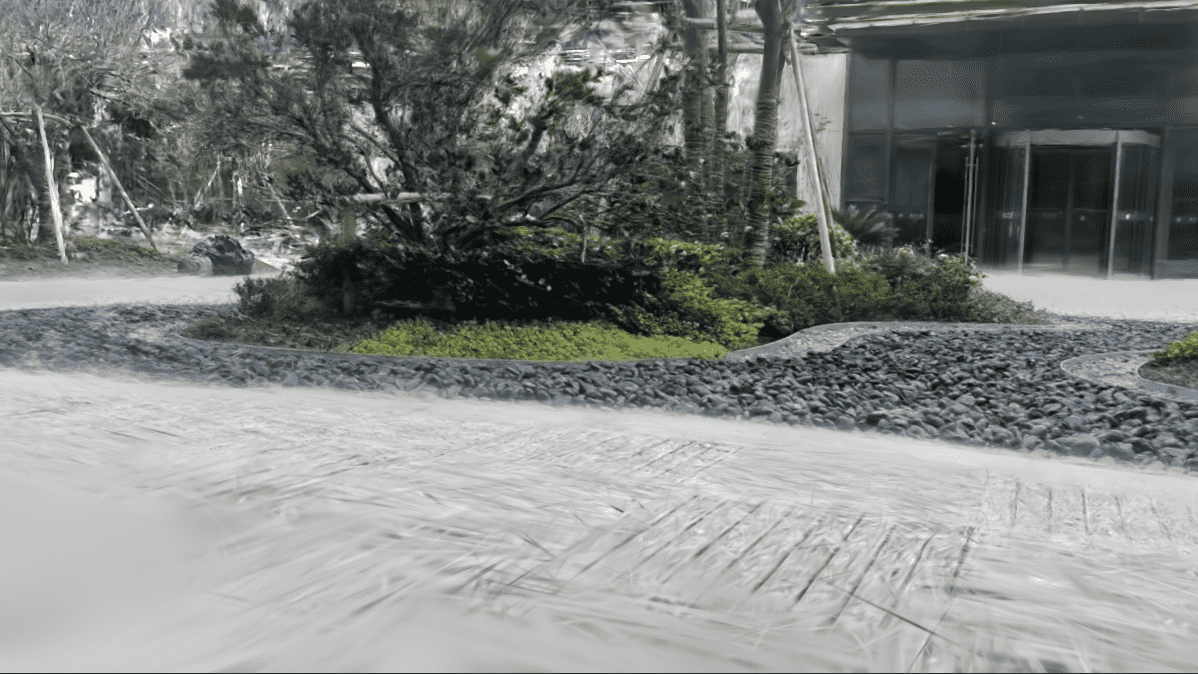} \\

        \small (a) Rendered Image & 
        \small (b) Rendered Normal & 
        \small (c) Extracted Mesh & 
        \small (d) Rendered Robot View \\
    \end{tabular}

    \caption{\textbf{Additional qualitative reconstruction results across various scenes.} 
The reconstruction comprises four components (from left to right): (a) rendered RGB image, (b) rendered normal map, (c) extracted mesh, and (d) simulated robot viewpoint (camera lowered to the eye level of a quadruped robot). These qualitative results further illustrate QuadVerse's visual rendering quality, mesh coherence, and robot-view consistency across diverse outdoor scenes.}
    \label{fig:qualitative_more}
\end{figure*}
