# Supplementary material for: QuadVerse: An Integrated Framework Aligning Visual-Physical Reality for Quadruped Simulation
Source: arXiv:2606.07118 source file (2026-06-08)
Supplement: Supplementary file 6 [file 4_dynamics_analysis.tex]

% !TeX root = ../../main.tex

\section{Further Experiments and Analysis on Dynamics Compensation}
\label{sec:supp_dynamics_analysis}

This section provides a deeper analysis of the residual dynamics module, evaluating its standalone tracking performance, the necessity of its reward components, and its downstream impact on locomotion policy fine-tuning. We also include preliminary sim-to-sim experiments on additional quadruped platforms.

\subsection{Evaluation of the Residual Network}
\label{sec:supp_residual_eval}

\paragraph{Dataset and Evaluation Protocol.}
To rigorously evaluate the generalization of the residual network, we collected a test dataset consisting of 31 distinct trajectories, each lasting 10,000 frames (20 seconds) with a sampling interval of 0.002s, totaling 620 seconds of diverse locomotion data.
For evaluation, we initialize the simulation at the start of each trajectory and perform an open-loop replay of the recorded joint commands. We assess performance based on joint tracking error and gait consistency over the first 3,000 frames of each segment.

\paragraph{Ablation Study.}
Training the residual network requires a delicate balance between minimizing joint tracking error, maintaining gait similarity, and ensuring long-horizon stability. Figure \ref{fig:train_log} illustrates the learning curves for these objectives. The joint compensation performance typically peaks early but must settle into an equilibrium as gait constraints and longer replay horizons are enforced.
We conducted ablation studies on two critical components: the \textit{Gait Reward} and the \textit{Reset Mechanism}. Removing the reset condition (triggered by large deviations) severely degrades joint tracking performance, as the policy overfits to divergent trajectories rather than learning to correct instantaneous dynamics mismatch. Removing gait constraints can further reduce joint-space error, but it induces physically unrealistic artifacts such as foot jitter and ``sliding'' contacts; including gait rewards therefore helps the learned residual dynamics remain accurate in joint space while staying physically consistent at the contact level.

\begin{figure*}[t]
\centering
\includegraphics[width=1.0\linewidth]{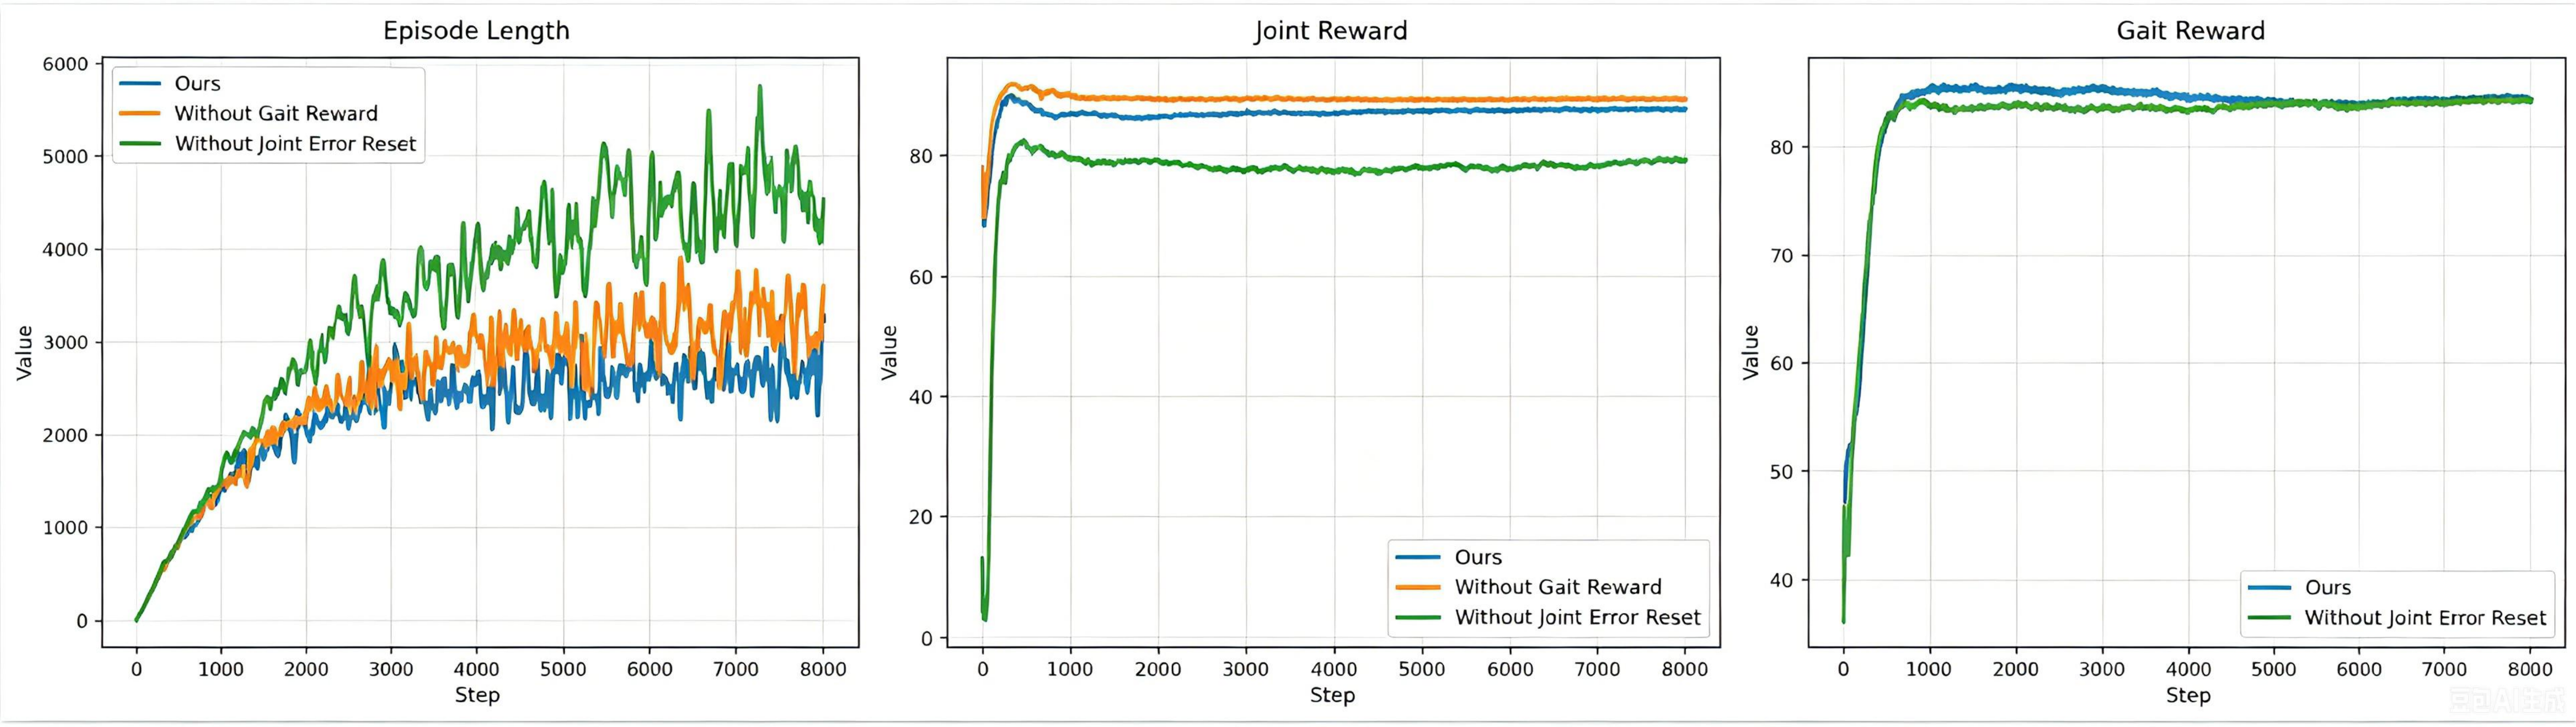}
\caption{Learning curves for average playback length, joint tracking reward, and gait reward. Our method (blue) achieves a balanced performance, whereas removing gait rewards (orange) or reset conditions (green) leads to suboptimal convergence in stability or tracking accuracy.}
\label{fig:train_log}
\end{figure*}

\subsection{Cross-Platform Sim-to-Sim Transfer}
\label{sec:supp_cross_platform}

To assess whether the proposed residual dynamics compensation pipeline is specific to a single robot platform, we further conduct cross-platform sim-to-sim transfer experiments on Unitree Go1 and Unitree A2. 
Due to limited access to additional hardware platforms, these experiments are performed as Isaac Gym-to-MuJoCo transfer rather than full real-world deployment. 
For each robot, we train the residual compensator in Isaac Gym using replay data generated from the target MuJoCo model, and evaluate whether the compensated Isaac Gym replay better matches the MuJoCo reference.

We adopt the same open-loop joint-space replay protocol as in Sec.~\ref{sec:supp_residual_eval}. 
Specifically, we compare the nominal simulator and the residual-compensated simulator by measuring joint-space replay error under identical command replay. 
The compensator consistently improves replay fidelity across platforms. 
For Unitree Go1, the residual compensator reduces the joint-space replay error by 72.5\%; for Unitree A2, the reduction is 85.4\%. 
For reference, the corresponding improvement on Unitree Go2 is 66.1\%. Figures~\ref{fig:cross_platform_joint_space} provides representative joint-space replay curves, analogous to Fig.~\ref{fig:joint_space} in the main paper. 
In both cases, the compensated simulator tracks the reference trajectory much more closely than the nominal simulator, indicating that the benefit of residual compensation is not limited to a single quadruped embodiment. 

\begin{figure*}[t]
    \centering
    \begin{subfigure}[t]{0.48\linewidth}
        \centering
        \includegraphics[width=\linewidth]{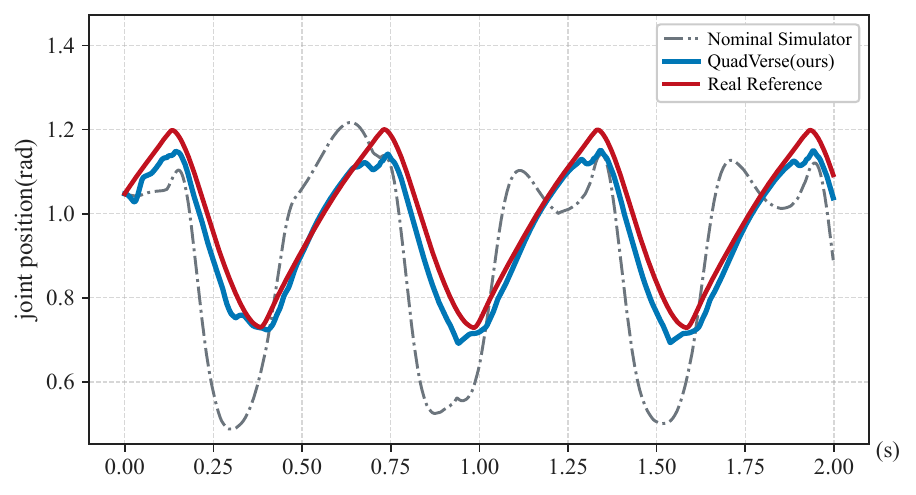}
        \caption{Unitree Go1}
        \label{fig:go1_joint_space}
    \end{subfigure}
    \hfill
    \begin{subfigure}[t]{0.48\linewidth}
        \centering
        \includegraphics[width=\linewidth]{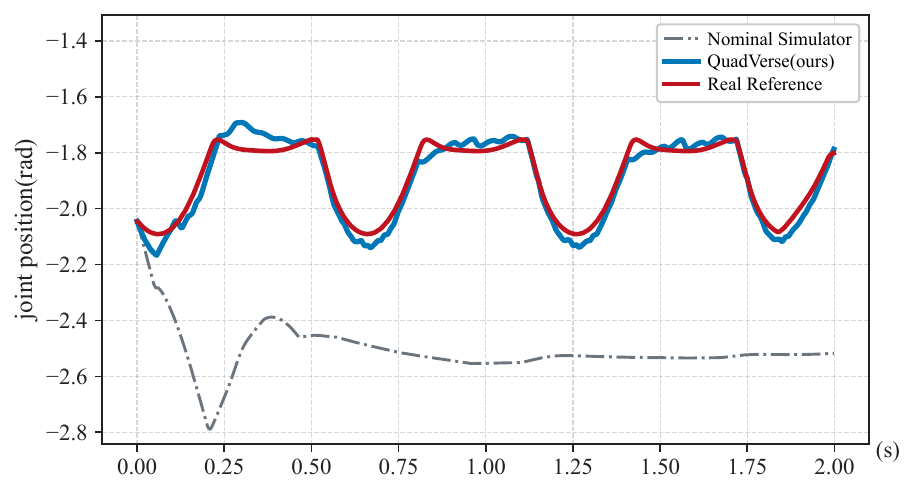}
        \caption{Unitree A2}
        \label{fig:a2_joint_space}
    \end{subfigure}
    \caption{\textbf{Cross-platform joint-space replay in sim-to-sim transfer.}
    Open-loop joint-space replay on Unitree Go1 (left) and Unitree A2 (right). 
    On both platforms, the residual-compensated simulator tracks the reference trajectory more closely than the nominal simulator.}
    \label{fig:cross_platform_joint_space}
\end{figure*}

\subsection{Locomotion Policy Fine-tuning and Deployment}
\label{sec:supp_locomotion_finetuning}

To evaluate whether the compensated dynamics benefits downstream policy learning, we fine-tune a locomotion policy with the frozen residual compensator inserted into the simulation loop. 
Both the nominal pre-training and QuadVerse fine-tuning use the Heterogeneous Information Matching (HIM) locomotion framework with a control frequency of 50\,Hz. 
During fine-tuning, the residual compensator is treated as part of the environment dynamics and its parameters are kept fixed. 
We fine-tune from a pre-trained locomotion policy rather than training from scratch because the pre-trained policy already provides a strong locomotion prior. 
This makes adaptation more sample-efficient and keeps exploration close to the replay distribution where the residual compensator is reliable, whereas early-stage training from scratch may visit highly out-of-distribution actions and states that are not covered by the compensation model.

We evaluate the resulting policies on five real-world locomotion tasks specified by velocity commands: \textit{right-turn}, \textit{left-turn}, \textit{slow-forward}, \textit{fast-forward}, and \textit{figure-eight}, with 10 trials per task. 
As shown in Fig.~\ref{fig:all_traj}, the QuadVerse policy consistently reduces trajectory error across different locomotion modes compared with the nominal policy. 
The improvement is especially visible in turning and figure-eight maneuvers, where actuator mismatch can accumulate into substantial heading and curvature errors; fine-tuning with compensated dynamics improves command tracking and yields more stable real-world trajectories. 
The remaining difference between left-turn and right-turn performance is mainly attributed to the command-tracking bias of the pre-trained locomotion policy, which can already favor one turning direction over the other in simulation.

\begin{figure*}[t]
\centering
\includegraphics[width=1.0\linewidth]{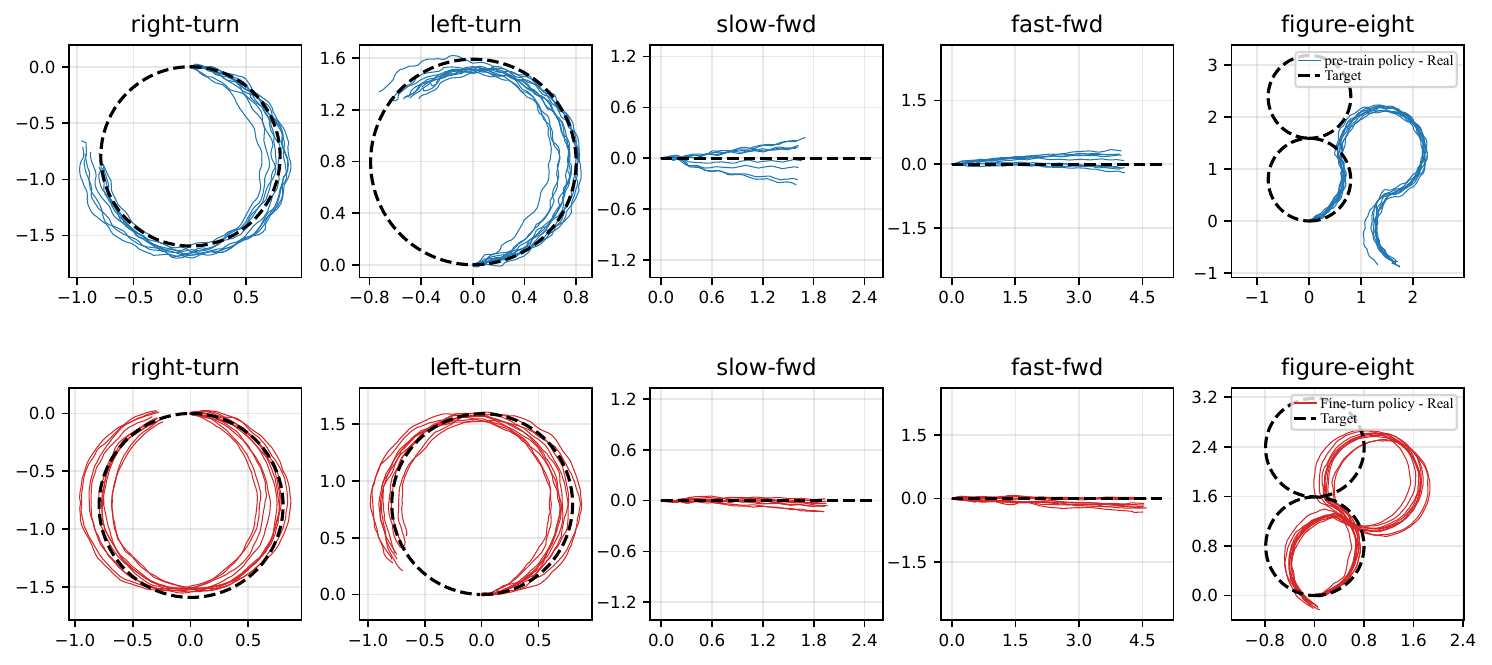}
\caption{\textbf{Additional real-world locomotion tracking results.}
Trajectory error across five locomotion tasks. 
The QuadVerse policy consistently reduces tracking error compared with the nominal policy across different commanded motion patterns.}
\label{fig:all_traj}
\end{figure*}
