# Supplementary material for: QuadVerse: An Integrated Framework Aligning Visual-Physical Reality for Quadruped Simulation
Source: arXiv:2606.07118 source file (2026-06-08)
Supplement: Supplementary file 7 [file 5_navigation_details.tex]

% !TeX root = ../../main.tex

\section{Details of Navigation Policy}
\label{sec:supp_navigation_details}

\subsection{Task Formulation and Evaluation Protocol} 
\label{sec:supp_nav_task}
We evaluate the full QuadVerse framework through an outdoor visual goal-seeking task. The robot is required to locate and approach a colored target cone using ego-centric RGB observations within a maximum episode duration of $T_{\max}=25$ seconds. An episode is considered successful if the robot's reference point reaches within $\epsilon=0.35$\,m of the target cone. To prevent the policy from overfitting to a fixed start-goal configuration, both the robot initial state and the goal location are randomized within predefined feasible regions during training and evaluation. For real-world evaluation, we conduct 25 trials with randomized initial robot poses and goal locations. Simulation results are averaged over 200 episodes. Success rate (SR) is defined as the fraction of successful episodes, and average reaching time (ART) is computed over all trials, with failed trials assigned the maximum episode duration $T_{\max}$.

\subsection{Navigation Policy Training} 
\label{sec:supp_nav_hierarchy}
The navigation policy is trained entirely within the QuadVerse simulation framework. We first reconstruct the deployment scene from captured RGB videos and use the optimized 3DGS representation to render ego-centric visual observations consistent with the robot's head-mounted camera. The reconstructed scene is also converted into a collision-ready semantic mesh and calibrated into a contact-calibrated terrain. The replay-trained residual actuator compensator is then frozen and inserted into the simulation loop, allowing the navigation policy to be trained under dynamics that better match real-world execution. The navigation policy itself does not use real-world navigation rollouts for training or fine-tuning. After training in simulation, the visual navigation policy is deployed zero-shot to the physical robot.

We use a hierarchical control architecture to decouple visual navigation from low-level locomotion. 
The high-level visual navigation policy runs at 5\,Hz and outputs a velocity command $\boldsymbol{v}_{\mathrm{cmd}}=(v_x, v_y, \omega_{\mathrm{yaw}})$, which is then tracked by the low-level locomotion controller.
The low-level controller runs at 50\,Hz and generates joint position targets from the commanded velocity and proprioceptive observations. During navigation policy training, the low-level locomotion controller is frozen, while the residual actuator compensator remains active in the simulation loop. The high-level policy observation consists of three components: 
(1) visual observation, ego-centric RGB images rendered from the reconstructed 3DGS scene. A frozen visual encoder is used to extract image features.
(2) task command, a one-hot encoding of the target color or target category.
(3) proprioceptive history, robot state history including base angular velocity, projected gravity, joint states, and the previous velocity command.
The policy output is squashed by a $\tanh$ activation and then scaled to predefined command limits, i.e., $|v_x| \leq 0.9$\,m/s, $|v_y| \leq 0.4$\,m/s, and $|\omega_{yaw}| \leq 1.0$\,rad/s.

The high-level visual navigation policy is modeled as an actor-critic network and trained using PPO. To handle partial observability, the policy includes an LSTM recurrent module. Training is performed in the QuadVerse simulation environment using 1024 parallel environments for 150 iterations. We apply visual and dynamics domain randomization to improve deployment robustness. Visual randomization includes camera extrinsic perturbation, image noise, brightness variation, and motion blur. Dynamics randomization includes perturbations to robot mass, friction, external disturbances, and initial robot states. 

\begin{table}[h]
\caption{Reward Function for the High-Level Navigation Policy}
\label{tab:nav_rewards}
\centering

\begin{tabular}{llc}
\toprule
\textbf{Reward Term} & \textbf{Mathematical Formulation} & \textbf{Weight} \\
\midrule
\multicolumn{3}{c}{\textit{Task Achievement}} \\
\midrule
Reach Goal & $\mathbb{I}(d_t < 0.35)$ & $0.5$ \\
Goal Progress & $(d_{t-1} - d_t)\,\mathbb{I}(d_t > 0.35)$ & $5.0$ \\
Goal Close & $\mathrm{clip}\!\left(\frac{0.75-d_t}{0.75-0.35},0,1\right)$ & $0.2$ \\
Goal Heading & $1 - 2|\Delta\psi_t|/\pi$, if $d_t>0.35$; otherwise $1$ & $0.3$ \\
Stand Still & $\mathbb{I}(d_t < 0.35)(\|\boldsymbol{v}_{cmd}\|_2+0.4)^{-1}$ & $1.0$ \\
\midrule
\multicolumn{3}{c}{\textit{Command Tracking \& Regularization}} \\
\midrule
Track Lin. Vel. & $\exp(-\|\boldsymbol{v}_{xy}^{cmd}-\boldsymbol{v}_{xy}^{base}\|_2^2/0.25)$ & $0.2$ \\
Track Ang. Vel. & $\exp(-(\omega_z^{cmd}-\omega_z^{base})^2/0.25)$ & $0.2$ \\
Action Magnitude & $\|\boldsymbol{a}_{high}\|_2^2$ & $-0.002$ \\
\bottomrule
\end{tabular}
\end{table}

\subsection{Reward Design} 
\label{sec:supp_nav_reward} 
The high-level policy is trained with a composite reward consisting of target-reaching rewards, planar progress and heading terms, velocity-tracking terms, and an action-magnitude penalty. Let $d_t$ denote the planar head-to-goal distance and $\Delta\psi_t$ denote the yaw error between the robot heading and the goal direction. The configured reward weights are shown in Table~\ref{tab:nav_rewards}; internally, each configured weight is multiplied by the high-level control period.
