# Supplementary material for: QuadVerse: An Integrated Framework Aligning Visual-Physical Reality for Quadruped Simulation
Source: arXiv:2606.07118 source file (2026-06-08)
Supplement: Supplementary file 8 [file 6_conclusion.tex]

\section{Conclusion}
\label{sec:supp_conclusion}

This supplementary material provides implementation details and extended analyses that support the main paper. 
We first present the reconstruction losses and semantic mesh calibration protocol, including semantic Gaussian training, LLM-assisted coarse friction priors, and trajectory-based posterior friction search. 
We then detail the residual actuator compensation module, including its network architecture, replay initialization, reward design, and ablation studies. 
Additional reconstruction examples, cross-platform sim-to-sim transfer results, locomotion fine-tuning experiments, and navigation policy details further demonstrate how the components of QuadVerse are instantiated in practice. 
Together, these supplementary results clarify the calibration and training procedures used to construct the aligned simulation environment for zero-shot quadruped visual-navigation deployment.
